# Supplementary material for: A Sound and Complete Equational Theory for 3-Qubit Toffoli-Hadamard Circuits
Source: arXiv:2407.11152 ancillary file (2024-08-12)
Supplement: Supplementary file 1 [file supplement.pdf]

# Supplement: A Sound and Complete Equational Theory for 3-Qubit Toffoli-Hadamard Circuits

Matthew Amy  
Simon Fraser University  
Burnaby, Canada  
matt.amy@sfu.ca

Neil J. Ross  
Dalhousie University  
Halifax, Canada  
neil.jr.ross@dal.ca

Scott Wesley  
Dalhousie University  
Halifax, Canada  
scott.wesley@dal.ca

This supplement to “A Sound and Complete Equational Theory for 3-Qubit Toffoli-Hadamard Circuits” establishes the derivations necessary to prove Theorem 4.1 and Corollary 4.2.

## 1 Derivations for $W(E_8)$

This supplement first shows that all of the relations in  $R_D$  are derivable from  $R_0$ . It is then shown that all of the relations in  $R_{D(E_8)}$  and  $R_{E_8}$  are derivable from  $R_0$ . To simplify the later steps, some lemmas are derived from  $R_0$  regarding global phases and control manipulation. We represent our derivations as described in Appendix B.3 of the main paper. The well-foundedness and acyclicity of each derivation is validated in TIETZE. Furthermore, TIETZE also validates the validity of each relation in  $R_0$ ,  $R_{D(E_8)}$ , and  $R_{E_8}$  relative to the intended semantics. It then follows by Theorem B.25 of the main paper, that the claims in Sections 4.3 and 4.4 of the main paper hold.

In a derivation, an underline (resp. overline) denotes the left (resp. right) side of a relation. Relation  $n$  in Figure 4 of the main paper is denoted  $(n)$ . The Coxeter relation for  $r_j$  and  $r_k$  is denoted  $(j;k)$ . In terms of derived relations, the  $n$ -th order, symmetry, bifunctionality, and commutator relations are denoted  $C_n$ ,  $B_n$ ,  $S_n$ , and  $E_n$  respectively. The  $n$ -th global phase and control lemmas are denoted  $\gamma_n$  and  $\chi_n$ , respectively. For example, the following derivation replaces  $CCX_{0,1}$  with  $K_{1,2} \cdot CCX_{0,2} \cdot K_{1,2}$  via an application of Relation (17), and then replaces  $K_{1,2} \cdot K_{1,2}$  with  $\varepsilon$  via an application of Relation (23). The resulting *derived relation* is named  $C_1$ .

$$(C_1) : K_{1,2} \cdot \underline{CCX_{0,1}} \xrightarrow{(17)} \underline{K_{1,2} \cdot \overline{K_{1,2} \cdot CCX_{0,2} \cdot K_{1,2}}} \xrightarrow{(23)} CCX_{0,2} \cdot K_{1,2}$$

### 1.1 Deriving the Circuit Relations

This section begins by deriving all order relations. Then all symmetry relations are derived. Then all bifunctionality relations are derived. Finally, all commutator relations are derived. Derivations may appear out of order, when necessitated by proof dependencies. For example,  $B_1$  depends on  $C_4$ .

$$(C_2) : X_1 \cdot K_{1,2} \xleftarrow{(23)} \overline{K_{1,2} \cdot K_{1,2} \cdot X_1 \cdot K_{1,2}} \xleftarrow{(4)} K_{1,2} \cdot \overline{Z_1}$$

$$\begin{aligned} (C_3) : X_0 \cdot CX_{0,1} &\xleftarrow{(21)} X_0 \cdot CX_{0,1} \cdot \overline{X_0 \cdot X_0} \\ &\xleftarrow{(22)} \overline{CX_{0,1} \cdot CX_{0,1} \cdot X_0 \cdot CX_{0,1} \cdot X_0 \cdot X_0} \\ &\xleftarrow{(2)} CX_{0,1} \cdot \overline{X_1} \cdot X_0 \end{aligned}$$

$$\begin{aligned} (C_4) : K_{1,2} \cdot CX_{2,1} &\xleftarrow{(23)} \overline{K_{1,2} \cdot CX_{2,1} \cdot K_{1,2} \cdot K_{1,2}} \\ &\xleftarrow{(7)} \overline{CX_{1,2} \cdot K_{1,2}} \end{aligned}$$

$$(C_5) : X_0 \cdot CCX_{0,2}$$

$$\xleftarrow{(23)} X_0 \cdot \overline{CCX_{0,2} \cdot \overline{K_{1,2} \cdot K_{1,2}}}$$

$$\xleftarrow{C_1} X_0 \cdot \overline{K_{1,2} \cdot CCX_{0,1} \cdot K_{1,2}}$$

$$\xrightarrow{(27)} \overline{K_{1,2} \cdot X_0 \cdot CCX_{0,1} \cdot K_{1,2}}$$

$$\xrightarrow{(42)} \overline{K_{1,2} \cdot \overline{CCX_{0,1} \cdot CX_{1,2} \cdot X_0} \cdot K_{1,2}}$$

$$\xrightarrow{C_1} \overline{CCX_{0,2} \cdot K_{1,2} \cdot CX_{1,2} \cdot X_0 \cdot K_{1,2}}$$

$$\xrightarrow{(7)} CCX_{0,2} \cdot \overline{K_{1,2} \cdot \overline{K_{1,2} \cdot CX_{2,1} \cdot K_{1,2} \cdot X_0 \cdot K_{1,2}}}$$

$$\xrightarrow{(23)} CCX_{0,2} \cdot CX_{2,1} \cdot K_{1,2} \cdot \overline{X_0 \cdot K_{1,2}}$$

$$\xrightarrow{(27)} CCX_{0,2} \cdot CX_{2,1} \cdot \overline{K_{1,2} \cdot \overline{K_{1,2} \cdot X_0}}$$

$$\xrightarrow{(23)} CCX_{0,2} \cdot CX_{2,1} \cdot X_0$$

$$(B_1) : CX_{2,1} \cdot X_0$$

$$\xleftarrow{(23)} \overline{K_{1,2} \cdot \overline{K_{1,2} \cdot CX_{2,1} \cdot X_0}}$$

$$\xrightarrow{C_4} K_{1,2} \cdot \overline{CX_{1,2} \cdot \overline{K_{1,2} \cdot X_0}}$$

$$\xleftarrow{(27)} K_{1,2} \cdot \overline{CX_{1,2} \cdot X_0 \cdot K_{1,2}}$$

$$\xrightarrow{(26)} \overline{K_{1,2} \cdot X_0 \cdot CX_{1,2} \cdot K_{1,2}}$$

$$\xleftarrow{(27)} \overline{X_0 \cdot K_{1,2} \cdot CX_{1,2} \cdot K_{1,2}}$$

$$\xleftarrow{C_4} X_0 \cdot \overline{K_{1,2} \cdot \overline{K_{1,2} \cdot CX_{2,1}}}$$

$$\xrightarrow{(23)} X_0 \cdot CX_{2,1}$$

$$(E_1) : CX_{1,0} \cdot \overline{CX_{1,0}} \xrightarrow{(12)} \overline{CX_{1,0} \cdot \overline{K_{0,1} \cdot CX_{0,1} \cdot K_{0,1}}}$$

$$\xrightarrow{(12)} \overline{K_{0,1} \cdot CX_{0,1} \cdot \overline{K_{0,1} \cdot K_{0,1}} \cdot CX_{0,1} \cdot K_{0,1}}$$

$$\xrightarrow{(25)} K_{0,1} \cdot \overline{CX_{0,1} \cdot CX_{0,1} \cdot K_{0,1}}$$

$$\xrightarrow{(22)} \overline{K_{0,1} \cdot K_{0,1}}$$

$$\xrightarrow{(25)} \varepsilon$$

$$(E_2) : CZ_{0,1} \cdot \overline{CZ_{0,1}} \xrightarrow{(1)} \overline{CZ_{0,1} \cdot \overline{K_{1,2} \cdot CX_{0,1} \cdot K_{1,2}}}$$

$$\xrightarrow{(1)} \overline{K_{1,2} \cdot CX_{0,1} \cdot \overline{K_{1,2} \cdot K_{1,2}} \cdot CX_{0,1} \cdot K_{1,2}}$$

$$\xrightarrow{(23)} K_{1,2} \cdot \overline{CX_{0,1} \cdot CX_{0,1} \cdot K_{1,2}}$$

$$\xrightarrow{(22)} \overline{K_{1,2} \cdot K_{1,2}}$$

$$\xrightarrow{(23)} \varepsilon$$

$$(E_3) : Z_0 \cdot Z_0 \xleftarrow{(25)} \overline{K_{0,1} \cdot \overline{K_{0,1} \cdot Z_0 \cdot Z_0}}$$

$$\xrightarrow{(41)} K_{0,1} \cdot \overline{X_0 \cdot \overline{K_{0,1} \cdot Z_0}}$$

$$\xrightarrow{(41)} K_{0,1} \cdot \overline{X_0 \cdot \overline{K_{0,1} \cdot Z_0}}$$

$$\xrightarrow{(21)} \overline{K_{0,1} \cdot K_{0,1}}$$

$$\xrightarrow{(25)} \varepsilon$$

$$(E_4) : \sigma_{0,1} \cdot \overline{\sigma_{0,1}} \xrightarrow{(13)} \overline{\sigma_{0,1} \cdot \overline{CX_{0,1} \cdot CX_{1,0} \cdot CX_{0,1}}}$$

$$\xrightarrow{(13)} \overline{CX_{0,1} \cdot CX_{1,0} \cdot \overline{CX_{0,1} \cdot CX_{0,1}} \cdot CX_{1,0} \cdot CX_{0,1}}$$

$$\xrightarrow{(22)} CX_{0,1} \cdot \overline{CX_{1,0} \cdot CX_{1,0} \cdot CX_{0,1}}$$

$$\xrightarrow{E_1} \overline{CX_{0,1} \cdot CX_{0,1}}$$

$$\xrightarrow{(22)} \varepsilon$$

$$\begin{aligned}
(E_5) : Z_1 \cdot \underline{Z_1} &\xrightarrow{(34)} \underline{Z_1 \cdot \overline{\sigma_{0,1}} \cdot Z_0 \cdot \sigma_{0,1}} \\
&\xrightarrow{(34)} \overline{\sigma_{0,1} \cdot Z_0 \cdot \overline{\sigma_{0,1}} \cdot \sigma_{0,1}} \cdot Z_0 \cdot \sigma_{0,1} \\
&\xrightarrow{E_4} \sigma_{0,1} \cdot \underline{Z_0 \cdot Z_0} \cdot \sigma_{0,1} \\
&\xrightarrow{E_3} \underline{\sigma_{0,1} \cdot \sigma_{0,1}} \\
&\xrightarrow{E_4} \varepsilon
\end{aligned}$$

$$\begin{aligned}
(E_6^*) : K_{1,2} \cdot X_0 \cdot CCX_{0,2} \cdot X_0 \cdot \underline{CCX_{0,2}} \cdot K_{1,2} \\
&\xrightarrow{(14)} K_{1,2} \cdot X_0 \cdot \underline{CCX_{0,2}} \cdot X_0 \cdot \overline{\sigma_{0,1} \cdot \overline{CCX_{1,2}} \cdot \sigma_{0,1}} \cdot K_{1,2} \\
&\xrightarrow{(14)} K_{1,2} \cdot X_0 \cdot \sigma_{0,1} \cdot \overline{CCX_{1,2}} \cdot \underline{\sigma_{0,1} \cdot X_0 \cdot \sigma_{0,1}} \cdot CCX_{1,2} \cdot \sigma_{0,1} \cdot K_{1,2} \\
&\xleftarrow{(28)} K_{1,2} \cdot X_0 \cdot \sigma_{0,1} \cdot CCX_{1,2} \cdot \overline{X_1} \cdot CCX_{1,2} \cdot \sigma_{0,1} \cdot K_{1,2} \\
&\xleftarrow{E_4} K_{1,2} \cdot \overline{\sigma_{0,1} \cdot \overline{\sigma_{0,1}} \cdot X_0 \cdot \sigma_{0,1}} \cdot CCX_{1,2} \cdot X_1 \cdot CCX_{1,2} \cdot \sigma_{0,1} \cdot K_{1,2} \\
&\xleftarrow{(28)} K_{1,2} \cdot \sigma_{0,1} \cdot \overline{X_1} \cdot CCX_{1,2} \cdot X_1 \cdot \underline{CCX_{1,2}} \cdot \sigma_{0,1} \cdot K_{1,2} \\
&\xleftarrow{(5)} K_{1,2} \cdot \underline{\sigma_{0,1} \cdot \overline{CX_{2,0}} \cdot \sigma_{0,1}} \cdot K_{1,2} \\
&\xleftarrow{(31)} K_{1,2} \cdot \overline{CX_{2,1}} \cdot K_{1,2} \\
&\xleftarrow{(7)} \overline{CX_{1,2}}
\end{aligned}$$

$$\begin{aligned}
(E_7) : CCX_{0,2} \cdot \underline{CCX_{0,2}} \\
&\xrightarrow{(14)} \underline{CCX_{0,2} \cdot \sigma_{0,1} \cdot \overline{CCX_{1,2}} \cdot \sigma_{0,1}} \\
&\xrightarrow{(14)} \overline{\sigma_{0,1} \cdot \overline{CCX_{1,2}} \cdot \underline{\sigma_{0,1}} \cdot \sigma_{0,1}} \cdot CCX_{1,2} \cdot \sigma_{0,1} \\
&\xrightarrow{E_4} \sigma_{0,1} \cdot \underline{CCX_{1,2} \cdot \overline{CCX_{1,2}}} \cdot \sigma_{0,1} \\
&\xrightarrow{(24)} \underline{\sigma_{0,1} \cdot \sigma_{0,1}} \\
&\xrightarrow{E_4} \varepsilon
\end{aligned}$$

$$\begin{aligned}
(C_6) : CX_{0,1} \cdot CX_{1,0} \\
&\xleftarrow{E_1} \overline{CX_{1,0} \cdot CX_{1,0}} \cdot CX_{0,1} \cdot \underline{CX_{1,0}} \\
&\xrightarrow{(12)} CX_{1,0} \cdot \underline{CX_{1,0}} \cdot CX_{0,1} \cdot \overline{K_{0,1} \cdot CX_{0,1} \cdot K_{0,1}} \\
&\xrightarrow{(12)} CX_{1,0} \cdot \overline{K_{0,1} \cdot \overline{CX_{0,1}} \cdot K_{0,1}} \cdot \underline{CX_{0,1} \cdot K_{0,1}} \cdot CX_{0,1} \cdot K_{0,1} \\
&\xleftarrow{(12)} CX_{1,0} \cdot K_{0,1} \cdot \underline{CX_{0,1} \cdot \overline{CX_{1,0}} \cdot CX_{0,1}} \cdot K_{0,1} \\
&\xleftarrow{(13)} CX_{1,0} \cdot \underline{K_{0,1}} \cdot \overline{\sigma_{0,1}} \cdot K_{0,1} \\
&\xrightarrow{(35)} CX_{1,0} \cdot \overline{\sigma_{0,1} \cdot K_{0,1} \cdot \underline{\sigma_{0,1}} \cdot \sigma_{0,1}} \cdot K_{0,1} \\
&\xrightarrow{E_4} CX_{1,0} \cdot \sigma_{0,1} \cdot \underline{K_{0,1} \cdot K_{0,1}} \\
&\xrightarrow{(25)} CX_{1,0} \cdot \sigma_{0,1}
\end{aligned}$$

$$\begin{aligned}
(E_8) : CX_{1,2} \cdot \underline{CX_{1,2}} &\xleftarrow{E_6^*} \underline{CX_{1,2} \cdot \overline{K_{1,2} \cdot X_0 \cdot CCX_{0,2} \cdot X_0 \cdot \overline{CCX_{0,2}}} \cdot K_{1,2}} \\
&\xleftarrow{E_6^*} \overline{K_{1,2} \cdot X_0 \cdot \overline{CCX_{0,2}} \cdot X_0 \cdot \overline{CCX_{0,2}} \cdot K_{1,2}} \cdot K_{1,2} \cdot X_0 \cdot CCX_{0,2} \cdot X_0 \cdot \overline{CCX_{0,2}} \cdot K_{1,2} \\
&\xrightarrow{(23)} K_{1,2} \cdot X_0 \cdot CCX_{0,2} \cdot X_0 \cdot \overline{CCX_{0,2}} \cdot X_0 \cdot \underline{CCX_{0,2}} \cdot K_{1,2} \\
&\xrightarrow{C_5} K_{1,2} \cdot X_0 \cdot CCX_{0,2} \cdot X_0 \cdot \overline{CCX_{0,2} \cdot \overline{CCX_{0,2}} \cdot CX_{2,1} \cdot X_0} \cdot K_{1,2} \\
&\xrightarrow{E_7} K_{1,2} \cdot X_0 \cdot CCX_{0,2} \cdot X_0 \cdot \overline{CCX_{0,2}} \cdot X_0 \cdot \underline{CX_{2,1}} \cdot X_0 \cdot K_{1,2} \\
&\xleftarrow{B_1} K_{1,2} \cdot X_0 \cdot CCX_{0,2} \cdot X_0 \cdot \overline{CCX_{0,2} \cdot \overline{CX_{2,1}} \cdot X_0} \cdot X_0 \cdot K_{1,2} \\
&\xleftarrow{C_5} K_{1,2} \cdot X_0 \cdot CCX_{0,2} \cdot X_0 \cdot \overline{X_0 \cdot \overline{CCX_{0,2}}} \cdot X_0 \cdot K_{1,2} \\
&\xrightarrow{(21)} K_{1,2} \cdot X_0 \cdot \underline{CCX_{0,2} \cdot \overline{CCX_{0,2}}} \cdot X_0 \cdot K_{1,2} \\
&\xrightarrow{E_7} K_{1,2} \cdot \underline{X_0 \cdot X_0} \cdot K_{1,2} \\
&\xrightarrow{(21)} \underline{K_{1,2} \cdot K_{1,2}} \\
&\xrightarrow{(23)} \varepsilon
\end{aligned}$$

$$\begin{aligned}
(E_9) : CX_{2,1} \cdot CX_{2,1} &\xleftarrow{(23)} \overline{K_{1,2} \cdot \overline{K_{1,2} \cdot CX_{2,1}} \cdot CX_{2,1}} \\
&\xrightarrow{C_4} K_{1,2} \cdot \overline{CX_{1,2} \cdot \overline{K_{1,2} \cdot CX_{2,1}}} \\
&\xrightarrow{C_4} K_{1,2} \cdot \overline{CX_{1,2} \cdot \overline{CX_{1,2} \cdot K_{1,2}}} \\
&\xrightarrow{E_8} \overline{K_{1,2} \cdot K_{1,2}} \\
&\xrightarrow{(23)} \varepsilon
\end{aligned}$$

$$\begin{aligned}
(E_{10}) : \sigma_{1,2} \cdot \underline{\sigma_{1,2}} &\xrightarrow{(8)} \sigma_{1,2} \cdot \overline{CX_{1,2} \cdot CX_{2,1} \cdot CX_{1,2}} \\
&\xrightarrow{(8)} \overline{CX_{1,2} \cdot CX_{2,1} \cdot \overline{CX_{1,2} \cdot CX_{1,2}}} \cdot CX_{2,1} \cdot CX_{1,2} \\
&\xrightarrow{E_8} CX_{1,2} \cdot \overline{CX_{2,1} \cdot CX_{2,1}} \cdot CX_{1,2} \\
&\xrightarrow{E_9} \overline{CX_{1,2} \cdot CX_{1,2}} \\
&\xrightarrow{E_8} \varepsilon
\end{aligned}$$

$$\begin{aligned}
(E_{11}) : CZ_{0,2} \cdot \underline{CZ_{0,2}} &\xrightarrow{(18)} \underline{CZ_{0,2}} \cdot \overline{\sigma_{1,2} \cdot \overline{CZ_{0,1}} \cdot \sigma_{1,2}} \\
&\xrightarrow{(18)} \overline{\sigma_{1,2} \cdot \overline{CZ_{0,1}} \cdot \sigma_{1,2} \cdot \sigma_{1,2}} \cdot CZ_{0,1} \cdot \sigma_{1,2} \\
&\xrightarrow{E_{10}} \sigma_{1,2} \cdot \overline{CZ_{0,1} \cdot \overline{CZ_{0,1}}} \cdot \sigma_{1,2} \\
&\xrightarrow{E_2} \overline{\sigma_{1,2} \cdot \sigma_{1,2}} \\
&\xrightarrow{E_{10}} \varepsilon
\end{aligned}$$

$$\begin{aligned}
(E_{12}) : CZ_{1,2} \cdot \underline{CZ_{1,2}} &\xrightarrow{(19)} \underline{CZ_{1,2}} \cdot \overline{\sigma_{0,1} \cdot \overline{CZ_{0,2}} \cdot \sigma_{0,1}} \\
&\xrightarrow{(19)} \overline{\sigma_{0,1} \cdot \overline{CZ_{0,2}} \cdot \sigma_{0,1} \cdot \sigma_{0,1}} \cdot CZ_{0,2} \cdot \sigma_{0,1} \\
&\xrightarrow{E_4} \sigma_{0,1} \cdot \overline{CZ_{0,2} \cdot \overline{CZ_{0,2}}} \cdot \sigma_{0,1} \\
&\xrightarrow{E_{11}} \overline{\sigma_{0,1} \cdot \sigma_{0,1}} \\
&\xrightarrow{E_4} \varepsilon
\end{aligned}$$

$$\begin{aligned}
(S_1) : CX_{0,1} &\xleftarrow{E_1} CX_{0,1} \cdot \overline{CX_{1,0} \cdot CX_{1,0}} \\
&\xleftarrow{(22)} \overline{CX_{0,1} \cdot CX_{1,0} \cdot \overline{CX_{0,1}} \cdot CX_{0,1}} \cdot CX_{1,0} \\
&\xleftarrow{(13)} \overline{\sigma_{0,1} \cdot \overline{CX_{0,1}} \cdot CX_{1,0}} \\
&\xrightarrow{C_6} \sigma_{0,1} \cdot \overline{CX_{1,0} \cdot \sigma_{0,1}}
\end{aligned}$$

$$\begin{aligned}
(C_7) : X_1 \cdot \underline{CX_{0,1}} &\xrightarrow{S_1} \underline{X_1} \cdot \overline{\sigma_{0,1} \cdot \overline{CX_{1,0}} \cdot \sigma_{0,1}} \\
&\xrightarrow{(28)} \overline{\sigma_{0,1} \cdot \overline{X_0} \cdot \overline{\sigma_{0,1}} \cdot \sigma_{0,1}} \cdot CX_{1,0} \cdot \sigma_{0,1} \\
&\xrightarrow{E_4} \sigma_{0,1} \cdot \overline{X_0 \cdot \overline{CX_{1,0}}} \cdot \sigma_{0,1} \\
&\xrightarrow{(38)} \sigma_{0,1} \cdot \overline{CX_{1,0} \cdot \overline{X_0}} \cdot \sigma_{0,1} \\
&\xleftarrow{E_4} \sigma_{0,1} \cdot CX_{1,0} \cdot \overline{\sigma_{0,1} \cdot \overline{\sigma_{0,1}}} \cdot X_0 \cdot \sigma_{0,1} \\
&\xleftarrow{(28)} \overline{\sigma_{0,1} \cdot CX_{1,0} \cdot \sigma_{0,1} \cdot \overline{X_1}} \\
&\xleftarrow{S_1} \overline{CX_{0,1}} \cdot X_1
\end{aligned}$$

$$\begin{aligned}
(C_8) : X_1 \cdot CCX_{1,2} &\xleftarrow{E_4} \underline{X_1} \cdot \overline{CCX_{1,2} \cdot \sigma_{0,1} \cdot \sigma_{0,1}} \\
&\xrightarrow{(28)} \overline{\sigma_{0,1} \cdot \overline{X_0} \cdot \sigma_{0,1} \cdot \overline{CCX_{1,2} \cdot \sigma_{0,1} \cdot \sigma_{0,1}}} \\
&\xleftarrow{(14)} \sigma_{0,1} \cdot \overline{X_0 \cdot \overline{CCX_{0,2}}} \cdot \sigma_{0,1} \\
&\xrightarrow{C_5} \sigma_{0,1} \cdot \overline{CCX_{0,2} \cdot CX_{2,1} \cdot X_0} \cdot \sigma_{0,1} \\
&\xrightarrow{(14)} \overline{\sigma_{0,1} \cdot \overline{\sigma_{0,1}} \cdot \overline{CCX_{1,2} \cdot \sigma_{0,1} \cdot CX_{2,1} \cdot X_0 \cdot \sigma_{0,1}}} \\
&\xrightarrow{E_4} \overline{CCX_{1,2} \cdot \sigma_{0,1} \cdot \overline{CX_{2,1} \cdot X_0 \cdot \sigma_{0,1}}} \\
&\xrightarrow{(31)} \overline{CCX_{1,2} \cdot \sigma_{0,1} \cdot \overline{\sigma_{0,1} \cdot \overline{CX_{2,0} \cdot \sigma_{0,1} \cdot X_0 \cdot \sigma_{0,1}}} \\
&\xleftarrow{(28)} \overline{CCX_{1,2} \cdot \sigma_{0,1} \cdot \overline{\sigma_{0,1} \cdot CX_{2,0} \cdot \overline{X_1}}} \\
&\xrightarrow{E_4} \overline{CCX_{1,2} \cdot CX_{2,0} \cdot X_1}
\end{aligned}$$

$$\begin{aligned}
(B_2) : X_0 \cdot \underline{X_1} &\xrightarrow{(2)} \underline{X_0} \cdot \overline{CX_{0,1} \cdot X_0 \cdot CX_{0,1} \cdot X_0} \\
&\xrightarrow{C_3} \overline{CX_{0,1} \cdot X_1 \cdot \overline{X_0} \cdot X_0} \cdot CX_{0,1} \cdot X_0 \\
&\xrightarrow{(21)} \overline{CX_{0,1} \cdot X_1 \cdot CX_{0,1} \cdot X_0} \\
&\xrightarrow{C_7} \overline{CX_{0,1} \cdot \overline{CX_{0,1}} \cdot X_1 \cdot X_0} \\
&\xrightarrow{(22)} X_1 \cdot X_0
\end{aligned}$$

$$\begin{aligned}
(E_{13}) : & \underline{X_1 \cdot X_1} \\
& \xrightarrow{(2)} \underline{X_1 \cdot \overline{CX_{0,1} \cdot X_0 \cdot CX_{0,1} \cdot X_0}} \\
& \xrightarrow{(2)} \overline{CX_{0,1} \cdot X_0 \cdot CX_{0,1} \cdot X_0 \cdot CX_{0,1} \cdot \underline{X_0 \cdot CX_{0,1} \cdot X_0}} \\
& \xrightarrow{C_3} CX_{0,1} \cdot X_0 \cdot CX_{0,1} \cdot X_0 \cdot CX_{0,1} \cdot \overline{CX_{0,1} \cdot X_1 \cdot X_0 \cdot X_0} \\
& \xrightarrow{(21)} CX_{0,1} \cdot X_0 \cdot CX_{0,1} \cdot X_0 \cdot \underline{CX_{0,1} \cdot CX_{0,1} \cdot X_1} \\
& \xrightarrow{(22)} CX_{0,1} \cdot X_0 \cdot CX_{0,1} \cdot \underline{X_0 \cdot X_1} \\
& \xrightarrow{B_2} CX_{0,1} \cdot X_0 \cdot \underline{CX_{0,1} \cdot X_1 \cdot X_0} \\
& \xleftarrow{C_3} CX_{0,1} \cdot \underline{X_0 \cdot X_0 \cdot CX_{0,1}} \\
& \xrightarrow{(21)} \underline{CX_{0,1} \cdot CX_{0,1}} \\
& \xrightarrow{(22)} \varepsilon
\end{aligned}$$

$$\begin{aligned}
(E_{14}) : & \underline{CX_{2,0} \cdot CX_{2,0}} \\
& \xrightarrow{(5)} \overline{X_1 \cdot \overline{CCX_{1,2} \cdot X_1 \cdot \overline{CCX_{1,2}}} \cdot CX_{2,0}} \\
& \xleftarrow{E_{13}} X_1 \cdot \overline{CCX_{1,2} \cdot X_1 \cdot \underline{CCX_{1,2} \cdot CX_{2,0} \cdot X_1 \cdot X_1}} \\
& \xleftarrow{C_8} X_1 \cdot \overline{CCX_{1,2} \cdot X_1 \cdot X_1 \cdot \overline{CCX_{1,2}}} \cdot X_1 \\
& \xrightarrow{E_{13}} X_1 \cdot \underline{CCX_{1,2} \cdot \overline{CCX_{1,2}}} \cdot X_1 \\
& \xrightarrow{(24)} \underline{X_1 \cdot X_1} \\
& \xrightarrow{E_{13}} \varepsilon
\end{aligned}$$

$$\begin{aligned}
(E_{15}) : & CX_{0,2} \cdot \underline{CX_{0,2}} \xrightarrow{(9)} \underline{CX_{0,2} \cdot \overline{\sigma_{1,2} \cdot CX_{0,1} \cdot \sigma_{1,2}}} \\
& \xrightarrow{(9)} \overline{\sigma_{1,2} \cdot CX_{0,1} \cdot \underline{\sigma_{1,2} \cdot \sigma_{1,2}}} \cdot CX_{0,1} \cdot \sigma_{1,2} \\
& \xrightarrow{E_{10}} \sigma_{1,2} \cdot \underline{CX_{0,1} \cdot CX_{0,1}} \cdot \sigma_{1,2} \\
& \xrightarrow{(22)} \underline{\sigma_{1,2} \cdot \sigma_{1,2}} \\
& \xrightarrow{E_{10}} \varepsilon
\end{aligned}$$

$$\begin{aligned}
(E_{16}) : & \sigma_{0,2} \cdot \underline{\sigma_{0,2}} \xrightarrow{(10)} \underline{\sigma_{0,2} \cdot \overline{CX_{0,2} \cdot CX_{2,0} \cdot CX_{0,2}}} \\
& \xrightarrow{(10)} \overline{CX_{0,2} \cdot CX_{2,0} \cdot \underline{CX_{0,2} \cdot CX_{0,2}}} \cdot CX_{2,0} \cdot CX_{0,2} \\
& \xrightarrow{E_{15}} CX_{0,2} \cdot \underline{CX_{2,0} \cdot CX_{2,0}} \cdot CX_{0,2} \\
& \xrightarrow{E_{14}} \underline{CX_{0,2} \cdot CX_{0,2}} \\
& \xrightarrow{E_{15}} \varepsilon
\end{aligned}$$

$$\begin{aligned}
(E_{17}) : & X_2 \cdot \underline{X_2} \xrightarrow{(15)} \underline{X_2 \cdot \overline{\sigma_{0,2} \cdot X_0 \cdot \sigma_{0,2}}} \\
& \xrightarrow{(15)} \overline{\sigma_{0,2} \cdot X_0 \cdot \underline{\sigma_{0,2} \cdot \sigma_{0,2}}} \cdot X_0 \cdot \sigma_{0,2} \\
& \xrightarrow{E_{16}} \sigma_{0,2} \cdot \underline{X_0 \cdot X_0} \cdot \sigma_{0,2} \\
& \xrightarrow{(21)} \underline{\sigma_{0,2} \cdot \sigma_{0,2}} \\
& \xrightarrow{E_{16}} \varepsilon
\end{aligned}$$

$$\begin{aligned}
(E_{18}) : & \overline{CCX_{0,1} \cdot \underline{CCX_{0,1}}} \xrightarrow{(32)} \underline{\overline{CCX_{0,1} \cdot \overline{\sigma_{0,2} \cdot \overline{CCX_{1,2} \cdot \sigma_{0,2}}}}} \\
& \xrightarrow{(32)} \overline{\sigma_{0,2} \cdot \overline{CCX_{1,2} \cdot \underline{\sigma_{0,2} \cdot \sigma_{0,2}}} \cdot \overline{CCX_{1,2} \cdot \sigma_{0,2}}} \\
& \xrightarrow{E_{16}} \sigma_{0,2} \cdot \underline{CCX_{1,2} \cdot \overline{CCX_{1,2}}} \cdot \sigma_{0,2} \\
& \xrightarrow{(24)} \underline{\sigma_{0,2} \cdot \sigma_{0,2}} \\
& \xrightarrow{E_{16}} \varepsilon
\end{aligned}$$

$$\begin{aligned}
(E_{19}) : & Z_2 \cdot \underline{Z_2} \xrightarrow{(16)} \underline{Z_2 \cdot \overline{\sigma_{0,2} \cdot Z_0 \cdot \sigma_{0,2}}} \\
& \xrightarrow{(16)} \overline{\sigma_{0,2} \cdot Z_0 \cdot \underline{\sigma_{0,2} \cdot \sigma_{0,2}}} \cdot Z_0 \cdot \sigma_{0,2} \\
& \xrightarrow{E_{16}} \sigma_{0,2} \cdot \underline{Z_0 \cdot Z_0} \cdot \sigma_{0,2} \\
& \xrightarrow{E_3} \underline{\sigma_{0,2} \cdot \sigma_{0,2}} \\
& \xrightarrow{E_{16}} \varepsilon
\end{aligned}$$

$$\begin{aligned}
(S_2) : & CZ_{0,2} \xleftarrow{E_4} \overline{CZ_{0,2} \cdot \overline{\sigma_{0,1} \cdot \overline{\sigma_{0,1}}}} \\
& \xleftarrow{E_4} \overline{\sigma_{0,1} \cdot \overline{\sigma_{0,1} \cdot CZ_{0,2} \cdot \sigma_{0,1} \cdot \sigma_{0,1}}} \\
& \xleftarrow{(19)} \overline{\sigma_{0,1} \cdot \overline{CZ_{1,2}}} \cdot \sigma_{0,1}
\end{aligned}$$

$$\begin{aligned}
(S_3) : \sigma_{0,2} &\xrightarrow{(10)} \overline{CX_{0,2} \cdot CX_{2,0} \cdot CX_{0,2}} \\
&\xleftarrow{E_4} CX_{0,2} \cdot CX_{2,0} \cdot CX_{0,2} \cdot \overline{\sigma_{0,1} \cdot \sigma_{0,1}} \\
&\xleftarrow{E_4} CX_{0,2} \cdot CX_{2,0} \cdot \overline{\sigma_{0,1} \cdot \sigma_{0,1}} \cdot \overline{CX_{0,2} \cdot \sigma_{0,1} \cdot \sigma_{0,1}} \\
&\xleftarrow{(30)} CX_{0,2} \cdot CX_{2,0} \cdot \sigma_{0,1} \cdot \overline{CX_{1,2} \cdot \sigma_{0,1}} \\
&\xleftarrow{E_4} CX_{0,2} \cdot \overline{\sigma_{0,1} \cdot \sigma_{0,1}} \cdot \overline{CX_{2,0} \cdot \sigma_{0,1} \cdot CX_{1,2} \cdot \sigma_{0,1}} \\
&\xleftarrow{(31)} CX_{0,2} \cdot \sigma_{0,1} \cdot \overline{CX_{2,1} \cdot CX_{1,2} \cdot \sigma_{0,1}} \\
&\xleftarrow{E_4} \overline{\sigma_{0,1} \cdot \sigma_{0,1}} \cdot \overline{CX_{0,2} \cdot \sigma_{0,1} \cdot CX_{2,1} \cdot CX_{1,2} \cdot \sigma_{0,1}} \\
&\xleftarrow{(30)} \sigma_{0,1} \cdot \overline{CX_{1,2} \cdot CX_{2,1} \cdot CX_{1,2} \cdot \sigma_{0,1}} \\
&\xleftarrow{(8)} \sigma_{0,1} \cdot \overline{\sigma_{1,2} \cdot \sigma_{0,1}}
\end{aligned}$$

$$\begin{aligned}
(S_5) : CX_{2,1} &\xrightarrow{(31)} \overline{\sigma_{0,1} \cdot \overline{CX_{2,0} \cdot \sigma_{0,1}}} \\
&\xrightarrow{(29)} \sigma_{0,1} \cdot \overline{\sigma_{0,2} \cdot CX_{0,2} \cdot \sigma_{0,2}} \cdot \sigma_{0,1} \\
&\xrightarrow{S_3} \sigma_{0,1} \cdot \overline{\sigma_{0,2} \cdot CX_{0,2} \cdot \sigma_{0,1} \cdot \sigma_{1,2} \cdot \sigma_{0,1}} \cdot \sigma_{0,1} \\
&\xrightarrow{S_3} \sigma_{0,1} \cdot \overline{\sigma_{0,1} \cdot \sigma_{1,2} \cdot \sigma_{0,1} \cdot CX_{0,2} \cdot \sigma_{0,1} \cdot \sigma_{1,2} \cdot \sigma_{0,1} \cdot \sigma_{0,1}} \\
&\xrightarrow{E_4} \overline{\sigma_{0,1} \cdot \sigma_{0,1} \cdot \sigma_{1,2} \cdot \sigma_{0,1} \cdot CX_{0,2} \cdot \sigma_{0,1} \cdot \sigma_{1,2}} \\
&\xrightarrow{E_4} \sigma_{1,2} \cdot \overline{\sigma_{0,1} \cdot CX_{0,2} \cdot \sigma_{0,1} \cdot \sigma_{1,2}} \\
&\xleftarrow{(30)} \sigma_{1,2} \cdot \overline{CX_{1,2} \cdot \sigma_{1,2}}
\end{aligned}$$

$$\begin{aligned}
(S_7) : CX_{1,2} &\xrightarrow{(30)} \overline{\sigma_{0,1} \cdot \overline{CX_{0,2} \cdot \sigma_{0,1}}} \\
&\xrightarrow{(9)} \sigma_{0,1} \cdot \overline{\sigma_{1,2} \cdot \overline{CX_{0,1} \cdot \sigma_{1,2} \cdot \sigma_{0,1}}} \\
&\xrightarrow{S_1} \sigma_{0,1} \cdot \sigma_{1,2} \cdot \overline{\sigma_{0,1} \cdot \overline{CX_{1,0} \cdot \sigma_{0,1} \cdot \sigma_{1,2} \cdot \sigma_{0,1}}} \\
&\xleftarrow{S_3} \sigma_{0,1} \cdot \sigma_{1,2} \cdot \sigma_{0,1} \cdot \overline{CX_{1,0} \cdot \sigma_{0,2}} \\
&\xleftarrow{S_3} \overline{\sigma_{0,2} \cdot CX_{1,0} \cdot \sigma_{0,2}}
\end{aligned}$$

$$\begin{aligned}
(C_{10}) : CX_{2,1} \cdot K_{1,2} &\xleftarrow{E_8} CX_{2,1} \cdot K_{1,2} \cdot \overline{CX_{1,2} \cdot CX_{1,2}} \\
&\xleftarrow{(23)} CX_{2,1} \cdot K_{1,2} \cdot \overline{CX_{1,2} \cdot \overline{K_{1,2} \cdot K_{1,2}} \cdot CX_{1,2}} \\
&\xleftarrow{C_4} CX_{2,1} \cdot \overline{K_{1,2} \cdot \overline{CX_{2,1}} \cdot K_{1,2} \cdot CX_{1,2}} \\
&\xrightarrow{(23)} \overline{CX_{2,1} \cdot CX_{2,1} \cdot K_{1,2} \cdot CX_{1,2}} \\
&\xrightarrow{E_9} K_{1,2} \cdot CX_{1,2}
\end{aligned}$$

$$\begin{aligned}
(S_4) : Z_0 &\xleftarrow{E_{16}} Z_0 \cdot \overline{\sigma_{0,2} \cdot \sigma_{0,2}} \\
&\xleftarrow{E_{19}} Z_0 \cdot \sigma_{0,2} \cdot \overline{Z_2 \cdot Z_2 \cdot \sigma_{0,2}} \\
&\xleftarrow{E_{16}} Z_0 \cdot \sigma_{0,2} \cdot \overline{Z_2 \cdot \sigma_{0,2} \cdot \sigma_{0,2} \cdot Z_2 \cdot \sigma_{0,2}} \\
&\xrightarrow{(16)} Z_0 \cdot \overline{\sigma_{0,2} \cdot \sigma_{0,2}} \cdot \overline{Z_0 \cdot \sigma_{0,2} \cdot \sigma_{0,2} \cdot \sigma_{0,2} \cdot Z_2 \cdot \sigma_{0,2}} \\
&\xrightarrow{E_{16}} Z_0 \cdot Z_0 \cdot \sigma_{0,2} \cdot \sigma_{0,2} \cdot \sigma_{0,2} \cdot Z_2 \cdot \sigma_{0,2} \\
&\xrightarrow{E_3} \overline{\sigma_{0,2} \cdot \sigma_{0,2} \cdot \sigma_{0,2} \cdot Z_2 \cdot \sigma_{0,2}} \\
&\xrightarrow{E_{16}} \sigma_{0,2} \cdot Z_2 \cdot \sigma_{0,2}
\end{aligned}$$

$$\begin{aligned}
(S_6) : CX_{2,0} &\xrightarrow{(29)} \overline{\sigma_{0,2} \cdot CX_{0,2} \cdot \sigma_{0,2}} \\
&\xrightarrow{S_3} \overline{\sigma_{0,2} \cdot CX_{0,2} \cdot \sigma_{0,1} \cdot \sigma_{1,2} \cdot \sigma_{0,1}} \\
&\xrightarrow{S_3} \overline{\sigma_{0,1} \cdot \sigma_{1,2} \cdot \sigma_{0,1} \cdot CX_{0,2} \cdot \sigma_{0,1} \cdot \sigma_{1,2} \cdot \sigma_{0,1}} \\
&\xleftarrow{(30)} \sigma_{0,1} \cdot \overline{\sigma_{1,2} \cdot \overline{CX_{1,2} \cdot \sigma_{1,2} \cdot \sigma_{0,1}}} \\
&\xleftarrow{S_5} \sigma_{0,1} \cdot \overline{CX_{2,1} \cdot \sigma_{0,1}}
\end{aligned}$$

$$\begin{aligned}
(C_9) : CX_{1,2} \cdot CX_{2,1} &\xrightarrow{S_5} CX_{1,2} \cdot \overline{\sigma_{1,2} \cdot \overline{CX_{1,2} \cdot \sigma_{1,2}}} \\
&\xrightarrow{(8)} CX_{1,2} \cdot \sigma_{1,2} \cdot \overline{CX_{1,2} \cdot \overline{CX_{1,2} \cdot CX_{2,1} \cdot CX_{1,2}}} \\
&\xrightarrow{E_8} CX_{1,2} \cdot \overline{\sigma_{1,2} \cdot CX_{2,1} \cdot CX_{1,2}} \\
&\xrightarrow{(8)} \overline{CX_{1,2} \cdot \overline{CX_{1,2} \cdot CX_{2,1} \cdot CX_{1,2}} \cdot CX_{2,1} \cdot CX_{1,2}} \\
&\xrightarrow{E_8} CX_{2,1} \cdot \overline{CX_{1,2} \cdot CX_{2,1} \cdot CX_{1,2}} \\
&\xleftarrow{(8)} CX_{2,1} \cdot \overline{\sigma_{1,2}}
\end{aligned}$$

$$\begin{aligned}
(S_8) : CX_{1,2} &\xleftarrow{E_9} CX_{1,2} \cdot \overline{CX_{2,1} \cdot CX_{2,1}} \\
&\xleftarrow{E_8} \overline{CX_{1,2} \cdot CX_{2,1} \cdot \overline{CX_{1,2} \cdot CX_{1,2}} \cdot CX_{2,1}} \\
&\xleftarrow{(8)} \overline{\sigma_{1,2} \cdot CX_{1,2} \cdot CX_{2,1}} \\
&\xrightarrow{C_9} \sigma_{1,2} \cdot \overline{CX_{2,1} \cdot \sigma_{1,2}}
\end{aligned}$$

$$\begin{aligned}
(S_9) : CX_{2,1} &\xleftarrow{(23)} \overline{K_{1,2} \cdot \overline{K_{1,2}} \cdot CX_{2,1}} \\
&\xrightarrow{C_4} K_{1,2} \cdot \overline{CX_{1,2} \cdot \overline{K_{1,2}}} \\
&\xrightarrow{S_7} K_{1,2} \cdot \overline{\sigma_{0,2} \cdot CX_{1,0} \cdot \sigma_{0,2}} \cdot K_{1,2} \\
&\xleftarrow{E_{16}} K_{1,2} \cdot \sigma_{0,2} \cdot CX_{1,0} \cdot \overline{\sigma_{0,2} \cdot K_{1,2} \cdot \overline{\sigma_{0,2}} \cdot \sigma_{0,2}} \\
&\xleftarrow{(11)} K_{1,2} \cdot \sigma_{0,2} \cdot CX_{1,0} \cdot \overline{K_{0,1}} \cdot \sigma_{0,2} \\
&\xleftarrow{E_{16}} \overline{\sigma_{0,2} \cdot \overline{\sigma_{0,2}} \cdot K_{1,2} \cdot \sigma_{0,2}} \cdot CX_{1,0} \cdot K_{0,1} \cdot \sigma_{0,2} \\
&\xleftarrow{(11)} \sigma_{0,2} \cdot \overline{K_{0,1}} \cdot \overline{CX_{1,0}} \cdot K_{0,1} \cdot \sigma_{0,2} \\
&\xrightarrow{(12)} \sigma_{0,2} \cdot K_{0,1} \cdot \overline{K_{0,1} \cdot CX_{0,1} \cdot \overline{K_{0,1}} \cdot K_{0,1}} \cdot \sigma_{0,2} \\
&\xrightarrow{(25)} \sigma_{0,2} \cdot \overline{K_{0,1} \cdot K_{0,1}} \cdot CX_{0,1} \cdot \sigma_{0,2} \\
&\xrightarrow{(25)} \sigma_{0,2} \cdot CX_{0,1} \cdot \sigma_{0,2}
\end{aligned}$$

$$\begin{aligned}
(S_{10}) : K_{1,2} &\xleftarrow{E_{10}} K_{1,2} \cdot \overline{\sigma_{1,2} \cdot \sigma_{1,2}} \\
&\xrightarrow{(8)} K_{1,2} \cdot \overline{CX_{1,2} \cdot CX_{2,1} \cdot CX_{1,2}} \cdot \sigma_{1,2} \\
&\xleftarrow{C_{10}} \overline{CX_{2,1} \cdot \overline{K_{1,2}} \cdot CX_{2,1}} \cdot CX_{1,2} \cdot \sigma_{1,2} \\
&\xrightarrow{C_4} CX_{2,1} \cdot \overline{CX_{1,2} \cdot \overline{K_{1,2}} \cdot CX_{1,2}} \cdot \sigma_{1,2} \\
&\xleftarrow{C_{10}} CX_{2,1} \cdot \overline{CX_{1,2} \cdot CX_{2,1}} \cdot \overline{K_{1,2}} \cdot \sigma_{1,2} \\
&\xrightarrow{C_9} CX_{2,1} \cdot \overline{CX_{2,1}} \cdot \sigma_{1,2} \cdot K_{1,2} \cdot \sigma_{1,2} \\
&\xrightarrow{E_9} \sigma_{1,2} \cdot K_{1,2} \cdot \sigma_{1,2}
\end{aligned}$$

$$\begin{aligned}
(S_{11}) : CX_{1,0} &\xleftarrow{E_{16}} CX_{1,0} \cdot \overline{\sigma_{0,2} \cdot \sigma_{0,2}} \\
&\xleftarrow{E_{16}} \overline{\sigma_{0,2} \cdot \overline{\sigma_{0,2}} \cdot CX_{1,0} \cdot \sigma_{0,2}} \cdot \sigma_{0,2} \\
&\xleftarrow{S_7} \sigma_{0,2} \cdot \overline{CX_{1,2}} \cdot \sigma_{0,2}
\end{aligned}$$

$$\begin{aligned}
(S_{12}) : \sigma_{0,1} &\xleftarrow{E_1} \overline{CX_{1,0} \cdot \overline{CX_{1,0}} \cdot \sigma_{0,1}} \\
&\xleftarrow{C_6} CX_{1,0} \cdot \overline{CX_{0,1} \cdot \overline{CX_{1,0}}} \\
&\xrightarrow{S_{11}} CX_{1,0} \cdot CX_{0,1} \cdot \overline{\sigma_{0,2} \cdot CX_{1,2} \cdot \sigma_{0,2}} \\
&\xrightarrow{S_{11}} \overline{\sigma_{0,2} \cdot CX_{1,2} \cdot \overline{\sigma_{0,2}} \cdot CX_{0,1} \cdot \sigma_{0,2}} \cdot CX_{1,2} \cdot \sigma_{0,2} \\
&\xleftarrow{S_9} \sigma_{0,2} \cdot CX_{1,2} \cdot \overline{CX_{2,1}} \cdot CX_{1,2} \cdot \sigma_{0,2} \\
&\xleftarrow{(8)} \sigma_{0,2} \cdot \overline{\sigma_{1,2}} \cdot \sigma_{0,2}
\end{aligned}$$

$$\begin{aligned}
(S_{13}) : K_{1,2} \cdot CZ_{1,2} \cdot K_{1,2} \cdot CZ_{1,2} \cdot K_{1,2} \cdot CZ_{1,2} &\xleftarrow{E_{10}} \overline{\sigma_{1,2} \cdot \overline{\sigma_{1,2}}} \cdot K_{1,2} \cdot CZ_{1,2} \cdot K_{1,2} \cdot CZ_{1,2} \cdot K_{1,2} \cdot CZ_{1,2} \\
&\xrightarrow{(20)} \sigma_{1,2} \cdot \overline{CZ_{1,2} \cdot K_{1,2} \cdot CZ_{1,2} \cdot K_{1,2} \cdot CZ_{1,2} \cdot \overline{K_{1,2} \cdot K_{1,2}}} \cdot CZ_{1,2} \cdot K_{1,2} \cdot CZ_{1,2} \cdot K_{1,2} \cdot CZ_{1,2} \\
&\xrightarrow{(23)} \sigma_{1,2} \cdot CZ_{1,2} \cdot K_{1,2} \cdot CZ_{1,2} \cdot K_{1,2} \cdot \overline{CZ_{1,2} \cdot CZ_{1,2}} \cdot K_{1,2} \cdot CZ_{1,2} \cdot K_{1,2} \cdot CZ_{1,2} \\
&\xrightarrow{E_{12}} \sigma_{1,2} \cdot CZ_{1,2} \cdot K_{1,2} \cdot CZ_{1,2} \cdot \overline{K_{1,2} \cdot K_{1,2}} \cdot CZ_{1,2} \cdot K_{1,2} \cdot CZ_{1,2} \\
&\xrightarrow{(23)} \sigma_{1,2} \cdot CZ_{1,2} \cdot K_{1,2} \cdot \overline{CZ_{1,2} \cdot CZ_{1,2}} \cdot K_{1,2} \cdot CZ_{1,2} \\
&\xrightarrow{E_{12}} \sigma_{1,2} \cdot CZ_{1,2} \cdot \overline{K_{1,2} \cdot K_{1,2}} \cdot CZ_{1,2} \\
&\xrightarrow{(23)} \sigma_{1,2} \cdot \overline{CZ_{1,2} \cdot CZ_{1,2}} \\
&\xrightarrow{E_{12}} \sigma_{1,2}
\end{aligned}$$

$$\begin{aligned}
(S_{14}) : \underline{CX_{2,0}} &\xrightarrow{S_6} \overline{\sigma_{0,1} \cdot CX_{2,1} \cdot \sigma_{0,1}} \\
&\xrightarrow{S_5} \sigma_{0,1} \cdot \overline{\sigma_{1,2} \cdot CX_{1,2} \cdot \sigma_{1,2}} \cdot \sigma_{0,1} \\
&\xrightarrow{S_7} \sigma_{0,1} \cdot \sigma_{1,2} \cdot \overline{\sigma_{0,2} \cdot CX_{1,0} \cdot \sigma_{0,2}} \cdot \sigma_{1,2} \cdot \sigma_{0,1} \\
&\xleftarrow{E_{16}} \sigma_{0,1} \cdot \sigma_{1,2} \cdot \sigma_{0,2} \cdot CX_{1,0} \cdot \overline{\sigma_{0,2} \cdot \sigma_{1,2} \cdot \sigma_{0,2}} \cdot \sigma_{0,1} \\
&\xleftarrow{S_{12}} \sigma_{0,1} \cdot \sigma_{1,2} \cdot \sigma_{0,2} \cdot CX_{1,0} \cdot \overline{\sigma_{0,1}} \cdot \sigma_{0,2} \cdot \sigma_{0,1} \\
&\xleftarrow{E_{16}} \sigma_{0,1} \cdot \overline{\sigma_{0,2} \cdot \sigma_{0,2} \cdot \sigma_{1,2} \cdot \sigma_{0,2}} \cdot CX_{1,0} \cdot \sigma_{0,1} \cdot \sigma_{0,2} \cdot \sigma_{0,1} \\
&\xleftarrow{S_{12}} \sigma_{0,1} \cdot \sigma_{0,2} \cdot \overline{\sigma_{0,1}} \cdot CX_{1,0} \cdot \sigma_{0,1} \cdot \overline{\sigma_{0,2}} \cdot \sigma_{0,1} \\
&\xrightarrow{S_3} \sigma_{0,1} \cdot \sigma_{0,2} \cdot \sigma_{0,1} \cdot CX_{1,0} \cdot \sigma_{0,1} \cdot \overline{\sigma_{0,1} \cdot \sigma_{1,2} \cdot \sigma_{0,1}} \cdot \sigma_{0,1} \\
&\xrightarrow{E_4} \sigma_{0,1} \cdot \sigma_{0,2} \cdot \sigma_{0,1} \cdot CX_{1,0} \cdot \overline{\sigma_{0,1} \cdot \sigma_{0,1}} \cdot \sigma_{1,2} \\
&\xrightarrow{E_4} \sigma_{0,1} \cdot \overline{\sigma_{0,2}} \cdot \sigma_{0,1} \cdot CX_{1,0} \cdot \sigma_{1,2} \\
&\xrightarrow{S_3} \sigma_{0,1} \cdot \overline{\sigma_{0,1} \cdot \sigma_{1,2} \cdot \sigma_{0,1}} \cdot \sigma_{0,1} \cdot CX_{1,0} \cdot \sigma_{1,2} \\
&\xrightarrow{E_4} \overline{\sigma_{0,1} \cdot \sigma_{0,1}} \cdot \sigma_{1,2} \cdot CX_{1,0} \cdot \sigma_{1,2} \xrightarrow{E_4} \sigma_{1,2} \cdot CX_{1,0} \cdot \sigma_{1,2}
\end{aligned}$$

$$\begin{aligned}
(S_{15}) : \underline{\sigma_{0,2}} &\xrightarrow{(10)} \overline{CX_{0,2} \cdot CX_{2,0} \cdot CX_{0,2}} \\
&\xrightarrow{(9)} CX_{0,2} \cdot \overline{CX_{2,0}} \cdot \overline{\sigma_{1,2} \cdot CX_{0,1} \cdot \sigma_{1,2}} \\
&\xrightarrow{S_{14}} \overline{CX_{0,2}} \cdot \overline{\sigma_{1,2} \cdot CX_{1,0} \cdot \sigma_{1,2}} \cdot \sigma_{1,2} \cdot CX_{0,1} \cdot \sigma_{1,2} \\
&\xrightarrow{(9)} \overline{\sigma_{1,2} \cdot CX_{0,1} \cdot \sigma_{1,2}} \cdot \sigma_{1,2} \cdot CX_{1,0} \cdot \overline{\sigma_{1,2} \cdot \sigma_{1,2}} \cdot CX_{0,1} \cdot \sigma_{1,2} \\
&\xrightarrow{E_{10}} \sigma_{1,2} \cdot CX_{0,1} \cdot \overline{\sigma_{1,2} \cdot \sigma_{1,2}} \cdot CX_{1,0} \cdot CX_{0,1} \cdot \sigma_{1,2} \\
&\xrightarrow{E_{10}} \sigma_{1,2} \cdot \overline{CX_{0,1} \cdot CX_{1,0} \cdot CX_{0,1}} \cdot \sigma_{1,2} \\
&\xleftarrow{(13)} \sigma_{1,2} \cdot \overline{\sigma_{0,1}} \cdot \sigma_{1,2}
\end{aligned}$$

$$\begin{aligned}
(S_{16}) : \underline{\sigma_{0,1}} &\xrightarrow{(13)} \overline{CX_{0,1} \cdot CX_{1,0} \cdot CX_{0,1}} \\
&\xleftarrow{E_{10}} CX_{0,1} \cdot CX_{1,0} \cdot CX_{0,1} \cdot \overline{\sigma_{1,2} \cdot \sigma_{1,2}} \\
&\xleftarrow{E_{10}} CX_{0,1} \cdot CX_{1,0} \cdot \overline{\sigma_{1,2} \cdot \sigma_{1,2}} \cdot CX_{0,1} \cdot \sigma_{1,2} \cdot \sigma_{1,2} \\
&\xleftarrow{E_{10}} CX_{0,1} \cdot \overline{\sigma_{1,2} \cdot \sigma_{1,2}} \cdot CX_{1,0} \cdot \sigma_{1,2} \cdot \sigma_{1,2} \cdot CX_{0,1} \cdot \sigma_{1,2} \cdot \sigma_{1,2} \\
&\xleftarrow{E_{10}} \overline{\sigma_{1,2} \cdot \sigma_{1,2}} \cdot CX_{0,1} \cdot \sigma_{1,2} \cdot \sigma_{1,2} \cdot CX_{1,0} \cdot \sigma_{1,2} \cdot \overline{\sigma_{1,2} \cdot CX_{0,1} \cdot \sigma_{1,2}} \cdot \sigma_{1,2} \\
&\xleftarrow{(9)} \sigma_{1,2} \cdot \sigma_{1,2} \cdot CX_{0,1} \cdot \sigma_{1,2} \cdot \overline{\sigma_{1,2} \cdot CX_{1,0} \cdot \sigma_{1,2}} \cdot \overline{CX_{0,2}} \cdot \sigma_{1,2} \\
&\xleftarrow{S_{14}} \sigma_{1,2} \cdot \overline{\sigma_{1,2} \cdot CX_{0,1} \cdot \sigma_{1,2}} \cdot \overline{CX_{2,0}} \cdot CX_{0,2} \cdot \sigma_{1,2} \\
&\xleftarrow{(9)} \sigma_{1,2} \cdot \overline{CX_{0,2} \cdot CX_{2,0} \cdot CX_{0,2}} \cdot \sigma_{1,2} \xleftarrow{(10)} \sigma_{1,2} \cdot \overline{\sigma_{0,2}} \cdot \sigma_{1,2}
\end{aligned}$$

$$\begin{aligned}
(S_{17}) : \underline{CCX_{0,1}} &\xrightarrow{(33)} \overline{\sigma_{1,2} \cdot \overline{CCX_{0,2}} \cdot \sigma_{1,2}} \\
&\xrightarrow{(14)} \sigma_{1,2} \cdot \overline{\sigma_{0,1} \cdot \overline{CCX_{1,2}} \cdot \sigma_{0,1}} \cdot \sigma_{1,2} \\
&\xleftarrow{E_{16}} \sigma_{1,2} \cdot \sigma_{0,1} \cdot \overline{CCX_{1,2} \cdot \overline{\sigma_{0,2} \cdot \sigma_{0,2}}} \cdot \sigma_{0,1} \cdot \sigma_{1,2} \\
&\xleftarrow{E_{16}} \sigma_{1,2} \cdot \sigma_{0,1} \cdot \overline{\sigma_{0,2} \cdot \overline{\sigma_{0,2}} \cdot CCX_{1,2} \cdot \sigma_{0,2}} \cdot \sigma_{0,2} \cdot \sigma_{0,1} \cdot \sigma_{1,2} \\
&\xleftarrow{(32)} \sigma_{1,2} \cdot \sigma_{0,1} \cdot \sigma_{0,2} \cdot \overline{CCX_{0,1} \cdot \sigma_{0,2} \cdot \overline{\sigma_{0,1}}} \cdot \sigma_{1,2} \\
&\xrightarrow{S_{12}} \sigma_{1,2} \cdot \overline{\sigma_{0,1}} \cdot \sigma_{0,2} \cdot \overline{CCX_{0,1} \cdot \sigma_{0,2} \cdot \overline{\sigma_{0,2} \cdot \sigma_{1,2} \cdot \sigma_{0,2}}} \cdot \sigma_{1,2} \\
&\xrightarrow{S_{12}} \sigma_{1,2} \cdot \overline{\sigma_{0,2} \cdot \sigma_{1,2} \cdot \overline{\sigma_{0,2}} \cdot \sigma_{0,2}} \cdot \overline{CCX_{0,1} \cdot \overline{\sigma_{0,2} \cdot \sigma_{0,2}}} \cdot \sigma_{1,2} \cdot \sigma_{0,2} \cdot \sigma_{1,2} \\
&\xrightarrow{E_{16}} \sigma_{1,2} \cdot \sigma_{0,2} \cdot \sigma_{1,2} \cdot \overline{\sigma_{0,2} \cdot \sigma_{0,2}} \cdot \overline{CCX_{0,1} \cdot \sigma_{1,2} \cdot \sigma_{0,2}} \cdot \sigma_{1,2} \\
&\xrightarrow{E_{16}} \sigma_{1,2} \cdot \sigma_{0,2} \cdot \sigma_{1,2} \cdot \overline{CCX_{0,1} \cdot \sigma_{1,2} \cdot \sigma_{0,2} \cdot \sigma_{1,2}} \\
&\xleftarrow{S_{16}} \sigma_{1,2} \cdot \sigma_{0,2} \cdot \sigma_{1,2} \cdot \overline{CCX_{0,1} \cdot \overline{\sigma_{0,1}}} \\
&\xleftarrow{S_{16}} \overline{\sigma_{0,1}} \cdot \overline{CCX_{0,1} \cdot \sigma_{0,1}}
\end{aligned}$$

$$\begin{aligned}
(B_3) : CX_{0,2} \cdot \underline{X_1} &\xrightarrow{(28)} CX_{0,2} \cdot \overline{\sigma_{0,1} \cdot X_0 \cdot \sigma_{0,1}} \\
&\xleftarrow{E_4} \overline{\sigma_{0,1} \cdot \underline{\sigma_{0,1}} \cdot CX_{0,2} \cdot \sigma_{0,1} \cdot X_0 \cdot \sigma_{0,1}} \\
&\xleftarrow{(30)} \sigma_{0,1} \cdot \overline{CX_{1,2} \cdot X_0 \cdot \sigma_{0,1}} \\
&\xrightarrow{(26)} \sigma_{0,1} \cdot \overline{X_0 \cdot CX_{1,2}} \cdot \sigma_{0,1} \\
&\xrightarrow{(30)} \overline{\sigma_{0,1} \cdot X_0 \cdot \sigma_{0,1} \cdot CX_{0,2} \cdot \sigma_{0,1}} \cdot \sigma_{0,1} \\
&\xleftarrow{(28)} \overline{X_1 \cdot CX_{0,2} \cdot \sigma_{0,1} \cdot \sigma_{0,1}} \\
&\xrightarrow{E_4} X_1 \cdot CX_{0,2}
\end{aligned}$$

$$\begin{aligned}
(B_5) : X_1 \cdot \underline{\sigma_{0,2}} &\xrightarrow{(10)} X_1 \cdot \overline{CX_{0,2} \cdot CX_{2,0} \cdot CX_{0,2}} \\
&\xleftarrow{B_3} \overline{CX_{0,2} \cdot X_1 \cdot CX_{2,0} \cdot CX_{0,2}} \\
&\xleftarrow{B_4} CX_{0,2} \cdot \overline{CX_{2,0} \cdot X_1 \cdot CX_{0,2}} \\
&\xleftarrow{B_3} \overline{CX_{0,2} \cdot CX_{2,0} \cdot CX_{0,2} \cdot X_1} \\
&\xleftarrow{(10)} \overline{\sigma_{0,2}} \cdot X_1
\end{aligned}$$

$$\begin{aligned}
(C_{12}) : X_2 \cdot \underline{CX_{2,1}} &\xrightarrow{S_9} X_2 \cdot \overline{\sigma_{0,2} \cdot CX_{0,1} \cdot \sigma_{0,2}} \\
&\xrightarrow{(15)} \overline{\sigma_{0,2} \cdot X_0 \cdot \sigma_{0,2} \cdot \sigma_{0,2} \cdot CX_{0,1} \cdot \sigma_{0,2}} \\
&\xrightarrow{E_{16}} \sigma_{0,2} \cdot X_0 \cdot CX_{0,1} \cdot \sigma_{0,2} \\
&\xrightarrow{C_3} \sigma_{0,2} \cdot \overline{CX_{0,1} \cdot X_1 \cdot X_0 \cdot \sigma_{0,2}} \\
&\xleftarrow{E_{16}} \sigma_{0,2} \cdot CX_{0,1} \cdot X_1 \cdot \overline{\sigma_{0,2} \cdot \sigma_{0,2} \cdot X_0 \cdot \sigma_{0,2}} \\
&\xleftarrow{(15)} \sigma_{0,2} \cdot CX_{0,1} \cdot X_1 \cdot \overline{\sigma_{0,2} \cdot X_2} \\
&\xrightarrow{B_5} \overline{\sigma_{0,2} \cdot CX_{0,1} \cdot \sigma_{0,2} \cdot X_1 \cdot X_2} \\
&\xleftarrow{S_9} \overline{CX_{2,1}} \cdot X_1 \cdot X_2
\end{aligned}$$

$$\begin{aligned}
(C_{14}) : X_1 \cdot \underline{CX_{1,2}} &\xrightarrow{S_7} X_1 \cdot \overline{\sigma_{0,2} \cdot CX_{1,0} \cdot \sigma_{0,2}} \\
&\xrightarrow{B_5} \overline{\sigma_{0,2} \cdot X_1 \cdot CX_{1,0} \cdot \sigma_{0,2}} \\
&\xrightarrow{C_{13}} \sigma_{0,2} \cdot \overline{CX_{1,0} \cdot X_0 \cdot X_1 \cdot \sigma_{0,2}} \\
&\xrightarrow{B_5} \sigma_{0,2} \cdot CX_{1,0} \cdot X_0 \cdot \overline{\sigma_{0,2} \cdot X_1} \\
&\xleftarrow{E_{16}} \sigma_{0,2} \cdot CX_{1,0} \cdot \overline{\sigma_{0,2} \cdot \sigma_{0,2} \cdot X_0 \cdot \sigma_{0,2} \cdot X_1} \\
&\xleftarrow{(15)} \overline{\sigma_{0,2} \cdot CX_{1,0} \cdot \sigma_{0,2} \cdot X_2 \cdot X_1} \xleftarrow{S_7} \overline{CX_{1,2}} \cdot X_2 \cdot X_1
\end{aligned}$$

$$\begin{aligned}
(B_4) : CX_{2,0} \cdot \underline{X_1} &\xrightarrow{(28)} CX_{2,0} \cdot \overline{\sigma_{0,1} \cdot X_0 \cdot \sigma_{0,1}} \\
&\xrightarrow{S_6} \overline{\sigma_{0,1} \cdot CX_{2,1} \cdot \sigma_{0,1} \cdot \sigma_{0,1} \cdot X_0 \cdot \sigma_{0,1}} \\
&\xrightarrow{E_4} \sigma_{0,1} \cdot CX_{2,1} \cdot X_0 \cdot \sigma_{0,1} \\
&\xrightarrow{B_1} \sigma_{0,1} \cdot \overline{X_0 \cdot CX_{2,1}} \cdot \sigma_{0,1} \\
&\xleftarrow{E_4} \sigma_{0,1} \cdot X_0 \cdot \overline{\sigma_{0,1} \cdot \sigma_{0,1} \cdot CX_{2,1} \cdot \sigma_{0,1}} \\
&\xleftarrow{S_6} \overline{\sigma_{0,1} \cdot X_0 \cdot \sigma_{0,1} \cdot CX_{2,0}} \\
&\xleftarrow{(28)} \overline{X_1 \cdot CX_{2,0}}
\end{aligned}$$

$$\begin{aligned}
(C_{11}) : X_2 \cdot \underline{CX_{1,2}} &\xrightarrow{S_7} X_2 \cdot \overline{\sigma_{0,2} \cdot CX_{1,0} \cdot \sigma_{0,2}} \\
&\xrightarrow{(15)} \overline{\sigma_{0,2} \cdot X_0 \cdot \sigma_{0,2} \cdot \sigma_{0,2} \cdot CX_{1,0} \cdot \sigma_{0,2}} \\
&\xrightarrow{E_{16}} \sigma_{0,2} \cdot X_0 \cdot CX_{1,0} \cdot \sigma_{0,2} \\
&\xrightarrow{(38)} \sigma_{0,2} \cdot \overline{CX_{1,0} \cdot X_0 \cdot \sigma_{0,2}} \\
&\xleftarrow{E_{16}} \sigma_{0,2} \cdot CX_{1,0} \cdot \overline{\sigma_{0,2} \cdot \sigma_{0,2} \cdot X_0 \cdot \sigma_{0,2}} \\
&\xleftarrow{(15)} \overline{\sigma_{0,2} \cdot CX_{1,0} \cdot \sigma_{0,2} \cdot X_2} \\
&\xleftarrow{S_7} \overline{CX_{1,2}} \cdot X_2
\end{aligned}$$

$$\begin{aligned}
(C_{13}) : \underline{X_1} \cdot CX_{1,0} &\xrightarrow{(28)} \overline{\sigma_{0,1} \cdot X_0 \cdot \sigma_{0,1} \cdot CX_{1,0}} \\
&\xleftarrow{E_4} \overline{\sigma_{0,1} \cdot X_0 \cdot \sigma_{0,1} \cdot CX_{1,0} \cdot \overline{\sigma_{0,1} \cdot \sigma_{0,1}}} \\
&\xleftarrow{S_1} \sigma_{0,1} \cdot X_0 \cdot \overline{CX_{0,1}} \cdot \sigma_{0,1} \\
&\xrightarrow{C_3} \sigma_{0,1} \cdot \overline{CX_{0,1} \cdot X_1 \cdot X_0 \cdot \sigma_{0,1}} \\
&\xrightarrow{(28)} \sigma_{0,1} \cdot CX_{0,1} \cdot \overline{\sigma_{0,1} \cdot X_0 \cdot \sigma_{0,1} \cdot X_0 \cdot \sigma_{0,1}} \\
&\xleftarrow{(28)} \sigma_{0,1} \cdot \overline{CX_{0,1} \cdot \sigma_{0,1} \cdot X_0 \cdot X_1} \\
&\xrightarrow{S_1} \sigma_{0,1} \cdot \overline{\sigma_{0,1} \cdot CX_{1,0} \cdot \sigma_{0,1} \cdot \sigma_{0,1} \cdot X_0 \cdot X_1} \\
&\xrightarrow{E_4} \overline{\sigma_{0,1} \cdot \sigma_{0,1} \cdot CX_{1,0} \cdot X_0 \cdot X_1} \\
&\xrightarrow{E_4} CX_{1,0} \cdot X_0 \cdot X_1
\end{aligned}$$

$$\begin{aligned}
(C_{15}) : CX_{1,2} \cdot X_1 &\xleftarrow{E_8} CX_{1,2} \cdot X_1 \cdot \overline{CX_{1,2} \cdot CX_{1,2}} \\
&\xleftarrow{E_{17}} CX_{1,2} \cdot X_1 \cdot CX_{1,2} \cdot \overline{X_2 \cdot X_2} \cdot CX_{1,2} \\
&\xleftarrow{E_{13}} CX_{1,2} \cdot X_1 \cdot \overline{CX_{1,2} \cdot X_2 \cdot X_1 \cdot X_1 \cdot X_2 \cdot CX_{1,2}} \\
&\xleftarrow{C_{14}} CX_{1,2} \cdot X_1 \cdot \overline{X_1 \cdot CX_{1,2}} \cdot X_1 \cdot X_2 \cdot CX_{1,2} \\
&\xrightarrow{E_{13}} CX_{1,2} \cdot CX_{1,2} \cdot X_1 \cdot X_2 \cdot CX_{1,2} \\
&\xrightarrow{E_8} X_1 \cdot X_2 \cdot CX_{1,2}
\end{aligned}$$

$$\begin{aligned}
(S_{18}) : X_2 &\xleftarrow{E_{10}} X_2 \cdot \overline{\sigma_{1,2} \cdot \sigma_{1,2}} \\
&\xrightarrow{(8)} X_2 \cdot \overline{CX_{1,2} \cdot CX_{2,1} \cdot CX_{1,2}} \cdot \sigma_{1,2} \\
&\xrightarrow{C_{11}} \overline{CX_{1,2} \cdot X_2 \cdot CX_{2,1}} \cdot CX_{1,2} \cdot \sigma_{1,2} \\
&\xrightarrow{C_{12}} CX_{1,2} \cdot \overline{CX_{2,1} \cdot X_1 \cdot X_2 \cdot CX_{1,2}} \cdot \sigma_{1,2} \\
&\xleftarrow{C_{15}} CX_{1,2} \cdot CX_{2,1} \cdot \overline{CX_{1,2}} \cdot X_1 \cdot \sigma_{1,2} \\
&\xleftarrow{(8)} \overline{\sigma_{1,2}} \cdot X_1 \cdot \sigma_{1,2}
\end{aligned}$$

$$\begin{aligned}
(S_{19}) : CCX_{0,2} &\xleftarrow{E_{10}} CCX_{0,2} \cdot \overline{\sigma_{1,2} \cdot \sigma_{1,2}} \\
&\xleftarrow{E_{10}} \overline{\sigma_{1,2} \cdot \sigma_{1,2}} \cdot CCX_{0,2} \cdot \sigma_{1,2} \cdot \sigma_{1,2} \\
&\xleftarrow{(33)} \sigma_{1,2} \cdot \overline{CCX_{0,1}} \cdot \sigma_{1,2} \\
&\xrightarrow{S_{17}} \sigma_{1,2} \cdot \overline{\sigma_{0,1} \cdot \overline{CCX_{0,1}} \cdot \sigma_{0,1}} \cdot \sigma_{1,2} \\
&\xrightarrow{(33)} \sigma_{1,2} \cdot \sigma_{0,1} \cdot \overline{\sigma_{1,2} \cdot \overline{CCX_{0,2}} \cdot \sigma_{1,2}} \cdot \sigma_{0,1} \cdot \sigma_{1,2} \\
&\xleftarrow{S_{15}} \sigma_{1,2} \cdot \sigma_{0,1} \cdot \sigma_{1,2} \cdot CCX_{0,2} \cdot \overline{\sigma_{0,2}} \\
&\xleftarrow{S_{15}} \overline{\sigma_{0,2}} \cdot CCX_{0,2} \cdot \sigma_{0,2}
\end{aligned}$$

$$\begin{aligned}
(S_{20}) : CCX_{1,2} &\xleftarrow{E_4} CCX_{1,2} \cdot \overline{\sigma_{0,1} \cdot \sigma_{0,1}} \\
&\xleftarrow{E_4} \overline{\sigma_{0,1} \cdot \sigma_{0,1}} \cdot CCX_{1,2} \cdot \sigma_{0,1} \cdot \sigma_{0,1} \\
&\xleftarrow{(14)} \sigma_{0,1} \cdot \overline{CCX_{0,2}} \cdot \sigma_{0,1} \\
&\xrightarrow{S_{19}} \sigma_{0,1} \cdot \overline{\sigma_{0,2} \cdot \overline{CCX_{0,2}} \cdot \sigma_{0,2}} \cdot \sigma_{0,1} \\
&\xrightarrow{S_3} \sigma_{0,1} \cdot \overline{\sigma_{0,2} \cdot CCX_{0,2} \cdot \sigma_{0,1} \cdot \sigma_{1,2} \cdot \sigma_{0,1}} \cdot \sigma_{0,1} \\
&\xrightarrow{S_3} \sigma_{0,1} \cdot \overline{\sigma_{0,1} \cdot \sigma_{1,2} \cdot \sigma_{0,1}} \cdot CCX_{0,2} \cdot \sigma_{0,1} \cdot \sigma_{1,2} \cdot \overline{\sigma_{0,1} \cdot \sigma_{0,1}} \\
&\xrightarrow{E_4} \overline{\sigma_{0,1} \cdot \sigma_{0,1}} \cdot \sigma_{1,2} \cdot \sigma_{0,1} \cdot CCX_{0,2} \cdot \sigma_{0,1} \cdot \sigma_{1,2} \\
&\xrightarrow{E_4} \sigma_{1,2} \cdot \sigma_{0,1} \cdot \overline{CCX_{0,2}} \cdot \sigma_{0,1} \cdot \sigma_{1,2} \\
&\xrightarrow{(14)} \sigma_{1,2} \cdot \sigma_{0,1} \cdot \overline{\sigma_{0,1} \cdot \overline{CCX_{1,2}} \cdot \sigma_{0,1} \cdot \sigma_{1,2}} \\
&\xrightarrow{E_4} \sigma_{1,2} \cdot \overline{\sigma_{0,1} \cdot \sigma_{0,1}} \cdot CCX_{1,2} \cdot \sigma_{1,2} \\
&\xrightarrow{E_4} \sigma_{1,2} \cdot CCX_{1,2} \cdot \sigma_{1,2}
\end{aligned}$$

$$\begin{aligned}
(C_{16}) : X_2 \cdot K_{1,2} &\xrightarrow{(15)} \overline{\sigma_{0,2} \cdot X_0 \cdot \sigma_{0,2}} \cdot K_{1,2} \\
&\xleftarrow{E_{16}} \sigma_{0,2} \cdot X_0 \cdot \overline{\sigma_{0,2} \cdot K_{1,2} \cdot \sigma_{0,2}} \cdot \overline{\sigma_{0,2}} \\
&\xleftarrow{(11)} \sigma_{0,2} \cdot X_0 \cdot \overline{K_{0,1}} \cdot \sigma_{0,2} \\
&\xleftarrow{(41)} \sigma_{0,2} \cdot \overline{K_{0,1}} \cdot Z_0 \cdot \sigma_{0,2} \\
&\xrightarrow{(11)} \overline{\sigma_{0,2} \cdot \sigma_{0,2} \cdot K_{1,2} \cdot \sigma_{0,2} \cdot Z_0 \cdot \sigma_{0,2}} \\
&\xrightarrow{E_{16}} K_{1,2} \cdot \overline{\sigma_{0,2} \cdot Z_0 \cdot \sigma_{0,2}} \\
&\xleftarrow{(16)} K_{1,2} \cdot \overline{Z_2}
\end{aligned}$$

$$(S_{21}) : CZ_{1,2} \xleftarrow{E_{10}} \overline{\sigma_{1,2} \cdot \sigma_{1,2}} \cdot CZ_{1,2} \xrightarrow{(20)} \sigma_{1,2} \cdot \overline{CZ_{1,2} \cdot \overline{K_{1,2}} \cdot CZ_{1,2} \cdot K_{1,2} \cdot CZ_{1,2} \cdot K_{1,2} \cdot CZ_{1,2}} \xrightarrow{S_{13}} \sigma_{1,2} \cdot CZ_{1,2} \cdot \overline{\sigma_{1,2}}$$

$$\begin{aligned}
(S_{22}) : Z_2 &\xleftarrow{(23)} \overline{K_{1,2} \cdot K_{1,2} \cdot Z_2} \\
&\xleftarrow{C_{16}} K_{1,2} \cdot \overline{X_2 \cdot K_{1,2}} \\
&\xrightarrow{S_{18}} K_{1,2} \cdot \overline{\sigma_{1,2} \cdot X_1 \cdot \sigma_{1,2}} \cdot K_{1,2} \\
&\xrightarrow{S_{10}} K_{1,2} \cdot \sigma_{1,2} \cdot X_1 \cdot \overline{\sigma_{1,2} \cdot K_{1,2} \cdot \sigma_{1,2}} \\
&\xrightarrow{E_{10}} K_{1,2} \cdot \sigma_{1,2} \cdot X_1 \cdot K_{1,2} \cdot \sigma_{1,2} \\
&\xrightarrow{S_{10}} \overline{\sigma_{1,2} \cdot K_{1,2} \cdot \sigma_{1,2} \cdot X_1 \cdot K_{1,2} \cdot \sigma_{1,2}} \\
&\xrightarrow{E_{10}} \sigma_{1,2} \cdot K_{1,2} \cdot \overline{X_1 \cdot K_{1,2}} \cdot \sigma_{1,2} \\
&\xrightarrow{C_2} \sigma_{1,2} \cdot K_{1,2} \cdot \overline{K_{1,2} \cdot Z_1} \cdot \sigma_{1,2} \\
&\xrightarrow{(23)} \sigma_{1,2} \cdot Z_1 \cdot \sigma_{1,2}
\end{aligned}$$

$$\begin{aligned}
(S_{23}) : CZ_{0,2} &\xleftarrow{E_4} CZ_{0,2} \cdot \overline{\sigma_{0,1} \cdot \sigma_{0,1}} \\
&\xleftarrow{E_4} \overline{\sigma_{0,1} \cdot \sigma_{0,1}} \cdot CZ_{0,2} \cdot \sigma_{0,1} \cdot \sigma_{0,1} \\
&\xleftarrow{(19)} \sigma_{0,1} \cdot \overline{CZ_{1,2}} \cdot \sigma_{0,1} \\
&\xrightarrow{S_{21}} \sigma_{0,1} \cdot \overline{\sigma_{1,2} \cdot \overline{CZ_{1,2}} \cdot \sigma_{1,2}} \cdot \sigma_{0,1} \\
&\xrightarrow{(19)} \sigma_{0,1} \cdot \sigma_{1,2} \cdot \overline{\sigma_{0,1} \cdot CZ_{0,2} \cdot \sigma_{0,1} \cdot \sigma_{1,2} \cdot \sigma_{0,1}} \\
&\xleftarrow{S_3} \overline{\sigma_{0,1} \cdot \sigma_{1,2} \cdot \sigma_{0,1} \cdot CZ_{0,2} \cdot \sigma_{0,2}} \\
&\xleftarrow{S_3} \overline{\sigma_{0,2} \cdot CZ_{0,2} \cdot \sigma_{0,2}}
\end{aligned}$$

$$\begin{aligned}
(S_{24}) : CZ_{0,1} &\xleftarrow{E_{10}} CZ_{0,1} \cdot \overline{\sigma_{1,2} \cdot \sigma_{1,2}} \\
&\xleftarrow{E_{10}} \overline{\sigma_{1,2} \cdot \sigma_{1,2}} \cdot CZ_{0,1} \cdot \sigma_{1,2} \cdot \sigma_{1,2} \\
&\xleftarrow{(18)} \sigma_{1,2} \cdot \overline{CZ_{0,2}} \cdot \sigma_{1,2} \\
&\xrightarrow{S_{23}} \sigma_{1,2} \cdot \sigma_{0,2} \cdot \overline{CZ_{0,2}} \cdot \sigma_{0,2} \cdot \sigma_{1,2} \\
&\xrightarrow{(18)} \sigma_{1,2} \cdot \sigma_{0,2} \cdot \overline{\sigma_{1,2} \cdot CZ_{0,1} \cdot \sigma_{1,2} \cdot \sigma_{0,2} \cdot \sigma_{1,2}} \\
&\xleftarrow{S_{16}} \overline{\sigma_{1,2} \cdot \sigma_{0,2} \cdot \sigma_{1,2} \cdot CZ_{0,1} \cdot \sigma_{0,1}} \\
&\xleftarrow{S_{16}} \overline{\sigma_{0,1} \cdot CZ_{0,1} \cdot \sigma_{0,1}}
\end{aligned}
\qquad
\begin{aligned}
(B_6) : Z_0 \cdot K_{1,2} &\xleftarrow{(25)} \overline{K_{0,1} \cdot K_{0,1}} \cdot Z_0 \cdot K_{1,2} \\
&\xrightarrow{(41)} K_{0,1} \cdot \overline{X_0 \cdot K_{0,1}} \cdot K_{1,2} \\
&\xrightarrow{(39)} K_{0,1} \cdot \overline{X_0 \cdot K_{1,2}} \cdot K_{0,1} \\
&\xrightarrow{(27)} K_{0,1} \cdot \overline{K_{1,2}} \cdot X_0 \cdot K_{0,1} \\
&\xrightarrow{(39)} \overline{K_{1,2} \cdot K_{0,1}} \cdot X_0 \cdot K_{0,1} \\
&\xleftarrow{(41)} K_{1,2} \cdot \overline{K_{0,1} \cdot K_{0,1}} \cdot Z_0 \xrightarrow{(25)} K_{1,2} \cdot Z_0
\end{aligned}$$

$$\begin{aligned}
(C_{17}) : CX_{0,1} \cdot CX_{1,2} &\xleftarrow{E_8} \overline{CX_{1,2} \cdot CX_{1,2}} \cdot CX_{0,1} \cdot CX_{1,2} \xleftarrow{(22)} CX_{1,2} \cdot \overline{CX_{0,1} \cdot CX_{0,1}} \cdot CX_{1,2} \cdot CX_{0,1} \cdot \overline{CX_{1,2}} \\
&\xrightarrow{S_8} CX_{1,2} \cdot CX_{0,1} \cdot CX_{0,1} \cdot \overline{CX_{1,2} \cdot CX_{0,1} \cdot \sigma_{1,2} \cdot \overline{CX_{2,1}} \cdot \sigma_{1,2}} \\
&\xrightarrow{S_8} CX_{1,2} \cdot CX_{0,1} \cdot CX_{0,1} \cdot \overline{\sigma_{1,2} \cdot CX_{2,1} \cdot \sigma_{1,2} \cdot CX_{0,1} \cdot \sigma_{1,2} \cdot CX_{2,1} \cdot \sigma_{1,2}} \\
&\xleftarrow{(9)} CX_{1,2} \cdot CX_{0,1} \cdot CX_{0,1} \cdot \sigma_{1,2} \cdot CX_{2,1} \cdot \overline{CX_{0,2}} \cdot CX_{2,1} \cdot \sigma_{1,2} \\
&\xleftarrow{E_{10}} CX_{1,2} \cdot CX_{0,1} \cdot \overline{\sigma_{1,2} \cdot \sigma_{1,2}} \cdot CX_{0,1} \cdot \sigma_{1,2} \cdot CX_{2,1} \cdot CX_{0,2} \cdot CX_{2,1} \cdot \sigma_{1,2} \\
&\xleftarrow{(9)} CX_{1,2} \cdot CX_{0,1} \cdot \sigma_{1,2} \cdot \overline{CX_{0,2}} \cdot CX_{2,1} \cdot CX_{0,2} \cdot \overline{CX_{2,1}} \cdot \sigma_{1,2} \\
&\xrightarrow{S_9} CX_{1,2} \cdot CX_{0,1} \cdot \sigma_{1,2} \cdot CX_{0,2} \cdot \overline{CX_{2,1} \cdot CX_{0,2} \cdot \sigma_{0,2} \cdot \overline{CX_{0,1}} \cdot \sigma_{0,2}} \cdot \sigma_{1,2} \\
&\xrightarrow{S_9} CX_{1,2} \cdot CX_{0,1} \cdot \sigma_{1,2} \cdot CX_{0,2} \cdot \overline{\sigma_{0,2} \cdot \overline{CX_{0,1}} \cdot \sigma_{0,2} \cdot CX_{0,2} \cdot \sigma_{0,2}} \cdot CX_{0,1} \cdot \sigma_{0,2} \cdot \sigma_{1,2} \\
&\xleftarrow{(29)} CX_{1,2} \cdot CX_{0,1} \cdot \sigma_{1,2} \cdot CX_{0,2} \cdot \sigma_{0,2} \cdot CX_{0,1} \cdot \overline{CX_{2,0}} \cdot CX_{0,1} \cdot \sigma_{0,2} \cdot \sigma_{1,2} \\
&\xleftarrow{E_{16}} CX_{1,2} \cdot CX_{0,1} \cdot \sigma_{1,2} \cdot \overline{\sigma_{0,2} \cdot \sigma_{0,2}} \cdot CX_{0,2} \cdot \sigma_{0,2} \cdot CX_{0,1} \cdot CX_{2,0} \cdot CX_{0,1} \cdot \sigma_{0,2} \cdot \sigma_{1,2} \\
&\xleftarrow{(29)} CX_{1,2} \cdot CX_{0,1} \cdot \sigma_{1,2} \cdot \sigma_{0,2} \cdot \overline{CX_{2,0}} \cdot CX_{0,1} \cdot CX_{2,0} \cdot \overline{CX_{0,1}} \cdot \sigma_{0,2} \cdot \sigma_{1,2} \\
&\xleftarrow{(6)} CX_{1,2} \cdot CX_{0,1} \cdot \sigma_{1,2} \cdot \sigma_{0,2} \cdot \overline{CX_{2,1}} \cdot \sigma_{0,2} \cdot \sigma_{1,2} \\
&\xrightarrow{S_9} CX_{1,2} \cdot CX_{0,1} \cdot \sigma_{1,2} \cdot \sigma_{0,2} \cdot \overline{\sigma_{0,2} \cdot \overline{CX_{0,1}} \cdot \sigma_{0,2} \cdot \sigma_{0,2}} \cdot \sigma_{1,2} \\
&\xrightarrow{E_{16}} CX_{1,2} \cdot CX_{0,1} \cdot \sigma_{1,2} \cdot \overline{\sigma_{0,2} \cdot \sigma_{0,2}} \cdot CX_{0,1} \cdot \sigma_{1,2} \\
&\xrightarrow{E_{16}} CX_{1,2} \cdot CX_{0,1} \cdot \overline{\sigma_{1,2} \cdot CX_{0,1} \cdot \sigma_{1,2}} \xleftarrow{(9)} CX_{1,2} \cdot CX_{0,1} \cdot \overline{CX_{0,2}}
\end{aligned}$$

$$\begin{aligned}
(S_{25}) : CZ_{1,2} &\xrightarrow{(19)} \overline{\sigma_{0,1} \cdot CZ_{0,2} \cdot \sigma_{0,1}} \\
&\xrightarrow{(18)} \sigma_{0,1} \cdot \overline{\sigma_{1,2} \cdot CZ_{0,1} \cdot \sigma_{1,2}} \cdot \sigma_{0,1} \\
&\xrightarrow{S_{24}} \sigma_{0,1} \cdot \sigma_{1,2} \cdot \overline{\sigma_{0,1} \cdot CZ_{0,1} \cdot \sigma_{0,1} \cdot \sigma_{1,2} \cdot \sigma_{0,1}} \\
&\xleftarrow{S_3} \overline{\sigma_{0,1} \cdot \sigma_{1,2} \cdot \sigma_{0,1} \cdot CZ_{0,1} \cdot \sigma_{0,2}} \\
&\xleftarrow{S_3} \overline{\sigma_{0,2} \cdot CZ_{0,1} \cdot \sigma_{0,2}}
\end{aligned}$$

$$\begin{aligned}
(C_{18}) : CX_{0,2} \cdot \underline{CX_{2,1}} &\xrightarrow{S_5} CX_{0,2} \cdot \overline{\sigma_{1,2} \cdot \overline{CX_{1,2}} \cdot \sigma_{1,2}} \\
&\xrightarrow{(9)} \overline{\sigma_{1,2} \cdot \overline{CX_{0,1}} \cdot \underline{\sigma_{1,2}} \cdot \sigma_{1,2}} \cdot CX_{1,2} \cdot \sigma_{1,2} \\
&\xrightarrow{E_{10}} \sigma_{1,2} \cdot \overline{CX_{0,1}} \cdot CX_{1,2} \cdot \sigma_{1,2} \\
&\xrightarrow{C_{17}} \sigma_{1,2} \cdot \overline{CX_{1,2} \cdot \overline{CX_{0,1}} \cdot \overline{CX_{0,2}} \cdot \sigma_{1,2}} \\
&\xrightarrow{(9)} \sigma_{1,2} \cdot CX_{1,2} \cdot CX_{0,1} \cdot \overline{\sigma_{1,2} \cdot \overline{CX_{0,1}} \cdot \underline{\sigma_{1,2}} \cdot \sigma_{1,2}} \\
&\xrightarrow{E_{10}} \sigma_{1,2} \cdot CX_{1,2} \cdot CX_{0,1} \cdot \sigma_{1,2} \cdot CX_{0,1} \\
&\xleftarrow{E_{10}} \sigma_{1,2} \cdot CX_{1,2} \cdot \overline{\sigma_{1,2} \cdot \underline{\sigma_{1,2}} \cdot \overline{CX_{0,1}} \cdot \sigma_{1,2}} \cdot CX_{0,1} \\
&\xleftarrow{(9)} \underline{\sigma_{1,2} \cdot CX_{1,2} \cdot \sigma_{1,2}} \cdot \overline{CX_{0,2}} \cdot CX_{0,1} \\
&\xleftarrow{S_5} \overline{CX_{2,1}} \cdot CX_{0,2} \cdot CX_{0,1} \\
(C_{19}) : CX_{2,1} \cdot CX_{0,2} &\xleftarrow{(22)} \overline{CX_{2,1} \cdot CX_{0,2} \cdot \overline{CX_{0,1}} \cdot \overline{CX_{0,1}}} \\
&\xleftarrow{C_{18}} \overline{CX_{0,2} \cdot CX_{2,1}} \cdot CX_{0,1} \\
(C_{20}) : CX_{0,1} \cdot CX_{2,1} &\xleftarrow{E_{15}} \overline{CX_{0,2} \cdot \overline{CX_{0,2}} \cdot CX_{0,1} \cdot CX_{2,1}} \\
&\xleftarrow{E_9} CX_{0,2} \cdot \overline{CX_{2,1}} \cdot \overline{CX_{2,1}} \cdot CX_{0,2} \cdot \overline{CX_{0,1}} \cdot CX_{2,1} \\
&\xleftarrow{C_{18}} CX_{0,2} \cdot CX_{2,1} \cdot \overline{CX_{0,2}} \cdot \overline{CX_{2,1}} \cdot CX_{2,1} \\
&\xrightarrow{E_9} CX_{0,2} \cdot \overline{CX_{2,1}} \cdot CX_{0,2} \\
&\xrightarrow{C_{19}} \overline{CX_{0,2} \cdot \overline{CX_{0,2}} \cdot CX_{2,1} \cdot \overline{CX_{0,1}}} \\
&\xrightarrow{E_{15}} CX_{2,1} \cdot CX_{0,1} \\
(C_{21}) : CX_{1,2} \cdot \underline{CZ_{0,1}} &\xrightarrow{(1)} \overline{CX_{1,2} \cdot \overline{K_{1,2}} \cdot \overline{CX_{0,1}} \cdot \overline{K_{1,2}}} \\
&\xrightarrow{(7)} \overline{K_{1,2} \cdot \overline{CX_{2,1}} \cdot \underline{K_{1,2}} \cdot K_{1,2}} \cdot CX_{0,1} \cdot K_{1,2} \\
&\xrightarrow{(23)} K_{1,2} \cdot \overline{CX_{2,1}} \cdot \overline{CX_{0,1}} \cdot K_{1,2} \\
&\xleftarrow{C_{20}} K_{1,2} \cdot \overline{CX_{0,1}} \cdot \overline{CX_{2,1}} \cdot K_{1,2} \\
&\xleftarrow{(23)} K_{1,2} \cdot CX_{0,1} \cdot \overline{K_{1,2}} \cdot \underline{K_{1,2}} \cdot \overline{CX_{2,1}} \cdot K_{1,2} \\
&\xleftarrow{(7)} \underline{K_{1,2} \cdot CX_{0,1} \cdot K_{1,2}} \cdot \overline{CX_{1,2}} \\
&\xleftarrow{(1)} \overline{CZ_{0,1}} \cdot CX_{1,2} \\
(C_{22}) : CX_{0,1} \cdot CX_{0,2} &\xleftarrow{E_9} \overline{CX_{2,1} \cdot \overline{CX_{2,1}} \cdot CX_{0,1} \cdot CX_{0,2}} \\
&\xleftarrow{E_{15}} CX_{2,1} \cdot \overline{CX_{0,2}} \cdot \overline{CX_{0,2}} \cdot CX_{2,1} \cdot \overline{CX_{0,1}} \cdot CX_{0,2} \\
&\xleftarrow{C_{19}} CX_{2,1} \cdot CX_{0,2} \cdot \overline{CX_{2,1}} \cdot \overline{CX_{0,2}} \cdot CX_{0,2} \\
&\xrightarrow{E_{15}} CX_{2,1} \cdot \overline{CX_{0,2}} \cdot CX_{2,1} \\
&\xrightarrow{C_{18}} \overline{CX_{2,1} \cdot \overline{CX_{2,1}} \cdot \overline{CX_{0,2}} \cdot \overline{CX_{0,1}}} \\
&\xrightarrow{E_9} CX_{0,2} \cdot CX_{0,1} \\
(C_{23}) : CX_{0,1} \cdot \underline{CZ_{0,2}} &\xrightarrow{(18)} CX_{0,1} \cdot \overline{\sigma_{1,2} \cdot \overline{CZ_{0,1}} \cdot \sigma_{1,2}} \\
&\xleftarrow{E_{10}} \overline{\sigma_{1,2} \cdot \underline{\sigma_{1,2}} \cdot \overline{CX_{0,1}} \cdot \sigma_{1,2}} \cdot CZ_{0,1} \cdot \sigma_{1,2} \\
&\xleftarrow{(9)} \sigma_{1,2} \cdot \overline{CX_{0,2}} \cdot \overline{CZ_{0,1}} \cdot \sigma_{1,2} \\
&\xrightarrow{S_{24}} \sigma_{1,2} \cdot CX_{0,2} \cdot \overline{\sigma_{0,1} \cdot \overline{CZ_{0,1}} \cdot \sigma_{0,1}} \cdot \sigma_{1,2} \\
&\xleftarrow{E_4} \sigma_{1,2} \cdot \overline{\sigma_{0,1}} \cdot \overline{\sigma_{0,1}} \cdot \overline{CX_{0,2} \cdot \sigma_{0,1}} \cdot CZ_{0,1} \cdot \sigma_{0,1} \cdot \sigma_{1,2} \\
&\xleftarrow{(30)} \sigma_{1,2} \cdot \sigma_{0,1} \cdot \overline{CX_{1,2}} \cdot \overline{CZ_{0,1}} \cdot \sigma_{0,1} \cdot \sigma_{1,2} \\
&\xrightarrow{C_{21}} \sigma_{1,2} \cdot \sigma_{0,1} \cdot \overline{CZ_{0,1}} \cdot \overline{CX_{1,2}} \cdot \sigma_{0,1} \cdot \sigma_{1,2} \\
&\xrightarrow{(30)} \sigma_{1,2} \cdot \sigma_{0,1} \cdot CZ_{0,1} \cdot \overline{\sigma_{0,1} \cdot \overline{CX_{0,2}} \cdot \underline{\sigma_{0,1}} \cdot \sigma_{1,2}} \\
&\xrightarrow{E_4} \sigma_{1,2} \cdot \overline{\sigma_{0,1}} \cdot \overline{CZ_{0,1}} \cdot \overline{CX_{0,2}} \cdot \sigma_{1,2} \\
&\xleftarrow{S_{24}} \sigma_{1,2} \cdot \overline{CZ_{0,1}} \cdot \overline{CX_{0,2}} \cdot \sigma_{1,2} \\
&\xrightarrow{(9)} \sigma_{1,2} \cdot CZ_{0,1} \cdot \overline{\sigma_{1,2} \cdot \overline{CX_{0,1}} \cdot \underline{\sigma_{1,2}} \cdot \sigma_{1,2}} \\
&\xrightarrow{E_{10}} \overline{\sigma_{1,2} \cdot CZ_{0,1} \cdot \sigma_{1,2}} \cdot CX_{0,1} \\
&\xleftarrow{(18)} \overline{CZ_{0,2}} \cdot CX_{0,1} \\
(C_{24}) : CX_{0,2} \cdot CZ_{0,1} &\xleftarrow{E_{10}} \overline{CX_{0,2} \cdot \overline{CZ_{0,1}} \cdot \underline{\sigma_{1,2}} \cdot \sigma_{1,2}} \\
&\xrightarrow{(9)} \overline{\sigma_{1,2} \cdot \overline{CX_{0,1}} \cdot \underline{\sigma_{1,2}} \cdot \overline{CZ_{0,1}} \cdot \sigma_{1,2}} \cdot \sigma_{1,2} \\
&\xleftarrow{(18)} \sigma_{1,2} \cdot \overline{CX_{0,1}} \cdot \overline{CZ_{0,2}} \cdot \sigma_{1,2} \\
&\xrightarrow{C_{23}} \sigma_{1,2} \cdot \overline{CZ_{0,2}} \cdot \overline{CX_{0,1}} \cdot \sigma_{1,2} \\
&\xrightarrow{(18)} \sigma_{1,2} \cdot \overline{\sigma_{1,2}} \cdot \overline{CZ_{0,1}} \cdot \underline{\sigma_{1,2}} \cdot \overline{CX_{0,1}} \cdot \sigma_{1,2} \\
&\xleftarrow{(9)} \underline{\sigma_{1,2} \cdot \sigma_{1,2}} \cdot CZ_{0,1} \cdot \overline{CX_{0,2}} \\
&\xrightarrow{E_{10}} CZ_{0,1} \cdot CX_{0,2}
\end{aligned}$$

$$(B_7) : \underline{Z_0} \cdot CX_{1,2} \xrightarrow{(3)} \overline{CZ_{0,1} \cdot CX_{0,1} \cdot CZ_{0,1} \cdot CX_{0,1} \cdot CX_{1,2}}$$

$$\xrightarrow{C_{17}} CZ_{0,1} \cdot CX_{0,1} \cdot \overline{CZ_{0,1} \cdot CX_{1,2} \cdot CX_{0,1} \cdot CX_{0,2}}$$

$$\xleftarrow{C_{21}} CZ_{0,1} \cdot \overline{CX_{0,1} \cdot CX_{1,2} \cdot CZ_{0,1} \cdot CX_{0,1} \cdot CX_{0,2}}$$

$$\xrightarrow{C_{17}} \overline{CZ_{0,1} \cdot CX_{1,2} \cdot CX_{0,1} \cdot CX_{0,2} \cdot CZ_{0,1} \cdot CX_{0,1} \cdot CX_{0,2}}$$

$$\xleftarrow{C_{21}} \overline{CX_{1,2} \cdot CZ_{0,1} \cdot CX_{0,1} \cdot CX_{0,2} \cdot CZ_{0,1} \cdot CX_{0,1} \cdot CX_{0,2}}$$

$$\xrightarrow{C_{24}} CX_{1,2} \cdot CZ_{0,1} \cdot CX_{0,1} \cdot \overline{CZ_{0,1} \cdot CX_{0,2} \cdot CX_{0,1} \cdot CX_{0,2}}$$

$$\xleftarrow{C_{22}} CX_{1,2} \cdot CZ_{0,1} \cdot CX_{0,1} \cdot CZ_{0,1} \cdot \overline{CX_{0,1} \cdot CX_{0,2} \cdot CX_{0,2}}$$

$$\xrightarrow{E_{15}} CX_{1,2} \cdot \overline{CZ_{0,1} \cdot CX_{0,1} \cdot CZ_{0,1} \cdot CX_{0,1}}$$

$$\xleftarrow{(3)} CX_{1,2} \cdot \overline{Z_0}$$

$$(B_9) : \underline{Z_1} \cdot CX_{2,0} \xrightarrow{(34)} \overline{\sigma_{0,1} \cdot Z_0 \cdot \sigma_{0,1} \cdot CX_{2,0}}$$

$$\xrightarrow{S_6} \sigma_{0,1} \cdot Z_0 \cdot \overline{\sigma_{0,1} \cdot \sigma_{0,1} \cdot CX_{2,1} \cdot \sigma_{0,1}}$$

$$\xrightarrow{E_4} \sigma_{0,1} \cdot \overline{Z_0 \cdot CX_{2,1} \cdot \sigma_{0,1}}$$

$$\xrightarrow{B_8} \sigma_{0,1} \cdot \overline{CX_{2,1} \cdot Z_0 \cdot \sigma_{0,1}}$$

$$\xleftarrow{E_4} \sigma_{0,1} \cdot CX_{2,1} \cdot \overline{\sigma_{0,1} \cdot \sigma_{0,1} \cdot Z_0 \cdot \sigma_{0,1}}$$

$$\xleftarrow{(34)} \overline{\sigma_{0,1} \cdot CX_{2,1} \cdot \sigma_{0,1} \cdot \overline{Z_1}}$$

$$\xleftarrow{S_6} \overline{CX_{2,0} \cdot Z_1}$$

$$(S_{26}) : Z_1 \xleftarrow{E_{16}} \overline{\sigma_{0,2} \cdot \sigma_{0,2} \cdot Z_1}$$

$$\xrightarrow{(10)} \sigma_{0,2} \cdot \overline{CX_{0,2} \cdot CX_{2,0} \cdot CX_{0,2} \cdot Z_1}$$

$$\xleftarrow{B_{10}} \sigma_{0,2} \cdot CX_{0,2} \cdot \overline{CX_{2,0} \cdot \overline{Z_1} \cdot CX_{0,2}}$$

$$\xleftarrow{B_9} \sigma_{0,2} \cdot \overline{CX_{0,2} \cdot \overline{Z_1} \cdot CX_{2,0} \cdot CX_{0,2}}$$

$$\xleftarrow{B_{10}} \sigma_{0,2} \cdot \overline{Z_1 \cdot CX_{0,2} \cdot CX_{2,0} \cdot CX_{0,2}}$$

$$\xleftarrow{(10)} \sigma_{0,2} \cdot Z_1 \cdot \overline{\sigma_{0,2}}$$

$$(B_{12}) : Z_0 \cdot \underline{\sigma_{1,2}} \xrightarrow{(8)} \overline{Z_0 \cdot CX_{1,2} \cdot CX_{2,1} \cdot CX_{1,2}}$$

$$\xrightarrow{B_7} \overline{CX_{1,2} \cdot Z_0 \cdot CX_{2,1} \cdot CX_{1,2}}$$

$$\xrightarrow{B_8} CX_{1,2} \cdot \overline{CX_{2,1} \cdot Z_0 \cdot CX_{1,2}}$$

$$\xrightarrow{B_7} \overline{CX_{1,2} \cdot CX_{2,1} \cdot CX_{1,2} \cdot Z_0}$$

$$\xleftarrow{(8)} \overline{\sigma_{1,2} \cdot Z_0}$$

$$(B_8) : Z_0 \cdot CX_{2,1} \xleftarrow{(23)} \overline{Z_0 \cdot \overline{K_{1,2} \cdot K_{1,2} \cdot CX_{2,1}}}$$

$$\xrightarrow{C_4} \overline{Z_0 \cdot K_{1,2} \cdot \overline{CX_{1,2} \cdot K_{1,2}}}$$

$$\xrightarrow{B_6} \overline{K_{1,2} \cdot Z_0 \cdot CX_{1,2} \cdot K_{1,2}}$$

$$\xrightarrow{B_7} K_{1,2} \cdot \overline{CX_{1,2} \cdot Z_0 \cdot K_{1,2}}$$

$$\xrightarrow{B_6} K_{1,2} \cdot \overline{CX_{1,2} \cdot \overline{K_{1,2} \cdot Z_0}}$$

$$\xleftarrow{C_4} \overline{K_{1,2} \cdot \overline{K_{1,2} \cdot CX_{2,1} \cdot Z_0}}$$

$$\xrightarrow{(23)} CX_{2,1} \cdot Z_0$$

$$(B_{10}) : \underline{Z_1} \cdot CX_{0,2} \xrightarrow{(34)} \overline{\sigma_{0,1} \cdot Z_0 \cdot \sigma_{0,1} \cdot CX_{0,2}}$$

$$\xleftarrow{E_4} \sigma_{0,1} \cdot Z_0 \cdot \overline{\sigma_{0,1} \cdot CX_{0,2} \cdot \sigma_{0,1} \cdot \sigma_{0,1}}$$

$$\xleftarrow{(30)} \sigma_{0,1} \cdot \overline{Z_0 \cdot CX_{1,2} \cdot \sigma_{0,1}}$$

$$\xrightarrow{B_7} \sigma_{0,1} \cdot \overline{CX_{1,2} \cdot Z_0 \cdot \sigma_{0,1}}$$

$$\xrightarrow{(30)} \sigma_{0,1} \cdot \overline{\sigma_{0,1} \cdot CX_{0,2} \cdot \sigma_{0,1} \cdot Z_0 \cdot \sigma_{0,1}}$$

$$\xleftarrow{(34)} \overline{\sigma_{0,1} \cdot \sigma_{0,1} \cdot CX_{0,2} \cdot \overline{Z_1}}$$

$$\xrightarrow{E_4} CX_{0,2} \cdot Z_1$$

$$(B_{11}) : X_0 \cdot \underline{\sigma_{1,2}} \xrightarrow{(8)} \overline{X_0 \cdot CX_{1,2} \cdot CX_{2,1} \cdot CX_{1,2}}$$

$$\xleftarrow{(26)} \overline{CX_{1,2} \cdot \overline{X_0} \cdot CX_{2,1} \cdot CX_{1,2}}$$

$$\xleftarrow{B_1} CX_{1,2} \cdot \overline{CX_{2,1} \cdot \overline{X_0} \cdot CX_{1,2}}$$

$$\xleftarrow{(26)} \overline{CX_{1,2} \cdot CX_{2,1} \cdot CX_{1,2} \cdot X_0}$$

$$\xleftarrow{(8)} \overline{\sigma_{1,2} \cdot X_0}$$

$$(B_{13}) : X_0 \cdot \underline{X_2} \xrightarrow{S_{18}} \overline{X_0 \cdot \overline{\sigma_{1,2} \cdot X_1 \cdot \sigma_{1,2}}}$$

$$\xrightarrow{B_{11}} \overline{\sigma_{1,2} \cdot \overline{X_0} \cdot X_1 \cdot \sigma_{1,2}}$$

$$\xrightarrow{B_2} \sigma_{1,2} \cdot \overline{X_1 \cdot \overline{X_0} \cdot \sigma_{1,2}}$$

$$\xrightarrow{B_{11}} \overline{\sigma_{1,2} \cdot X_1 \cdot \overline{\sigma_{1,2} \cdot X_0}}$$

$$\xleftarrow{S_{18}} \overline{X_2 \cdot X_0}$$

$$\begin{aligned}
(B_{14}) : X_0 \cdot Z_1 &\stackrel{(23)}{\longleftarrow} X_0 \cdot \overline{K_{1,2}} \cdot \overline{K_{1,2}} \cdot Z_1 \\
&\stackrel{(27)}{\longrightarrow} \overline{K_{1,2}} \cdot \overline{X_0} \cdot \overline{K_{1,2}} \cdot Z_1 \\
&\stackrel{C_2}{\longleftarrow} K_{1,2} \cdot \overline{X_0} \cdot \overline{X_1} \cdot \overline{K_{1,2}} \\
&\stackrel{B_2}{\longrightarrow} K_{1,2} \cdot \overline{X_1} \cdot \overline{X_0} \cdot \overline{K_{1,2}} \\
&\stackrel{(27)}{\longrightarrow} K_{1,2} \cdot \overline{X_1} \cdot \overline{K_{1,2}} \cdot \overline{X_0} \\
&\stackrel{C_2}{\longrightarrow} \overline{K_{1,2}} \cdot \overline{K_{1,2}} \cdot \overline{Z_1} \cdot X_0 \\
&\stackrel{(23)}{\longrightarrow} Z_1 \cdot X_0
\end{aligned}$$

$$\begin{aligned}
(B_{15}) : X_1 \cdot Z_0 &\stackrel{(25)}{\longleftarrow} \overline{K_{0,1}} \cdot \overline{K_{0,1}} \cdot X_1 \cdot Z_0 \\
&\stackrel{C_{25}}{\longleftarrow} K_{0,1} \cdot \overline{Z_1} \cdot \overline{K_{0,1}} \cdot Z_0 \\
&\stackrel{(41)}{\longrightarrow} K_{0,1} \cdot \overline{Z_1} \cdot \overline{X_0} \cdot \overline{K_{0,1}} \\
&\stackrel{B_{14}}{\longleftarrow} K_{0,1} \cdot \overline{X_0} \cdot \overline{Z_1} \cdot \overline{K_{0,1}} \\
&\stackrel{C_{25}}{\longrightarrow} K_{0,1} \cdot \overline{X_0} \cdot \overline{K_{0,1}} \cdot \overline{X_1} \\
&\stackrel{(41)}{\longleftarrow} \overline{K_{0,1}} \cdot \overline{K_{0,1}} \cdot \overline{Z_0} \cdot X_1 \stackrel{(25)}{\longrightarrow} Z_0 \cdot X_1
\end{aligned}$$

$$\begin{aligned}
(B_{17}) : X_2 \cdot \overline{K_{0,1}} &\stackrel{(11)}{\longrightarrow} \overline{X_2} \cdot \overline{\sigma_{0,2}} \cdot \overline{K_{1,2}} \cdot \overline{\sigma_{0,2}} \\
&\stackrel{(15)}{\longrightarrow} \overline{\sigma_{0,2}} \cdot \overline{X_0} \cdot \overline{\sigma_{0,2}} \cdot \overline{\sigma_{0,2}} \cdot K_{1,2} \cdot \sigma_{0,2} \\
&\stackrel{E_{16}}{\longrightarrow} \sigma_{0,2} \cdot \overline{X_0} \cdot \overline{K_{1,2}} \cdot \sigma_{0,2} \\
&\stackrel{(27)}{\longrightarrow} \sigma_{0,2} \cdot \overline{K_{1,2}} \cdot \overline{X_0} \cdot \sigma_{0,2} \\
&\stackrel{E_{16}}{\longleftarrow} \sigma_{0,2} \cdot K_{1,2} \cdot \overline{\sigma_{0,2}} \cdot \overline{\sigma_{0,2}} \cdot X_0 \cdot \sigma_{0,2} \\
&\stackrel{(15)}{\longleftarrow} \overline{\sigma_{0,2}} \cdot \overline{K_{1,2}} \cdot \overline{\sigma_{0,2}} \cdot \overline{X_2} \stackrel{(11)}{\longleftarrow} \overline{K_{0,1}} \cdot X_2
\end{aligned}$$

$$\begin{aligned}
(B_{18}) : Z_2 \cdot K_{0,1} &\stackrel{(23)}{\longleftarrow} \overline{Z_2} \cdot \overline{K_{1,2}} \cdot \overline{K_{1,2}} \cdot K_{0,1} \\
&\stackrel{C_{26}}{\longleftarrow} \overline{K_{1,2}} \cdot \overline{X_2} \cdot \overline{K_{1,2}} \cdot \overline{K_{0,1}} \\
&\stackrel{(39)}{\longleftarrow} K_{1,2} \cdot \overline{X_2} \cdot \overline{K_{0,1}} \cdot \overline{K_{1,2}} \\
&\stackrel{B_{17}}{\longrightarrow} K_{1,2} \cdot \overline{K_{0,1}} \cdot \overline{X_2} \cdot K_{1,2} \\
&\stackrel{(39)}{\longleftarrow} \overline{K_{0,1}} \cdot \overline{K_{1,2}} \cdot \overline{X_2} \cdot K_{1,2} \\
&\stackrel{C_{26}}{\longrightarrow} K_{0,1} \cdot \overline{Z_2} \cdot \overline{K_{1,2}} \cdot \overline{K_{1,2}} \stackrel{(23)}{\longrightarrow} K_{0,1} \cdot Z_2
\end{aligned}$$

$$\begin{aligned}
(C_{25}) : \overline{Z_1} \cdot K_{0,1} &\stackrel{(34)}{\longrightarrow} \overline{\sigma_{0,1}} \cdot \overline{Z_0} \cdot \overline{\sigma_{0,1}} \cdot \overline{K_{0,1}} \\
&\stackrel{(35)}{\longrightarrow} \sigma_{0,1} \cdot Z_0 \cdot \overline{\sigma_{0,1}} \cdot \overline{\sigma_{0,1}} \cdot \overline{K_{0,1}} \cdot \sigma_{0,1} \\
&\stackrel{E_4}{\longrightarrow} \sigma_{0,1} \cdot Z_0 \cdot K_{0,1} \cdot \sigma_{0,1} \\
&\stackrel{(25)}{\longleftarrow} \sigma_{0,1} \cdot \overline{K_{0,1}} \cdot \overline{K_{0,1}} \cdot \overline{Z_0} \cdot K_{0,1} \cdot \sigma_{0,1} \\
&\stackrel{(41)}{\longrightarrow} \sigma_{0,1} \cdot K_{0,1} \cdot \overline{X_0} \cdot \overline{K_{0,1}} \cdot \overline{K_{0,1}} \cdot \sigma_{0,1} \\
&\stackrel{(25)}{\longrightarrow} \sigma_{0,1} \cdot \overline{K_{0,1}} \cdot X_0 \cdot \sigma_{0,1} \\
&\stackrel{(35)}{\longrightarrow} \overline{\sigma_{0,1}} \cdot \overline{\sigma_{0,1}} \cdot \overline{K_{0,1}} \cdot \overline{\sigma_{0,1}} \cdot X_0 \cdot \sigma_{0,1} \\
&\stackrel{E_4}{\longrightarrow} K_{0,1} \cdot \overline{\sigma_{0,1}} \cdot X_0 \cdot \overline{\sigma_{0,1}} \stackrel{(28)}{\longleftarrow} K_{0,1} \cdot \overline{X_1}
\end{aligned}$$

$$\begin{aligned}
(B_{16}) : CX_{0,1} \cdot \overline{X_2} &\stackrel{(15)}{\longrightarrow} CX_{0,1} \cdot \overline{\sigma_{0,2}} \cdot \overline{X_0} \cdot \overline{\sigma_{0,2}} \\
&\stackrel{E_{16}}{\longleftarrow} \overline{\sigma_{0,2}} \cdot \overline{\sigma_{0,2}} \cdot CX_{0,1} \cdot \overline{\sigma_{0,2}} \cdot X_0 \cdot \sigma_{0,2} \\
&\stackrel{S_9}{\longleftarrow} \sigma_{0,2} \cdot \overline{CX_{2,1}} \cdot X_0 \cdot \sigma_{0,2} \\
&\stackrel{B_1}{\longrightarrow} \sigma_{0,2} \cdot \overline{X_0} \cdot \overline{CX_{2,1}} \cdot \sigma_{0,2} \\
&\stackrel{S_9}{\longrightarrow} \sigma_{0,2} \cdot X_0 \cdot \overline{\sigma_{0,2}} \cdot \overline{CX_{0,1}} \cdot \overline{\sigma_{0,2}} \cdot \sigma_{0,2} \\
&\stackrel{E_{16}}{\longrightarrow} \sigma_{0,2} \cdot X_0 \cdot \overline{\sigma_{0,2}} \cdot CX_{0,1} \\
&\stackrel{(15)}{\longleftarrow} \overline{X_2} \cdot CX_{0,1}
\end{aligned}$$

$$\begin{aligned}
(C_{26}) : K_{1,2} \cdot X_2 &\stackrel{(23)}{\longleftarrow} K_{1,2} \cdot X_2 \cdot \overline{K_{1,2}} \cdot \overline{K_{1,2}} \\
&\stackrel{E_{19}}{\longleftarrow} K_{1,2} \cdot X_2 \cdot \overline{K_{1,2}} \cdot \overline{Z_2} \cdot \overline{Z_2} \cdot K_{1,2} \\
&\stackrel{C_{16}}{\longleftarrow} K_{1,2} \cdot \overline{X_2} \cdot \overline{K_{1,2}} \cdot \overline{Z_2} \cdot K_{1,2} \\
&\stackrel{E_{17}}{\longrightarrow} K_{1,2} \cdot \overline{K_{1,2}} \cdot Z_2 \cdot K_{1,2} \\
&\stackrel{(23)}{\longrightarrow} Z_2 \cdot K_{1,2}
\end{aligned}$$

$$\begin{aligned}
(B_{19}) : \overline{X_1} \cdot X_2 &\stackrel{(2)}{\longrightarrow} \overline{CX_{0,1}} \cdot \overline{X_0} \cdot \overline{CX_{0,1}} \cdot \overline{X_0} \cdot X_2 \\
&\stackrel{B_{13}}{\longrightarrow} CX_{0,1} \cdot X_0 \cdot \overline{CX_{0,1}} \cdot \overline{X_2} \cdot \overline{X_0} \\
&\stackrel{B_{16}}{\longrightarrow} CX_{0,1} \cdot \overline{X_0} \cdot \overline{X_2} \cdot \overline{CX_{0,1}} \cdot X_0 \\
&\stackrel{B_{13}}{\longrightarrow} \overline{CX_{0,1}} \cdot \overline{X_2} \cdot \overline{X_0} \cdot CX_{0,1} \cdot X_0 \\
&\stackrel{B_{16}}{\longrightarrow} \overline{X_2} \cdot \overline{CX_{0,1}} \cdot X_0 \cdot \overline{CX_{0,1}} \cdot X_0 \\
&\stackrel{(2)}{\longleftarrow} X_2 \cdot \overline{X_1}
\end{aligned}$$

$$\begin{aligned}
(C_{27}) : K_{1,2} \cdot X_1 &\xleftarrow{(23)} K_{1,2} \cdot X_1 \cdot \overline{K_{1,2} \cdot K_{1,2}} \\
&\xleftarrow{E_5} K_{1,2} \cdot X_1 \cdot \overline{K_{1,2} \cdot Z_1 \cdot K_{1,2}} \\
&\xleftarrow{C_2} K_{1,2} \cdot X_1 \cdot \overline{X_1 \cdot K_{1,2} \cdot Z_1 \cdot K_{1,2}} \\
&\xrightarrow{E_{13}} \overline{K_{1,2} \cdot K_{1,2} \cdot Z_1 \cdot K_{1,2}} \\
&\xrightarrow{(23)} Z_1 \cdot K_{1,2}
\end{aligned}$$

$$\begin{aligned}
(C_{28}) : K_{1,2} \cdot \underline{CZ_{0,2}} &\xrightarrow{(18)} K_{1,2} \cdot \overline{\sigma_{1,2} \cdot CZ_{0,1} \cdot \sigma_{1,2}} \\
&\xleftarrow{E_{10}} \overline{\sigma_{1,2} \cdot \overline{\sigma_{1,2} \cdot K_{1,2} \cdot \sigma_{1,2}} \cdot CZ_{0,1} \cdot \sigma_{1,2}} \\
&\xleftarrow{S_{10}} \sigma_{1,2} \cdot \overline{K_{1,2} \cdot CZ_{0,1} \cdot \sigma_{1,2}} \\
&\xrightarrow{(1)} \sigma_{1,2} \cdot \overline{K_{1,2} \cdot K_{1,2} \cdot CX_{0,1} \cdot K_{1,2} \cdot \sigma_{1,2}} \\
&\xrightarrow{(23)} \sigma_{1,2} \cdot CX_{0,1} \cdot K_{1,2} \cdot \sigma_{1,2} \\
&\xleftarrow{E_{10}} \sigma_{1,2} \cdot CX_{0,1} \cdot \overline{\sigma_{1,2} \cdot \overline{\sigma_{1,2} \cdot K_{1,2} \cdot \sigma_{1,2}}} \\
&\xleftarrow{S_{10}} \overline{\sigma_{1,2} \cdot CX_{0,1} \cdot \sigma_{1,2} \cdot K_{1,2}} \\
&\xleftarrow{(9)} \overline{CX_{0,2} \cdot K_{1,2}}
\end{aligned}$$

$$\begin{aligned}
(C_{29}) : CZ_{0,2} \cdot K_{1,2} &\xleftarrow{E_{15}} CZ_{0,2} \cdot K_{1,2} \cdot \overline{CX_{0,2} \cdot CX_{0,2}} \\
&\xleftarrow{(23)} CZ_{0,2} \cdot K_{1,2} \cdot \overline{CX_{0,2} \cdot K_{1,2} \cdot K_{1,2} \cdot CX_{0,2}} \\
&\xleftarrow{C_{28}} CZ_{0,2} \cdot \overline{K_{1,2} \cdot K_{1,2} \cdot CZ_{0,2} \cdot K_{1,2} \cdot CX_{0,2}} \\
&\xrightarrow{(23)} \overline{CZ_{0,2} \cdot CZ_{0,2} \cdot K_{1,2} \cdot CX_{0,2}} \\
&\xrightarrow{E_{11}} K_{1,2} \cdot CX_{0,2}
\end{aligned}$$

$$\begin{aligned}
(B_{20}) : CZ_{0,2} \cdot Z_1 &\xleftarrow{(23)} \overline{K_{1,2} \cdot K_{1,2} \cdot CZ_{0,2} \cdot Z_1} \\
&\xrightarrow{C_{28}} K_{1,2} \cdot \overline{CX_{0,2} \cdot K_{1,2} \cdot Z_1} \\
&\xleftarrow{C_2} K_{1,2} \cdot \overline{CX_{0,2} \cdot X_1 \cdot K_{1,2}} \\
&\xrightarrow{B_3} \overline{K_{1,2} \cdot X_1 \cdot CX_{0,2} \cdot K_{1,2}} \\
&\xrightarrow{C_{27}} \overline{Z_1 \cdot K_{1,2} \cdot CX_{0,2} \cdot K_{1,2}} \\
&\xleftarrow{C_{29}} Z_1 \cdot \overline{CZ_{0,2} \cdot K_{1,2} \cdot K_{1,2}} \xrightarrow{(23)} Z_1 \cdot CZ_{0,2}
\end{aligned}$$

$$\begin{aligned}
(B_{21}) : \underline{CX_{1,0}} \cdot X_2 &\xrightarrow{(12)} \overline{K_{0,1} \cdot CX_{0,1} \cdot K_{0,1} \cdot X_2} \\
&\xleftarrow{B_{17}} K_{0,1} \cdot \overline{CX_{0,1} \cdot X_2 \cdot K_{0,1}} \\
&\xrightarrow{B_{16}} \overline{K_{0,1} \cdot X_2 \cdot CX_{0,1} \cdot K_{0,1}} \\
&\xleftarrow{B_{17}} \overline{X_2 \cdot K_{0,1} \cdot CX_{0,1} \cdot K_{0,1}} \\
&\xleftarrow{(12)} X_2 \cdot \overline{CX_{1,0}}
\end{aligned}$$

$$\begin{aligned}
(B_{22}) : X_2 \cdot \underline{\sigma_{0,1}} &\xrightarrow{(13)} X_2 \cdot \overline{CX_{0,1} \cdot CX_{1,0} \cdot CX_{0,1}} \\
&\xleftarrow{B_{16}} \overline{CX_{0,1} \cdot X_2 \cdot CX_{1,0} \cdot CX_{0,1}} \\
&\xleftarrow{B_{21}} CX_{0,1} \cdot \overline{CX_{1,0} \cdot X_2 \cdot CX_{0,1}} \\
&\xleftarrow{B_{16}} \overline{CX_{0,1} \cdot CX_{1,0} \cdot CX_{0,1} \cdot X_2} \\
&\xleftarrow{(13)} \overline{\sigma_{0,1} \cdot X_2}
\end{aligned}$$

$$\begin{aligned}
(B_{23}) : X_2 \cdot Z_0 &\xleftarrow{(25)} X_2 \cdot \overline{K_{0,1} \cdot K_{0,1} \cdot Z_0} \\
&\xrightarrow{(41)} \overline{X_2 \cdot K_{0,1} \cdot X_0 \cdot K_{0,1}} \\
&\xrightarrow{B_{17}} \overline{K_{0,1} \cdot X_2 \cdot X_0 \cdot K_{0,1}} \\
&\xleftarrow{B_{13}} K_{0,1} \cdot \overline{X_0 \cdot X_2 \cdot K_{0,1}} \\
&\xrightarrow{B_{17}} K_{0,1} \cdot \overline{X_0 \cdot K_{0,1} \cdot X_2} \\
&\xleftarrow{(41)} \overline{K_{0,1} \cdot K_{0,1} \cdot Z_0 \cdot X_2} \\
&\xrightarrow{(25)} Z_0 \cdot X_2
\end{aligned}$$

$$\begin{aligned}
(B_{24}) : X_2 \cdot \underline{Z_1} &\xrightarrow{(34)} X_2 \cdot \overline{\sigma_{0,1} \cdot Z_0 \cdot \sigma_{0,1}} \\
&\xrightarrow{B_{22}} \overline{\sigma_{0,1} \cdot X_2 \cdot Z_0 \cdot \sigma_{0,1}} \\
&\xrightarrow{B_{23}} \sigma_{0,1} \cdot \overline{Z_0 \cdot X_2 \cdot \sigma_{0,1}} \\
&\xrightarrow{B_{22}} \overline{\sigma_{0,1} \cdot Z_0 \cdot \sigma_{0,1} \cdot X_2} \\
&\xleftarrow{(34)} \overline{Z_1 \cdot X_2}
\end{aligned}$$

$$\begin{aligned}
(B_{25}) : X_1 \cdot Z_2 &\xleftarrow{(23)} \overline{K_{1,2} \cdot K_{1,2} \cdot X_1 \cdot Z_2} \\
&\xrightarrow{C_{27}} K_{1,2} \cdot \overline{Z_1 \cdot K_{1,2} \cdot Z_2} \\
&\xleftarrow{C_{16}} K_{1,2} \cdot \overline{Z_1 \cdot X_2 \cdot K_{1,2}} \\
&\xleftarrow{B_{24}} \overline{K_{1,2} \cdot X_2 \cdot Z_1 \cdot K_{1,2}} \\
&\xrightarrow{C_{26}} \overline{Z_2 \cdot K_{1,2} \cdot Z_1 \cdot K_{1,2}} \\
&\xleftarrow{C_2} \overline{Z_2 \cdot X_1 \cdot K_{1,2} \cdot K_{1,2}} \\
&\xrightarrow{(23)} Z_2 \cdot X_1
\end{aligned}$$

$$\begin{aligned}
(B_{26}) : X_0 \cdot \underline{Z_2} &\xrightarrow{(16)} X_0 \cdot \overline{\sigma_{0,2} \cdot Z_0 \cdot \sigma_{0,2}} \\
&\xleftarrow{E_{16}} \overline{\sigma_{0,2} \cdot \sigma_{0,2} \cdot X_0 \cdot \sigma_{0,2} \cdot Z_0 \cdot \sigma_{0,2}} \\
&\xleftarrow{(15)} \sigma_{0,2} \cdot \overline{X_2 \cdot Z_0 \cdot \sigma_{0,2}} \\
&\xrightarrow{B_{23}} \sigma_{0,2} \cdot \overline{Z_0 \cdot X_2 \cdot \sigma_{0,2}} \\
&\xrightarrow{(15)} \overline{\sigma_{0,2} \cdot Z_0 \cdot \sigma_{0,2} \cdot X_0 \cdot \sigma_{0,2} \cdot \sigma_{0,2}} \\
&\xleftarrow{(16)} \overline{Z_2 \cdot X_0 \cdot \sigma_{0,2} \cdot \sigma_{0,2}} \\
&\xrightarrow{E_{16}} Z_2 \cdot X_0
\end{aligned}$$

$$\begin{aligned}
(B_{27}) : \underline{CZ_{0,1}} \cdot Z_2 &\xrightarrow{(1)} \overline{K_{1,2} \cdot CX_{0,1} \cdot K_{1,2} \cdot Z_2} \\
&\xleftarrow{C_{16}} K_{1,2} \cdot \overline{CX_{0,1} \cdot X_2 \cdot K_{1,2}} \\
&\xrightarrow{B_{16}} \overline{K_{1,2} \cdot X_2 \cdot CX_{0,1} \cdot K_{1,2}} \\
&\xrightarrow{C_{26}} \overline{Z_2 \cdot K_{1,2} \cdot CX_{0,1} \cdot K_{1,2}} \\
&\xleftarrow{(1)} \overline{Z_2 \cdot CZ_{0,1}}
\end{aligned}$$

$$\begin{aligned}
(B_{28}) : Z_0 \cdot Z_2 &\xleftarrow{(25)} \overline{K_{0,1} \cdot K_{0,1} \cdot Z_0 \cdot Z_2} \\
&\xrightarrow{(41)} K_{0,1} \cdot \overline{X_0 \cdot K_{0,1} \cdot Z_2} \\
&\xleftarrow{B_{18}} K_{0,1} \cdot \overline{X_0 \cdot Z_2 \cdot K_{0,1}} \\
&\xrightarrow{B_{26}} \overline{K_{0,1} \cdot Z_2 \cdot X_0 \cdot K_{0,1}} \\
&\xleftarrow{B_{18}} \overline{Z_2 \cdot K_{0,1} \cdot X_0 \cdot K_{0,1}} \\
&\xleftarrow{(41)} \overline{Z_2 \cdot K_{0,1} \cdot K_{0,1} \cdot Z_0} \\
&\xrightarrow{(25)} Z_2 \cdot Z_0
\end{aligned}$$

$$\begin{aligned}
(C_{30}) : X_1 \cdot K_{0,1} &\xleftarrow{E_5} X_1 \cdot K_{0,1} \cdot \overline{Z_1 \cdot Z_1} \\
&\xleftarrow{(25)} X_1 \cdot K_{0,1} \cdot \overline{Z_1 \cdot K_{0,1} \cdot K_{0,1} \cdot Z_1} \\
&\xrightarrow{C_{25}} X_1 \cdot \overline{K_{0,1} \cdot K_{0,1} \cdot X_1 \cdot K_{0,1} \cdot Z_1} \\
&\xrightarrow{(25)} \overline{X_1 \cdot X_1 \cdot K_{0,1} \cdot Z_1} \\
&\xrightarrow{E_{13}} K_{0,1} \cdot Z_1
\end{aligned}$$

$$\begin{aligned}
(B_{29}) : Z_0 \cdot Z_1 &\xleftarrow{(25)} \overline{K_{0,1} \cdot K_{0,1} \cdot Z_0 \cdot Z_1} \\
&\xrightarrow{(41)} K_{0,1} \cdot \overline{X_0 \cdot K_{0,1} \cdot Z_1} \\
&\xleftarrow{C_{30}} K_{0,1} \cdot \overline{X_0 \cdot X_1 \cdot K_{0,1}} \\
&\xrightarrow{B_2} K_{0,1} \cdot \overline{X_1 \cdot X_0 \cdot K_{0,1}} \\
&\xleftarrow{(41)} K_{0,1} \cdot \overline{X_1 \cdot K_{0,1} \cdot Z_0} \\
&\xrightarrow{C_{30}} \overline{K_{0,1} \cdot K_{0,1} \cdot Z_1 \cdot Z_0} \\
&\xrightarrow{(25)} Z_1 \cdot Z_0
\end{aligned}$$

$$\begin{aligned}
(B_{30}) : Z_2 \cdot CX_{0,1} &\xleftarrow{(25)} Z_2 \cdot CX_{0,1} \cdot \overline{K_{0,1} \cdot K_{0,1}} \\
&\xleftarrow{(25)} Z_2 \cdot \overline{K_{0,1} \cdot K_{0,1}} \cdot CX_{0,1} \cdot K_{0,1} \cdot K_{0,1} \\
&\xleftarrow{(12)} Z_2 \cdot K_{0,1} \cdot \overline{CX_{1,0}} \cdot K_{0,1} \\
&\xrightarrow{B_{18}} \overline{K_{0,1} \cdot Z_2} \cdot CX_{1,0} \cdot K_{0,1} \\
&\xrightarrow{(16)} K_{0,1} \cdot \overline{\sigma_{0,2} \cdot Z_0 \cdot \sigma_{0,2}} \cdot CX_{1,0} \cdot K_{0,1} \\
&\xleftarrow{E_{16}} K_{0,1} \cdot \sigma_{0,2} \cdot Z_0 \cdot \overline{\sigma_{0,2} \cdot CX_{1,0} \cdot \sigma_{0,2} \cdot \sigma_{0,2}} \cdot K_{0,1} \\
&\xleftarrow{S_7} K_{0,1} \cdot \sigma_{0,2} \cdot \overline{Z_0 \cdot CX_{1,2}} \cdot \sigma_{0,2} \cdot K_{0,1} \\
&\xrightarrow{B_7} K_{0,1} \cdot \sigma_{0,2} \cdot \overline{CX_{1,2}} \cdot Z_0 \cdot \sigma_{0,2} \cdot K_{0,1} \\
&\xrightarrow{S_7} K_{0,1} \cdot \overline{\sigma_{0,2} \cdot \sigma_{0,2} \cdot CX_{1,0} \cdot \sigma_{0,2}} \cdot Z_0 \cdot \sigma_{0,2} \cdot K_{0,1} \\
&\xrightarrow{E_{16}} K_{0,1} \cdot CX_{1,0} \cdot \overline{\sigma_{0,2} \cdot Z_0 \cdot \sigma_{0,2}} \cdot K_{0,1} \\
&\xleftarrow{(16)} K_{0,1} \cdot \overline{CX_{1,0}} \cdot \overline{Z_2} \cdot K_{0,1} \\
&\xrightarrow{(12)} \overline{K_{0,1} \cdot K_{0,1}} \cdot CX_{0,1} \cdot \overline{K_{0,1}} \cdot Z_2 \cdot K_{0,1} \\
&\xrightarrow{(25)} CX_{0,1} \cdot K_{0,1} \cdot \overline{Z_2 \cdot K_{0,1}} \\
&\xrightarrow{B_{18}} CX_{0,1} \cdot \overline{K_{0,1} \cdot K_{0,1}} \cdot Z_2 \xrightarrow{(25)} CX_{0,1} \cdot Z_2
\end{aligned}$$

$$\begin{aligned}
(B_{32}) : Z_2 \cdot CX_{1,0} &\xrightarrow{(12)} Z_2 \cdot \overline{K_{0,1} \cdot CX_{0,1} \cdot K_{0,1}} \\
&\xrightarrow{B_{18}} \overline{K_{0,1} \cdot Z_2} \cdot CX_{0,1} \cdot K_{0,1} \\
&\xrightarrow{B_{30}} K_{0,1} \cdot \overline{CX_{0,1} \cdot Z_2} \cdot K_{0,1} \\
&\xrightarrow{B_{18}} \overline{K_{0,1} \cdot CX_{0,1} \cdot K_{0,1}} \cdot Z_2 \xleftarrow{(12)} \overline{CX_{1,0}} \cdot Z_2
\end{aligned}$$

$$\begin{aligned}
(B_{34}) : Z_1 \cdot Z_2 &\xleftarrow{(23)} \overline{K_{1,2} \cdot K_{1,2}} \cdot Z_1 \cdot Z_2 \\
&\xleftarrow{C_2} K_{1,2} \cdot \overline{X_1 \cdot K_{1,2}} \cdot Z_2 \\
&\xleftarrow{C_{16}} K_{1,2} \cdot X_1 \cdot \overline{X_2} \cdot K_{1,2} \\
&\xrightarrow{B_{19}} K_{1,2} \cdot \overline{X_2 \cdot X_1} \cdot K_{1,2} \\
&\xrightarrow{C_2} K_{1,2} \cdot X_2 \cdot \overline{K_{1,2} \cdot Z_1} \\
&\xrightarrow{C_{16}} K_{1,2} \cdot \overline{K_{1,2} \cdot Z_2} \cdot Z_1 \\
&\xrightarrow{(23)} Z_2 \cdot Z_1
\end{aligned}$$

$$\begin{aligned}
(B_{31}) : CZ_{1,2} \cdot Z_0 &\xrightarrow{(19)} \overline{\sigma_{0,1} \cdot CZ_{0,2} \cdot \sigma_{0,1}} \cdot Z_0 \\
&\xleftarrow{E_4} \sigma_{0,1} \cdot CZ_{0,2} \cdot \overline{\sigma_{0,1} \cdot Z_0 \cdot \sigma_{0,1}} \cdot \sigma_{0,1} \\
&\xleftarrow{(34)} \sigma_{0,1} \cdot CZ_{0,2} \cdot \overline{Z_1} \cdot \sigma_{0,1} \\
&\xleftarrow{(23)} \sigma_{0,1} \cdot \overline{K_{1,2} \cdot K_{1,2}} \cdot CZ_{0,2} \cdot Z_1 \cdot \sigma_{0,1} \\
&\xrightarrow{C_{28}} \sigma_{0,1} \cdot K_{1,2} \cdot \overline{CX_{0,2} \cdot K_{1,2}} \cdot Z_1 \cdot \sigma_{0,1} \\
&\xleftarrow{C_2} \sigma_{0,1} \cdot K_{1,2} \cdot \overline{CX_{0,2} \cdot X_1 \cdot K_{1,2}} \cdot \sigma_{0,1} \\
&\xrightarrow{B_3} \sigma_{0,1} \cdot \overline{K_{1,2} \cdot X_1} \cdot CX_{0,2} \cdot K_{1,2} \cdot \sigma_{0,1} \\
&\xrightarrow{C_{27}} \sigma_{0,1} \cdot \overline{Z_1 \cdot K_{1,2}} \cdot CX_{0,2} \cdot K_{1,2} \cdot \sigma_{0,1} \\
&\xleftarrow{C_{29}} \sigma_{0,1} \cdot Z_1 \cdot \overline{CZ_{0,2} \cdot K_{1,2} \cdot K_{1,2}} \cdot \sigma_{0,1} \\
&\xrightarrow{(23)} \sigma_{0,1} \cdot \overline{Z_1} \cdot CZ_{0,2} \cdot \sigma_{0,1} \\
&\xrightarrow{(34)} \sigma_{0,1} \cdot \overline{\sigma_{0,1} \cdot Z_0 \cdot \sigma_{0,1}} \cdot CZ_{0,2} \cdot \sigma_{0,1} \\
&\xrightarrow{E_4} Z_0 \cdot \overline{\sigma_{0,1} \cdot CZ_{0,2}} \cdot \sigma_{0,1} \\
&\xleftarrow{(19)} Z_0 \cdot \overline{CZ_{1,2}}
\end{aligned}$$

$$\begin{aligned}
(B_{33}) : Z_2 \cdot \overline{\sigma_{0,1}} &\xrightarrow{(13)} Z_2 \cdot \overline{CX_{0,1} \cdot CX_{1,0} \cdot CX_{0,1}} \\
&\xrightarrow{B_{30}} \overline{CX_{0,1} \cdot Z_2} \cdot CX_{1,0} \cdot CX_{0,1} \\
&\xrightarrow{B_{32}} CX_{0,1} \cdot \overline{CX_{1,0} \cdot Z_2} \cdot CX_{0,1} \\
&\xrightarrow{B_{30}} \overline{CX_{0,1} \cdot CX_{1,0} \cdot CX_{0,1}} \cdot Z_2 \xleftarrow{(13)} \overline{\sigma_{0,1}} \cdot Z_2
\end{aligned}$$

$$\begin{aligned}
(B_{35}) : X_1 \cdot CZ_{0,2} &\xrightarrow{(18)} X_1 \cdot \overline{\sigma_{1,2} \cdot CZ_{0,1} \cdot \sigma_{1,2}} \\
&\xleftarrow{E_{10}} \overline{\sigma_{1,2} \cdot \sigma_{1,2}} \cdot X_1 \cdot \overline{\sigma_{1,2}} \cdot CZ_{0,1} \cdot \sigma_{1,2} \\
&\xleftarrow{S_{18}} \sigma_{1,2} \cdot \overline{X_2} \cdot \overline{CZ_{0,1}} \cdot \sigma_{1,2} \\
&\xrightarrow{(1)} \sigma_{1,2} \cdot X_2 \cdot \overline{K_{1,2}} \cdot CX_{0,1} \cdot \overline{K_{1,2}} \cdot \sigma_{1,2} \\
&\xrightarrow{C_{16}} \sigma_{1,2} \cdot \overline{K_{1,2} \cdot Z_2} \cdot CX_{0,1} \cdot K_{1,2} \cdot \sigma_{1,2} \\
&\xrightarrow{B_{30}} \sigma_{1,2} \cdot K_{1,2} \cdot \overline{CX_{0,1} \cdot Z_2} \cdot K_{1,2} \cdot \sigma_{1,2} \\
&\xleftarrow{C_{26}} \sigma_{1,2} \cdot K_{1,2} \cdot CX_{0,1} \cdot \overline{K_{1,2} \cdot X_2} \cdot \sigma_{1,2} \\
&\xrightarrow{S_{18}} \sigma_{1,2} \cdot K_{1,2} \cdot CX_{0,1} \cdot K_{1,2} \cdot \overline{\sigma_{1,2} \cdot X_1 \cdot \sigma_{1,2} \cdot \sigma_{1,2}} \\
&\xrightarrow{E_{10}} \sigma_{1,2} \cdot \overline{K_{1,2} \cdot CX_{0,1} \cdot K_{1,2}} \cdot \sigma_{1,2} \cdot X_1 \\
&\xleftarrow{(1)} \sigma_{1,2} \cdot \overline{CZ_{0,1} \cdot \sigma_{1,2}} \cdot X_1 \xleftarrow{(18)} \overline{CZ_{0,2}} \cdot X_1
\end{aligned}$$

$$\begin{aligned}
(B_{36}) : X_0 \cdot \underline{CZ_{1,2}} &\xrightarrow{(19)} X_0 \cdot \overline{\sigma_{0,1} \cdot CZ_{0,2} \cdot \sigma_{0,1}} \\
&\xleftarrow{E_4} \overline{\sigma_{0,1} \cdot \sigma_{0,1} \cdot X_0 \cdot \sigma_{0,1} \cdot CZ_{0,2} \cdot \sigma_{0,1}} \\
&\xleftarrow{(28)} \sigma_{0,1} \cdot \overline{X_1} \cdot \underline{CZ_{0,2}} \cdot \sigma_{0,1} \\
&\xrightarrow{B_{35}} \sigma_{0,1} \cdot \overline{CZ_{0,2} \cdot X_1} \cdot \sigma_{0,1} \\
&\xrightarrow{(28)} \sigma_{0,1} \cdot CZ_{0,2} \cdot \sigma_{0,1} \cdot \overline{X_0 \cdot \sigma_{0,1} \cdot \sigma_{0,1}} \\
&\xrightarrow{E_4} \underline{\sigma_{0,1} \cdot CZ_{0,2} \cdot \sigma_{0,1}} \cdot X_0 \xleftarrow{(19)} \overline{CZ_{1,2}} \cdot X_0
\end{aligned}$$

$$\begin{aligned}
(B_{37}) : X_2 \cdot \underline{CZ_{0,1}} &\xrightarrow{(1)} X_2 \cdot \overline{K_{1,2} \cdot CX_{0,1} \cdot K_{1,2}} \\
&\xrightarrow{C_{16}} \overline{K_{1,2} \cdot \underline{Z_2} \cdot CX_{0,1}} \cdot K_{1,2} \\
&\xrightarrow{B_{30}} K_{1,2} \cdot \overline{CX_{0,1} \cdot \underline{Z_2} \cdot K_{1,2}} \\
&\xleftarrow{C_{26}} \underline{K_{1,2} \cdot CX_{0,1} \cdot \overline{K_{1,2} \cdot X_2}} \\
&\xleftarrow{(1)} \overline{CZ_{0,1}} \cdot X_2
\end{aligned}$$

$$\begin{aligned}
(C_{31}) : Z_2 \cdot CX_{1,2} &\xleftarrow{(23)} \overline{K_{1,2} \cdot \underline{K_{1,2}} \cdot Z_2} \cdot CX_{1,2} \\
&\xleftarrow{C_{16}} K_{1,2} \cdot \overline{X_2 \cdot \underline{K_{1,2}}} \cdot CX_{1,2} \\
&\xleftarrow{C_{10}} K_{1,2} \cdot \underline{X_2 \cdot \overline{CX_{2,1}}} \cdot K_{1,2} \\
&\xrightarrow{C_{12}} K_{1,2} \cdot \overline{CX_{2,1} \cdot X_1 \cdot X_2} \cdot K_{1,2} \\
&\xrightarrow{B_{19}} K_{1,2} \cdot CX_{2,1} \cdot \overline{X_2 \cdot X_1} \cdot K_{1,2} \\
&\xrightarrow{C_4} \overline{CX_{1,2} \cdot \underline{K_{1,2}}} \cdot X_2 \cdot X_1 \cdot K_{1,2} \\
&\xrightarrow{C_{26}} CX_{1,2} \cdot \underline{Z_2 \cdot \overline{K_{1,2}}} \cdot X_1 \cdot K_{1,2} \\
&\xrightarrow{C_{27}} CX_{1,2} \cdot Z_2 \cdot \overline{Z_1 \cdot \underline{K_{1,2}}} \cdot K_{1,2} \\
&\xrightarrow{(23)} CX_{1,2} \cdot \underline{Z_2 \cdot Z_1} \xleftarrow{B_{34}} CX_{1,2} \cdot \overline{Z_1 \cdot Z_2}
\end{aligned}$$

$$\begin{aligned}
(C_{32}) : Z_0 \cdot CX_{1,0} &\xleftarrow{E_{16}} Z_0 \cdot CX_{1,0} \cdot \overline{\sigma_{0,2} \cdot \sigma_{0,2}} \\
&\xleftarrow{E_{16}} Z_0 \cdot \overline{\sigma_{0,2} \cdot \sigma_{0,2}} \cdot CX_{1,0} \cdot \sigma_{0,2} \cdot \sigma_{0,2} \\
&\xleftarrow{E_{16}} \overline{\sigma_{0,2} \cdot \sigma_{0,2} \cdot Z_0 \cdot \sigma_{0,2}} \cdot \sigma_{0,2} \cdot CX_{1,0} \cdot \sigma_{0,2} \cdot \sigma_{0,2} \\
&\xleftarrow{(16)} \sigma_{0,2} \cdot \underline{Z_2} \cdot \overline{\sigma_{0,2} \cdot CX_{1,0} \cdot \sigma_{0,2}} \cdot \sigma_{0,2} \\
&\xleftarrow{S_7} \sigma_{0,2} \cdot \underline{Z_2 \cdot \overline{CX_{1,2}}} \cdot \sigma_{0,2} \\
&\xrightarrow{C_{31}} \sigma_{0,2} \cdot \overline{CX_{1,2} \cdot Z_1 \cdot Z_2} \cdot \sigma_{0,2} \\
&\xleftarrow{E_{16}} \sigma_{0,2} \cdot CX_{1,2} \cdot Z_1 \cdot \overline{\sigma_{0,2} \cdot \sigma_{0,2}} \cdot Z_2 \cdot \sigma_{0,2} \\
&\xleftarrow{E_{16}} \sigma_{0,2} \cdot CX_{1,2} \cdot \overline{\sigma_{0,2} \cdot \sigma_{0,2}} \cdot Z_1 \cdot \underline{\sigma_{0,2} \cdot Z_2 \cdot \sigma_{0,2}} \\
&\xleftarrow{S_{26}} \sigma_{0,2} \cdot CX_{1,2} \cdot \sigma_{0,2} \cdot \overline{Z_1 \cdot \sigma_{0,2} \cdot Z_2 \cdot \sigma_{0,2}} \\
&\xleftarrow{S_4} \underline{\sigma_{0,2} \cdot CX_{1,2} \cdot \sigma_{0,2}} \cdot Z_1 \cdot \overline{Z_0} \\
&\xleftarrow{S_{11}} \overline{CX_{1,0} \cdot Z_1 \cdot Z_0}
\end{aligned}$$

$$\begin{aligned}
(C_{33}) : \underline{CX_{1,2}} \cdot CX_{0,2} &\xrightarrow{(30)} \overline{\sigma_{0,1} \cdot CX_{0,2} \cdot \sigma_{0,1}} \cdot CX_{0,2} \\
&\xleftarrow{E_4} \sigma_{0,1} \cdot CX_{0,2} \cdot \sigma_{0,1} \cdot \overline{CX_{0,2} \cdot \sigma_{0,1}} \\
&\xleftarrow{(30)} \sigma_{0,1} \cdot \underline{CX_{0,2}} \cdot \overline{CX_{1,2}} \cdot \sigma_{0,1} \\
&\xrightarrow{(9)} \sigma_{0,1} \cdot \overline{\sigma_{1,2} \cdot CX_{0,1} \cdot \sigma_{1,2}} \cdot \underline{CX_{1,2}} \cdot \sigma_{0,1} \\
&\xrightarrow{S_8} \sigma_{0,1} \cdot \sigma_{1,2} \cdot CX_{0,1} \cdot \overline{\sigma_{1,2} \cdot CX_{2,1} \cdot \sigma_{1,2} \cdot \sigma_{0,1}} \\
&\xrightarrow{E_{10}} \sigma_{0,1} \cdot \sigma_{1,2} \cdot \underline{CX_{0,1} \cdot CX_{2,1}} \cdot \sigma_{1,2} \cdot \sigma_{0,1} \\
&\xrightarrow{C_{20}} \sigma_{0,1} \cdot \sigma_{1,2} \cdot \overline{CX_{2,1} \cdot CX_{0,1}} \cdot \sigma_{1,2} \cdot \sigma_{0,1} \\
&\xleftarrow{E_{10}} \sigma_{0,1} \cdot \sigma_{1,2} \cdot CX_{2,1} \cdot \overline{\sigma_{1,2} \cdot CX_{0,1} \cdot \sigma_{1,2}} \cdot \sigma_{0,1} \\
&\xleftarrow{(9)} \sigma_{0,1} \cdot \sigma_{1,2} \cdot CX_{2,1} \cdot \sigma_{1,2} \cdot \overline{CX_{0,2}} \cdot \sigma_{0,1} \\
&\xleftarrow{S_8} \sigma_{0,1} \cdot \overline{CX_{1,2}} \cdot CX_{0,2} \cdot \sigma_{0,1} \\
&\xrightarrow{(30)} \underline{\sigma_{0,1} \cdot \overline{\sigma_{0,1} \cdot CX_{0,2} \cdot \sigma_{0,1}}} \cdot CX_{0,2} \cdot \sigma_{0,1} \\
&\xrightarrow{E_4} CX_{0,2} \cdot \underline{\sigma_{0,1} \cdot CX_{0,2} \cdot \sigma_{0,1}} \xleftarrow{(30)} CX_{0,2} \cdot \overline{CX_{1,2}}
\end{aligned}$$

$$\begin{aligned}
(C_{34}) : CX_{0,2} \cdot \underline{CCX_{0,2}} &\xrightarrow{(14)} CX_{0,2} \cdot \overline{\sigma_{0,1} \cdot CCX_{1,2} \cdot \sigma_{0,1}} \\
&\xleftarrow{E_4} \overline{\sigma_{0,1} \cdot \sigma_{0,1} \cdot CX_{0,2} \cdot \sigma_{0,1}} \cdot CCX_{1,2} \cdot \sigma_{0,1} \\
&\xleftarrow{(30)} \sigma_{0,1} \cdot \overline{CX_{1,2} \cdot CCX_{1,2}} \cdot \sigma_{0,1} \\
&\xrightarrow{(44)} \sigma_{0,1} \cdot \overline{CCX_{1,2} \cdot CX_{1,0} \cdot \underline{CX_{1,2}}} \cdot \sigma_{0,1} \\
&\xrightarrow{(30)} \sigma_{0,1} \cdot CCX_{1,2} \cdot CX_{1,0} \cdot \overline{\sigma_{0,1} \cdot CX_{0,2} \cdot \sigma_{0,1}} \cdot \sigma_{0,1} \\
&\xrightarrow{E_4} \sigma_{0,1} \cdot CCX_{1,2} \cdot CX_{1,0} \cdot \sigma_{0,1} \cdot CX_{0,2} \\
&\xleftarrow{E_4} \sigma_{0,1} \cdot CCX_{1,2} \cdot \overline{\sigma_{0,1} \cdot \sigma_{0,1} \cdot CX_{1,0} \cdot \sigma_{0,1}} \cdot CX_{0,2} \\
&\xleftarrow{S_1} \underline{\sigma_{0,1} \cdot CCX_{1,2} \cdot \sigma_{0,1} \cdot \overline{CX_{0,1}}} \cdot CX_{0,2} \\
&\xleftarrow{(14)} \overline{CCX_{0,2}} \cdot CX_{0,1} \cdot CX_{0,2}
\end{aligned}$$

$$\begin{aligned}
(C_{35}) : X_1 \cdot \overline{CCX_{0,1}} & \xrightarrow{(32)} \overline{X_1 \cdot \sigma_{0,2} \cdot \overline{CCX_{1,2}} \cdot \sigma_{0,2}} \\
& \xrightarrow{B_5} \overline{\sigma_{0,2} \cdot \overline{X_1} \cdot \overline{CCX_{1,2}} \cdot \sigma_{0,2}} \\
& \xrightarrow{C_8} \overline{\sigma_{0,2} \cdot \overline{CCX_{1,2}} \cdot \overline{CX_{2,0}} \cdot \overline{X_1} \cdot \sigma_{0,2}} \\
& \xrightarrow{B_5} \overline{\sigma_{0,2} \cdot \overline{CCX_{1,2}} \cdot \overline{CX_{2,0}} \cdot \overline{\sigma_{0,2}} \cdot \overline{X_1}} \\
& \xrightarrow{(29)} \overline{\sigma_{0,2} \cdot \overline{CCX_{1,2}} \cdot \overline{\sigma_{0,2}} \cdot \overline{CX_{0,2}} \cdot \overline{\sigma_{0,2}} \cdot \overline{\sigma_{0,2}} \cdot X_1} \\
& \xrightarrow{E_{16}} \overline{\sigma_{0,2} \cdot \overline{CCX_{1,2}} \cdot \overline{\sigma_{0,2}} \cdot \overline{CX_{0,2}} \cdot X_1} \\
& \xleftarrow{(32)} \overline{CCX_{0,1}} \cdot \overline{CX_{0,2}} \cdot X_1
\end{aligned}$$

$$\begin{aligned}
(C_{37}) : X_1 \cdot \overline{CCX_{0,2}} & \xrightarrow{(14)} \overline{X_1 \cdot \overline{\sigma_{0,1}} \cdot \overline{CCX_{1,2}} \cdot \sigma_{0,1}} \\
& \xrightarrow{(28)} \overline{\sigma_{0,1} \cdot \overline{X_0} \cdot \overline{\sigma_{0,1}} \cdot \overline{\sigma_{0,1}} \cdot \overline{CCX_{1,2}} \cdot \sigma_{0,1}} \\
& \xrightarrow{E_4} \overline{\sigma_{0,1} \cdot \overline{X_0} \cdot \overline{CCX_{1,2}} \cdot \sigma_{0,1}} \\
& \xrightarrow{(37)} \overline{\sigma_{0,1} \cdot \overline{CCX_{1,2}} \cdot \overline{X_0} \cdot \sigma_{0,1}} \\
& \xleftarrow{E_4} \overline{\sigma_{0,1} \cdot \overline{CCX_{1,2}} \cdot \overline{\sigma_{0,1}} \cdot \overline{\sigma_{0,1}} \cdot X_0 \cdot \sigma_{0,1}} \\
& \xleftarrow{(14)} \overline{CCX_{0,2}} \cdot \overline{\sigma_{0,1}} \cdot \overline{X_0} \cdot \sigma_{0,1} \\
& \xleftarrow{(28)} \overline{CCX_{0,2}} \cdot \overline{X_1}
\end{aligned}$$

$$\begin{aligned}
(C_{39}) : X_2 \cdot \overline{CCX_{0,1}} & \xrightarrow{(32)} \overline{X_2 \cdot \overline{\sigma_{0,2}} \cdot \overline{CCX_{1,2}} \cdot \sigma_{0,2}} \\
& \xrightarrow{(15)} \overline{\sigma_{0,2} \cdot \overline{X_0} \cdot \overline{\sigma_{0,2}} \cdot \overline{\sigma_{0,2}} \cdot \overline{CCX_{1,2}} \cdot \sigma_{0,2}} \\
& \xrightarrow{E_{16}} \overline{\sigma_{0,2} \cdot \overline{X_0} \cdot \overline{CCX_{1,2}} \cdot \sigma_{0,2}} \\
& \xrightarrow{(37)} \overline{\sigma_{0,2} \cdot \overline{CCX_{1,2}} \cdot \overline{X_0} \cdot \sigma_{0,2}} \\
& \xleftarrow{E_{16}} \overline{\sigma_{0,2} \cdot \overline{CCX_{1,2}} \cdot \overline{\sigma_{0,2}} \cdot \overline{\sigma_{0,2}} \cdot X_0 \cdot \sigma_{0,2}} \\
& \xleftarrow{(32)} \overline{CCX_{0,1}} \cdot \overline{\sigma_{0,2}} \cdot \overline{X_0} \cdot \sigma_{0,2} \\
& \xleftarrow{(15)} \overline{CCX_{0,1}} \cdot \overline{X_2}
\end{aligned}$$

$$\begin{aligned}
(C_{41}) : K_{1,2} \cdot \overline{CZ_{0,1}} & \xrightarrow{(1)} \overline{K_{1,2} \cdot \overline{K_{1,2}} \cdot \overline{CX_{0,1}} \cdot \overline{K_{1,2}}} \\
& \xrightarrow{(23)} \overline{CX_{0,1}} \cdot K_{1,2}
\end{aligned}$$

$$\begin{aligned}
(C_{36}) : K_{0,1} \cdot \overline{CCX_{1,2}} & \xrightarrow{(11)} \overline{\sigma_{0,2} \cdot \overline{K_{1,2}} \cdot \overline{\sigma_{0,2}} \cdot \overline{CCX_{1,2}}} \\
& \xleftarrow{E_{16}} \overline{\sigma_{0,2} \cdot K_{1,2} \cdot \overline{\sigma_{0,2}} \cdot \overline{CCX_{1,2}} \cdot \overline{\sigma_{0,2}} \cdot \overline{\sigma_{0,2}}} \\
& \xleftarrow{(32)} \overline{\sigma_{0,2} \cdot K_{1,2} \cdot \overline{CCX_{0,1}} \cdot \sigma_{0,2}} \\
& \xrightarrow{C_1} \overline{\sigma_{0,2} \cdot \overline{CCX_{0,2}} \cdot \overline{K_{1,2}} \cdot \sigma_{0,2}} \\
& \xleftarrow{E_{16}} \overline{\sigma_{0,2} \cdot \overline{CCX_{0,2}} \cdot \overline{\sigma_{0,2}} \cdot \overline{\sigma_{0,2}} \cdot K_{1,2} \cdot \sigma_{0,2}} \\
& \xleftarrow{(11)} \overline{\sigma_{0,2} \cdot \overline{CCX_{0,2}} \cdot \overline{\sigma_{0,2}} \cdot \overline{K_{0,1}}} \\
& \xleftarrow{S_{19}} \overline{CCX_{0,2}} \cdot K_{0,1}
\end{aligned}$$

$$\begin{aligned}
(C_{38}) : \overline{CCX_{0,1}} \cdot K_{1,2} & \xleftarrow{E_7} \overline{CCX_{0,1} \cdot K_{1,2} \cdot \overline{CCX_{0,2}} \cdot \overline{CCX_{0,2}}} \\
& \xleftarrow{(23)} \overline{CCX_{0,1} \cdot K_{1,2} \cdot \overline{CCX_{0,2}} \cdot \overline{K_{1,2}} \cdot \overline{K_{1,2}} \cdot \overline{CCX_{0,2}}} \\
& \xleftarrow{C_1} \overline{CCX_{0,1} \cdot K_{1,2} \cdot \overline{K_{1,2}} \cdot \overline{CCX_{0,1}} \cdot K_{1,2} \cdot \overline{CCX_{0,2}}} \\
& \xrightarrow{(23)} \overline{CCX_{0,1} \cdot \overline{CCX_{0,1}} \cdot K_{1,2} \cdot \overline{CCX_{0,2}}} \\
& \xrightarrow{E_{18}} K_{1,2} \cdot \overline{CCX_{0,2}}
\end{aligned}$$

$$\begin{aligned}
(C_{40}) : Z_1 \cdot \overline{CCX_{0,2}} & \xleftarrow{(23)} \overline{K_{1,2} \cdot \overline{K_{1,2}} \cdot Z_1 \cdot \overline{CCX_{0,2}}} \\
& \xleftarrow{C_2} \overline{K_{1,2} \cdot \overline{X_1} \cdot \overline{K_{1,2}} \cdot \overline{CCX_{0,2}}} \\
& \xleftarrow{C_{38}} \overline{K_{1,2} \cdot \overline{X_1} \cdot \overline{CCX_{0,1}} \cdot \overline{K_{1,2}}} \\
& \xrightarrow{C_{35}} \overline{K_{1,2} \cdot \overline{CCX_{0,1}} \cdot \overline{CX_{0,2}} \cdot \overline{X_1} \cdot K_{1,2}} \\
& \xleftarrow{C_2} \overline{K_{1,2} \cdot \overline{CCX_{0,1}} \cdot \overline{CX_{0,2}} \cdot \overline{K_{1,2}} \cdot Z_1} \\
& \xleftarrow{C_{28}} \overline{K_{1,2} \cdot \overline{CCX_{0,1}} \cdot \overline{K_{1,2}} \cdot \overline{CZ_{0,2}} \cdot Z_1} \\
& \xrightarrow{C_{38}} \overline{K_{1,2} \cdot \overline{K_{1,2}} \cdot \overline{CCX_{0,2}} \cdot \overline{CZ_{0,2}} \cdot Z_1} \\
& \xrightarrow{(23)} \overline{CCX_{0,2}} \cdot \overline{CZ_{0,2}} \cdot Z_1
\end{aligned}$$

$$\begin{aligned}
(C_{42}) : \overline{CCX_{1,2}} \cdot K_{0,1} & \xleftarrow{(25)} \overline{K_{0,1} \cdot \overline{K_{0,1}} \cdot \overline{CCX_{1,2}} \cdot K_{0,1}} \\
& \xrightarrow{C_{36}} \overline{K_{0,1} \cdot \overline{CCX_{0,2}} \cdot \overline{K_{0,1}} \cdot K_{0,1}} \\
& \xrightarrow{(25)} \overline{K_{0,1} \cdot \overline{CCX_{0,2}}}
\end{aligned}$$

$$\begin{aligned}
(C_{43}) : CX_{0,1} \cdot CZ_{0,1} &\stackrel{(22)}{\longleftarrow} CX_{0,1} \cdot CZ_{0,1} \cdot \overline{CX_{0,1} \cdot CX_{0,1}} \\
&\stackrel{E_2}{\longleftarrow} \overline{CZ_{0,1} \cdot CX_{0,1}} \cdot CX_{0,1} \cdot CZ_{0,1} \cdot CX_{0,1} \cdot CX_{0,1} \\
&\stackrel{(3)}{\longleftarrow} CZ_{0,1} \cdot \overline{Z_0} \cdot CX_{0,1}
\end{aligned}$$

$$\begin{aligned}
(C_{44}) : K_{1,2} \cdot CCX_{0,1} &\stackrel{(23)}{\longleftarrow} K_{1,2} \cdot \overline{CCX_{0,1} \cdot \overline{K_{1,2} \cdot K_{1,2}}} \\
&\stackrel{C_{38}}{\longrightarrow} \overline{K_{1,2} \cdot \overline{K_{1,2}}} \cdot \overline{CCX_{0,2} \cdot K_{1,2}} \\
&\stackrel{(23)}{\longrightarrow} CCX_{0,2} \cdot K_{1,2}
\end{aligned}$$

$$\begin{aligned}
(C_{45}) : CX_{2,1} \cdot CX_{0,1} \cdot CX_{0,2} \\
&\stackrel{E_{15}}{\longleftarrow} \overline{CX_{0,2} \cdot CX_{0,2} \cdot CX_{2,1} \cdot CX_{0,1} \cdot CX_{0,2}} \\
&\stackrel{C_{19}}{\longleftarrow} CX_{0,2} \cdot \overline{CX_{2,1} \cdot CX_{0,2}} \cdot CX_{0,2} \\
&\stackrel{E_{15}}{\longrightarrow} CX_{0,2} \cdot CX_{2,1}
\end{aligned}$$

$$\begin{aligned}
(C_{46}) : CZ_{0,1} \cdot K_{1,2} &\stackrel{(22)}{\longleftarrow} CZ_{0,1} \cdot K_{1,2} \cdot \overline{CX_{0,1} \cdot CX_{0,1}} \\
&\stackrel{(23)}{\longleftarrow} CZ_{0,1} \cdot K_{1,2} \cdot \overline{CX_{0,1} \cdot \overline{K_{1,2} \cdot K_{1,2}}} \cdot CX_{0,1} \\
&\stackrel{C_{41}}{\longleftarrow} CZ_{0,1} \cdot \overline{K_{1,2} \cdot \overline{K_{1,2}}} \cdot \overline{CZ_{0,1} \cdot K_{1,2} \cdot CX_{0,1}} \\
&\stackrel{(23)}{\longrightarrow} \overline{CZ_{0,1} \cdot CZ_{0,1}} \cdot K_{1,2} \cdot CX_{0,1} \\
&\stackrel{E_2}{\longrightarrow} K_{1,2} \cdot CX_{0,1}
\end{aligned}$$

$$\begin{aligned}
(C_{47}) : \underline{Z_1} \cdot CCX_{0,1} &\stackrel{(4)}{\longrightarrow} \overline{K_{1,2} \cdot X_1 \cdot \overline{K_{1,2} \cdot CCX_{0,1}}} \\
&\stackrel{C_{44}}{\longrightarrow} K_{1,2} \cdot X_1 \cdot \overline{CCX_{0,2} \cdot K_{1,2}} \\
&\stackrel{C_{37}}{\longrightarrow} \overline{K_{1,2} \cdot \overline{CCX_{0,2} \cdot X_1} \cdot K_{1,2}} \\
&\stackrel{C_{38}}{\longleftarrow} \overline{CCX_{0,1} \cdot \overline{K_{1,2} \cdot X_1 \cdot K_{1,2}}} \\
&\stackrel{(4)}{\longleftarrow} CCX_{0,1} \cdot \overline{Z_1}
\end{aligned}$$

$$\begin{aligned}
(C_{48}) : \underline{CX_{1,0}} \cdot Z_1 &\stackrel{(12)}{\longrightarrow} \overline{K_{0,1} \cdot \overline{CX_{0,1} \cdot K_{0,1}}} \cdot Z_1 \\
&\stackrel{C_{30}}{\longleftarrow} K_{0,1} \cdot \overline{CX_{0,1} \cdot \overline{X_1 \cdot K_{0,1}}} \\
&\stackrel{C_7}{\longleftarrow} \overline{K_{0,1} \cdot \overline{X_1 \cdot CX_{0,1} \cdot K_{0,1}}} \\
&\stackrel{C_{25}}{\longleftarrow} \overline{Z_1 \cdot \overline{K_{0,1} \cdot CX_{0,1} \cdot K_{0,1}}} \\
&\stackrel{(12)}{\longleftarrow} Z_1 \cdot \overline{CX_{1,0}}
\end{aligned}$$

$$\begin{aligned}
(C_{49}) : Z_0 \cdot CCX_{1,2} &\stackrel{E_4}{\longleftarrow} Z_0 \cdot CCX_{1,2} \cdot \overline{\sigma_{0,1} \cdot \sigma_{0,1}} \\
&\stackrel{E_4}{\longleftarrow} Z_0 \cdot \overline{\sigma_{0,1} \cdot \sigma_{0,1}} \cdot CCX_{1,2} \cdot \sigma_{0,1} \cdot \sigma_{0,1} \\
&\stackrel{E_4}{\longleftarrow} \overline{\sigma_{0,1} \cdot \sigma_{0,1} \cdot Z_0 \cdot \sigma_{0,1} \cdot \sigma_{0,1} \cdot CCX_{1,2} \cdot \sigma_{0,1} \cdot \sigma_{0,1}} \\
&\stackrel{(34)}{\longleftarrow} \sigma_{0,1} \cdot \overline{Z_1} \cdot \sigma_{0,1} \cdot \overline{CCX_{1,2} \cdot \sigma_{0,1} \cdot \sigma_{0,1}} \\
&\stackrel{(14)}{\longleftarrow} \sigma_{0,1} \cdot \overline{Z_1 \cdot \overline{CCX_{0,2} \cdot \sigma_{0,1}}} \\
&\stackrel{C_{40}}{\longrightarrow} \sigma_{0,1} \cdot \overline{CCX_{0,2} \cdot CZ_{0,2} \cdot \overline{Z_1} \cdot \sigma_{0,1}} \\
&\stackrel{(14)}{\longrightarrow} \overline{\sigma_{0,1} \cdot \sigma_{0,1} \cdot CCX_{1,2} \cdot \sigma_{0,1} \cdot CZ_{0,2} \cdot Z_1 \cdot \sigma_{0,1}} \\
&\stackrel{E_4}{\longrightarrow} CCX_{1,2} \cdot \sigma_{0,1} \cdot CZ_{0,2} \cdot \overline{Z_1} \cdot \sigma_{0,1} \\
&\stackrel{(34)}{\longrightarrow} CCX_{1,2} \cdot \sigma_{0,1} \cdot CZ_{0,2} \cdot \overline{\sigma_{0,1} \cdot Z_0 \cdot \sigma_{0,1} \cdot \sigma_{0,1}} \\
&\stackrel{E_4}{\longrightarrow} CCX_{1,2} \cdot \sigma_{0,1} \cdot CZ_{0,2} \cdot \sigma_{0,1} \cdot Z_0 \\
&\stackrel{(19)}{\longleftarrow} CCX_{1,2} \cdot \overline{CZ_{1,2}} \cdot Z_0
\end{aligned}$$

$$\begin{aligned}
(C_{50}) : Z_2 \cdot CCX_{1,2} &\stackrel{(25)}{\longleftarrow} \overline{K_{0,1} \cdot \overline{K_{0,1}}} \cdot Z_2 \cdot CCX_{1,2} \\
&\stackrel{B_{18}}{\longleftarrow} K_{0,1} \cdot \overline{Z_2 \cdot \overline{K_{0,1} \cdot CCX_{1,2}}} \\
&\stackrel{C_{36}}{\longrightarrow} K_{0,1} \cdot Z_2 \cdot \overline{CCX_{0,2} \cdot K_{0,1}} \\
&\stackrel{(23)}{\longleftarrow} K_{0,1} \cdot \overline{K_{1,2} \cdot \overline{K_{1,2}}} \cdot Z_2 \cdot CCX_{0,2} \cdot K_{0,1} \\
&\stackrel{C_{16}}{\longleftarrow} K_{0,1} \cdot K_{1,2} \cdot \overline{X_2 \cdot \overline{K_{1,2} \cdot CCX_{0,2} \cdot K_{0,1}}} \\
&\stackrel{C_{38}}{\longleftarrow} K_{0,1} \cdot K_{1,2} \cdot \overline{X_2 \cdot \overline{CCX_{0,1} \cdot K_{1,2} \cdot K_{0,1}}} \\
&\stackrel{C_{39}}{\longrightarrow} K_{0,1} \cdot K_{1,2} \cdot \overline{CCX_{0,1} \cdot \overline{X_2 \cdot K_{1,2} \cdot K_{0,1}}} \\
&\stackrel{C_{16}}{\longrightarrow} K_{0,1} \cdot K_{1,2} \cdot \overline{CCX_{0,1} \cdot \overline{K_{1,2} \cdot Z_2 \cdot K_{0,1}}} \\
&\stackrel{C_{38}}{\longrightarrow} K_{0,1} \cdot \overline{K_{1,2} \cdot \overline{K_{1,2}}} \cdot CCX_{0,2} \cdot Z_2 \cdot K_{0,1} \\
&\stackrel{(23)}{\longrightarrow} K_{0,1} \cdot CCX_{0,2} \cdot \overline{Z_2 \cdot K_{0,1}} \\
&\stackrel{B_{18}}{\longrightarrow} K_{0,1} \cdot \overline{CCX_{0,2} \cdot \overline{K_{0,1} \cdot Z_2}} \\
&\stackrel{C_{36}}{\longleftarrow} K_{0,1} \cdot \overline{K_{0,1} \cdot CCX_{1,2} \cdot Z_2} \\
&\stackrel{(25)}{\longrightarrow} CCX_{1,2} \cdot Z_2
\end{aligned}$$

$$\begin{aligned}
(C_{51}) : \underline{CX_{1,2}} \cdot CZ_{0,2} &\xrightarrow{(30)} \overline{\sigma_{0,1} \cdot \underline{CX_{0,2}} \cdot \sigma_{0,1}} \cdot CZ_{0,2} \xrightarrow{(9)} \sigma_{0,1} \cdot \overline{\sigma_{1,2} \cdot CX_{0,1} \cdot \sigma_{1,2}} \cdot \sigma_{0,1} \cdot \underline{CZ_{0,2}} \\
&\xrightarrow{S_2} \sigma_{0,1} \cdot \sigma_{1,2} \cdot CX_{0,1} \cdot \sigma_{1,2} \cdot \sigma_{0,1} \cdot \overline{\sigma_{0,1} \cdot \underline{CZ_{1,2}} \cdot \sigma_{0,1}} \\
&\xrightarrow{S_{21}} \sigma_{0,1} \cdot \sigma_{1,2} \cdot CX_{0,1} \cdot \sigma_{1,2} \cdot \overline{\sigma_{0,1} \cdot \sigma_{0,1} \cdot \sigma_{1,2} \cdot \underline{CZ_{1,2}} \cdot \sigma_{1,2}} \cdot \sigma_{0,1} \\
&\xrightarrow{E_4} \sigma_{0,1} \cdot \sigma_{1,2} \cdot CX_{0,1} \cdot \overline{\sigma_{1,2} \cdot \sigma_{1,2}} \cdot CZ_{1,2} \cdot \sigma_{1,2} \cdot \sigma_{0,1} \\
&\xrightarrow{E_{10}} \sigma_{0,1} \cdot \sigma_{1,2} \cdot \underline{CX_{0,1}} \cdot \underline{CZ_{1,2}} \cdot \sigma_{1,2} \cdot \sigma_{0,1} \\
&\xrightarrow{(43)} \sigma_{0,1} \cdot \sigma_{1,2} \cdot \overline{\underline{CZ_{1,2}} \cdot \underline{CZ_{0,2}} \cdot CX_{0,1}} \cdot \sigma_{1,2} \cdot \sigma_{0,1} \\
&\xrightarrow{(18)} \sigma_{0,1} \cdot \sigma_{1,2} \cdot CZ_{1,2} \cdot \overline{\sigma_{1,2} \cdot \underline{CZ_{0,1}} \cdot \sigma_{1,2}} \cdot \underline{CX_{0,1} \cdot \sigma_{1,2}} \cdot \sigma_{0,1} \\
&\xleftarrow{(9)} \sigma_{0,1} \cdot \overline{\sigma_{1,2} \cdot \underline{CZ_{1,2}} \cdot \sigma_{1,2}} \cdot CZ_{0,1} \cdot \overline{CX_{0,2}} \cdot \sigma_{0,1} \\
&\xleftarrow{S_{21}} \sigma_{0,1} \cdot \overline{\underline{CZ_{1,2}} \cdot \underline{CZ_{0,1}}} \cdot CX_{0,2} \cdot \sigma_{0,1} \\
&\xrightarrow{S_{24}} \sigma_{0,1} \cdot CZ_{1,2} \cdot \overline{\sigma_{0,1} \cdot \underline{CZ_{0,1}} \cdot \sigma_{0,1}} \cdot \underline{CX_{0,2}} \cdot \sigma_{0,1} \\
&\xleftarrow{(30)} \sigma_{0,1} \cdot \underline{CZ_{1,2}} \cdot \sigma_{0,1} \cdot CZ_{0,1} \cdot \overline{CX_{1,2}} \\
&\xleftarrow{S_2} \overline{CZ_{0,2}} \cdot CZ_{0,1} \cdot CX_{1,2}
\end{aligned}$$

$$\begin{aligned}
(C_{52}) : \underline{CX_{2,0}} \cdot CZ_{0,1} &\xrightarrow{(29)} \overline{\sigma_{0,2} \cdot \underline{CX_{0,2}} \cdot \sigma_{0,2}} \cdot CZ_{0,1} \\
&\xrightarrow{(9)} \sigma_{0,2} \cdot \overline{\sigma_{1,2} \cdot \underline{CX_{0,1}} \cdot \sigma_{1,2}} \cdot \sigma_{0,2} \cdot CZ_{0,1} \\
&\xleftarrow{E_{16}} \sigma_{0,2} \cdot \sigma_{1,2} \cdot CX_{0,1} \cdot \sigma_{1,2} \cdot \sigma_{0,2} \cdot \underline{CZ_{0,1} \cdot \sigma_{0,2} \cdot \sigma_{0,2}} \\
&\xleftarrow{E_{10}} \sigma_{0,2} \cdot \sigma_{1,2} \cdot CX_{0,1} \cdot \sigma_{1,2} \cdot \overline{\sigma_{0,2} \cdot \underline{CZ_{0,1}} \cdot \sigma_{0,2}} \cdot \overline{\sigma_{1,2} \cdot \sigma_{1,2}} \cdot \sigma_{0,2} \\
&\xleftarrow{S_{25}} \sigma_{0,2} \cdot \sigma_{1,2} \cdot CX_{0,1} \cdot \overline{\sigma_{1,2} \cdot \underline{CZ_{1,2}} \cdot \sigma_{1,2}} \cdot \sigma_{1,2} \cdot \sigma_{0,2} \\
&\xleftarrow{S_{21}} \sigma_{0,2} \cdot \sigma_{1,2} \cdot \underline{CX_{0,1}} \cdot \overline{\underline{CZ_{1,2}}} \cdot \sigma_{1,2} \cdot \sigma_{0,2} \\
&\xrightarrow{(43)} \sigma_{0,2} \cdot \sigma_{1,2} \cdot \overline{\underline{CZ_{1,2}} \cdot \underline{CZ_{0,2}} \cdot CX_{0,1}} \cdot \sigma_{1,2} \cdot \sigma_{0,2} \\
&\xrightarrow{(18)} \sigma_{0,2} \cdot \sigma_{1,2} \cdot CZ_{1,2} \cdot \overline{\sigma_{1,2} \cdot \underline{CZ_{0,1}} \cdot \sigma_{1,2}} \cdot \underline{CX_{0,1} \cdot \sigma_{1,2}} \cdot \sigma_{0,2} \\
&\xleftarrow{(9)} \sigma_{0,2} \cdot \overline{\sigma_{1,2} \cdot \underline{CZ_{1,2}} \cdot \sigma_{1,2}} \cdot CZ_{0,1} \cdot \overline{CX_{0,2}} \cdot \sigma_{0,2} \\
&\xleftarrow{S_{21}} \sigma_{0,2} \cdot \overline{\underline{CZ_{1,2}}} \cdot CZ_{0,1} \cdot CX_{0,2} \cdot \sigma_{0,2} \\
&\xleftarrow{E_{16}} \sigma_{0,2} \cdot CZ_{1,2} \cdot CZ_{0,1} \cdot \overline{\sigma_{0,2} \cdot \sigma_{0,2}} \cdot \underline{CX_{0,2}} \cdot \sigma_{0,2} \\
&\xleftarrow{(29)} \sigma_{0,2} \cdot \underline{CZ_{1,2}} \cdot CZ_{0,1} \cdot \sigma_{0,2} \cdot \overline{CX_{2,0}} \\
&\xrightarrow{S_{25}} \overline{\sigma_{0,2} \cdot \sigma_{0,2}} \cdot \underline{CZ_{0,1} \cdot \sigma_{0,2}} \cdot CZ_{0,1} \cdot \sigma_{0,2} \cdot CX_{2,0} \\
&\xrightarrow{E_{16}} CZ_{0,1} \cdot \overline{\sigma_{0,2} \cdot \underline{CZ_{0,1}} \cdot \sigma_{0,2}} \cdot CX_{2,0} \\
&\xleftarrow{S_{25}} CZ_{0,1} \cdot \overline{\underline{CZ_{1,2}}} \cdot CX_{2,0}
\end{aligned}$$

$$\begin{aligned}
(C_{53}) : X_0 \cdot CZ_{0,1} &\xleftarrow{(23)} \underline{X_0 \cdot \overline{K_{1,2}} \cdot K_{1,2}} \cdot CZ_{0,1} \\
&\xrightarrow{(27)} \overline{K_{1,2} \cdot X_0} \cdot \underline{K_{1,2} \cdot CZ_{0,1}} \\
&\xrightarrow{C_{41}} K_{1,2} \cdot \underline{X_0 \cdot \overline{CX_{0,1}}} \cdot K_{1,2} \\
&\xrightarrow{C_3} K_{1,2} \cdot \overline{CX_{0,1} \cdot X_1 \cdot X_0} \cdot K_{1,2} \\
&\xleftarrow{B_2} K_{1,2} \cdot CX_{0,1} \cdot \overline{X_0 \cdot X_1} \cdot K_{1,2} \\
&\xrightarrow{B_2} K_{1,2} \cdot CX_{0,1} \cdot \overline{X_1 \cdot X_0} \cdot K_{1,2} \\
&\xrightarrow{(27)} K_{1,2} \cdot CX_{0,1} \cdot X_1 \cdot \overline{K_{1,2} \cdot X_0} \\
&\xleftarrow{(23)} K_{1,2} \cdot CX_{0,1} \cdot \overline{K_{1,2} \cdot K_{1,2}} \cdot X_1 \cdot K_{1,2} \cdot X_0 \\
&\xleftarrow{(4)} K_{1,2} \cdot CX_{0,1} \cdot K_{1,2} \cdot \overline{Z_1} \cdot X_0 \\
&\xleftarrow{(1)} \overline{CZ_{0,1}} \cdot Z_1 \cdot X_0
\end{aligned}$$

$$\begin{aligned}
(C_{54}) : Z_0 \cdot \overline{CCX_{0,1}} &\xrightarrow{S_{17}} Z_0 \cdot \overline{\sigma_{0,1} \cdot \overline{CCX_{0,1}} \cdot \sigma_{0,1}} \\
&\xleftarrow{E_4} \overline{\sigma_{0,1} \cdot \overline{\sigma_{0,1}} \cdot Z_0 \cdot \sigma_{0,1}} \cdot \overline{CCX_{0,1}} \cdot \sigma_{0,1} \\
&\xleftarrow{(34)} \sigma_{0,1} \cdot \overline{Z_1} \cdot \overline{CCX_{0,1}} \cdot \sigma_{0,1} \\
&\xrightarrow{C_{47}} \sigma_{0,1} \cdot \overline{CCX_{0,1}} \cdot \overline{Z_1} \cdot \sigma_{0,1} \\
&\xrightarrow{(34)} \sigma_{0,1} \cdot \overline{CCX_{0,1}} \cdot \overline{\sigma_{0,1} \cdot Z_0 \cdot \sigma_{0,1}} \cdot \sigma_{0,1} \\
&\xrightarrow{E_4} \sigma_{0,1} \cdot \overline{CCX_{0,1}} \cdot \sigma_{0,1} \cdot Z_0 \\
&\xleftarrow{S_{17}} \overline{CCX_{0,1}} \cdot Z_0
\end{aligned}
\qquad
\begin{aligned}
(C_{55}) : CZ_{0,1} \cdot Z_1 &\xleftarrow{(23)} \overline{K_{1,2} \cdot \overline{K_{1,2}} \cdot CZ_{0,1}} \cdot Z_1 \\
&\xrightarrow{C_{41}} K_{1,2} \cdot \overline{CX_{0,1}} \cdot \overline{K_{1,2}} \cdot Z_1 \\
&\xleftarrow{C_2} K_{1,2} \cdot \overline{CX_{0,1}} \cdot \overline{X_1} \cdot \overline{K_{1,2}} \\
&\xleftarrow{C_7} K_{1,2} \cdot \overline{X_1} \cdot \overline{CX_{0,1}} \cdot K_{1,2} \\
&\xrightarrow{C_{27}} \overline{Z_1} \cdot \overline{K_{1,2}} \cdot \overline{CX_{0,1}} \cdot K_{1,2} \\
&\xleftarrow{C_{46}} Z_1 \cdot \overline{CZ_{0,1}} \cdot \overline{K_{1,2}} \cdot K_{1,2} \\
&\xrightarrow{(23)} Z_1 \cdot CZ_{0,1}
\end{aligned}$$

$$\begin{aligned}
(C_{56}) : X_0 \cdot CX_{1,2} \cdot \overline{CCX_{0,1}} &\xleftarrow{(21)} X_0 \cdot CX_{1,2} \cdot \overline{CCX_{0,1}} \cdot \overline{X_0 \cdot X_0} \xrightarrow{E_{18}} X_0 \cdot CX_{1,2} \cdot \overline{CCX_{0,1}} \cdot \overline{X_0 \cdot \overline{CCX_{0,1}} \cdot \overline{CCX_{0,1}}} \cdot X_0 \\
&\xrightarrow{(42)} X_0 \cdot CX_{1,2} \cdot \overline{CCX_{0,1}} \cdot \overline{CX_{1,2} \cdot \overline{X_0} \cdot \overline{CCX_{0,1}}} \cdot X_0 \\
&\xrightarrow{E_{18}} X_0 \cdot \overline{CX_{1,2}} \cdot \overline{CX_{1,2}} \cdot X_0 \cdot \overline{CCX_{0,1}} \cdot X_0 \\
&\xrightarrow{E_8} \overline{X_0 \cdot X_0} \cdot \overline{CCX_{0,1}} \cdot X_0 \xrightarrow{(21)} \overline{CCX_{0,1}} \cdot X_0
\end{aligned}$$

$$\begin{aligned}
(C_{57}) : CCX_{1,2} \cdot Z_0 &\xleftarrow{(24)} \overline{CCX_{1,2} \cdot Z_0 \cdot \overline{CCX_{1,2}} \cdot \overline{CCX_{1,2}}} \\
&\xleftarrow{E_{12}} \overline{CCX_{1,2} \cdot Z_0 \cdot \overline{CCX_{1,2}} \cdot \overline{CZ_{1,2}} \cdot \overline{CZ_{1,2}}} \cdot \overline{CCX_{1,2}} \\
&\xleftarrow{E_3} \overline{CCX_{1,2} \cdot Z_0 \cdot \overline{CCX_{1,2}} \cdot \overline{CZ_{1,2}} \cdot \overline{Z_0 \cdot Z_0} \cdot \overline{CZ_{1,2}}} \cdot \overline{CCX_{1,2}} \\
&\xleftarrow{C_{49}} \overline{CCX_{1,2} \cdot Z_0 \cdot \overline{Z_0} \cdot \overline{CCX_{1,2}} \cdot Z_0 \cdot \overline{CZ_{1,2}}} \cdot \overline{CCX_{1,2}} \\
&\xrightarrow{E_3} \overline{CCX_{1,2} \cdot \overline{CCX_{1,2}} \cdot Z_0 \cdot \overline{CZ_{1,2}}} \cdot \overline{CCX_{1,2}} \\
&\xrightarrow{(24)} \overline{Z_0 \cdot \overline{CZ_{1,2}}} \cdot \overline{CCX_{1,2}}
\end{aligned}
\qquad
\begin{aligned}
(C_{58}) : Z_0 \cdot \overline{CCX_{0,2}} &\xleftarrow{(25)} \overline{K_{0,1} \cdot \overline{K_{0,1}} \cdot Z_0 \cdot \overline{CCX_{0,2}}} \\
&\xrightarrow{(41)} K_{0,1} \cdot \overline{X_0} \cdot \overline{K_{0,1}} \cdot \overline{CCX_{0,2}} \\
&\xleftarrow{C_{42}} K_{0,1} \cdot \overline{X_0} \cdot \overline{CCX_{1,2}} \cdot \overline{K_{0,1}} \\
&\xrightarrow{(37)} K_{0,1} \cdot \overline{CCX_{1,2}} \cdot \overline{X_0} \cdot K_{0,1} \\
&\xleftarrow{(41)} K_{0,1} \cdot \overline{CCX_{1,2}} \cdot \overline{K_{0,1}} \cdot \overline{Z_0} \\
&\xrightarrow{C_{42}} K_{0,1} \cdot \overline{K_{0,1}} \cdot \overline{CCX_{0,2}} \cdot Z_0 \\
&\xrightarrow{(25)} \overline{CCX_{0,2}} \cdot Z_0
\end{aligned}$$

$$\begin{aligned}
(C_{59}) : Z_1 \cdot \overline{CCX_{1,2}} &\xleftarrow{E_4} \overline{Z_1 \cdot \overline{CCX_{1,2}} \cdot \overline{\sigma_{0,1}} \cdot \overline{\sigma_{0,1}}} \\
&\xrightarrow{(34)} \overline{\sigma_{0,1} \cdot \overline{Z_0} \cdot \overline{\sigma_{0,1}} \cdot \overline{CCX_{1,2}} \cdot \sigma_{0,1}} \cdot \sigma_{0,1} \\
&\xleftarrow{(14)} \sigma_{0,1} \cdot \overline{Z_0} \cdot \overline{CCX_{0,2}} \cdot \sigma_{0,1} \\
&\xrightarrow{C_{58}} \sigma_{0,1} \cdot \overline{CCX_{0,2}} \cdot \overline{Z_0} \cdot \sigma_{0,1} \\
&\xrightarrow{(14)} \sigma_{0,1} \cdot \overline{\sigma_{0,1} \cdot \overline{CCX_{1,2}} \cdot \overline{\sigma_{0,1}} \cdot \overline{Z_0} \cdot \sigma_{0,1}} \\
&\xleftarrow{(34)} \overline{\sigma_{0,1} \cdot \sigma_{0,1} \cdot \overline{CCX_{1,2}} \cdot \overline{Z_1}} \\
&\xrightarrow{E_4} \overline{CCX_{1,2}} \cdot Z_1
\end{aligned}
\qquad
\begin{aligned}
(C_{60}) : CZ_{0,1} \cdot CZ_{0,2} &\xleftarrow{(23)} \overline{K_{1,2} \cdot \overline{K_{1,2}} \cdot CZ_{0,1}} \cdot CZ_{0,2} \\
&\xrightarrow{C_{41}} K_{1,2} \cdot \overline{CX_{0,1}} \cdot \overline{K_{1,2}} \cdot CZ_{0,2} \\
&\xrightarrow{C_{28}} K_{1,2} \cdot \overline{CX_{0,1}} \cdot \overline{CX_{0,2}} \cdot K_{1,2} \\
&\xrightarrow{C_{22}} K_{1,2} \cdot \overline{CX_{0,2}} \cdot \overline{CX_{0,1}} \cdot K_{1,2} \\
&\xleftarrow{C_{29}} \overline{CZ_{0,2}} \cdot \overline{K_{1,2}} \cdot \overline{CX_{0,1}} \cdot K_{1,2} \\
&\xleftarrow{C_{46}} \overline{CZ_{0,2}} \cdot \overline{CZ_{0,1}} \cdot \overline{K_{1,2}} \cdot K_{1,2} \\
&\xrightarrow{(23)} \overline{CZ_{0,2}} \cdot CZ_{0,1}
\end{aligned}$$

$$\begin{aligned}
(C_{61}) : \underline{CX}_{2,1} \cdot \underline{CCX}_{1,2} &\xrightarrow{S_5} \overline{\sigma_{1,2} \cdot \underline{CX}_{1,2} \cdot \sigma_{1,2} \cdot \underline{CCX}_{1,2}} \\
&\xleftarrow{E_{10}} \sigma_{1,2} \cdot \underline{CX}_{1,2} \cdot \underline{\sigma_{1,2} \cdot \underline{CCX}_{1,2} \cdot \overline{\sigma_{1,2} \cdot \sigma_{1,2}}} \\
&\xleftarrow{S_{20}} \sigma_{1,2} \cdot \underline{CX}_{1,2} \cdot \overline{\underline{CCX}_{1,2}} \cdot \sigma_{1,2} \\
&\xrightarrow{(44)} \sigma_{1,2} \cdot \overline{\underline{CCX}_{1,2} \cdot \underline{CX}_{1,0} \cdot \underline{CX}_{1,2} \cdot \sigma_{1,2}} \\
&\xleftarrow{E_{10}} \sigma_{1,2} \cdot \underline{CCX}_{1,2} \cdot \underline{CX}_{1,0} \cdot \overline{\sigma_{1,2} \cdot \sigma_{1,2} \cdot \underline{CX}_{1,2} \cdot \sigma_{1,2}} \\
&\xleftarrow{S_5} \sigma_{1,2} \cdot \underline{CCX}_{1,2} \cdot \underline{CX}_{1,0} \cdot \sigma_{1,2} \cdot \overline{\underline{CX}_{2,1}} \\
&\xleftarrow{E_{10}} \sigma_{1,2} \cdot \underline{CCX}_{1,2} \cdot \overline{\sigma_{1,2} \cdot \sigma_{1,2} \cdot \underline{CX}_{1,0} \cdot \sigma_{1,2} \cdot \underline{CX}_{2,1}} \\
&\xleftarrow{S_{14}} \sigma_{1,2} \cdot \underline{CCX}_{1,2} \cdot \underline{\sigma_{1,2} \cdot \overline{CX_{2,0}}} \cdot \underline{CX_{2,1}} \\
&\xleftarrow{S_{20}} \overline{\underline{CCX}_{1,2}} \cdot \underline{CX_{2,0}} \cdot \underline{CX_{2,1}}
\end{aligned}$$

$$\begin{aligned}
(C_{62}) : \underline{CZ}_{0,1} \cdot \underline{Z_1} \cdot \underline{CX}_{1,0} &\xrightarrow{(34)} \underline{CZ_{0,1}} \cdot \overline{\sigma_{0,1} \cdot \underline{Z_0} \cdot \sigma_{0,1}} \cdot \underline{CX_{1,0}} \\
&\xrightarrow{S_{24}} \overline{\sigma_{0,1} \cdot \underline{CZ_{0,1}} \cdot \underline{\sigma_{0,1} \cdot \sigma_{0,1}}} \cdot \underline{Z_0} \cdot \sigma_{0,1} \cdot \underline{CX_{1,0}} \\
&\xrightarrow{E_4} \sigma_{0,1} \cdot \underline{CZ_{0,1}} \cdot \underline{Z_0} \cdot \sigma_{0,1} \cdot \underline{CX_{1,0}} \\
&\xleftarrow{E_4} \sigma_{0,1} \cdot \underline{CZ_{0,1}} \cdot \underline{Z_0} \cdot \sigma_{0,1} \cdot \underline{CX_{1,0} \cdot \overline{\sigma_{0,1} \cdot \sigma_{0,1}}} \\
&\xleftarrow{S_1} \sigma_{0,1} \cdot \underline{CZ_{0,1}} \cdot \underline{Z_0} \cdot \overline{\underline{CX_{0,1}}} \cdot \sigma_{0,1} \\
&\xleftarrow{C_{43}} \sigma_{0,1} \cdot \overline{\underline{CX_{0,1}}} \cdot \underline{CZ_{0,1}} \cdot \sigma_{0,1} \\
&\xrightarrow{S_1} \sigma_{0,1} \cdot \overline{\sigma_{0,1} \cdot \underline{CX_{1,0}} \cdot \sigma_{0,1}} \cdot \underline{CZ_{0,1}} \cdot \sigma_{0,1} \\
&\xrightarrow{E_4} \underline{CX_{1,0}} \cdot \sigma_{0,1} \cdot \underline{CZ_{0,1}} \cdot \sigma_{0,1} \\
&\xleftarrow{S_{24}} \underline{CX_{1,0}} \cdot \overline{\underline{CZ_{0,1}}}
\end{aligned}$$

$$\begin{aligned}
(C_{63}) : \underline{CZ}_{0,2} \cdot \underline{Z_0} \cdot \underline{CX}_{0,2} &\xrightarrow{(9)} \underline{CZ_{0,2}} \cdot \underline{Z_0} \cdot \overline{\sigma_{1,2} \cdot \underline{CX_{0,1}} \cdot \sigma_{1,2}} \\
&\xrightarrow{(18)} \overline{\sigma_{1,2} \cdot \underline{CZ_{0,1}} \cdot \sigma_{1,2} \cdot \underline{Z_0} \cdot \sigma_{1,2} \cdot \underline{CX_{0,1}} \cdot \sigma_{1,2}} \\
&\xrightarrow{B_{12}} \sigma_{1,2} \cdot \underline{CZ_{0,1}} \cdot \underline{\sigma_{1,2} \cdot \overline{\sigma_{1,2} \cdot \underline{Z_0}}} \cdot \underline{CX_{0,1}} \cdot \sigma_{1,2} \\
&\xrightarrow{E_{10}} \sigma_{1,2} \cdot \underline{CZ_{0,1}} \cdot \underline{Z_0} \cdot \underline{CX_{0,1}} \cdot \sigma_{1,2} \\
&\xleftarrow{C_{43}} \sigma_{1,2} \cdot \overline{\underline{CX_{0,1}} \cdot \underline{CZ_{0,1}}} \cdot \sigma_{1,2} \\
&\xleftarrow{E_{10}} \sigma_{1,2} \cdot \underline{CX_{0,1}} \cdot \overline{\sigma_{1,2} \cdot \sigma_{1,2} \cdot \underline{CZ_{0,1}} \cdot \sigma_{1,2}} \\
&\xleftarrow{(18)} \overline{\sigma_{1,2} \cdot \underline{CX_{0,1}} \cdot \sigma_{1,2} \cdot \underline{CZ_{0,2}}} \\
&\xleftarrow{(9)} \overline{\underline{CX_{0,2}}} \cdot \underline{CZ_{0,2}}
\end{aligned}$$

$$\begin{aligned}
(C_{64}) : \underline{CZ}_{1,2} \cdot \underline{Z_1} \cdot \underline{CX}_{1,2} &\xrightarrow{(30)} \underline{CZ_{1,2}} \cdot \underline{Z_1} \cdot \overline{\sigma_{0,1} \cdot \underline{CX_{0,2}} \cdot \sigma_{0,1}} \\
&\xrightarrow{(34)} \underline{CZ_{1,2}} \cdot \overline{\sigma_{0,1} \cdot \underline{Z_0} \cdot \sigma_{0,1} \cdot \underline{\sigma_{0,1}}} \cdot \underline{CX_{0,2}} \cdot \sigma_{0,1} \\
&\xrightarrow{E_4} \underline{CZ_{1,2}} \cdot \sigma_{0,1} \cdot \underline{Z_0} \cdot \underline{CX_{0,2}} \cdot \sigma_{0,1} \\
&\xrightarrow{(19)} \overline{\sigma_{0,1} \cdot \underline{CZ_{0,2}} \cdot \underline{\sigma_{0,1} \cdot \sigma_{0,1}}} \cdot \underline{Z_0} \cdot \underline{CX_{0,2}} \cdot \sigma_{0,1} \\
&\xrightarrow{E_4} \sigma_{0,1} \cdot \underline{CZ_{0,2}} \cdot \underline{Z_0} \cdot \underline{CX_{0,2}} \cdot \sigma_{0,1} \\
&\xrightarrow{C_{63}} \sigma_{0,1} \cdot \overline{\underline{CX_{0,2}} \cdot \underline{CZ_{0,2}}} \cdot \sigma_{0,1} \\
&\xleftarrow{E_4} \sigma_{0,1} \cdot \underline{CX_{0,2}} \cdot \overline{\sigma_{0,1} \cdot \underline{\sigma_{0,1}}} \cdot \underline{CZ_{0,2}} \cdot \sigma_{0,1} \\
&\xleftarrow{(19)} \overline{\sigma_{0,1} \cdot \underline{CX_{0,2}} \cdot \sigma_{0,1} \cdot \underline{\overline{CZ_{1,2}}}} \\
&\xleftarrow{(30)} \overline{\underline{CX_{1,2}}} \cdot \underline{CZ_{1,2}}
\end{aligned}$$

$$\begin{aligned}
(C_{65}) : \underline{CX}_{0,2} \cdot \underline{X_2} &\xrightarrow{S_{18}} \underline{CX_{0,2}} \cdot \overline{\sigma_{1,2} \cdot \underline{X_1} \cdot \sigma_{1,2}} \\
&\xrightarrow{(9)} \overline{\sigma_{1,2} \cdot \underline{CX_{0,1}} \cdot \underline{\sigma_{1,2} \cdot \sigma_{1,2}}} \cdot \underline{X_1} \cdot \sigma_{1,2} \\
&\xrightarrow{E_{10}} \sigma_{1,2} \cdot \underline{CX_{0,1}} \cdot \underline{X_1} \cdot \sigma_{1,2} \\
&\xleftarrow{C_7} \sigma_{1,2} \cdot \overline{\underline{X_1} \cdot \underline{CX_{0,1}}} \cdot \sigma_{1,2} \\
&\xleftarrow{E_{10}} \sigma_{1,2} \cdot \underline{X_1} \cdot \overline{\sigma_{1,2} \cdot \underline{\sigma_{1,2} \cdot \underline{CX_{0,1}} \cdot \sigma_{1,2}}} \\
&\xleftarrow{(9)} \overline{\sigma_{1,2} \cdot \underline{X_1} \cdot \sigma_{1,2} \cdot \underline{CX_{0,2}}} \\
&\xleftarrow{S_{18}} \overline{\underline{X_2}} \cdot \underline{CX_{0,2}}
\end{aligned}$$

$$\begin{aligned}
(C_{66}) : \underline{CX}_{2,1} \cdot \underline{CZ}_{0,2} &\xrightarrow{(18)} \underline{CX_{2,1}} \cdot \overline{\sigma_{1,2} \cdot \underline{CZ_{0,1}} \cdot \sigma_{1,2}} \\
&\xrightarrow{S_5} \overline{\sigma_{1,2} \cdot \underline{CX_{1,2}} \cdot \underline{\sigma_{1,2} \cdot \sigma_{1,2}}} \cdot \underline{CZ_{0,1}} \cdot \sigma_{1,2} \\
&\xrightarrow{E_{10}} \sigma_{1,2} \cdot \underline{CX_{1,2}} \cdot \underline{CZ_{0,1}} \cdot \sigma_{1,2} \\
&\xrightarrow{C_{21}} \sigma_{1,2} \cdot \overline{\underline{CZ_{0,1}} \cdot \underline{CX_{1,2}}} \cdot \sigma_{1,2} \\
&\xleftarrow{E_{10}} \sigma_{1,2} \cdot \underline{CZ_{0,1}} \cdot \overline{\sigma_{1,2} \cdot \underline{\sigma_{1,2} \cdot \underline{CX_{1,2}} \cdot \sigma_{1,2}}} \\
&\xleftarrow{S_5} \overline{\sigma_{1,2} \cdot \underline{CZ_{0,1}} \cdot \sigma_{1,2} \cdot \underline{\overline{CX_{2,1}}}} \\
&\xleftarrow{(18)} \overline{\underline{CZ_{0,2}}} \cdot \underline{CX_{2,1}}
\end{aligned}$$

$$\begin{aligned}
(C_{67}) : CX_{2,1} \cdot \underline{CX_{2,0}} &\xrightarrow{(29)} \underline{CX_{2,1}} \cdot \overline{\sigma_{0,2} \cdot CX_{0,2} \cdot \sigma_{0,2}} \\
&\xrightarrow{S_9} \overline{\sigma_{0,2} \cdot CX_{0,1} \cdot \sigma_{0,2} \cdot CX_{0,2} \cdot \sigma_{0,2}} \\
&\xrightarrow{E_{16}} \sigma_{0,2} \cdot CX_{0,1} \cdot CX_{0,2} \cdot \sigma_{0,2} \\
&\xrightarrow{C_{22}} \sigma_{0,2} \cdot \overline{CX_{0,2} \cdot CX_{0,1}} \cdot \sigma_{0,2} \\
&\xleftarrow{E_{16}} \sigma_{0,2} \cdot CX_{0,2} \cdot \overline{\sigma_{0,2} \cdot \sigma_{0,2} \cdot CX_{0,1} \cdot \sigma_{0,2}} \\
&\xleftarrow{S_9} \overline{\sigma_{0,2} \cdot CX_{0,2} \cdot \sigma_{0,2} \cdot CX_{2,1}} \\
&\xleftarrow{(29)} \overline{CX_{2,0} \cdot CX_{2,1}}
\end{aligned}$$

$$\begin{aligned}
(C_{69}) : X_0 \cdot Z_1 \cdot CZ_{0,1} &\xleftarrow{(21)} X_0 \cdot Z_1 \cdot CZ_{0,1} \cdot \overline{X_0 \cdot X_0} \\
&\xleftarrow{E_2} X_0 \cdot Z_1 \cdot CZ_{0,1} \cdot \underline{X_0 \cdot \overline{CZ_{0,1} \cdot CZ_{0,1}}} \cdot X_0 \\
&\xrightarrow{C_{53}} X_0 \cdot Z_1 \cdot \underline{CZ_{0,1} \cdot \overline{CZ_{0,1} \cdot Z_1 \cdot X_0}} \cdot CZ_{0,1} \cdot X_0 \\
&\xrightarrow{E_2} X_0 \cdot Z_1 \cdot Z_1 \cdot X_0 \cdot CZ_{0,1} \cdot X_0 \\
&\xrightarrow{E_5} X_0 \cdot X_0 \cdot CZ_{0,1} \cdot X_0 \\
&\xrightarrow{(21)} CZ_{0,1} \cdot X_0
\end{aligned}$$

$$\begin{aligned}
(C_{71}) : CZ_{0,2} \cdot \underline{CZ_{1,2}} &\xrightarrow{S_{21}} \underline{CZ_{0,2}} \cdot \overline{\sigma_{1,2} \cdot CZ_{1,2} \cdot \sigma_{1,2}} \\
&\xrightarrow{(18)} \overline{\sigma_{1,2} \cdot CZ_{0,1} \cdot \sigma_{1,2} \cdot \sigma_{1,2} \cdot CZ_{1,2} \cdot \sigma_{1,2}} \\
&\xrightarrow{E_{10}} \sigma_{1,2} \cdot \underline{CZ_{0,1} \cdot CZ_{1,2}} \cdot \sigma_{1,2} \\
&\xrightarrow{(40)} \sigma_{1,2} \cdot \overline{CZ_{1,2} \cdot CZ_{0,1}} \cdot \sigma_{1,2} \\
&\xleftarrow{E_{10}} \underline{\sigma_{1,2} \cdot CZ_{1,2} \cdot \sigma_{1,2} \cdot \sigma_{1,2}} \cdot CZ_{0,1} \cdot \sigma_{1,2} \\
&\xleftarrow{S_{21}} \overline{CZ_{1,2} \cdot \sigma_{1,2} \cdot CZ_{0,1} \cdot \sigma_{1,2}} \\
&\xleftarrow{(18)} \underline{CZ_{1,2} \cdot \overline{CZ_{0,2}}}
\end{aligned}$$

$$\begin{aligned}
(C_{73}) : K_{0,1} \cdot \underline{CX_{2,0}} &\xrightarrow{(29)} \underline{K_{0,1}} \cdot \overline{\sigma_{0,2} \cdot CX_{0,2} \cdot \sigma_{0,2}} \\
&\xrightarrow{(11)} \overline{\sigma_{0,2} \cdot K_{1,2} \cdot \sigma_{0,2} \cdot \sigma_{0,2} \cdot CX_{0,2} \cdot \sigma_{0,2}} \\
&\xrightarrow{E_{16}} \sigma_{0,2} \cdot \underline{K_{1,2} \cdot CX_{0,2}} \cdot \sigma_{0,2} \\
&\xleftarrow{C_{29}} \sigma_{0,2} \cdot \overline{CZ_{0,2} \cdot K_{1,2}} \cdot \sigma_{0,2} \\
&\xleftarrow{E_{16}} \sigma_{0,2} \cdot CZ_{0,2} \cdot \overline{\sigma_{0,2} \cdot \sigma_{0,2} \cdot K_{1,2} \cdot \sigma_{0,2}} \\
&\xleftarrow{(11)} \overline{\sigma_{0,2} \cdot CZ_{0,2} \cdot \sigma_{0,2} \cdot K_{0,1}} \\
&\xleftarrow{S_{23}} \overline{CZ_{0,2} \cdot K_{0,1}}
\end{aligned}$$

$$\begin{aligned}
(C_{68}) : Z_1 \cdot \underline{CX_{0,1}} &\xrightarrow{S_1} \underline{Z_1} \cdot \overline{\sigma_{0,1} \cdot CX_{1,0} \cdot \sigma_{0,1}} \\
&\xrightarrow{(34)} \overline{\sigma_{0,1} \cdot Z_0 \cdot \sigma_{0,1} \cdot CX_{1,0} \cdot \sigma_{0,1}} \\
&\xrightarrow{E_4} \sigma_{0,1} \cdot Z_0 \cdot CX_{1,0} \cdot \sigma_{0,1} \\
&\xrightarrow{C_{32}} \sigma_{0,1} \cdot \overline{CX_{1,0} \cdot Z_1 \cdot Z_0} \cdot \sigma_{0,1} \\
&\xrightarrow{(34)} \sigma_{0,1} \cdot CX_{1,0} \cdot \overline{\sigma_{0,1} \cdot Z_0 \cdot \sigma_{0,1} \cdot Z_0 \cdot \sigma_{0,1}} \\
&\xleftarrow{(34)} \overline{\sigma_{0,1} \cdot CX_{1,0} \cdot \sigma_{0,1} \cdot Z_0 \cdot \overline{Z_1}} \\
&\xleftarrow{S_1} \overline{CX_{0,1} \cdot Z_0 \cdot Z_1}
\end{aligned}$$

$$\begin{aligned}
(C_{70}) : X_1 \cdot \underline{CZ_{0,1}} &\xrightarrow{S_{24}} \underline{X_1} \cdot \overline{\sigma_{0,1} \cdot CZ_{0,1} \cdot \sigma_{0,1}} \\
&\xrightarrow{(28)} \overline{\sigma_{0,1} \cdot X_0 \cdot \sigma_{0,1} \cdot \sigma_{0,1} \cdot CZ_{0,1} \cdot \sigma_{0,1}} \\
&\xrightarrow{E_4} \sigma_{0,1} \cdot \underline{X_0 \cdot CZ_{0,1}} \cdot \sigma_{0,1} \\
&\xrightarrow{C_{53}} \sigma_{0,1} \cdot \overline{CZ_{0,1} \cdot Z_1 \cdot X_0} \cdot \sigma_{0,1} \\
&\xrightarrow{(34)} \overline{\sigma_{0,1} \cdot CZ_{0,1} \cdot \sigma_{0,1} \cdot Z_0 \cdot \sigma_{0,1} \cdot X_0 \cdot \sigma_{0,1}} \\
&\xleftarrow{S_{24}} \overline{CZ_{0,1} \cdot Z_0 \cdot \sigma_{0,1} \cdot X_0 \cdot \sigma_{0,1}} \\
&\xleftarrow{(28)} \overline{CZ_{0,1} \cdot Z_0 \cdot \overline{X_1}}
\end{aligned}$$

$$\begin{aligned}
(C_{72}) : CX_{1,0} \cdot \underline{CCX_{0,1}} &\xrightarrow{(32)} CX_{1,0} \cdot \overline{\sigma_{0,2} \cdot CCX_{1,2} \cdot \sigma_{0,2}} \\
&\xleftarrow{E_{16}} \overline{\sigma_{0,2} \cdot \sigma_{0,2} \cdot CX_{1,0} \cdot \sigma_{0,2} \cdot CCX_{1,2} \cdot \sigma_{0,2}} \\
&\xleftarrow{S_7} \sigma_{0,2} \cdot \overline{CX_{1,2} \cdot CCX_{1,2}} \cdot \sigma_{0,2} \\
&\xrightarrow{(44)} \sigma_{0,2} \cdot \overline{CCX_{1,2} \cdot CX_{1,0} \cdot CX_{1,2}} \cdot \sigma_{0,2} \\
&\xrightarrow{S_{11}} \overline{\sigma_{0,2} \cdot CCX_{1,2} \cdot \sigma_{0,2} \cdot CX_{1,2} \cdot \sigma_{0,2} \cdot CX_{1,2} \cdot \sigma_{0,2}} \\
&\xleftarrow{(32)} \overline{CCX_{0,1} \cdot CX_{1,2} \cdot \sigma_{0,2} \cdot CX_{1,2} \cdot \sigma_{0,2}} \\
&\xleftarrow{S_{11}} \overline{CCX_{0,1} \cdot CX_{1,2} \cdot \overline{CX_{1,0}}}
\end{aligned}$$

$$\begin{aligned}
(C_{74}) : \underline{CZ_{1,2}} \cdot K_{0,1} &\xrightarrow{(19)} \overline{\sigma_{0,1} \cdot CZ_{0,2} \cdot \sigma_{0,1} \cdot K_{0,1}} \\
&\xrightarrow{(35)} \overline{\sigma_{0,1} \cdot CZ_{0,2} \cdot \sigma_{0,1} \cdot \sigma_{0,1} \cdot K_{0,1} \cdot \sigma_{0,1}} \\
&\xrightarrow{E_4} \sigma_{0,1} \cdot \underline{CZ_{0,2} \cdot K_{0,1}} \cdot \sigma_{0,1} \\
&\xleftarrow{C_{73}} \sigma_{0,1} \cdot \overline{K_{0,1} \cdot CX_{2,0}} \cdot \sigma_{0,1} \\
&\xrightarrow{(35)} \overline{\sigma_{0,1} \cdot \sigma_{0,1} \cdot K_{0,1} \cdot \sigma_{0,1} \cdot CX_{2,0} \cdot \sigma_{0,1}} \\
&\xrightarrow{E_4} K_{0,1} \cdot \sigma_{0,1} \cdot \underline{CX_{2,0}} \cdot \sigma_{0,1} \\
&\xrightarrow{S_6} K_{0,1} \cdot \sigma_{0,1} \cdot \overline{\sigma_{0,1} \cdot CX_{2,1} \cdot \sigma_{0,1} \cdot \sigma_{0,1}} \\
&\xrightarrow{E_4} K_{0,1} \cdot \sigma_{0,1} \cdot \sigma_{0,1} \cdot CX_{2,1} \xrightarrow{E_4} K_{0,1} \cdot CX_{2,1}
\end{aligned}$$

$$\begin{aligned}
(C_{75}) : CZ_{1,2} \cdot CX_{0,1} &\xleftarrow{E_{11}} \overline{CZ_{0,2} \cdot CZ_{0,2} \cdot CZ_{1,2} \cdot CX_{0,1}} \\
&\xrightarrow{C_{71}} CZ_{0,2} \cdot \overline{CZ_{1,2} \cdot CZ_{0,2} \cdot CX_{0,1}} \\
&\xleftarrow{(43)} \overline{CZ_{0,2} \cdot \overline{CX_{0,1}} \cdot CZ_{1,2}} \\
&\xleftarrow{C_{23}} \overline{CX_{0,1} \cdot CZ_{0,2} \cdot CZ_{1,2}} \\
(C_{76}) : CX_{0,1} \cdot Z_0 \cdot CZ_{0,1} &\xleftarrow{(22)} CX_{0,1} \cdot Z_0 \cdot CZ_{0,1} \cdot \overline{CX_{0,1} \cdot CX_{0,1}} \\
&\xleftarrow{E_2} CX_{0,1} \cdot Z_0 \cdot CZ_{0,1} \cdot \overline{CX_{0,1} \cdot CZ_{0,1} \cdot CZ_{0,1}} \cdot CX_{0,1} \\
&\xrightarrow{C_{43}} CX_{0,1} \cdot Z_0 \cdot \overline{CZ_{0,1} \cdot \overline{CZ_{0,1}} \cdot Z_0 \cdot CX_{0,1}} \cdot CZ_{0,1} \cdot CX_{0,1} \\
&\xrightarrow{E_2} CX_{0,1} \cdot \overline{Z_0 \cdot Z_0} \cdot CX_{0,1} \cdot CZ_{0,1} \cdot CX_{0,1} \\
&\xrightarrow{E_3} CX_{0,1} \cdot \overline{CX_{0,1}} \cdot CZ_{0,1} \cdot CX_{0,1} \\
&\xrightarrow{(22)} CZ_{0,1} \cdot CX_{0,1} \\
(C_{77}) : CZ_{0,1} \cdot CCX_{1,2} &\xleftarrow{(23)} \overline{K_{1,2} \cdot K_{1,2} \cdot CZ_{0,1} \cdot CCX_{1,2}} \\
&\xleftarrow{(25)} K_{1,2} \cdot \overline{K_{0,1} \cdot K_{0,1}} \cdot \overline{K_{1,2} \cdot CZ_{0,1}} \cdot CCX_{1,2} \\
&\xrightarrow{C_{41}} K_{1,2} \cdot K_{0,1} \cdot K_{0,1} \cdot \overline{CX_{0,1} \cdot K_{1,2}} \cdot CCX_{1,2} \\
&\xleftarrow{(25)} K_{1,2} \cdot K_{0,1} \cdot \overline{K_{0,1} \cdot CX_{0,1} \cdot K_{0,1} \cdot K_{1,2}} \cdot CCX_{1,2} \\
&\xleftarrow{(12)} K_{1,2} \cdot K_{0,1} \cdot \overline{CX_{1,0}} \cdot \overline{K_{0,1} \cdot K_{1,2}} \cdot CCX_{1,2} \\
&\xrightarrow{(39)} K_{1,2} \cdot K_{0,1} \cdot CX_{1,0} \cdot \overline{K_{1,2} \cdot K_{0,1}} \cdot CCX_{1,2} \\
&\xrightarrow{C_{36}} K_{1,2} \cdot K_{0,1} \cdot CX_{1,0} \cdot \overline{K_{1,2} \cdot \overline{CCX_{0,2}} \cdot K_{0,1}} \\
&\xleftarrow{C_{38}} K_{1,2} \cdot K_{0,1} \cdot \overline{CX_{1,0} \cdot \overline{CCX_{0,1}} \cdot K_{1,2}} \cdot K_{0,1} \\
&\xrightarrow{C_{72}} K_{1,2} \cdot K_{0,1} \cdot \overline{CCX_{0,1} \cdot CX_{1,2} \cdot CX_{1,0} \cdot K_{1,2} \cdot K_{0,1}} \\
&\xleftarrow{(39)} K_{1,2} \cdot K_{0,1} \cdot CCX_{0,1} \cdot CX_{1,2} \cdot \overline{CX_{1,0} \cdot K_{0,1} \cdot K_{1,2}} \\
&\xrightarrow{(12)} K_{1,2} \cdot K_{0,1} \cdot CCX_{0,1} \cdot CX_{1,2} \cdot \overline{K_{0,1} \cdot CX_{0,1} \cdot K_{0,1} \cdot K_{1,2}} \\
&\xrightarrow{(25)} K_{1,2} \cdot K_{0,1} \cdot CCX_{0,1} \cdot CX_{1,2} \cdot K_{0,1} \cdot CX_{0,1} \cdot K_{1,2} \\
&\xleftarrow{(23)} K_{1,2} \cdot K_{0,1} \cdot CCX_{0,1} \cdot CX_{1,2} \cdot K_{0,1} \cdot \overline{K_{1,2} \cdot K_{1,2}} \cdot CX_{0,1} \cdot K_{1,2} \\
&\xleftarrow{(1)} K_{1,2} \cdot \overline{K_{0,1} \cdot CCX_{0,1} \cdot CX_{1,2} \cdot K_{0,1} \cdot K_{1,2} \cdot \overline{CZ_{0,1}}} \\
&\xleftarrow{(39)} \overline{K_{0,1} \cdot K_{1,2} \cdot CCX_{0,1} \cdot CX_{1,2} \cdot K_{0,1} \cdot K_{1,2} \cdot CZ_{0,1}} \\
&\xrightarrow{C_{44}} K_{0,1} \cdot \overline{CCX_{0,2} \cdot K_{1,2} \cdot CX_{1,2} \cdot K_{0,1} \cdot K_{1,2}} \cdot CZ_{0,1} \\
&\xrightarrow{(39)} K_{0,1} \cdot \overline{CCX_{0,2} \cdot K_{1,2} \cdot CX_{1,2} \cdot K_{1,2} \cdot K_{0,1}} \cdot CZ_{0,1} \\
&\xleftarrow{C_{42}} \overline{CCX_{1,2} \cdot K_{0,1} \cdot K_{1,2} \cdot CX_{1,2} \cdot K_{1,2} \cdot K_{0,1}} \cdot CZ_{0,1} \\
&\xleftarrow{C_{10}} CCX_{1,2} \cdot K_{0,1} \cdot \overline{CX_{2,1} \cdot K_{1,2} \cdot K_{1,2} \cdot K_{0,1}} \cdot CZ_{0,1} \\
&\xrightarrow{(23)} CCX_{1,2} \cdot \overline{K_{0,1} \cdot CX_{2,1}} \cdot K_{0,1} \cdot CZ_{0,1} \\
&\xleftarrow{C_{74}} CCX_{1,2} \cdot \overline{CZ_{1,2} \cdot K_{0,1} \cdot K_{0,1}} \cdot CZ_{0,1} \\
&\xrightarrow{(25)} CCX_{1,2} \cdot CZ_{1,2} \cdot CZ_{0,1}
\end{aligned}$$

$$\begin{aligned}
(C_{78}) : CZ_{0,2} \cdot Z_2 &\stackrel{(23)}{\longleftarrow} \overline{K_{1,2} \cdot K_{1,2} \cdot CZ_{0,2} \cdot Z_2} \\
&\stackrel{C_{28}}{\longrightarrow} K_{1,2} \cdot \overline{CX_{0,2} \cdot K_{1,2} \cdot Z_2} \\
&\stackrel{C_{16}}{\longleftarrow} K_{1,2} \cdot \overline{CX_{0,2} \cdot X_2 \cdot K_{1,2}} \\
&\stackrel{C_{65}}{\longrightarrow} K_{1,2} \cdot \overline{X_2 \cdot CX_{0,2} \cdot K_{1,2}} \\
&\stackrel{C_{28}}{\longleftarrow} K_{1,2} \cdot \overline{X_2 \cdot K_{1,2} \cdot CZ_{0,2}} \\
&\stackrel{C_{16}}{\longrightarrow} K_{1,2} \cdot \overline{K_{1,2} \cdot Z_2 \cdot CZ_{0,2}} \\
&\stackrel{(23)}{\longrightarrow} Z_2 \cdot CZ_{0,2}
\end{aligned}$$

$$\begin{aligned}
(C_{79}) : X_0 \cdot X_1 \cdot CX_{0,1} &\stackrel{B_2}{\longrightarrow} \overline{X_1 \cdot X_0 \cdot CX_{0,1}} \\
&\stackrel{(22)}{\longleftarrow} \overline{CX_{0,1} \cdot CX_{0,1} \cdot X_1 \cdot X_0 \cdot CX_{0,1}} \\
&\stackrel{(21)}{\longleftarrow} CX_{0,1} \cdot \overline{X_0 \cdot X_0 \cdot CX_{0,1}} \cdot X_1 \cdot X_0 \cdot CX_{0,1} \\
&\stackrel{C_3}{\longrightarrow} CX_{0,1} \cdot X_0 \cdot \overline{CX_{0,1} \cdot X_1 \cdot X_0 \cdot CX_{0,1}} \\
&\stackrel{B_2}{\longleftarrow} CX_{0,1} \cdot X_0 \cdot CX_{0,1} \cdot \overline{X_0 \cdot X_1 \cdot X_1 \cdot X_0 \cdot CX_{0,1}} \\
&\stackrel{E_{13}}{\longrightarrow} CX_{0,1} \cdot X_0 \cdot CX_{0,1} \cdot \overline{X_0 \cdot X_0 \cdot CX_{0,1}} \\
&\stackrel{(21)}{\longrightarrow} CX_{0,1} \cdot X_0 \cdot \overline{CX_{0,1} \cdot CX_{0,1}} \\
&\stackrel{(22)}{\longrightarrow} CX_{0,1} \cdot X_0
\end{aligned}$$

$$\begin{aligned}
(C_{80}) : CZ_{0,1} \cdot \overline{CCX_{0,2}} &\stackrel{(14)}{\longrightarrow} \overline{CZ_{0,1} \cdot \overline{\sigma_{0,1} \cdot CCX_{1,2} \cdot \sigma_{0,1}}} \\
&\stackrel{S_{24}}{\longrightarrow} \overline{\sigma_{0,1} \cdot CZ_{0,1} \cdot \overline{\sigma_{0,1} \cdot \sigma_{0,1} \cdot CCX_{1,2} \cdot \sigma_{0,1}}} \\
&\stackrel{E_4}{\longrightarrow} \overline{\sigma_{0,1} \cdot CZ_{0,1} \cdot CCX_{1,2} \cdot \sigma_{0,1}} \\
&\stackrel{C_{77}}{\longrightarrow} \overline{\sigma_{0,1} \cdot \overline{CCX_{1,2} \cdot CZ_{1,2} \cdot CZ_{0,1} \cdot \sigma_{0,1}}} \\
&\stackrel{(19)}{\longrightarrow} \overline{\sigma_{0,1} \cdot CCX_{1,2} \cdot \overline{\sigma_{0,1} \cdot CZ_{0,2} \cdot \overline{\sigma_{0,1} \cdot CZ_{0,1} \cdot \sigma_{0,1}}}} \\
&\stackrel{S_{24}}{\longleftarrow} \overline{\sigma_{0,1} \cdot CCX_{1,2} \cdot \sigma_{0,1} \cdot CZ_{0,2} \cdot \overline{CZ_{0,1}}} \\
&\stackrel{(14)}{\longleftarrow} \overline{CCX_{0,2} \cdot CZ_{0,2} \cdot CZ_{0,1}} \\
&\stackrel{C_{60}}{\longleftarrow} \overline{CCX_{0,2} \cdot \overline{CZ_{0,1} \cdot CZ_{0,2}}}
\end{aligned}$$

$$\begin{aligned}
(C_{81}) : CZ_{0,2} \cdot \overline{CCX_{0,1}} &\stackrel{(33)}{\longrightarrow} \overline{CZ_{0,2} \cdot \overline{\sigma_{1,2} \cdot CCX_{0,2} \cdot \sigma_{1,2}}} \\
&\stackrel{(18)}{\longrightarrow} \overline{\sigma_{1,2} \cdot CZ_{0,1} \cdot \overline{\sigma_{1,2} \cdot \sigma_{1,2} \cdot CCX_{0,2} \cdot \sigma_{1,2}}} \\
&\stackrel{E_{10}}{\longrightarrow} \overline{\sigma_{1,2} \cdot CZ_{0,1} \cdot CCX_{0,2} \cdot \sigma_{1,2}} \\
&\stackrel{C_{80}}{\longrightarrow} \overline{\sigma_{1,2} \cdot \overline{CCX_{0,2} \cdot CZ_{0,1} \cdot CZ_{0,2} \cdot \sigma_{1,2}}} \\
&\stackrel{(18)}{\longrightarrow} \overline{\sigma_{1,2} \cdot CCX_{0,2} \cdot CZ_{0,1} \cdot \overline{\sigma_{1,2} \cdot CZ_{0,1} \cdot \overline{\sigma_{1,2} \cdot \sigma_{1,2}}}} \\
&\stackrel{E_{10}}{\longrightarrow} \overline{\sigma_{1,2} \cdot CCX_{0,2} \cdot CZ_{0,1} \cdot \sigma_{1,2} \cdot CZ_{0,1}} \\
&\stackrel{E_{10}}{\longleftarrow} \overline{\sigma_{1,2} \cdot CCX_{0,2} \cdot \overline{\sigma_{1,2} \cdot \overline{\sigma_{1,2} \cdot CZ_{0,1} \cdot \sigma_{1,2} \cdot CZ_{0,1}}}} \\
&\stackrel{(18)}{\longleftarrow} \overline{\sigma_{1,2} \cdot CCX_{0,2} \cdot \sigma_{1,2} \cdot \overline{CZ_{0,2} \cdot CZ_{0,1}}} \\
&\stackrel{(33)}{\longleftarrow} \overline{CCX_{0,1} \cdot CZ_{0,2} \cdot CZ_{0,1}} \\
&\stackrel{C_{60}}{\longleftarrow} \overline{CCX_{0,1} \cdot \overline{CZ_{0,1} \cdot CZ_{0,2}}}
\end{aligned}$$

$$\begin{aligned}
(C_{82}) : CZ_{1,2} \cdot \overline{CCX_{0,1}} &\stackrel{S_{17}}{\longrightarrow} \overline{CZ_{1,2} \cdot \overline{\sigma_{0,1} \cdot CCX_{0,1} \cdot \sigma_{0,1}}} \\
&\stackrel{(19)}{\longrightarrow} \overline{\sigma_{0,1} \cdot CZ_{0,2} \cdot \overline{\sigma_{0,1} \cdot \sigma_{0,1} \cdot CCX_{0,1} \cdot \sigma_{0,1}}} \\
&\stackrel{E_4}{\longrightarrow} \overline{\sigma_{0,1} \cdot CZ_{0,2} \cdot CCX_{0,1} \cdot \sigma_{0,1}} \\
&\stackrel{C_{81}}{\longrightarrow} \overline{\sigma_{0,1} \cdot \overline{CCX_{0,1} \cdot CZ_{0,1} \cdot CZ_{0,2} \cdot \sigma_{0,1}}} \\
&\stackrel{S_{24}}{\longrightarrow} \overline{\sigma_{0,1} \cdot CCX_{0,1} \cdot \overline{\sigma_{0,1} \cdot CZ_{0,1} \cdot \overline{\sigma_{0,1} \cdot CZ_{0,2} \cdot \sigma_{0,1}}}} \\
&\stackrel{(19)}{\longleftarrow} \overline{\sigma_{0,1} \cdot CCX_{0,1} \cdot \sigma_{0,1} \cdot CZ_{0,1} \cdot \overline{CZ_{1,2}}} \\
&\stackrel{S_{17}}{\longleftarrow} \overline{CCX_{0,1} \cdot CZ_{0,1} \cdot CZ_{1,2}}
\end{aligned}$$

$$\begin{aligned}
(C_{83}) : X_2 \cdot CCX_{1,2} &\stackrel{(15)}{\longrightarrow} \overline{\sigma_{0,2} \cdot X_0 \cdot \sigma_{0,2} \cdot CCX_{1,2}} \\
&\stackrel{E_{16}}{\longleftarrow} \overline{\sigma_{0,2} \cdot X_0 \cdot \sigma_{0,2} \cdot CCX_{1,2} \cdot \overline{\sigma_{0,2} \cdot \sigma_{0,2}}} \\
&\stackrel{(32)}{\longleftarrow} \overline{\sigma_{0,2} \cdot X_0 \cdot \overline{CCX_{0,1} \cdot \sigma_{0,2}}} \\
&\stackrel{(42)}{\longrightarrow} \overline{\sigma_{0,2} \cdot \overline{CCX_{0,1} \cdot CX_{1,2} \cdot X_0 \cdot \sigma_{0,2}}} \\
&\stackrel{(32)}{\longrightarrow} \overline{\sigma_{0,2} \cdot \overline{\sigma_{0,2} \cdot CCX_{1,2} \cdot \sigma_{0,2} \cdot CX_{1,2} \cdot X_0 \cdot \sigma_{0,2}}} \\
&\stackrel{E_{16}}{\longrightarrow} \overline{CCX_{1,2} \cdot \sigma_{0,2} \cdot CX_{1,2} \cdot X_0 \cdot \sigma_{0,2}} \\
&\stackrel{E_{16}}{\longleftarrow} \overline{CCX_{1,2} \cdot \sigma_{0,2} \cdot CX_{1,2} \cdot \overline{\sigma_{0,2} \cdot \overline{\sigma_{0,2} \cdot X_0 \cdot \sigma_{0,2}}}} \\
&\stackrel{(15)}{\longleftarrow} \overline{CCX_{1,2} \cdot \overline{\sigma_{0,2} \cdot CX_{1,2} \cdot \sigma_{0,2} \cdot X_2}} \\
&\stackrel{S_{11}}{\longleftarrow} \overline{CCX_{1,2} \cdot \overline{CX_{1,0} \cdot X_2}}
\end{aligned}$$

$$\begin{aligned}
(C_{84}) : CZ_{1,2} \cdot \underline{CX_{0,2}} &\xrightarrow{(9)} \underline{CZ_{1,2} \cdot \overline{\sigma_{1,2} \cdot CX_{0,1} \cdot \sigma_{1,2}}} \\
&\xrightarrow{S_{21}} \overline{\sigma_{1,2} \cdot CZ_{1,2} \cdot \sigma_{1,2} \cdot \sigma_{1,2}} \cdot CX_{0,1} \cdot \sigma_{1,2} \\
&\xrightarrow{E_{10}} \sigma_{1,2} \cdot \underline{CZ_{1,2} \cdot CX_{0,1} \cdot \sigma_{1,2}} \\
&\xrightarrow{C_{75}} \sigma_{1,2} \cdot \overline{CX_{0,1} \cdot CZ_{0,2} \cdot CZ_{1,2}} \cdot \sigma_{1,2} \\
&\xrightarrow{(18)} \sigma_{1,2} \cdot CX_{0,1} \cdot \overline{\sigma_{1,2} \cdot CZ_{0,1} \cdot \sigma_{1,2} \cdot CZ_{1,2} \cdot \sigma_{1,2}} \\
&\xleftarrow{S_{21}} \sigma_{1,2} \cdot CX_{0,1} \cdot \sigma_{1,2} \cdot CZ_{0,1} \cdot \overline{CZ_{1,2}} \\
&\xleftarrow{(9)} \overline{CX_{0,2} \cdot CZ_{0,1} \cdot CZ_{1,2}}
\end{aligned}$$

$$\begin{aligned}
(C_{86}) : \underline{X_1} \cdot CX_{2,1} &\xrightarrow{(2)} \overline{CX_{0,1} \cdot X_0 \cdot CX_{0,1} \cdot X_0 \cdot CX_{2,1}} \\
&\xleftarrow{B_1} CX_{0,1} \cdot X_0 \cdot \underline{CX_{0,1} \cdot \overline{CX_{2,1} \cdot X_0}} \\
&\xrightarrow{C_{20}} CX_{0,1} \cdot X_0 \cdot \overline{CX_{2,1} \cdot CX_{0,1} \cdot X_0} \\
&\xleftarrow{B_1} \underline{CX_{0,1} \cdot \overline{CX_{2,1} \cdot X_0}} \cdot CX_{0,1} \cdot X_0 \\
&\xrightarrow{C_{20}} \overline{CX_{2,1} \cdot CX_{0,1} \cdot X_0 \cdot CX_{0,1} \cdot X_0} \\
&\xleftarrow{(2)} CX_{2,1} \cdot \overline{X_1}
\end{aligned}$$

$$\begin{aligned}
(C_{88}) : CZ_{0,1} \cdot Z_0 &\xleftarrow{(23)} \overline{K_{1,2} \cdot \overline{K_{1,2}} \cdot CZ_{0,1} \cdot Z_0} \\
&\xrightarrow{C_{41}} K_{1,2} \cdot \overline{CX_{0,1} \cdot K_{1,2} \cdot Z_0} \\
&\xleftarrow{B_6} K_{1,2} \cdot \underline{CX_{0,1} \cdot \overline{Z_0 \cdot K_{1,2}}} \\
&\xrightarrow{C_{85}} \underline{K_{1,2} \cdot \overline{Z_0 \cdot CX_{0,1}}} \cdot K_{1,2} \\
&\xleftarrow{B_6} \overline{Z_0 \cdot K_{1,2}} \cdot CX_{0,1} \cdot K_{1,2} \\
&\xleftarrow{C_{46}} Z_0 \cdot \overline{CZ_{0,1} \cdot K_{1,2}} \cdot K_{1,2} \\
&\xrightarrow{(23)} Z_0 \cdot CZ_{0,1}
\end{aligned}$$

$$\begin{aligned}
(C_{90}) : \underline{CX_{0,2}} \cdot Z_0 &\xrightarrow{(9)} \overline{\sigma_{1,2} \cdot CX_{0,1} \cdot \sigma_{1,2} \cdot Z_0} \\
&\xleftarrow{B_{12}} \sigma_{1,2} \cdot \underline{CX_{0,1} \cdot \overline{Z_0 \cdot \sigma_{1,2}}} \\
&\xrightarrow{C_{85}} \sigma_{1,2} \cdot \overline{Z_0 \cdot CX_{0,1}} \cdot \sigma_{1,2} \\
&\xleftarrow{B_{12}} \overline{Z_0 \cdot \sigma_{1,2}} \cdot CX_{0,1} \cdot \sigma_{1,2} \\
&\xleftarrow{(9)} Z_0 \cdot \overline{CX_{0,2}}
\end{aligned}$$

$$\begin{aligned}
(C_{85}) : CX_{0,1} \cdot Z_0 &\xleftarrow{E_4} \overline{CX_{0,1} \cdot Z_0 \cdot \overline{\sigma_{0,1} \cdot \sigma_{0,1}}} \\
&\xrightarrow{S_1} \overline{\sigma_{0,1} \cdot CX_{1,0} \cdot \sigma_{0,1} \cdot Z_0 \cdot \sigma_{0,1} \cdot \sigma_{0,1}} \\
&\xleftarrow{(34)} \sigma_{0,1} \cdot \underline{CX_{1,0} \cdot \overline{Z_1 \cdot \sigma_{0,1}}} \\
&\xrightarrow{C_{48}} \sigma_{0,1} \cdot \underline{\overline{Z_1 \cdot CX_{1,0}}} \cdot \sigma_{0,1} \\
&\xrightarrow{(34)} \underline{\sigma_{0,1} \cdot \overline{\sigma_{0,1} \cdot Z_0 \cdot \sigma_{0,1}}} \cdot CX_{1,0} \cdot \sigma_{0,1} \\
&\xrightarrow{E_4} Z_0 \cdot \sigma_{0,1} \cdot \underline{CX_{1,0} \cdot \sigma_{0,1}} \\
&\xleftarrow{S_1} Z_0 \cdot \overline{CX_{0,1}}
\end{aligned}$$

$$\begin{aligned}
(C_{87}) : CX_{1,2} \cdot Z_1 &\xleftarrow{(23)} \overline{K_{1,2} \cdot \overline{K_{1,2}} \cdot CX_{1,2} \cdot Z_1} \\
&\xleftarrow{C_{10}} K_{1,2} \cdot \overline{CX_{2,1} \cdot K_{1,2} \cdot Z_1} \\
&\xleftarrow{C_2} K_{1,2} \cdot \underline{CX_{2,1} \cdot \overline{X_1 \cdot K_{1,2}}} \\
&\xleftarrow{C_{86}} \underline{K_{1,2} \cdot \overline{X_1 \cdot CX_{2,1}}} \cdot K_{1,2} \\
&\xrightarrow{C_{27}} \overline{Z_1 \cdot K_{1,2} \cdot CX_{2,1}} \cdot K_{1,2} \\
&\xrightarrow{C_4} Z_1 \cdot \overline{CX_{1,2} \cdot K_{1,2}} \cdot K_{1,2} \\
&\xrightarrow{(23)} Z_1 \cdot CX_{1,2}
\end{aligned}$$

$$\begin{aligned}
(C_{89}) : CCX_{0,2} \cdot \underline{CX_{0,1}} &\xrightarrow{S_1} \underline{CCX_{0,2} \cdot \overline{\sigma_{0,1} \cdot CX_{1,0} \cdot \sigma_{0,1}}} \\
&\xrightarrow{(14)} \overline{\sigma_{0,1} \cdot CCX_{1,2} \cdot \sigma_{0,1} \cdot \sigma_{0,1} \cdot CX_{1,0} \cdot \sigma_{0,1}} \\
&\xrightarrow{E_4} \sigma_{0,1} \cdot \underline{CCX_{1,2} \cdot CX_{1,0}} \cdot \sigma_{0,1} \\
&\xrightarrow{(36)} \sigma_{0,1} \cdot \overline{CX_{1,0} \cdot CCX_{1,2}} \cdot \sigma_{0,1} \\
&\xleftarrow{E_4} \sigma_{0,1} \cdot CX_{1,0} \cdot \overline{\sigma_{0,1} \cdot \sigma_{0,1} \cdot CCX_{1,2} \cdot \sigma_{0,1}} \\
&\xleftarrow{(14)} \underline{\sigma_{0,1} \cdot CX_{1,0} \cdot \sigma_{0,1} \cdot \overline{CCX_{0,2}}} \\
&\xleftarrow{S_1} \overline{CX_{0,1} \cdot CCX_{0,2}}
\end{aligned}$$

$$\begin{aligned}
(C_{91}) : \underline{CZ_{1,2}} \cdot Z_2 &\xrightarrow{(19)} \overline{\sigma_{0,1} \cdot CZ_{0,2} \cdot \sigma_{0,1} \cdot Z_2} \\
&\xleftarrow{B_{33}} \sigma_{0,1} \cdot \underline{CZ_{0,2} \cdot \overline{Z_2 \cdot \sigma_{0,1}}} \\
&\xrightarrow{C_{78}} \sigma_{0,1} \cdot \overline{Z_2 \cdot CZ_{0,2}} \cdot \sigma_{0,1} \\
&\xleftarrow{B_{33}} \overline{Z_2 \cdot \sigma_{0,1} \cdot CZ_{0,2} \cdot \sigma_{0,1}} \\
&\xleftarrow{(19)} Z_2 \cdot \overline{CZ_{1,2}}
\end{aligned}$$

$$(C_{92}) : CX_{1,2} \cdot CX_{2,0}$$

$$\begin{aligned} & \xleftarrow{E_4} CX_{1,2} \cdot CX_{2,0} \cdot \overline{\sigma_{0,1}} \cdot \sigma_{0,1} \\ & \xrightarrow{(30)} \overline{\sigma_{0,1} \cdot CX_{0,2} \cdot \sigma_{0,1} \cdot CX_{2,0} \cdot \sigma_{0,1}} \cdot \sigma_{0,1} \\ & \xleftarrow{(31)} \sigma_{0,1} \cdot \overline{CX_{0,2} \cdot CX_{2,1}} \cdot \sigma_{0,1} \\ & \xrightarrow{C_{18}} \sigma_{0,1} \cdot \overline{CX_{2,1} \cdot CX_{0,2} \cdot CX_{0,1}} \cdot \sigma_{0,1} \\ & \xrightarrow{(31)} \overline{\sigma_{0,1} \cdot \sigma_{0,1} \cdot CX_{2,0} \cdot \sigma_{0,1} \cdot CX_{0,2} \cdot CX_{0,1}} \cdot \sigma_{0,1} \\ & \xrightarrow{E_4} CX_{2,0} \cdot \sigma_{0,1} \cdot CX_{0,2} \cdot \overline{CX_{0,1}} \cdot \sigma_{0,1} \\ & \xrightarrow{S_1} CX_{2,0} \cdot \overline{\sigma_{0,1} \cdot CX_{0,2} \cdot \sigma_{0,1} \cdot CX_{1,0} \cdot \sigma_{0,1}} \cdot \sigma_{0,1} \\ & \xleftarrow{(30)} CX_{2,0} \cdot \overline{CX_{1,2} \cdot CX_{1,0} \cdot \sigma_{0,1} \cdot \sigma_{0,1}} \\ & \xrightarrow{E_4} CX_{2,0} \cdot CX_{1,2} \cdot CX_{1,0} \end{aligned}$$

$$(C_{93}) : CX_{2,0} \cdot \overline{CCX_{0,2}}$$

$$\begin{aligned} & \xrightarrow{(14)} CX_{2,0} \cdot \overline{\sigma_{0,1} \cdot \overline{CCX_{1,2}} \cdot \sigma_{0,1}} \\ & \xleftarrow{E_4} \overline{\sigma_{0,1} \cdot \sigma_{0,1} \cdot CX_{2,0} \cdot \sigma_{0,1} \cdot \overline{CCX_{1,2}} \cdot \sigma_{0,1}} \\ & \xleftarrow{(31)} \sigma_{0,1} \cdot \overline{CX_{2,1} \cdot \overline{CCX_{1,2}}} \cdot \sigma_{0,1} \\ & \xrightarrow{C_{61}} \sigma_{0,1} \cdot \overline{CCX_{1,2} \cdot CX_{2,0} \cdot \overline{CX_{2,1}}} \cdot \sigma_{0,1} \\ & \xrightarrow{(31)} \sigma_{0,1} \cdot \overline{CCX_{1,2} \cdot CX_{2,0} \cdot \sigma_{0,1} \cdot \overline{CX_{2,0} \cdot \sigma_{0,1} \cdot \sigma_{0,1}}} \\ & \xrightarrow{E_4} \sigma_{0,1} \cdot \overline{CCX_{1,2} \cdot CX_{2,0} \cdot \sigma_{0,1} \cdot CX_{2,0}} \\ & \xleftarrow{E_4} \sigma_{0,1} \cdot \overline{CCX_{1,2} \cdot \sigma_{0,1} \cdot \sigma_{0,1} \cdot CX_{2,0} \cdot \sigma_{0,1} \cdot CX_{2,0}} \\ & \xleftarrow{(31)} \overline{\sigma_{0,1} \cdot \overline{CCX_{1,2}} \cdot \sigma_{0,1} \cdot \overline{CX_{2,1}}} \cdot CX_{2,0} \\ & \xleftarrow{(14)} \overline{CCX_{0,2}} \cdot CX_{2,1} \cdot CX_{2,0} \end{aligned}$$

$$\begin{aligned} (C_{94}) : CX_{1,0} \cdot CX_{1,2} & \xleftarrow{E_{14}} CX_{1,0} \cdot CX_{1,2} \cdot \overline{CX_{2,0} \cdot CX_{2,0}} \\ & \xleftarrow{E_8} CX_{1,0} \cdot CX_{1,2} \cdot CX_{2,0} \cdot \overline{CX_{1,2} \cdot CX_{1,2}} \cdot CX_{2,0} \\ & \xleftarrow{E_{14}} CX_{1,0} \cdot CX_{1,2} \cdot CX_{2,0} \cdot \overline{CX_{1,2} \cdot \overline{CX_{2,0}} \cdot CX_{2,0}} \cdot CX_{1,2} \cdot CX_{2,0} \\ & \xrightarrow{C_{92}} CX_{1,0} \cdot CX_{1,2} \cdot \overline{CX_{2,0} \cdot \overline{CX_{2,0}} \cdot CX_{1,2} \cdot CX_{1,0}} \cdot CX_{2,0} \cdot CX_{1,2} \cdot CX_{2,0} \\ & \xrightarrow{E_{14}} CX_{1,0} \cdot \overline{CX_{1,2} \cdot CX_{1,2}} \cdot CX_{1,0} \cdot CX_{2,0} \cdot CX_{1,2} \cdot CX_{2,0} \\ & \xrightarrow{E_8} \overline{CX_{1,0} \cdot CX_{1,0}} \cdot CX_{2,0} \cdot CX_{1,2} \cdot CX_{2,0} \\ & \xrightarrow{E_1} CX_{2,0} \cdot \overline{CX_{1,2} \cdot CX_{2,0}} \\ & \xrightarrow{C_{92}} \overline{CX_{2,0} \cdot \overline{CX_{2,0}} \cdot CX_{1,2} \cdot CX_{1,0}} \\ & \xrightarrow{E_{14}} CX_{1,2} \cdot CX_{1,0} \end{aligned}$$

$$\begin{aligned} (C_{95}) : \overline{CZ_{0,1}} \cdot \overline{CCX_{0,1}} & \xrightarrow{(1)} \overline{K_{1,2} \cdot CX_{0,1} \cdot \overline{K_{1,2} \cdot \overline{CCX_{0,1}}}} \\ & \xrightarrow{C_1} K_{1,2} \cdot \overline{CX_{0,1} \cdot \overline{CCX_{0,2}}} \cdot K_{1,2} \\ & \xleftarrow{C_{89}} \overline{K_{1,2} \cdot \overline{CCX_{0,2}} \cdot CX_{0,1}} \cdot K_{1,2} \\ & \xleftarrow{C_{38}} \overline{CCX_{0,1} \cdot \overline{K_{1,2} \cdot CX_{0,1}}} \cdot K_{1,2} \\ & \xleftarrow{(1)} \overline{CCX_{0,1} \cdot \overline{CZ_{0,1}}} \end{aligned}$$

$$\begin{aligned} (C_{96}) : \overline{CZ_{0,2}} \cdot \overline{CCX_{0,2}} & \xrightarrow{(18)} \overline{\sigma_{1,2} \cdot \overline{CZ_{0,1}} \cdot \sigma_{1,2}} \cdot \overline{CCX_{0,2}} \\ & \xleftarrow{E_{10}} \sigma_{1,2} \cdot \overline{CZ_{0,1} \cdot \sigma_{1,2} \cdot \overline{CCX_{0,2}} \cdot \sigma_{1,2} \cdot \sigma_{1,2}} \\ & \xleftarrow{(33)} \sigma_{1,2} \cdot \overline{CZ_{0,1} \cdot \overline{CCX_{0,1}}} \cdot \sigma_{1,2} \\ & \xrightarrow{C_{95}} \sigma_{1,2} \cdot \overline{CCX_{0,1} \cdot \overline{CZ_{0,1}}} \cdot \sigma_{1,2} \\ & \xrightarrow{(33)} \sigma_{1,2} \cdot \overline{\sigma_{1,2} \cdot \overline{CCX_{0,2}} \cdot \sigma_{1,2} \cdot \overline{CZ_{0,1}} \cdot \sigma_{1,2}} \\ & \xleftarrow{(18)} \overline{\sigma_{1,2} \cdot \sigma_{1,2} \cdot \overline{CCX_{0,2}} \cdot \overline{CZ_{0,2}}} \\ & \xrightarrow{E_{10}} \overline{CCX_{0,2} \cdot \overline{CZ_{0,2}}} \end{aligned}$$

$$(C_{97}) : CZ_{1,2} \cdot CCX_{1,2}$$

$$\begin{aligned} & \xleftarrow{E_4} \overline{CZ_{1,2} \cdot CCX_{1,2} \cdot \sigma_{0,1} \cdot \sigma_{0,1}} \\ & \xrightarrow{(19)} \overline{\sigma_{0,1} \cdot CZ_{0,2} \cdot \sigma_{0,1} \cdot CCX_{1,2} \cdot \sigma_{0,1} \cdot \sigma_{0,1}} \\ & \xleftarrow{(14)} \overline{\sigma_{0,1} \cdot CZ_{0,2} \cdot \overline{CCX_{0,2}} \cdot \sigma_{0,1}} \\ & \xrightarrow{C_{96}} \overline{\sigma_{0,1} \cdot \overline{CCX_{0,2}} \cdot CZ_{0,2} \cdot \sigma_{0,1}} \\ & \xrightarrow{(14)} \overline{\sigma_{0,1} \cdot \sigma_{0,1} \cdot CCX_{1,2} \cdot \sigma_{0,1} \cdot CZ_{0,2} \cdot \sigma_{0,1}} \\ & \xleftarrow{(19)} \overline{\sigma_{0,1} \cdot \sigma_{0,1} \cdot CCX_{1,2} \cdot \overline{CZ_{1,2}}} \\ & \xrightarrow{E_4} CCX_{1,2} \cdot CZ_{1,2} \end{aligned}$$

$$(C_{98}) : CCX_{1,2} \cdot CX_{1,0}$$

$$\begin{aligned} & \xleftarrow{(25)} \overline{K_{0,1} \cdot \overline{K_{0,1}} \cdot CCX_{1,2} \cdot CX_{1,0}} \\ & \xrightarrow{C_{36}} K_{0,1} \cdot \overline{CCX_{0,2} \cdot K_{0,1}} \cdot CX_{1,0} \\ & \xrightarrow{(12)} K_{0,1} \cdot CCX_{0,2} \cdot \overline{K_{0,1} \cdot \overline{K_{0,1}} \cdot CX_{0,1} \cdot K_{0,1}} \\ & \xrightarrow{(25)} K_{0,1} \cdot \overline{CCX_{0,2} \cdot CX_{0,1}} \cdot K_{0,1} \\ & \xrightarrow{C_{89}} K_{0,1} \cdot \overline{CX_{0,1} \cdot \overline{CCX_{0,2}} \cdot K_{0,1}} \\ & \xleftarrow{C_{36}} \overline{K_{0,1} \cdot CX_{0,1} \cdot \overline{K_{0,1}} \cdot CCX_{1,2}} \\ & \xleftarrow{(12)} \overline{CX_{1,0} \cdot CCX_{1,2}} \end{aligned}$$

$$(C_{100}) : CZ_{0,2} \cdot \overline{CCX_{1,2}}$$

$$\begin{aligned} & \xrightarrow{S_{20}} \overline{CZ_{0,2} \cdot \sigma_{1,2} \cdot \overline{CCX_{1,2}} \cdot \sigma_{1,2}} \\ & \xrightarrow{(18)} \overline{\sigma_{1,2} \cdot CZ_{0,1} \cdot \sigma_{1,2} \cdot \sigma_{1,2} \cdot CCX_{1,2} \cdot \sigma_{1,2}} \\ & \xrightarrow{E_{10}} \sigma_{1,2} \cdot \overline{CZ_{0,1} \cdot CCX_{1,2}} \cdot \sigma_{1,2} \\ & \xrightarrow{C_{77}} \sigma_{1,2} \cdot \overline{CCX_{1,2} \cdot \overline{CZ_{1,2}} \cdot CZ_{0,1} \cdot \sigma_{1,2}} \\ & \xrightarrow{S_{21}} \sigma_{1,2} \cdot CCX_{1,2} \cdot \overline{\sigma_{1,2} \cdot \overline{CZ_{1,2}} \cdot \sigma_{1,2} \cdot CZ_{0,1} \cdot \sigma_{1,2}} \\ & \xleftarrow{(18)} \overline{\sigma_{1,2} \cdot CCX_{1,2} \cdot \sigma_{1,2} \cdot CZ_{1,2} \cdot \overline{CZ_{0,2}}} \\ & \xleftarrow{S_{20}} \overline{CCX_{1,2} \cdot CZ_{1,2} \cdot CZ_{0,2}} \end{aligned}$$

$$(C_{101}) : CCX_{1,2} \cdot \overline{CX_{2,0}}$$

$$\begin{aligned} & \xrightarrow{S_{14}} \overline{CCX_{1,2} \cdot \sigma_{1,2} \cdot \overline{CX_{1,0}} \cdot \sigma_{1,2}} \\ & \xrightarrow{S_{20}} \overline{\sigma_{1,2} \cdot \overline{CCX_{1,2}} \cdot \sigma_{1,2} \cdot \sigma_{1,2} \cdot CX_{1,0} \cdot \sigma_{1,2}} \\ & \xrightarrow{E_{10}} \sigma_{1,2} \cdot \overline{CCX_{1,2} \cdot CX_{1,0}} \cdot \sigma_{1,2} \\ & \xrightarrow{(36)} \sigma_{1,2} \cdot \overline{CX_{1,0} \cdot \overline{CCX_{1,2}} \cdot \sigma_{1,2}} \\ & \xleftarrow{E_{10}} \sigma_{1,2} \cdot CX_{1,0} \cdot \overline{\sigma_{1,2} \cdot \overline{\sigma_{1,2}} \cdot CCX_{1,2} \cdot \sigma_{1,2}} \\ & \xleftarrow{S_{20}} \overline{\sigma_{1,2} \cdot CX_{1,0} \cdot \sigma_{1,2} \cdot \overline{CCX_{1,2}}} \\ & \xleftarrow{S_{14}} \overline{CX_{2,0} \cdot CCX_{1,2}} \end{aligned}$$

$$\begin{aligned} (C_{101}) : CCX_{1,2} \cdot CZ_{0,2} & \xleftarrow{(24)} \overline{CCX_{1,2} \cdot CZ_{0,2} \cdot \overline{CCX_{1,2}} \cdot \overline{CCX_{1,2}}} \\ & \xleftarrow{E_{12}} \overline{CCX_{1,2} \cdot CZ_{0,2} \cdot CCX_{1,2} \cdot \overline{CZ_{1,2}} \cdot \overline{CZ_{1,2}} \cdot CCX_{1,2}} \\ & \xleftarrow{E_{11}} \overline{CCX_{1,2} \cdot CZ_{0,2} \cdot \overline{CCX_{1,2}} \cdot \overline{CZ_{1,2}} \cdot \overline{CZ_{0,2}} \cdot \overline{CZ_{0,2}} \cdot CZ_{1,2} \cdot CCX_{1,2}} \\ & \xleftarrow{C_{100}} \overline{CCX_{1,2} \cdot CZ_{0,2} \cdot \overline{CZ_{0,2}} \cdot \overline{CCX_{1,2}} \cdot CZ_{0,2} \cdot CZ_{1,2} \cdot CCX_{1,2}} \\ & \xrightarrow{E_{11}} \overline{CCX_{1,2} \cdot CCX_{1,2} \cdot CZ_{0,2} \cdot CZ_{1,2} \cdot CCX_{1,2}} \\ & \xrightarrow{(24)} \overline{CZ_{0,2} \cdot CZ_{1,2} \cdot CCX_{1,2}} \end{aligned}$$

$$\begin{aligned} (C_{102}) : CZ_{0,2} \cdot CX_{1,2} & \xleftarrow{E_8} \overline{CX_{1,2} \cdot \overline{CX_{1,2}} \cdot CZ_{0,2} \cdot CX_{1,2}} \\ & \xleftarrow{E_2} \overline{CX_{1,2} \cdot \overline{CZ_{0,1}} \cdot \overline{CZ_{0,1}} \cdot CX_{1,2} \cdot CZ_{0,2} \cdot CX_{1,2}} \\ & \xleftarrow{E_{11}} \overline{CX_{1,2} \cdot CZ_{0,1} \cdot \overline{CZ_{0,2}} \cdot \overline{CZ_{0,2}} \cdot \overline{CZ_{0,1}} \cdot CX_{1,2} \cdot CZ_{0,2} \cdot CX_{1,2}} \\ & \xleftarrow{C_{51}} \overline{CX_{1,2} \cdot CZ_{0,1} \cdot CZ_{0,2} \cdot \overline{CX_{1,2}} \cdot \overline{CZ_{0,2}} \cdot CZ_{0,2} \cdot CX_{1,2}} \\ & \xrightarrow{E_{11}} \overline{CX_{1,2} \cdot CZ_{0,1} \cdot CZ_{0,2} \cdot \overline{CX_{1,2}} \cdot \overline{CX_{1,2}}} \\ & \xrightarrow{E_8} \overline{CX_{1,2} \cdot CZ_{0,1} \cdot CZ_{0,2}} \end{aligned}$$

$$(C_{103}) : CZ_{0,2} \cdot Z_0$$

$$\xleftarrow{(23)} \overline{K_{1,2} \cdot K_{1,2}} \cdot CZ_{0,2} \cdot Z_0$$

$$\xrightarrow{C_{28}} K_{1,2} \cdot \overline{CX_{0,2}} \cdot \overline{K_{1,2}} \cdot Z_0$$

$$\xleftarrow{B_6} K_{1,2} \cdot \overline{CX_{0,2}} \cdot \overline{Z_0} \cdot \overline{K_{1,2}}$$

$$\xrightarrow{(9)} K_{1,2} \cdot \overline{\sigma_{1,2}} \cdot CX_{0,1} \cdot \overline{\sigma_{1,2}} \cdot Z_0 \cdot K_{1,2}$$

$$\xleftarrow{B_{12}} K_{1,2} \cdot \sigma_{1,2} \cdot \overline{CX_{0,1}} \cdot \overline{Z_0} \cdot \overline{\sigma_{1,2}} \cdot K_{1,2}$$

$$\xrightarrow{C_{85}} K_{1,2} \cdot \overline{\sigma_{1,2}} \cdot \overline{Z_0} \cdot CX_{0,1} \cdot \sigma_{1,2} \cdot K_{1,2}$$

$$\xleftarrow{B_{12}} K_{1,2} \cdot \overline{Z_0} \cdot \overline{\sigma_{1,2}} \cdot CX_{0,1} \cdot \sigma_{1,2} \cdot K_{1,2}$$

$$\xleftarrow{B_6} \overline{Z_0} \cdot \overline{K_{1,2}} \cdot \overline{\sigma_{1,2}} \cdot CX_{0,1} \cdot \overline{\sigma_{1,2}} \cdot K_{1,2}$$

$$\xleftarrow{(9)} Z_0 \cdot K_{1,2} \cdot \overline{CX_{0,2}} \cdot K_{1,2}$$

$$\xleftarrow{C_{28}} Z_0 \cdot K_{1,2} \cdot \overline{K_{1,2}} \cdot CZ_{0,2}$$

$$\xrightarrow{(23)} Z_0 \cdot CZ_{0,2}$$

$$(C_{104}) : X_2 \cdot CCX_{0,2}$$

$$\xleftarrow{(25)} X_2 \cdot \overline{CCX_{0,2}} \cdot \overline{K_{0,1}} \cdot \overline{K_{0,1}}$$

$$\xleftarrow{C_{36}} X_2 \cdot \overline{K_{0,1}} \cdot \overline{CCX_{1,2}} \cdot K_{0,1}$$

$$\xrightarrow{B_{17}} \overline{K_{0,1}} \cdot \overline{X_2} \cdot \overline{CCX_{1,2}} \cdot K_{0,1}$$

$$\xrightarrow{C_{83}} K_{0,1} \cdot \overline{CCX_{1,2}} \cdot \overline{CX_{1,0}} \cdot \overline{X_2} \cdot K_{0,1}$$

$$\xrightarrow{C_{36}} \overline{CCX_{0,2}} \cdot \overline{K_{0,1}} \cdot \overline{CX_{1,0}} \cdot \overline{X_2} \cdot K_{0,1}$$

$$\xrightarrow{B_{17}} CCX_{0,2} \cdot K_{0,1} \cdot \overline{CX_{1,0}} \cdot \overline{K_{0,1}} \cdot \overline{X_2}$$

$$\xrightarrow{(12)} CCX_{0,2} \cdot K_{0,1} \cdot \overline{K_{0,1}} \cdot \overline{CX_{0,1}} \cdot \overline{K_{0,1}} \cdot K_{0,1} \cdot X_2$$

$$\xrightarrow{(25)} CCX_{0,2} \cdot \overline{K_{0,1}} \cdot \overline{K_{0,1}} \cdot CX_{0,1} \cdot X_2$$

$$\xrightarrow{(25)} CCX_{0,2} \cdot CX_{0,1} \cdot X_2$$

$$(C_{105}) : \overline{CCX_{0,1}} \cdot CX_{0,2}$$

$$\xrightarrow{(32)} \overline{\sigma_{0,2}} \cdot \overline{CCX_{1,2}} \cdot \overline{\sigma_{0,2}} \cdot CX_{0,2}$$

$$\xleftarrow{E_{16}} \sigma_{0,2} \cdot CCX_{1,2} \cdot \overline{\sigma_{0,2}} \cdot CX_{0,2} \cdot \overline{\sigma_{0,2}} \cdot \overline{\sigma_{0,2}}$$

$$\xleftarrow{(29)} \sigma_{0,2} \cdot \overline{CCX_{1,2}} \cdot \overline{CX_{2,0}} \cdot \sigma_{0,2}$$

$$\xrightarrow{C_{101}} \sigma_{0,2} \cdot \overline{CX_{2,0}} \cdot \overline{CCX_{1,2}} \cdot \sigma_{0,2}$$

$$\xrightarrow{(29)} \sigma_{0,2} \cdot \overline{\sigma_{0,2}} \cdot \overline{CX_{0,2}} \cdot \overline{\sigma_{0,2}} \cdot \overline{CCX_{1,2}} \cdot \sigma_{0,2}$$

$$\xleftarrow{(32)} \overline{\sigma_{0,2}} \cdot \overline{\sigma_{0,2}} \cdot CX_{0,2} \cdot \overline{CCX_{0,1}}$$

$$\xrightarrow{E_{16}} CX_{0,2} \cdot CCX_{0,1}$$

$$(C_{106}) : \overline{CCX_{0,2}} \cdot CX_{2,1}$$

$$\xleftarrow{E_4} \overline{CCX_{0,2}} \cdot CX_{2,1} \cdot \overline{\sigma_{0,1}} \cdot \overline{\sigma_{0,1}}$$

$$\xrightarrow{(14)} \overline{\sigma_{0,1}} \cdot \overline{CCX_{1,2}} \cdot \overline{\sigma_{0,1}} \cdot CX_{2,1} \cdot \overline{\sigma_{0,1}} \cdot \overline{\sigma_{0,1}}$$

$$\xleftarrow{S_6} \sigma_{0,1} \cdot \overline{CCX_{1,2}} \cdot \overline{CX_{2,0}} \cdot \sigma_{0,1}$$

$$\xrightarrow{C_{101}} \sigma_{0,1} \cdot \overline{CX_{2,0}} \cdot \overline{CCX_{1,2}} \cdot \sigma_{0,1}$$

$$\xrightarrow{S_6} \overline{\sigma_{0,1}} \cdot \overline{\sigma_{0,1}} \cdot \overline{CX_{2,1}} \cdot \overline{\sigma_{0,1}} \cdot \overline{CCX_{1,2}} \cdot \sigma_{0,1}$$

$$\xrightarrow{E_4} CX_{2,1} \cdot \overline{\sigma_{0,1}} \cdot \overline{CCX_{1,2}} \cdot \sigma_{0,1}$$

$$\xleftarrow{(14)} CX_{2,1} \cdot \overline{CCX_{0,2}}$$

$$(C_{107}) : CCX_{0,1} \cdot CX_{1,2} \xleftarrow{(23)} \overline{K_{1,2}} \cdot \overline{K_{1,2}} \cdot \overline{CCX_{0,1}} \cdot CX_{1,2}$$

$$\xrightarrow{C_{44}} K_{1,2} \cdot \overline{CCX_{0,2}} \cdot \overline{K_{1,2}} \cdot CX_{1,2}$$

$$\xleftarrow{C_{10}} K_{1,2} \cdot \overline{CCX_{0,2}} \cdot \overline{CX_{2,1}} \cdot K_{1,2}$$

$$\xrightarrow{C_{106}} K_{1,2} \cdot \overline{CX_{2,1}} \cdot \overline{CCX_{0,2}} \cdot K_{1,2}$$

$$\xrightarrow{C_4} \overline{CX_{1,2}} \cdot \overline{K_{1,2}} \cdot \overline{CCX_{0,2}} \cdot K_{1,2}$$

$$\xleftarrow{C_{38}} CX_{1,2} \cdot \overline{CCX_{0,1}} \cdot \overline{K_{1,2}} \cdot K_{1,2}$$

$$\xrightarrow{(23)} CX_{1,2} \cdot CCX_{0,1}$$

$$(C_{108}) : X_0 \cdot \overline{CZ_{0,2}} \xrightarrow{(18)} X_0 \cdot \overline{\sigma_{1,2}} \cdot \overline{CZ_{0,1}} \cdot \overline{\sigma_{1,2}}$$

$$\xrightarrow{B_{11}} \overline{\sigma_{1,2}} \cdot \overline{X_0} \cdot \overline{CZ_{0,1}} \cdot \sigma_{1,2}$$

$$\xrightarrow{C_{53}} \sigma_{1,2} \cdot \overline{CZ_{0,1}} \cdot \overline{Z_1} \cdot \overline{X_0} \cdot \sigma_{1,2}$$

$$\xrightarrow{B_{11}} \sigma_{1,2} \cdot CZ_{0,1} \cdot Z_1 \cdot \overline{\sigma_{1,2}} \cdot \overline{X_0}$$

$$\xleftarrow{E_{10}} \sigma_{1,2} \cdot CZ_{0,1} \cdot \overline{\sigma_{1,2}} \cdot \overline{\sigma_{1,2}} \cdot Z_1 \cdot \overline{\sigma_{1,2}} \cdot X_0$$

$$\xleftarrow{S_{22}} \overline{\sigma_{1,2}} \cdot \overline{CZ_{0,1}} \cdot \overline{\sigma_{1,2}} \cdot \overline{Z_2} \cdot X_0$$

$$\xleftarrow{(18)} \overline{CZ_{0,2}} \cdot Z_2 \cdot X_0$$

$$\begin{aligned}
(C_{109}) : X_2 \cdot CX_{0,1} \cdot CCX_{0,2} &\xleftarrow{E_{17}} X_2 \cdot CX_{0,1} \cdot CCX_{0,2} \cdot \overline{X_2 \cdot X_2} \\
&\xleftarrow{E_7} X_2 \cdot CX_{0,1} \cdot CCX_{0,2} \cdot \underline{X_2 \cdot \overline{CCX_{0,2}} \cdot CCX_{0,2}} \cdot X_2 \\
&\xrightarrow{C_{104}} X_2 \cdot CX_{0,1} \cdot \underline{CCX_{0,2} \cdot \overline{CCX_{0,2}}} \cdot CX_{0,1} \cdot \overline{X_2} \cdot CCX_{0,2} \cdot X_2 \\
&\xrightarrow{E_7} X_2 \cdot \underline{CX_{0,1} \cdot CX_{0,1}} \cdot X_2 \cdot CCX_{0,2} \cdot X_2 \\
&\xrightarrow{(22)} \underline{X_2 \cdot X_2} \cdot CCX_{0,2} \cdot X_2 \\
&\xrightarrow{E_{17}} CCX_{0,2} \cdot X_2
\end{aligned}$$

$$\begin{aligned}
(C_{110}) : CZ_{0,2} \cdot CZ_{0,1} \cdot CCX_{0,1} &\xleftarrow{E_{11}} CZ_{0,2} \cdot CZ_{0,1} \cdot CCX_{0,1} \cdot \overline{CZ_{0,2} \cdot CZ_{0,2}} \\
&\xleftarrow{E_{18}} CZ_{0,2} \cdot CZ_{0,1} \cdot CCX_{0,1} \cdot \underline{CZ_{0,2} \cdot \overline{CCX_{0,1}} \cdot CCX_{0,1}} \cdot CZ_{0,2} \\
&\xrightarrow{C_{81}} CZ_{0,2} \cdot CZ_{0,1} \cdot \underline{CCX_{0,1} \cdot \overline{CCX_{0,1}}} \cdot CZ_{0,1} \cdot \overline{CZ_{0,2}} \cdot CCX_{0,1} \cdot CZ_{0,2} \\
&\xrightarrow{E_{18}} CZ_{0,2} \cdot \underline{CZ_{0,1} \cdot CZ_{0,1}} \cdot CZ_{0,2} \cdot CCX_{0,1} \cdot CZ_{0,2} \\
&\xrightarrow{E_2} \underline{CZ_{0,2} \cdot CZ_{0,2}} \cdot CCX_{0,1} \cdot CZ_{0,2} \\
&\xrightarrow{E_{11}} CCX_{0,1} \cdot CZ_{0,2}
\end{aligned}$$

$$\begin{aligned}
(C_{111}) : \underline{CZ_{0,1} \cdot CZ_{0,2}} \cdot CCX_{0,2} &\xrightarrow{C_{60}} \overline{CZ_{0,2} \cdot CZ_{0,1}} \cdot CCX_{0,2} \\
&\xleftarrow{E_2} CZ_{0,2} \cdot CZ_{0,1} \cdot CCX_{0,2} \cdot \overline{CZ_{0,1} \cdot CZ_{0,1}} \\
&\xleftarrow{E_7} CZ_{0,2} \cdot CZ_{0,1} \cdot CCX_{0,2} \cdot \underline{CZ_{0,1} \cdot \overline{CCX_{0,2}} \cdot CCX_{0,2}} \cdot CZ_{0,1} \\
&\xrightarrow{C_{80}} CZ_{0,2} \cdot CZ_{0,1} \cdot \underline{CCX_{0,2} \cdot \overline{CCX_{0,2}}} \cdot CZ_{0,1} \cdot \overline{CZ_{0,2}} \cdot CCX_{0,2} \cdot CZ_{0,1} \\
&\xrightarrow{E_7} CZ_{0,2} \cdot \underline{CZ_{0,1} \cdot CZ_{0,1}} \cdot CZ_{0,2} \cdot CCX_{0,2} \cdot CZ_{0,1} \\
&\xrightarrow{E_2} \underline{CZ_{0,2} \cdot CZ_{0,2}} \cdot CCX_{0,2} \cdot CZ_{0,1} \\
&\xrightarrow{E_{11}} CCX_{0,2} \cdot CZ_{0,1}
\end{aligned}$$

$$\begin{aligned}
(C_{112}) : X_1 \cdot Z_0 \cdot CZ_{0,1} &\xleftarrow{E_{13}} X_1 \cdot Z_0 \cdot CZ_{0,1} \cdot \overline{X_1 \cdot X_1} \\
&\xleftarrow{E_2} X_1 \cdot Z_0 \cdot CZ_{0,1} \cdot \underline{X_1 \cdot \overline{CZ_{0,1}} \cdot CZ_{0,1}} \cdot X_1 \\
&\xrightarrow{C_{70}} X_1 \cdot Z_0 \cdot \underline{CZ_{0,1} \cdot \overline{CZ_{0,1}}} \cdot \overline{Z_0 \cdot X_1} \cdot CZ_{0,1} \cdot X_1 \\
&\xrightarrow{E_2} X_1 \cdot \underline{Z_0 \cdot Z_0} \cdot X_1 \cdot CZ_{0,1} \cdot X_1 \\
&\xrightarrow{E_3} \underline{X_1 \cdot X_1} \cdot CZ_{0,1} \cdot X_1 \\
&\xrightarrow{E_{13}} CZ_{0,1} \cdot X_1
\end{aligned}$$

$$\begin{aligned}
(C_{113}) : CZ_{1,2} \cdot CZ_{0,1} \cdot CCX_{0,1} &\xleftarrow{E_{18}} \overline{CCX_{0,1} \cdot CCX_{0,1}} \cdot CZ_{1,2} \cdot CZ_{0,1} \cdot CCX_{0,1} \\
&\xleftarrow{E_{12}} CCX_{0,1} \cdot \overline{CZ_{1,2} \cdot CZ_{1,2} \cdot CCX_{0,1}} \cdot CZ_{1,2} \cdot CZ_{0,1} \cdot CCX_{0,1} \\
&\xrightarrow{C_{82}} CCX_{0,1} \cdot CZ_{1,2} \cdot \overline{CCX_{0,1} \cdot CZ_{0,1} \cdot CZ_{1,2} \cdot CZ_{1,2} \cdot CZ_{0,1} \cdot CCX_{0,1}} \\
&\xrightarrow{E_{12}} CCX_{0,1} \cdot CZ_{1,2} \cdot CCX_{0,1} \cdot \overline{CZ_{0,1} \cdot CZ_{0,1}} \cdot CCX_{0,1} \\
&\xrightarrow{E_2} CCX_{0,1} \cdot CZ_{1,2} \cdot \overline{CCX_{0,1} \cdot CCX_{0,1}} \\
&\xrightarrow{E_{18}} CCX_{0,1} \cdot CZ_{1,2}
\end{aligned}$$

$$\begin{aligned}
(C_{114}) : X_2 \cdot \overline{CZ_{0,2}} &\xrightarrow{S_{23}} \underline{X_2} \cdot \overline{\sigma_{0,2} \cdot CZ_{0,2} \cdot \sigma_{0,2}} \\
&\xrightarrow{(15)} \overline{\sigma_{0,2} \cdot X_0 \cdot \overline{\sigma_{0,2} \cdot \sigma_{0,2}}} \cdot CZ_{0,2} \cdot \sigma_{0,2} \\
&\xrightarrow{E_{16}} \sigma_{0,2} \cdot \underline{X_0} \cdot \overline{CZ_{0,2}} \cdot \sigma_{0,2} \\
&\xrightarrow{C_{108}} \sigma_{0,2} \cdot \overline{CZ_{0,2} \cdot \underline{Z_2} \cdot X_0} \cdot \sigma_{0,2} \\
&\xrightarrow{(16)} \sigma_{0,2} \cdot CZ_{0,2} \cdot \overline{\sigma_{0,2} \cdot Z_0 \cdot \overline{\sigma_{0,2} \cdot X_0 \cdot \sigma_{0,2}}} \\
&\xleftarrow{(15)} \overline{\sigma_{0,2} \cdot CZ_{0,2} \cdot \sigma_{0,2} \cdot Z_0 \cdot \overline{X_2}} \\
&\xleftarrow{S_{23}} \overline{CZ_{0,2} \cdot Z_0 \cdot X_2}
\end{aligned}
\qquad
\begin{aligned}
(C_{115}) : X_2 \cdot Z_0 \cdot CZ_{0,2} &\xleftarrow{E_{17}} X_2 \cdot Z_0 \cdot CZ_{0,2} \cdot \overline{X_2 \cdot X_2} \\
&\xleftarrow{E_{11}} X_2 \cdot Z_0 \cdot CZ_{0,2} \cdot \underline{X_2 \cdot \overline{CZ_{0,2} \cdot CZ_{0,2}}} \cdot X_2 \\
&\xrightarrow{C_{114}} X_2 \cdot Z_0 \cdot \overline{CZ_{0,2} \cdot \overline{CZ_{0,2} \cdot Z_0 \cdot X_2} \cdot CZ_{0,2} \cdot X_2} \\
&\xrightarrow{E_{11}} X_2 \cdot Z_0 \cdot Z_0 \cdot X_2 \cdot CZ_{0,2} \cdot X_2 \\
&\xrightarrow{E_3} \underline{X_2 \cdot X_2} \cdot CZ_{0,2} \cdot X_2 \\
&\xrightarrow{E_{17}} CZ_{0,2} \cdot X_2
\end{aligned}$$

$$\begin{aligned}
(C_{116}) : CZ_{0,1} \cdot CZ_{1,2} \cdot CCX_{1,2} &\xleftarrow{E_2} CZ_{0,1} \cdot CZ_{1,2} \cdot CCX_{1,2} \cdot \overline{CZ_{0,1} \cdot CZ_{0,1}} \\
&\xleftarrow{(24)} CZ_{0,1} \cdot CZ_{1,2} \cdot CCX_{1,2} \cdot \overline{CZ_{0,1} \cdot \overline{CCX_{1,2} \cdot CCX_{1,2}}} \cdot CZ_{0,1} \\
&\xrightarrow{C_{77}} CZ_{0,1} \cdot CZ_{1,2} \cdot \overline{CCX_{1,2} \cdot \overline{CCX_{1,2} \cdot CZ_{1,2} \cdot CZ_{0,1} \cdot CCX_{1,2} \cdot CZ_{0,1}}} \\
&\xrightarrow{(24)} CZ_{0,1} \cdot \overline{CZ_{1,2} \cdot CZ_{1,2}} \cdot CZ_{0,1} \cdot CCX_{1,2} \cdot CZ_{0,1} \\
&\xrightarrow{E_{12}} \overline{CZ_{0,1} \cdot CZ_{0,1}} \cdot CCX_{1,2} \cdot CZ_{0,1} \\
&\xrightarrow{E_2} CCX_{1,2} \cdot CZ_{0,1}
\end{aligned}$$

$$\begin{aligned}
(C_{117}) : X_0 \cdot Z_2 \cdot CZ_{0,2} &\xleftarrow{(21)} X_0 \cdot Z_2 \cdot CZ_{0,2} \cdot \overline{X_0 \cdot X_0} \\
&\xleftarrow{E_{11}} X_0 \cdot Z_2 \cdot CZ_{0,2} \cdot \underline{X_0 \cdot \overline{CZ_{0,2} \cdot CZ_{0,2}}} \cdot X_0 \\
&\xrightarrow{C_{108}} X_0 \cdot Z_2 \cdot \overline{CZ_{0,2} \cdot \overline{CZ_{0,2} \cdot Z_2 \cdot X_0} \cdot CZ_{0,2} \cdot X_0} \\
&\xrightarrow{E_{11}} X_0 \cdot \underline{Z_2 \cdot Z_2} \cdot X_0 \cdot CZ_{0,2} \cdot X_0 \\
&\xrightarrow{E_{19}} \underline{X_0 \cdot X_0} \cdot CZ_{0,2} \cdot X_0 \\
&\xrightarrow{(21)} CZ_{0,2} \cdot X_0
\end{aligned}$$

$$\begin{aligned}
(C_{118}) : X_0 \cdot \underline{CX_{0,2}} &\xrightarrow{(9)} \underline{X_0 \cdot \overline{\sigma_{1,2} \cdot CX_{0,1} \cdot \sigma_{1,2}}} \\
&\xrightarrow{B_{11}} \overline{\sigma_{1,2} \cdot \overline{X_0} \cdot CX_{0,1} \cdot \sigma_{1,2}} \\
&\xrightarrow{C_3} \sigma_{1,2} \cdot \overline{CX_{0,1} \cdot X_1 \cdot \overline{X_0} \cdot \sigma_{1,2}} \\
&\xrightarrow{B_{11}} \sigma_{1,2} \cdot CX_{0,1} \cdot X_1 \cdot \overline{\sigma_{1,2} \cdot \overline{X_0}} \\
&\xleftarrow{E_{10}} \sigma_{1,2} \cdot CX_{0,1} \cdot \overline{\sigma_{1,2} \cdot \sigma_{1,2} \cdot X_1 \cdot \sigma_{1,2} \cdot X_0} \\
&\xleftarrow{S_{18}} \sigma_{1,2} \cdot CX_{0,1} \cdot \sigma_{1,2} \cdot \overline{X_2} \cdot X_0 \\
&\xleftarrow{(9)} \overline{CX_{0,2} \cdot X_2 \cdot X_0}
\end{aligned}
\qquad
\begin{aligned}
(C_{119}) : CX_{0,1} \cdot \underline{CCX_{0,1}} &\xrightarrow{(32)} CX_{0,1} \cdot \overline{\sigma_{0,2} \cdot \overline{CCX_{1,2} \cdot \sigma_{0,2}}} \\
&\xleftarrow{E_{16}} \overline{\sigma_{0,2} \cdot \overline{\sigma_{0,2} \cdot CX_{0,1} \cdot \sigma_{0,2} \cdot CCX_{1,2} \cdot \sigma_{0,2}}} \\
&\xleftarrow{S_9} \sigma_{0,2} \cdot \overline{CX_{2,1} \cdot CCX_{1,2} \cdot \sigma_{0,2}} \\
&\xrightarrow{C_{61}} \sigma_{0,2} \cdot \overline{CCX_{1,2} \cdot \overline{CX_{2,0} \cdot CX_{2,1} \cdot \sigma_{0,2}}} \\
&\xrightarrow{(29)} \overline{\sigma_{0,2} \cdot CCX_{1,2} \cdot \overline{\sigma_{0,2} \cdot CX_{0,2} \cdot \sigma_{0,2} \cdot CX_{2,1} \cdot \sigma_{0,2}}} \\
&\xleftarrow{(32)} \overline{CCX_{0,1} \cdot CX_{0,2} \cdot \sigma_{0,2} \cdot \overline{CX_{2,1} \cdot \sigma_{0,2}}} \\
&\xrightarrow{S_9} \overline{CCX_{0,1} \cdot CX_{0,2} \cdot \sigma_{0,2} \cdot \overline{\sigma_{0,2} \cdot CX_{0,1} \cdot \overline{\sigma_{0,2} \cdot \sigma_{0,2}}}} \\
&\xrightarrow{E_{16}} \overline{CCX_{0,1} \cdot CX_{0,2} \cdot \overline{\sigma_{0,2} \cdot \sigma_{0,2} \cdot CX_{0,1}}} \\
&\xrightarrow{E_{16}} \overline{CCX_{0,1} \cdot CX_{0,2} \cdot CX_{0,1}}
\end{aligned}$$

$$\begin{aligned}
(C_{120}) : X_0 \cdot X_2 \cdot CX_{0,2} &\xleftarrow{E_{15}} \overline{CX_{0,2} \cdot \overline{CX_{0,2} \cdot X_0 \cdot X_2 \cdot CX_{0,2}}} \\
&\xleftarrow{(21)} \overline{CX_{0,2} \cdot \overline{X_0} \cdot \overline{X_0} \cdot CX_{0,2} \cdot X_0 \cdot X_2 \cdot CX_{0,2}} \\
&\xrightarrow{C_{118}} \overline{CX_{0,2} \cdot X_0 \cdot \overline{CX_{0,2} \cdot X_2 \cdot \overline{X_0} \cdot X_0} \cdot X_2 \cdot CX_{0,2}} \\
&\xrightarrow{(21)} \overline{CX_{0,2} \cdot X_0 \cdot CX_{0,2} \cdot \overline{X_2 \cdot X_2} \cdot CX_{0,2}} \\
&\xrightarrow{E_{17}} \overline{CX_{0,2} \cdot X_0 \cdot \overline{CX_{0,2} \cdot CX_{0,2}}} \\
&\xrightarrow{E_{15}} \overline{CX_{0,2} \cdot X_0}
\end{aligned}
\qquad
\begin{aligned}
(C_{121}) : CZ_{0,1} \cdot \underline{CX_{2,1}} &\xrightarrow{S_5} \overline{CZ_{0,1} \cdot \overline{\sigma_{1,2} \cdot \overline{CX_{1,2} \cdot \sigma_{1,2}}}} \\
&\xleftarrow{E_{10}} \overline{\sigma_{1,2} \cdot \overline{\sigma_{1,2} \cdot CZ_{0,1} \cdot \sigma_{1,2} \cdot CX_{1,2} \cdot \sigma_{1,2}}} \\
&\xleftarrow{(18)} \sigma_{1,2} \cdot \overline{CZ_{0,2} \cdot CX_{1,2} \cdot \sigma_{1,2}} \\
&\xrightarrow{C_{102}} \sigma_{1,2} \cdot \overline{CX_{1,2} \cdot \overline{CZ_{0,1} \cdot CZ_{0,2} \cdot \sigma_{1,2}}} \\
&\xrightarrow{C_{60}} \sigma_{1,2} \cdot CX_{1,2} \cdot \overline{CZ_{0,2} \cdot CZ_{0,1} \cdot \sigma_{1,2}} \\
&\xrightarrow{(18)} \sigma_{1,2} \cdot CX_{1,2} \cdot \overline{\sigma_{1,2} \cdot CZ_{0,1} \cdot \overline{\sigma_{1,2} \cdot CZ_{0,1} \cdot \sigma_{1,2}}} \\
&\xleftarrow{(18)} \sigma_{1,2} \cdot CX_{1,2} \cdot \sigma_{1,2} \cdot \overline{CZ_{0,1} \cdot \overline{CZ_{0,2}}} \\
&\xleftarrow{S_5} \overline{CX_{2,1} \cdot CZ_{0,1} \cdot CZ_{0,2}}
\end{aligned}$$

$$\begin{aligned}
(C_{122}) : CCX_{0,1} \cdot CX_{0,1} &\xleftarrow{E_{18}} \overline{CCX_{0,1} \cdot CX_{0,1} \cdot \overline{CCX_{0,1} \cdot CCX_{0,1}}} \\
&\xleftarrow{E_{15}} \overline{CCX_{0,1} \cdot CX_{0,1} \cdot \overline{CCX_{0,1} \cdot \overline{CX_{0,2} \cdot CX_{0,2}}} \cdot CCX_{0,1}} \\
&\xleftarrow{(22)} \overline{CCX_{0,1} \cdot CX_{0,1} \cdot \overline{CCX_{0,1} \cdot CX_{0,2} \cdot \overline{CX_{0,1} \cdot CX_{0,1} \cdot CX_{0,2} \cdot CCX_{0,1}}}} \\
&\xleftarrow{C_{119}} \overline{CCX_{0,1} \cdot \overline{CX_{0,1} \cdot \overline{CX_{0,1} \cdot CCX_{0,1}}} \cdot CX_{0,1} \cdot CX_{0,2} \cdot CCX_{0,1}} \\
&\xrightarrow{(22)} \overline{CCX_{0,1} \cdot \overline{CCX_{0,1} \cdot CX_{0,1} \cdot CX_{0,2} \cdot CCX_{0,1}}} \\
&\xrightarrow{E_{18}} \overline{CX_{0,1} \cdot CX_{0,2} \cdot CCX_{0,1}}
\end{aligned}$$

$$\begin{aligned}
(C_{123}) : CZ_{1,2} \cdot CZ_{0,1} \cdot CX_{0,2} &\xleftarrow{E_{15}} \overline{CX_{0,2} \cdot \overline{CX_{0,2} \cdot CZ_{1,2} \cdot CZ_{0,1} \cdot CX_{0,2}}} \xleftarrow{E_{12}} \overline{CX_{0,2} \cdot \overline{CZ_{1,2} \cdot \overline{CZ_{1,2} \cdot CX_{0,2} \cdot CZ_{1,2} \cdot CZ_{0,1} \cdot CX_{0,2}}}} \\
&\xrightarrow{C_{84}} \overline{CX_{0,2} \cdot CZ_{1,2} \cdot \overline{CX_{0,2} \cdot CZ_{0,1} \cdot \overline{CZ_{1,2} \cdot CZ_{1,2} \cdot CZ_{0,1} \cdot CX_{0,2}}}} \\
&\xrightarrow{E_{12}} \overline{CX_{0,2} \cdot CZ_{1,2} \cdot CX_{0,2} \cdot \overline{CZ_{0,1} \cdot CZ_{0,1} \cdot CX_{0,2}}} \\
&\xrightarrow{E_2} \overline{CX_{0,2} \cdot CZ_{1,2} \cdot \overline{CX_{0,2} \cdot CX_{0,2}}} \\
&\xrightarrow{E_{15}} \overline{CX_{0,2} \cdot CZ_{1,2}}
\end{aligned}$$

$$\begin{array}{ll}
(C_{124}) : Z_1 \cdot \underline{CZ_{1,2}} \xrightarrow{(19)} Z_1 \cdot \overline{\sigma_{0,1} \cdot CZ_{0,2} \cdot \sigma_{0,1}} & (C_{125}) : Z_2 \cdot \underline{CCX_{0,1}} \xrightarrow{(33)} Z_2 \cdot \overline{\sigma_{1,2} \cdot \overline{CCX_{0,2}} \cdot \sigma_{1,2}} \\
\xrightarrow{(34)} \overline{\sigma_{0,1} \cdot Z_0 \cdot \sigma_{0,1}} \cdot \sigma_{0,1} \cdot CZ_{0,2} \cdot \sigma_{0,1} & \xrightarrow{S_{22}} \overline{\sigma_{1,2} \cdot Z_1 \cdot \sigma_{1,2}} \cdot \sigma_{1,2} \cdot CCX_{0,2} \cdot \sigma_{1,2} \\
\xrightarrow{E_4} \sigma_{0,1} \cdot Z_0 \cdot CZ_{0,2} \cdot \sigma_{0,1} & \xrightarrow{E_{10}} \sigma_{1,2} \cdot Z_1 \cdot CCX_{0,2} \cdot \sigma_{1,2} \\
\xleftarrow{C_{103}} \sigma_{0,1} \cdot \overline{CZ_{0,2} \cdot Z_0} \cdot \sigma_{0,1} & \xleftarrow{C_{40}} \sigma_{1,2} \cdot \overline{CCX_{0,2} \cdot CZ_{0,2} \cdot Z_1} \cdot \sigma_{1,2} \\
\xleftarrow{E_4} \sigma_{0,1} \cdot CZ_{0,2} \cdot \overline{\sigma_{0,1} \cdot \sigma_{0,1}} \cdot Z_0 \cdot \sigma_{0,1} & \xleftarrow{E_{10}} \sigma_{1,2} \cdot CCX_{0,2} \cdot CZ_{0,2} \cdot \overline{\sigma_{1,2} \cdot \sigma_{1,2}} \cdot Z_1 \cdot \sigma_{1,2} \\
\xleftarrow{(34)} \overline{\sigma_{0,1} \cdot CZ_{0,2} \cdot \sigma_{0,1}} \cdot \overline{Z_1} & \xleftarrow{S_{22}} \sigma_{1,2} \cdot CCX_{0,2} \cdot \overline{CZ_{0,2}} \cdot \sigma_{1,2} \cdot \overline{Z_2} \\
\xleftarrow{(19)} \overline{CZ_{1,2}} \cdot Z_1 & \xleftarrow{(18)} \sigma_{1,2} \cdot CCX_{0,2} \cdot \overline{\sigma_{1,2} \cdot CZ_{0,1} \cdot \sigma_{1,2}} \cdot Z_2 \\
& \xleftarrow{E_{10}} \sigma_{1,2} \cdot CCX_{0,2} \cdot \overline{\sigma_{1,2}} \cdot CZ_{0,1} \cdot Z_2 \\
& \xleftarrow{(33)} \overline{CCX_{0,1}} \cdot CZ_{0,1} \cdot Z_2
\end{array}$$

## 1.2 Some Global Phase Lemmas

A global phase is a multiple of  $I$ . Since  $O(8, \mathbb{D})$  is a real matrix group, where all matrices have operator norm 1, it follows that the only global phase in  $O(8, \mathbb{D})$  is  $-I$ . It can be shown that  $-I = X_j \cdot Z_j \cdot X_j \cdot Z_j$  for all  $j \in \{0, 1, 2\}$ . Since  $-I$  is in the center of  $O(8, \mathbb{D})$ , then  $-I$  commutes with all generators in  $\Sigma_D$ . These facts prove useful in deriving the relations in  $R_{D(E8)}$  and  $R_{E8(D)}$ . To this end, we consider the relation  $(-I) \approx X_0 \cdot Z_0 \cdot X_0 \cdot Z_0$ , henceforth referred to as relation  $P_1$ . By Theorems B.6 and Theorem B.11 in the main paper, we can freely introduce and eliminate  $P_1$  for the purposes of the remaining proofs.

$$\begin{array}{ll}
(\gamma_2) : (-I) \cdot X_1 \xrightarrow{P_1} \overline{X_0 \cdot Z_0 \cdot X_0 \cdot Z_0} \cdot X_1 & (\gamma_3) : (-I) \cdot X_2 \xrightarrow{P_1} \overline{X_0 \cdot Z_0 \cdot X_0 \cdot Z_0} \cdot X_2 \\
\xleftarrow{B_{15}} X_0 \cdot Z_0 \cdot X_0 \cdot \overline{X_1} \cdot \overline{Z_0} & \xleftarrow{B_{23}} X_0 \cdot Z_0 \cdot X_0 \cdot \overline{X_2} \cdot \overline{Z_0} \\
\xrightarrow{B_2} X_0 \cdot Z_0 \cdot \overline{X_1} \cdot \overline{X_0} \cdot Z_0 & \xrightarrow{B_{13}} X_0 \cdot Z_0 \cdot \overline{X_2} \cdot \overline{X_0} \cdot Z_0 \\
\xleftarrow{B_{15}} X_0 \cdot \overline{X_1} \cdot \overline{Z_0} \cdot X_0 \cdot Z_0 & \xleftarrow{B_{23}} X_0 \cdot \overline{X_2} \cdot \overline{Z_0} \cdot X_0 \cdot Z_0 \\
\xrightarrow{B_2} \overline{X_1 \cdot X_0 \cdot Z_0 \cdot X_0 \cdot Z_0} \xleftarrow{P_1} X_1 \cdot \overline{(-I)} & \xrightarrow{B_{13}} \overline{X_2 \cdot X_0 \cdot Z_0 \cdot X_0 \cdot Z_0} \xleftarrow{P_1} X_2 \cdot \overline{(-I)} \\
\\
(\gamma_4) : (-I) \cdot CX_{0,1} \xrightarrow{P_1} \overline{X_0 \cdot Z_0 \cdot X_0 \cdot Z_0} \cdot CX_{0,1} & (\gamma_5) : (-I) \cdot CX_{1,0} \xrightarrow{P_1} \overline{X_0 \cdot Z_0 \cdot X_0 \cdot Z_0} \cdot CX_{1,0} \\
\xleftarrow{C_{85}} X_0 \cdot Z_0 \cdot X_0 \cdot \overline{CX_{0,1}} \cdot \overline{Z_0} & \xleftarrow{C_{32}} X_0 \cdot Z_0 \cdot X_0 \cdot \overline{CX_{1,0}} \cdot \overline{Z_1} \cdot \overline{Z_0} \\
\xrightarrow{C_3} X_0 \cdot Z_0 \cdot \overline{CX_{0,1}} \cdot \overline{X_1} \cdot \overline{X_0} \cdot Z_0 & \xrightarrow{(38)} X_0 \cdot Z_0 \cdot \overline{CX_{1,0}} \cdot \overline{X_0} \cdot \overline{Z_1} \cdot \overline{Z_0} \\
\xleftarrow{C_{85}} X_0 \cdot \overline{CX_{0,1}} \cdot \overline{Z_0} \cdot X_1 \cdot X_0 \cdot Z_0 & \xleftarrow{C_{32}} X_0 \cdot \overline{CX_{1,0}} \cdot \overline{Z_1} \cdot \overline{Z_0} \cdot X_0 \cdot \overline{Z_1} \cdot \overline{Z_0} \\
\xrightarrow{C_3} \overline{CX_{0,1} \cdot X_1 \cdot X_0 \cdot Z_0 \cdot X_1} \cdot X_0 \cdot Z_0 & \xrightarrow{(38)} \overline{CX_{1,0} \cdot X_0 \cdot Z_0 \cdot X_1 \cdot X_0 \cdot Z_0} \\
\xleftarrow{B_{15}} CX_{0,1} \cdot X_1 \cdot X_0 \cdot \overline{X_1} \cdot \overline{Z_0} \cdot X_0 \cdot Z_0 & \xleftarrow{B_{29}} CX_{1,0} \cdot X_0 \cdot \overline{Z_0} \cdot \overline{X_1} \cdot \overline{X_0} \cdot \overline{Z_1} \cdot \overline{Z_0} \\
\xleftarrow{B_2} CX_{0,1} \cdot \overline{X_0} \cdot \overline{X_1} \cdot \overline{X_1} \cdot \overline{Z_0} \cdot X_0 \cdot Z_0 & \xleftarrow{B_{14}} CX_{1,0} \cdot X_0 \cdot Z_0 \cdot \overline{X_0} \cdot \overline{Z_1} \cdot \overline{Z_0} \\
\xrightarrow{E_{13}} CX_{0,1} \cdot \overline{X_0 \cdot Z_0 \cdot X_0 \cdot Z_0} \xleftarrow{P_1} CX_{0,1} \cdot \overline{(-I)} & \xrightarrow{E_5} CX_{1,0} \cdot \overline{X_0 \cdot Z_0 \cdot X_0 \cdot Z_0} \xleftarrow{P_1} CX_{1,0} \cdot \overline{(-I)}
\end{array}$$

$$\begin{aligned}
(\gamma_6) : & \underline{(-I)} \cdot Z_1 \xrightarrow{P_1} \overline{X_0 \cdot Z_0 \cdot X_0 \cdot Z_0 \cdot Z_1} \\
& \xrightarrow{B_{29}} X_0 \cdot Z_0 \cdot \underline{X_0 \cdot Z_1 \cdot Z_0} \\
& \xrightarrow{B_{14}} X_0 \cdot \underline{Z_0 \cdot Z_1 \cdot X_0} \cdot Z_0 \\
& \xrightarrow{B_{29}} \underline{X_0 \cdot Z_1 \cdot Z_0} \cdot X_0 \cdot Z_0 \\
& \xrightarrow{B_{14}} \overline{Z_1 \cdot X_0 \cdot Z_0 \cdot X_0 \cdot Z_0} \\
& \xleftarrow{P_1} Z_1 \cdot \overline{(-I)} \\
(\gamma_7) : & \underline{(-I)} \cdot K_{1,2} \xrightarrow{P_1} \overline{X_0 \cdot Z_0 \cdot X_0 \cdot Z_0 \cdot K_{1,2}} \\
& \xrightarrow{B_6} X_0 \cdot Z_0 \cdot \underline{X_0 \cdot K_{1,2} \cdot Z_0} \\
& \xrightarrow{(27)} X_0 \cdot \underline{Z_0 \cdot K_{1,2} \cdot X_0} \cdot Z_0 \\
& \xrightarrow{B_6} \underline{X_0 \cdot K_{1,2} \cdot Z_0} \cdot X_0 \cdot Z_0 \\
& \xrightarrow{(27)} \overline{K_{1,2} \cdot X_0 \cdot Z_0 \cdot X_0 \cdot Z_0} \\
& \xleftarrow{P_1} K_{1,2} \cdot \overline{(-I)} \\
(\gamma_8) : & \underline{(-I)} \xleftarrow{E_4} \overline{\sigma_{0,1} \cdot \sigma_{0,1}} \cdot \underline{(-I)} \xrightarrow{(13)} \sigma_{0,1} \cdot \overline{CX_{0,1} \cdot CX_{1,0} \cdot CX_{0,1}} \cdot \underline{(-I)} \xleftarrow{\gamma_4} \sigma_{0,1} \cdot CX_{0,1} \cdot \underline{CX_{1,0} \cdot \overline{(-I)} \cdot CX_{0,1}} \\
& \xleftarrow{\gamma_5} \sigma_{0,1} \cdot \underline{CX_{0,1} \cdot \overline{(-I)} \cdot CX_{1,0}} \cdot CX_{0,1} \\
& \xleftarrow{\gamma_4} \sigma_{0,1} \cdot \overline{(-I) \cdot CX_{0,1} \cdot CX_{1,0} \cdot CX_{0,1}} \\
& \xleftarrow{(13)} \sigma_{0,1} \cdot \underline{(-I) \cdot \overline{\sigma_{0,1}}} \\
& \xrightarrow{P_1} \sigma_{0,1} \cdot \overline{X_0 \cdot Z_0 \cdot X_0 \cdot Z_0} \cdot \sigma_{0,1} \\
& \xleftarrow{E_4} \sigma_{0,1} \cdot X_0 \cdot Z_0 \cdot X_0 \cdot \overline{\sigma_{0,1} \cdot \sigma_{0,1}} \cdot Z_0 \cdot \sigma_{0,1} \\
& \xleftarrow{E_4} \sigma_{0,1} \cdot X_0 \cdot Z_0 \cdot \overline{\sigma_{0,1} \cdot \sigma_{0,1}} \cdot X_0 \cdot \sigma_{0,1} \cdot \sigma_{0,1} \cdot Z_0 \cdot \sigma_{0,1} \\
& \xleftarrow{E_4} \underline{\sigma_{0,1} \cdot X_0 \cdot \overline{\sigma_{0,1} \cdot \sigma_{0,1}}} \cdot Z_0 \cdot \sigma_{0,1} \cdot \sigma_{0,1} \cdot X_0 \cdot \sigma_{0,1} \cdot \sigma_{0,1} \cdot Z_0 \cdot \sigma_{0,1} \\
& \xleftarrow{(28)} \overline{X_1 \cdot \sigma_{0,1} \cdot Z_0 \cdot \sigma_{0,1} \cdot \sigma_{0,1} \cdot X_0 \cdot \sigma_{0,1} \cdot \sigma_{0,1} \cdot Z_0 \cdot \sigma_{0,1}} \\
& \xleftarrow{(34)} X_1 \cdot \overline{Z_1 \cdot \sigma_{0,1} \cdot X_0 \cdot \sigma_{0,1}} \cdot \sigma_{0,1} \cdot Z_0 \cdot \sigma_{0,1} \\
& \xleftarrow{(28)} X_1 \cdot Z_1 \cdot \overline{X_1 \cdot \sigma_{0,1} \cdot Z_0 \cdot \sigma_{0,1}} \xleftarrow{(34)} X_1 \cdot Z_1 \cdot X_1 \cdot \overline{Z_1} \\
(\gamma_9) : & \underline{(-I)} \cdot CX_{0,2} \xrightarrow{\gamma_8} \overline{X_1 \cdot Z_1 \cdot X_1 \cdot Z_1 \cdot CX_{0,2}} \\
& \xrightarrow{B_{10}} X_1 \cdot Z_1 \cdot \underline{X_1 \cdot CX_{0,2} \cdot Z_1} \\
& \xleftarrow{B_3} X_1 \cdot \underline{Z_1 \cdot CX_{0,2} \cdot X_1} \cdot Z_1 \\
& \xrightarrow{B_{10}} \underline{X_1 \cdot CX_{0,2} \cdot Z_1} \cdot X_1 \cdot Z_1 \\
& \xleftarrow{B_3} \overline{CX_{0,2} \cdot X_1 \cdot Z_1 \cdot X_1 \cdot Z_1} \xleftarrow{\gamma_8} CX_{0,2} \cdot \overline{(-I)} \\
(\gamma_{10}) : & \underline{(-I)} \cdot CX_{2,0} \xrightarrow{\gamma_8} \overline{X_1 \cdot Z_1 \cdot X_1 \cdot Z_1 \cdot CX_{2,0}} \\
& \xrightarrow{B_9} X_1 \cdot Z_1 \cdot \underline{X_1 \cdot CX_{2,0} \cdot Z_1} \\
& \xleftarrow{B_4} X_1 \cdot \underline{Z_1 \cdot CX_{2,0} \cdot X_1} \cdot Z_1 \\
& \xrightarrow{B_9} \underline{X_1 \cdot CX_{2,0} \cdot Z_1} \cdot X_1 \cdot Z_1 \\
& \xleftarrow{B_4} \overline{CX_{2,0} \cdot X_1 \cdot Z_1 \cdot X_1 \cdot Z_1} \xleftarrow{\gamma_8} CX_{2,0} \cdot \overline{(-I)} \\
(\gamma_{11}) : & X_1 \cdot Z_1 \xleftarrow{E_{13}} X_1 \cdot Z_1 \cdot \overline{X_1 \cdot X_1} \xleftarrow{E_5} \underline{X_1 \cdot Z_1 \cdot X_1 \cdot Z_1 \cdot Z_1} \cdot X_1 \xleftarrow{\gamma_8} \overline{(-I)} \cdot Z_1 \cdot X_1 \\
(\gamma_{12}) : & \underline{(-I)} \cdot \underline{(-I)} \xrightarrow{\gamma_8} \underline{(-I) \cdot \overline{X_1 \cdot Z_1 \cdot X_1 \cdot Z_1}} \xrightarrow{\gamma_2} \overline{X_1 \cdot \underline{(-I)} \cdot Z_1 \cdot X_1 \cdot Z_1} \xleftarrow{\gamma_{11}} \underline{X_1 \cdot \overline{X_1} \cdot Z_1 \cdot Z_1} \xrightarrow{E_{13}} \underline{Z_1 \cdot Z_1} \xrightarrow{E_5} \varepsilon \\
(\gamma_{13}) : & Z_1 \cdot X_1 \xleftarrow{E_{13}} \overline{X_1 \cdot X_1 \cdot Z_1 \cdot X_1} \xrightarrow{\gamma_{11}} X_1 \cdot \overline{(-I) \cdot Z_1 \cdot X_1 \cdot X_1} \xrightarrow{E_{13}} X_1 \cdot \underline{(-I) \cdot Z_1} \xleftarrow{\gamma_6} X_1 \cdot \overline{Z_1 \cdot (-I)}
\end{aligned}$$

$$\begin{aligned}
(\gamma_{14}) : (-I) &\xleftarrow{E_{16}} \overline{\sigma_{0,2} \cdot \sigma_{0,2}} \cdot (-I) \xrightarrow{(10)} \sigma_{0,2} \cdot \overline{CX_{0,2} \cdot CX_{2,0} \cdot CX_{0,2}} \cdot (-I) \xleftarrow{\gamma_9} \sigma_{0,2} \cdot CX_{0,2} \cdot \overline{CX_{2,0} \cdot (-I) \cdot CX_{0,2}} \\
&\xleftarrow{\gamma_{10}} \sigma_{0,2} \cdot \overline{CX_{0,2} \cdot (-I) \cdot CX_{2,0}} \cdot CX_{0,2} \\
&\xleftarrow{\gamma_9} \sigma_{0,2} \cdot \overline{(-I) \cdot CX_{0,2} \cdot CX_{2,0} \cdot CX_{0,2}} \\
&\xleftarrow{(10)} \sigma_{0,2} \cdot \overline{(-I) \cdot \sigma_{0,2}} \\
&\xrightarrow{P_1} \sigma_{0,2} \cdot \overline{X_0 \cdot Z_0 \cdot X_0 \cdot Z_0} \cdot \sigma_{0,2} \\
&\xleftarrow{E_{16}} \sigma_{0,2} \cdot X_0 \cdot Z_0 \cdot X_0 \cdot \overline{\sigma_{0,2} \cdot \sigma_{0,2}} \cdot Z_0 \cdot \sigma_{0,2} \\
&\xleftarrow{E_{16}} \sigma_{0,2} \cdot X_0 \cdot Z_0 \cdot \overline{\sigma_{0,2} \cdot \sigma_{0,2}} \cdot X_0 \cdot \sigma_{0,2} \cdot \sigma_{0,2} \cdot Z_0 \cdot \sigma_{0,2} \\
&\xleftarrow{E_{16}} \sigma_{0,2} \cdot X_0 \cdot \overline{\sigma_{0,2} \cdot \sigma_{0,2}} \cdot Z_0 \cdot \sigma_{0,2} \cdot \sigma_{0,2} \cdot X_0 \cdot \sigma_{0,2} \cdot \sigma_{0,2} \cdot Z_0 \cdot \sigma_{0,2} \\
&\xleftarrow{(15)} \overline{X_2} \cdot \overline{\sigma_{0,2} \cdot Z_0 \cdot \sigma_{0,2}} \cdot \sigma_{0,2} \cdot X_0 \cdot \sigma_{0,2} \cdot \sigma_{0,2} \cdot Z_0 \cdot \sigma_{0,2} \\
&\xleftarrow{(16)} X_2 \cdot \overline{Z_2} \cdot \overline{\sigma_{0,2} \cdot X_0 \cdot \sigma_{0,2}} \cdot \sigma_{0,2} \cdot Z_0 \cdot \sigma_{0,2} \\
&\xleftarrow{(15)} X_2 \cdot Z_2 \cdot \overline{X_2} \cdot \overline{\sigma_{0,2} \cdot Z_0 \cdot \sigma_{0,2}} \\
&\xleftarrow{(16)} X_2 \cdot Z_2 \cdot X_2 \cdot \overline{Z_2}
\end{aligned}$$

$$\begin{aligned}
(\gamma_{15}) : (-I) \cdot CZ_{0,1} &\xrightarrow{\gamma_{14}} \overline{X_2 \cdot Z_2 \cdot X_2 \cdot Z_2} \cdot CZ_{0,1} \\
&\xleftarrow{B_{27}} X_2 \cdot Z_2 \cdot X_2 \cdot \overline{CZ_{0,1}} \cdot Z_2 \\
&\xrightarrow{B_{37}} X_2 \cdot Z_2 \cdot \overline{CZ_{0,1}} \cdot X_2 \cdot Z_2 \\
&\xleftarrow{B_{27}} X_2 \cdot \overline{CZ_{0,1}} \cdot Z_2 \cdot X_2 \cdot Z_2 \\
&\xrightarrow{B_{37}} \overline{CZ_{0,1}} \cdot X_2 \cdot Z_2 \cdot X_2 \cdot Z_2 \\
&\xleftarrow{\gamma_{14}} CZ_{0,1} \cdot \overline{(-I)}
\end{aligned}
\qquad
\begin{aligned}
(\gamma_{16}) : (-I) \cdot CZ_{0,2} &\xrightarrow{\gamma_8} \overline{X_1 \cdot Z_1 \cdot X_1 \cdot Z_1} \cdot CZ_{0,2} \\
&\xleftarrow{B_{20}} X_1 \cdot Z_1 \cdot X_1 \cdot \overline{CZ_{0,2}} \cdot Z_1 \\
&\xrightarrow{B_{35}} X_1 \cdot Z_1 \cdot \overline{CZ_{0,2}} \cdot X_1 \cdot Z_1 \\
&\xleftarrow{B_{20}} X_1 \cdot \overline{CZ_{0,2}} \cdot Z_1 \cdot X_1 \cdot Z_1 \\
&\xrightarrow{B_{35}} \overline{CZ_{0,2}} \cdot X_1 \cdot Z_1 \cdot X_1 \cdot Z_1 \\
&\xleftarrow{\gamma_8} CZ_{0,2} \cdot \overline{(-I)}
\end{aligned}$$

$$\begin{aligned}
(\gamma_{17}) : (-I) \cdot CCX_{1,2} &\xrightarrow{P_1} \overline{X_0 \cdot Z_0 \cdot X_0 \cdot Z_0} \cdot CCX_{1,2} \xrightarrow{C_{49}} X_0 \cdot Z_0 \cdot X_0 \cdot \overline{CCX_{1,2}} \cdot \overline{CZ_{1,2}} \cdot Z_0 \\
&\xrightarrow{(37)} X_0 \cdot Z_0 \cdot \overline{CCX_{1,2}} \cdot X_0 \cdot CZ_{1,2} \cdot Z_0 \\
&\xrightarrow{C_{49}} X_0 \cdot \overline{CCX_{1,2}} \cdot \overline{CZ_{1,2}} \cdot Z_0 \cdot X_0 \cdot CZ_{1,2} \cdot Z_0 \\
&\xrightarrow{B_{31}} X_0 \cdot CCX_{1,2} \cdot \overline{Z_0 \cdot \overline{CZ_{1,2}} \cdot X_0} \cdot CZ_{1,2} \cdot Z_0 \\
&\xleftarrow{B_{36}} X_0 \cdot CCX_{1,2} \cdot Z_0 \cdot \overline{X_0 \cdot \overline{CZ_{1,2}} \cdot CZ_{1,2}} \cdot Z_0 \\
&\xrightarrow{E_{12}} X_0 \cdot \overline{CCX_{1,2}} \cdot Z_0 \cdot X_0 \cdot Z_0 \\
&\xrightarrow{(37)} \overline{CCX_{1,2} \cdot X_0 \cdot Z_0 \cdot X_0 \cdot Z_0} \\
&\xleftarrow{P_1} CCX_{1,2} \cdot \overline{(-I)}
\end{aligned}$$

$$\begin{aligned}
(\gamma_{18}) : & \underline{(-I)} \cdot CCX_{0,1} \xrightarrow{\gamma_{14}} \overline{X_2 \cdot Z_2 \cdot X_2 \cdot Z_2} \cdot CCX_{0,1} \xrightarrow{(32)} X_2 \cdot Z_2 \cdot X_2 \cdot \underline{Z_2} \cdot \overline{\sigma_{0,2} \cdot CCX_{1,2} \cdot \sigma_{0,2}} \\
& \xrightarrow{(16)} X_2 \cdot Z_2 \cdot \underline{X_2} \cdot \overline{\sigma_{0,2} \cdot Z_0 \cdot \sigma_{0,2} \cdot \sigma_{0,2} \cdot CCX_{1,2} \cdot \sigma_{0,2}} \\
& \xrightarrow{(15)} X_2 \cdot \underline{Z_2} \cdot \overline{\sigma_{0,2} \cdot X_0 \cdot \sigma_{0,2} \cdot \sigma_{0,2} \cdot Z_0 \cdot \sigma_{0,2} \cdot \sigma_{0,2} \cdot CCX_{1,2} \cdot \sigma_{0,2}} \\
& \xrightarrow{(16)} \underline{X_2} \cdot \overline{\sigma_{0,2} \cdot Z_0 \cdot \sigma_{0,2} \cdot \sigma_{0,2} \cdot X_0 \cdot \sigma_{0,2} \cdot \sigma_{0,2} \cdot Z_0 \cdot \sigma_{0,2} \cdot \sigma_{0,2} \cdot CCX_{1,2} \cdot \sigma_{0,2}} \\
& \xrightarrow{(15)} \overline{\sigma_{0,2} \cdot X_0 \cdot \sigma_{0,2} \cdot \sigma_{0,2} \cdot Z_0 \cdot \sigma_{0,2} \cdot \sigma_{0,2} \cdot X_0 \cdot \sigma_{0,2} \cdot \sigma_{0,2} \cdot Z_0 \cdot \underline{\sigma_{0,2} \cdot \sigma_{0,2}} \cdot CCX_{1,2} \cdot \sigma_{0,2}} \\
& \xrightarrow{E_{16}} \sigma_{0,2} \cdot X_0 \cdot \sigma_{0,2} \cdot \sigma_{0,2} \cdot Z_0 \cdot \sigma_{0,2} \cdot \sigma_{0,2} \cdot X_0 \cdot \underline{\sigma_{0,2} \cdot \sigma_{0,2}} \cdot Z_0 \cdot CCX_{1,2} \cdot \sigma_{0,2} \\
& \xrightarrow{E_{16}} \sigma_{0,2} \cdot X_0 \cdot \sigma_{0,2} \cdot \sigma_{0,2} \cdot Z_0 \cdot \underline{\sigma_{0,2} \cdot \sigma_{0,2}} \cdot X_0 \cdot Z_0 \cdot CCX_{1,2} \cdot \sigma_{0,2} \\
& \xrightarrow{E_{16}} \sigma_{0,2} \cdot X_0 \cdot \underline{\sigma_{0,2} \cdot \sigma_{0,2}} \cdot Z_0 \cdot X_0 \cdot Z_0 \cdot CCX_{1,2} \cdot \sigma_{0,2} \\
& \xrightarrow{E_{16}} \sigma_{0,2} \cdot \underline{X_0 \cdot Z_0 \cdot X_0 \cdot Z_0} \cdot CCX_{1,2} \cdot \sigma_{0,2} \\
& \xleftarrow{P_1} \sigma_{0,2} \cdot \underline{(-I)} \cdot CCX_{1,2} \cdot \sigma_{0,2} \xrightarrow{\gamma_{17}} \sigma_{0,2} \cdot \overline{CCX_{1,2} \cdot (-I)} \cdot \sigma_{0,2} \\
& \xrightarrow{P_1} \sigma_{0,2} \cdot CCX_{1,2} \cdot \overline{X_0 \cdot Z_0 \cdot X_0 \cdot Z_0} \cdot \sigma_{0,2} \\
& \xleftarrow{E_{16}} \sigma_{0,2} \cdot CCX_{1,2} \cdot X_0 \cdot Z_0 \cdot X_0 \cdot \overline{\sigma_{0,2} \cdot \sigma_{0,2}} \cdot Z_0 \cdot \sigma_{0,2} \\
& \xleftarrow{E_{16}} \sigma_{0,2} \cdot CCX_{1,2} \cdot X_0 \cdot Z_0 \cdot \overline{\sigma_{0,2} \cdot \sigma_{0,2}} \cdot X_0 \cdot \sigma_{0,2} \cdot \sigma_{0,2} \cdot Z_0 \cdot \sigma_{0,2} \\
& \xleftarrow{E_{16}} \sigma_{0,2} \cdot CCX_{1,2} \cdot X_0 \cdot \overline{\sigma_{0,2} \cdot \sigma_{0,2}} \cdot Z_0 \cdot \sigma_{0,2} \cdot \sigma_{0,2} \cdot X_0 \cdot \sigma_{0,2} \cdot \sigma_{0,2} \cdot Z_0 \cdot \sigma_{0,2} \\
& \xleftarrow{E_{16}} \sigma_{0,2} \cdot CCX_{1,2} \cdot \overline{\sigma_{0,2} \cdot \sigma_{0,2}} \cdot X_0 \cdot \sigma_{0,2} \cdot \sigma_{0,2} \cdot Z_0 \cdot \sigma_{0,2} \cdot \sigma_{0,2} \cdot X_0 \cdot \sigma_{0,2} \cdot \underline{\sigma_{0,2} \cdot \sigma_{0,2}} \cdot Z_0 \cdot \sigma_{0,2} \\
& \xleftarrow{(16)} \sigma_{0,2} \cdot CCX_{1,2} \cdot \sigma_{0,2} \cdot \sigma_{0,2} \cdot X_0 \cdot \sigma_{0,2} \cdot \sigma_{0,2} \cdot Z_0 \cdot \sigma_{0,2} \cdot \underline{\sigma_{0,2} \cdot X_0 \cdot \sigma_{0,2}} \cdot \overline{Z_2} \\
& \xleftarrow{(15)} \sigma_{0,2} \cdot CCX_{1,2} \cdot \sigma_{0,2} \cdot \sigma_{0,2} \cdot X_0 \cdot \sigma_{0,2} \cdot \underline{\sigma_{0,2} \cdot Z_0 \cdot \sigma_{0,2}} \cdot \overline{X_2} \cdot Z_2 \\
& \xleftarrow{(16)} \sigma_{0,2} \cdot CCX_{1,2} \cdot \sigma_{0,2} \cdot \underline{\sigma_{0,2} \cdot X_0 \cdot \sigma_{0,2}} \cdot \overline{Z_2} \cdot X_2 \cdot Z_2 \\
& \xleftarrow{(15)} \sigma_{0,2} \cdot CCX_{1,2} \cdot \sigma_{0,2} \cdot \overline{X_2} \cdot Z_2 \cdot X_2 \cdot Z_2 \\
& \xleftarrow{(32)} \overline{CCX_{0,1} \cdot X_2 \cdot Z_2 \cdot X_2 \cdot Z_2} \xleftarrow{\gamma_{14}} CCX_{0,1} \cdot \overline{(-I)}
\end{aligned}$$

### 1.3 Some Control Manipulation Lemmas

The following two relation families are commonly used when working with controls.

1. **Control Elimination.** Let  $M$  and  $N$  be any two operators acting on the same number of qubits. If  $M$  is self-inverse, then  $CM_{j,k} \circ CN_{j,k} \circ CM_{j,k} = M_k \circ CN_{j,k} \circ M_k$ . This is because, either wire  $j$  is in state  $|0\rangle$ , and the  $M_k$  operators will cancel out as if they were controlled, or the wire  $j$  is in state  $|1\rangle$  and the  $M_k$  operators would be applied even if the controls were still present.
2. **Control Flip.** Let  $M$  be any  $n$ -fold controlled  $X$ -gate. Since  $\sigma_{j,k} = CX_{j,k} \circ CX_{k,j} \circ CX_{j,k}$  and  $\sigma_{j,k} = CX_{k,j} \circ CX_{j,k} \circ CX_{k,j}$ , then  $CM_{j,k} \circ CM_{k,j} \circ CX_{j,M}$  and  $CM_{k,j} \circ CM_{j,k} \circ CM_{k,j}$  are  $n$ -fold controlled  $\sigma_{j,k}$  operators, with the same controls. Therefore,  $CM_{j,k} \circ CM_{k,j} \circ CX_{j,M} = CM_{k,j} \circ CM_{j,k} \circ CM_{k,j}$ .

Careful inspection reveals that instances of control elimination and control flip follow immediately from (45) and (46). The remaining instances can be derived via symmetry relations. In this section, some instances of control elimination and control flips are derived which help to eliminate  $R_{D(E8)}$  and  $R_{E8(D)}$ .

$$(\chi_1) : CX_{0,1} \cdot \underline{CCX_{1,2} \cdot CX_{0,1}} \xrightarrow{(45)} CX_{0,1} \cdot \overline{CX_{0,1} \cdot CCX_{0,2} \cdot CCX_{1,2} \cdot CCX_{0,2}} \xrightarrow{(22)} CCX_{0,2} \cdot CCX_{1,2} \cdot CCX_{0,2}$$

$$\begin{aligned}
(\chi_2) : & \underline{CX_{1,0}} \cdot \overline{CCX_{0,1}} \cdot CX_{1,0} \\
& \xrightarrow{C_{72}} \overline{\overline{CCX_{0,1}} \cdot CX_{1,2} \cdot \underline{CX_{1,0}} \cdot CX_{1,0}} \\
& \xleftarrow{E_1} CCX_{0,1} \cdot CX_{1,2} \\
& \xleftarrow{(21)} \overline{X_0 \cdot X_0 \cdot CCX_{0,1}} \cdot CX_{1,2} \\
& \xrightarrow{(42)} X_0 \cdot \overline{\overline{CCX_{0,1}} \cdot CX_{1,2} \cdot X_0} \cdot CX_{1,2} \\
& \xrightarrow{(26)} X_0 \cdot CCX_{0,1} \cdot \overline{X_0 \cdot CX_{1,2}} \cdot CX_{1,2} \xrightarrow{E_8} X_0 \cdot CCX_{0,1} \cdot X_0 \\
(\chi_4) : & CX_{0,2} \cdot CCX_{1,2} \cdot \underline{CX_{0,2}} \xrightarrow{(9)} \underline{CX_{0,2}} \cdot CCX_{1,2} \cdot \overline{\sigma_{1,2} \cdot CX_{0,1} \cdot \sigma_{1,2}} \xrightarrow{(9)} \overline{\sigma_{1,2} \cdot CX_{0,1} \cdot \sigma_{1,2}} \cdot CCX_{1,2} \cdot \underline{\sigma_{1,2} \cdot CX_{0,1} \cdot \sigma_{1,2}} \\
& \xleftarrow{S_{20}} \sigma_{1,2} \cdot \underline{CX_{0,1} \cdot \overline{CCX_{1,2}}} \cdot CX_{0,1} \cdot \sigma_{1,2} \\
& \xrightarrow{X_1} \sigma_{1,2} \cdot \overline{CCX_{0,2} \cdot \underline{CCX_{1,2}}} \cdot \overline{CCX_{0,2}} \cdot \sigma_{1,2} \\
& \xrightarrow{S_{20}} \sigma_{1,2} \cdot CCX_{0,2} \cdot \overline{\sigma_{1,2} \cdot \underline{CCX_{1,2}}} \cdot \underline{\sigma_{1,2} \cdot CCX_{0,2}} \cdot \sigma_{1,2} \\
& \xleftarrow{(33)} \underline{\sigma_{1,2} \cdot CCX_{0,2} \cdot \sigma_{1,2}} \cdot CCX_{1,2} \cdot \overline{CCX_{0,1}} \xleftarrow{(33)} \overline{CCX_{0,1}} \cdot CCX_{1,2} \cdot CCX_{0,1} \\
(\chi_5) : & CX_{2,0} \cdot CCX_{0,1} \cdot \underline{CX_{2,0}} \xrightarrow{(29)} \underline{CX_{2,0}} \cdot CCX_{0,1} \cdot \overline{\sigma_{0,2} \cdot CX_{0,2} \cdot \sigma_{0,2}} \xrightarrow{(29)} \overline{\sigma_{0,2} \cdot CX_{0,2} \cdot \sigma_{0,2}} \cdot \underline{CCX_{0,1}} \cdot \sigma_{0,2} \cdot CX_{0,2} \cdot \sigma_{0,2} \\
& \xrightarrow{(32)} \sigma_{0,2} \cdot CX_{0,2} \cdot \sigma_{0,2} \cdot \overline{\sigma_{0,2} \cdot \underline{CCX_{1,2}}} \cdot \underline{\sigma_{0,2} \cdot \sigma_{0,2}} \cdot CX_{0,2} \cdot \sigma_{0,2} \\
& \xrightarrow{E_{16}} \sigma_{0,2} \cdot CX_{0,2} \cdot \underline{\sigma_{0,2} \cdot \sigma_{0,2}} \cdot \underline{CCX_{1,2}} \cdot CX_{0,2} \cdot \sigma_{0,2} \\
& \xrightarrow{E_{16}} \sigma_{0,2} \cdot \underline{CX_{0,2} \cdot CCX_{1,2}} \cdot \underline{CX_{0,2}} \cdot \sigma_{0,2} \\
& \xrightarrow{X_4} \sigma_{0,2} \cdot \overline{CCX_{0,1} \cdot \underline{CCX_{1,2}}} \cdot \underline{CCX_{0,1}} \cdot \sigma_{0,2} \\
& \xrightarrow{(32)} \sigma_{0,2} \cdot \underline{CCX_{0,1}} \cdot CCX_{1,2} \cdot \overline{\sigma_{0,2} \cdot \underline{CCX_{1,2}}} \cdot \sigma_{0,2} \cdot \sigma_{0,2} \\
& \xrightarrow{(32)} \sigma_{0,2} \cdot \overline{\sigma_{0,2} \cdot \underline{CCX_{1,2}}} \cdot \sigma_{0,2} \cdot CCX_{1,2} \cdot \sigma_{0,2} \cdot \underline{CCX_{1,2}} \cdot \underline{\sigma_{0,2} \cdot \sigma_{0,2}} \\
& \xrightarrow{E_{16}} \underline{\sigma_{0,2} \cdot \sigma_{0,2}} \cdot CCX_{1,2} \cdot \sigma_{0,2} \cdot CCX_{1,2} \cdot \sigma_{0,2} \cdot \underline{CCX_{1,2}} \\
& \xrightarrow{E_{16}} CCX_{1,2} \cdot \underline{\sigma_{0,2} \cdot \underline{CCX_{1,2}}} \cdot \sigma_{0,2} \cdot \underline{CCX_{1,2}} \\
& \xleftarrow{(32)} CCX_{1,2} \cdot \overline{CCX_{0,1}} \cdot CCX_{1,2} \\
(\chi_6) : & CX_{2,1} \cdot \overline{CCX_{0,1}} \cdot \underline{CX_{2,1}} \\
& \xrightarrow{(31)} \underline{CX_{2,1}} \cdot \overline{CCX_{0,1} \cdot \sigma_{0,1} \cdot CX_{2,0} \cdot \sigma_{0,1}} \\
& \xrightarrow{(31)} \overline{\sigma_{0,1} \cdot CX_{2,0} \cdot \sigma_{0,1}} \cdot \underline{CCX_{0,1} \cdot \sigma_{0,1}} \cdot CX_{2,0} \cdot \sigma_{0,1} \\
& \xleftarrow{S_{17}} \sigma_{0,1} \cdot \underline{CX_{2,0} \cdot \overline{CCX_{0,1}}} \cdot CX_{2,0} \cdot \sigma_{0,1} \\
& \xrightarrow{X_5} \sigma_{0,1} \cdot \overline{CCX_{1,2} \cdot \underline{CCX_{0,1}}} \cdot \underline{CCX_{1,2}} \cdot \sigma_{0,1} \\
& \xrightarrow{S_{17}} \sigma_{0,1} \cdot CCX_{1,2} \cdot \overline{\sigma_{0,1} \cdot \underline{CCX_{0,1}}} \cdot \underline{\sigma_{0,1} \cdot CCX_{1,2}} \cdot \sigma_{0,1} \\
& \xleftarrow{(14)} \underline{\sigma_{0,1} \cdot \underline{CCX_{1,2}} \cdot \sigma_{0,1}} \cdot \underline{CCX_{0,1} \cdot \overline{CCX_{0,2}}} \\
& \xleftarrow{(14)} \overline{CCX_{0,2}} \cdot CCX_{0,1} \cdot \underline{CCX_{0,2}} \\
(\chi_7) : & CX_{1,2} \cdot \overline{CCX_{0,2}} \cdot \underline{CX_{1,2}} \\
& \xrightarrow{(7)} \underline{CX_{1,2}} \cdot \overline{CCX_{0,2} \cdot K_{1,2} \cdot CX_{2,1} \cdot K_{1,2}} \\
& \xrightarrow{(7)} \overline{K_{1,2} \cdot CX_{2,1} \cdot K_{1,2}} \cdot \underline{CCX_{0,2} \cdot K_{1,2} \cdot CX_{2,1} \cdot K_{1,2}} \\
& \xleftarrow{(17)} K_{1,2} \cdot \underline{CX_{2,1} \cdot \overline{CCX_{0,1}}} \cdot CX_{2,1} \cdot K_{1,2} \\
& \xrightarrow{X_6} K_{1,2} \cdot \overline{CCX_{0,2} \cdot \underline{CCX_{0,1}}} \cdot \underline{CCX_{0,2}} \cdot K_{1,2} \\
& \xrightarrow{(17)} K_{1,2} \cdot \underline{CCX_{0,2} \cdot K_{1,2}} \cdot \overline{CCX_{0,2} \cdot K_{1,2}} \cdot \underline{CCX_{0,2} \cdot K_{1,2}} \\
& \xleftarrow{(17)} \underline{K_{1,2} \cdot \underline{CCX_{0,2}} \cdot K_{1,2}} \cdot \underline{CCX_{0,2} \cdot \overline{CCX_{0,1}}} \\
& \xleftarrow{(17)} \overline{CCX_{0,1}} \cdot \underline{CCX_{0,2}} \cdot \underline{CCX_{0,1}}
\end{aligned}$$

$$\begin{aligned}
(\chi_8) : CX_{1,0} \cdot CCX_{0,2} \cdot CX_{1,0} &\xleftarrow{E_4} CX_{1,0} \cdot \underline{CCX_{0,2}} \cdot CX_{1,0} \cdot \overline{\sigma_{0,1} \cdot \sigma_{0,1}} \xrightarrow{(14)} CX_{1,0} \cdot \overline{\sigma_{0,1} \cdot CCX_{1,2} \cdot \sigma_{0,1}} \cdot CX_{1,0} \cdot \sigma_{0,1} \cdot \sigma_{0,1} \\
&\xleftarrow{E_4} \overline{\sigma_{0,1} \cdot \sigma_{0,1}} \cdot CX_{1,0} \cdot \sigma_{0,1} \cdot CCX_{1,2} \cdot \underline{\sigma_{0,1} \cdot CX_{1,0} \cdot \sigma_{0,1}} \cdot \sigma_{0,1} \\
&\xleftarrow{S_1} \sigma_{0,1} \cdot \underline{\sigma_{0,1} \cdot CX_{1,0} \cdot \sigma_{0,1}} \cdot CCX_{1,2} \cdot \overline{CX_{0,1}} \cdot \sigma_{0,1} \\
&\xleftarrow{S_1} \sigma_{0,1} \cdot \overline{CX_{0,1}} \cdot CCX_{1,2} \cdot CX_{0,1} \cdot \sigma_{0,1} \\
&\xrightarrow{\chi_1} \sigma_{0,1} \cdot \overline{CCX_{0,2} \cdot CCX_{1,2} \cdot \underline{CCX_{0,2}}} \cdot \sigma_{0,1} \\
&\xrightarrow{(14)} \sigma_{0,1} \cdot \underline{CCX_{0,2}} \cdot CCX_{1,2} \cdot \overline{\sigma_{0,1} \cdot CCX_{1,2} \cdot \sigma_{0,1}} \cdot \sigma_{0,1} \\
&\xrightarrow{(14)} \sigma_{0,1} \cdot \overline{\sigma_{0,1} \cdot \overline{CCX_{1,2} \cdot \sigma_{0,1}}} \cdot CCX_{1,2} \cdot \sigma_{0,1} \cdot CCX_{1,2} \cdot \underline{\sigma_{0,1} \cdot \sigma_{0,1}} \\
&\xrightarrow{E_4} \sigma_{0,1} \cdot \underline{\sigma_{0,1}} \cdot CCX_{1,2} \cdot \sigma_{0,1} \cdot CCX_{1,2} \cdot \sigma_{0,1} \cdot CCX_{1,2} \\
&\xrightarrow{E_4} CCX_{1,2} \cdot \underline{\sigma_{0,1} \cdot CCX_{1,2} \cdot \sigma_{0,1}} \cdot CCX_{1,2} \\
&\xleftarrow{(14)} CCX_{1,2} \cdot \overline{CCX_{0,2}} \cdot CCX_{1,2}
\end{aligned}$$

$$(\chi_9) : CCX_{0,2} \cdot \underline{CCX_{0,1} \cdot CCX_{0,2}} \xrightarrow{(46)} \underline{CCX_{0,2} \cdot \overline{CCX_{0,2}}} \cdot CCX_{0,1} \cdot CCX_{0,2} \cdot CCX_{0,1} \xrightarrow{E_7} CCX_{0,1} \cdot CCX_{0,2} \cdot CCX_{0,1}$$

$$(\chi_{10}) : \underline{CX_{2,1} \cdot CCX_{0,1} \cdot CX_{2,1}} \xrightarrow{\chi_6} \underline{CCX_{0,2} \cdot CCX_{0,1} \cdot CCX_{0,2}} \xrightarrow{\chi_9} \underline{CCX_{0,1} \cdot CCX_{0,2} \cdot CCX_{0,1}} \xleftarrow{\chi_7} \overline{CX_{1,2} \cdot CCX_{0,2} \cdot CX_{1,2}}$$

$$\begin{aligned}
(\chi_{11}) : CCX_{0,1} \cdot CCX_{1,2} \cdot \underline{CCX_{0,1}} &\xrightarrow{S_{17}} \underline{CCX_{0,1} \cdot CCX_{1,2} \cdot \overline{\sigma_{0,1} \cdot CCX_{0,1} \cdot \sigma_{0,1}}} \xrightarrow{S_{17}} \overline{\sigma_{0,1} \cdot CCX_{0,1} \cdot \sigma_{0,1}} \cdot CCX_{1,2} \cdot \sigma_{0,1} \cdot CCX_{0,1} \cdot \sigma_{0,1} \\
&\xleftarrow{(14)} \sigma_{0,1} \cdot \underline{CCX_{0,1} \cdot \overline{CCX_{0,2}}} \cdot CCX_{0,1} \cdot \sigma_{0,1} \\
&\xleftarrow{\chi_9} \sigma_{0,1} \cdot \overline{CCX_{0,2} \cdot CCX_{0,1} \cdot \underline{CCX_{0,2}}} \cdot \sigma_{0,1} \\
&\xrightarrow{(14)} \sigma_{0,1} \cdot \underline{CCX_{0,2}} \cdot CCX_{0,1} \cdot \overline{\sigma_{0,1} \cdot CCX_{1,2} \cdot \sigma_{0,1}} \cdot \sigma_{0,1} \\
&\xrightarrow{(14)} \sigma_{0,1} \cdot \overline{\sigma_{0,1} \cdot CCX_{1,2} \cdot \underline{\sigma_{0,1} \cdot CCX_{0,1} \cdot \sigma_{0,1}}} \cdot CCX_{1,2} \cdot \sigma_{0,1} \cdot \sigma_{0,1} \\
&\xleftarrow{S_{17}} \sigma_{0,1} \cdot \sigma_{0,1} \cdot CCX_{1,2} \cdot \overline{CCX_{0,1}} \cdot CCX_{1,2} \cdot \underline{\sigma_{0,1} \cdot \sigma_{0,1}} \\
&\xrightarrow{E_4} \underline{\sigma_{0,1} \cdot \sigma_{0,1}} \cdot CCX_{1,2} \cdot CCX_{0,1} \cdot CCX_{1,2} \\
&\xrightarrow{E_4} CCX_{1,2} \cdot CCX_{0,1} \cdot CCX_{1,2}
\end{aligned}$$

$$\begin{aligned}
(\chi_{12}) : CCX_{0,2} \cdot CCX_{1,2} \cdot CCX_{0,2} &\xleftarrow{E_{10}} CCX_{0,2} \cdot \underline{CCX_{1,2}} \cdot CCX_{0,2} \cdot \overline{\sigma_{1,2} \cdot \sigma_{1,2}} \xrightarrow{S_{20}} CCX_{0,2} \cdot \overline{\sigma_{1,2} \cdot \overline{CCX_{1,2} \cdot \sigma_{1,2}}} \cdot CCX_{0,2} \cdot \sigma_{1,2} \cdot \sigma_{1,2} \\
&\xleftarrow{E_{10}} \overline{\sigma_{1,2} \cdot \sigma_{1,2}} \cdot CCX_{0,2} \cdot \sigma_{1,2} \cdot CCX_{1,2} \cdot \underline{\sigma_{1,2} \cdot CCX_{0,2} \cdot \sigma_{1,2}} \cdot \sigma_{1,2} \\
&\xleftarrow{(33)} \sigma_{1,2} \cdot \underline{\sigma_{1,2} \cdot CCX_{0,2} \cdot \sigma_{1,2}} \cdot CCX_{1,2} \cdot \overline{CCX_{0,1}} \cdot \sigma_{1,2} \\
&\xleftarrow{(33)} \sigma_{1,2} \cdot \overline{CCX_{0,1}} \cdot CCX_{1,2} \cdot CCX_{0,1} \cdot \sigma_{1,2} \\
&\xrightarrow{\chi_{11}} \sigma_{1,2} \cdot \overline{CCX_{1,2} \cdot \underline{CCX_{0,1} \cdot CCX_{1,2}}} \cdot \sigma_{1,2} \\
&\xrightarrow{(33)} \sigma_{1,2} \cdot CCX_{1,2} \cdot \overline{\sigma_{1,2} \cdot \overline{CCX_{0,2} \cdot \sigma_{1,2}}} \cdot CCX_{1,2} \cdot \sigma_{1,2} \\
&\xleftarrow{S_{20}} \underline{\sigma_{1,2} \cdot CCX_{1,2} \cdot \sigma_{1,2}} \cdot CCX_{0,2} \cdot \overline{CCX_{1,2}} \\
&\xleftarrow{S_{20}} \overline{CCX_{1,2}} \cdot CCX_{0,2} \cdot CCX_{1,2}
\end{aligned}$$

### 1.4 Some Lemmas to Eliminate the Circuit Definitions

This section derives lemmas to aid in the elimination of relations from  $R_{D(E8)}$ . The  $n$ -th lemma in this section is denoted  $\omega_n$ . From this section onward, the circuit decomposition for each  $r_j$  will be denoted  $D_j$  (see Section 4.1 in the main paper). Furthermore, the defining relation for each  $w_j$  in Appendix D of the main paper will be denoted  $W_j$ . Since  $W_1$  through to  $W_{13}$  induce an acyclic derived generator graph, then these generators can be freely introduced and eliminated by Theorem B.6 and Theorem B.11 of the main paper. Furthermore, when a word over  $\{w_1, \dots, w_{13}\}$  is eliminated, then a word over  $\{r_1, \dots, r_8\}$  is obtained.

$$\begin{aligned}
(\omega_1) : r_6 \cdot r_7 &\xrightarrow{D_7} r_6 \cdot \overline{CZ_{0,1} \cdot CX_{2,1} \cdot CCX_{0,1} \cdot CX_{2,1} \cdot CZ_{0,1}} \\
&\xrightarrow{D_6} \overline{CX_{2,1} \cdot CCX_{0,1} \cdot CX_{2,1}} \cdot CZ_{0,1} \cdot CX_{2,1} \cdot CCX_{0,1} \cdot CX_{2,1} \cdot CZ_{0,1} \\
&\xrightarrow{X_6} \overline{CCX_{0,2} \cdot CCX_{0,1} \cdot CCX_{0,2}} \cdot CZ_{0,1} \cdot \overline{CX_{2,1} \cdot CCX_{0,1} \cdot CX_{2,1}} \cdot CZ_{0,1} \\
&\xrightarrow{X_6} \overline{CCX_{0,2} \cdot CCX_{0,1} \cdot CCX_{0,2}} \cdot \overline{CZ_{0,1} \cdot CCX_{0,2} \cdot CCX_{0,1} \cdot CCX_{0,2}} \cdot CZ_{0,1} \\
&\xrightarrow{C_{80}} \overline{CCX_{0,2} \cdot CCX_{0,1} \cdot CCX_{0,2}} \cdot \overline{CCX_{0,2} \cdot CZ_{0,1} \cdot CZ_{0,2} \cdot CCX_{0,1} \cdot CCX_{0,2} \cdot CZ_{0,1}} \\
&\xrightarrow{C_{81}} \overline{CCX_{0,2} \cdot CCX_{0,1} \cdot CCX_{0,2} \cdot CCX_{0,2} \cdot CZ_{0,1} \cdot \overline{CCX_{0,1} \cdot CZ_{0,1} \cdot CZ_{0,2}}} \cdot CCX_{0,2} \cdot CZ_{0,1} \\
&\xrightarrow{C_{60}} \overline{CCX_{0,2} \cdot CCX_{0,1} \cdot CCX_{0,2} \cdot CCX_{0,2} \cdot CZ_{0,1} \cdot CCX_{0,1} \cdot \overline{CZ_{0,2} \cdot CZ_{0,1} \cdot CCX_{0,2}}} \cdot CZ_{0,1} \\
&\xrightarrow{C_{80}} \overline{CCX_{0,2} \cdot CCX_{0,1} \cdot CCX_{0,2} \cdot CCX_{0,2} \cdot CZ_{0,1} \cdot CCX_{0,1} \cdot CZ_{0,2} \cdot \overline{CCX_{0,2} \cdot CZ_{0,1} \cdot CZ_{0,2}}} \cdot CZ_{0,1} \\
&\xrightarrow{C_{60}} \overline{CCX_{0,2} \cdot CCX_{0,1} \cdot CCX_{0,2} \cdot CCX_{0,2} \cdot CZ_{0,1} \cdot CCX_{0,1} \cdot \overline{CZ_{0,2} \cdot CCX_{0,2} \cdot CZ_{0,2} \cdot CZ_{0,1}}} \cdot CZ_{0,1} \\
&\xrightarrow{C_{96}} \overline{CCX_{0,2} \cdot CCX_{0,1} \cdot CCX_{0,2} \cdot CCX_{0,2} \cdot CZ_{0,1} \cdot CCX_{0,1} \cdot \overline{CCX_{0,2} \cdot CZ_{0,2} \cdot CZ_{0,2} \cdot CZ_{0,1} \cdot CZ_{0,1}}} \\
&\xrightarrow{E_{11}} \overline{CCX_{0,2} \cdot CCX_{0,1} \cdot CCX_{0,2} \cdot CCX_{0,2} \cdot \overline{CZ_{0,1} \cdot CCX_{0,1} \cdot CCX_{0,2} \cdot CZ_{0,1} \cdot CZ_{0,1}}} \\
&\xrightarrow{C_{95}} \overline{CCX_{0,2} \cdot CCX_{0,1} \cdot CCX_{0,2} \cdot CCX_{0,2} \cdot \overline{CCX_{0,1} \cdot CZ_{0,1} \cdot CCX_{0,2} \cdot CZ_{0,1} \cdot CZ_{0,1}}} \\
&\xrightarrow{C_{80}} \overline{CCX_{0,2} \cdot CCX_{0,1} \cdot CCX_{0,2} \cdot CCX_{0,2} \cdot CCX_{0,1} \cdot \overline{CCX_{0,2} \cdot CZ_{0,1} \cdot CZ_{0,2}}} \cdot CZ_{0,1} \cdot CZ_{0,1} \\
&\xrightarrow{C_{60}} \overline{CCX_{0,2} \cdot CCX_{0,1} \cdot CCX_{0,2} \cdot CCX_{0,2} \cdot CCX_{0,1} \cdot CCX_{0,2} \cdot \overline{CZ_{0,2} \cdot CZ_{0,1} \cdot CZ_{0,1}}} \cdot CZ_{0,1} \\
&\xrightarrow{E_2} \overline{CCX_{0,2} \cdot CCX_{0,1} \cdot \overline{CCX_{0,2} \cdot CCX_{0,2}}} \cdot CCX_{0,1} \cdot CCX_{0,2} \cdot CZ_{0,2} \cdot CZ_{0,1} \\
&\xrightarrow{E_7} \overline{CCX_{0,2} \cdot \overline{CCX_{0,1} \cdot CCX_{0,1}}} \cdot CCX_{0,2} \cdot CZ_{0,2} \cdot CZ_{0,1} \\
&\xrightarrow{E_{18}} \overline{CCX_{0,2} \cdot CCX_{0,2}} \cdot CZ_{0,2} \cdot CZ_{0,1} \xrightarrow{E_7} \overline{CZ_{0,2} \cdot CZ_{0,1}}
\end{aligned}$$

$$\begin{aligned}
(\omega_2) : r_3 &\xrightarrow{D_3} \overline{X_0 \cdot CCX_{0,1} \cdot X_0} \xleftarrow{C_{56}} \overline{X_0 \cdot X_0 \cdot CX_{1,2} \cdot CCX_{0,1}} \xrightarrow{(21)} CX_{1,2} \cdot CCX_{0,1} \\
(\omega_3) : w_1 &\xrightarrow{W_1} \overline{r_6 \cdot r_7} \xrightarrow{\omega_1} \overline{CZ_{0,2} \cdot CZ_{0,1}}
\end{aligned}$$

$$\begin{aligned}
(\omega_4) : r_2 \cdot r_3 &\xrightarrow{D_3} r_2 \cdot \overline{X_0 \cdot CCX_{0,1} \cdot X_0} \xrightarrow{D_2} \overline{X_0 \cdot CX_{2,1} \cdot CCX_{0,1} \cdot CX_{2,1} \cdot X_0} \cdot X_0 \cdot CCX_{0,1} \cdot X_0 \\
&\xrightarrow{(21)} X_0 \cdot CX_{2,1} \cdot CCX_{0,1} \cdot CX_{2,1} \cdot CCX_{0,1} \cdot X_0 \\
&\xrightarrow{X_6} X_0 \cdot \overline{CCX_{0,2} \cdot CCX_{0,1} \cdot CCX_{0,2}} \cdot CCX_{0,1} \cdot X_0 \\
&\xrightarrow{X_9} X_0 \cdot \overline{CCX_{0,1} \cdot CCX_{0,2} \cdot CCX_{0,1} \cdot CCX_{0,1}} \cdot X_0 \\
&\xrightarrow{E_{18}} X_0 \cdot CCX_{0,1} \cdot CCX_{0,2} \cdot X_0
\end{aligned}$$

$$\begin{aligned}
(\omega_5) : \underline{w_2} &\xrightarrow{w_2} r_6 \cdot r_5 \cdot \underline{w_1} \cdot r_5 \cdot r_6 \xrightarrow{\omega_3} r_6 \cdot r_5 \cdot \overline{CZ_{0,2} \cdot CZ_{0,1}} \cdot r_5 \cdot r_6 \\
&\xrightarrow{D_6} r_6 \cdot \overline{X_1 \cdot CCX_{0,1} \cdot X_1} \cdot CZ_{0,2} \cdot CZ_{0,1} \cdot r_5 \cdot r_6 \\
&\xrightarrow{D_6} \overline{CX_{2,1} \cdot CCX_{0,1} \cdot CX_{2,1}} \cdot X_1 \cdot CCX_{0,1} \cdot X_1 \cdot CZ_{0,2} \cdot CZ_{0,1} \cdot r_5 \cdot r_6 \\
&\xleftarrow{E_{13}} \overline{X_1 \cdot X_1 \cdot CX_{2,1} \cdot CCX_{0,1} \cdot CX_{2,1} \cdot X_1 \cdot CCX_{0,1} \cdot X_1} \cdot CZ_{0,2} \cdot CZ_{0,1} \cdot r_5 \cdot r_6 \\
&\xleftarrow{E_2} X_1 \cdot \overline{CZ_{0,1} \cdot CZ_{0,1}} \cdot X_1 \cdot CX_{2,1} \cdot CCX_{0,1} \cdot CX_{2,1} \cdot X_1 \cdot CCX_{0,1} \cdot X_1 \cdot CZ_{0,2} \cdot CZ_{0,1} \cdot r_5 \cdot r_6 \\
&\xleftarrow{C_{112}} X_1 \cdot CZ_{0,1} \cdot \overline{X_1 \cdot Z_0 \cdot CZ_{0,1}} \cdot CX_{2,1} \cdot CCX_{0,1} \cdot CX_{2,1} \cdot X_1 \cdot CCX_{0,1} \cdot X_1 \cdot CZ_{0,2} \cdot CZ_{0,1} \cdot r_5 \cdot r_6 \\
&\xrightarrow{X_6} X_1 \cdot CZ_{0,1} \cdot X_1 \cdot Z_0 \cdot \overline{CZ_{0,1} \cdot CCX_{0,2} \cdot CCX_{0,1} \cdot CCX_{0,2}} \cdot X_1 \cdot CCX_{0,1} \cdot X_1 \cdot CZ_{0,2} \cdot CZ_{0,1} \cdot r_5 \cdot r_6 \\
&\xrightarrow{C_{80}} X_1 \cdot CZ_{0,1} \cdot X_1 \cdot Z_0 \cdot \overline{CCX_{0,2} \cdot CZ_{0,1} \cdot CZ_{0,2}} \cdot CCX_{0,1} \cdot CCX_{0,2} \cdot X_1 \cdot CCX_{0,1} \cdot X_1 \cdot CZ_{0,2} \cdot CZ_{0,1} \cdot r_5 \cdot r_6 \\
&\xrightarrow{C_{60}} X_1 \cdot CZ_{0,1} \cdot X_1 \cdot Z_0 \cdot CCX_{0,2} \cdot \overline{CZ_{0,2} \cdot CZ_{0,1}} \cdot CCX_{0,1} \cdot CCX_{0,2} \cdot X_1 \cdot CCX_{0,1} \cdot X_1 \cdot CZ_{0,2} \cdot CZ_{0,1} \cdot r_5 \cdot r_6 \\
&\xrightarrow{C_{110}} X_1 \cdot CZ_{0,1} \cdot X_1 \cdot Z_0 \cdot CCX_{0,2} \cdot \overline{CCX_{0,1} \cdot CZ_{0,2} \cdot CCX_{0,2}} \cdot X_1 \cdot CCX_{0,1} \cdot X_1 \cdot CZ_{0,2} \cdot CZ_{0,1} \cdot r_5 \cdot r_6 \\
&\xrightarrow{C_{96}} X_1 \cdot CZ_{0,1} \cdot X_1 \cdot Z_0 \cdot CCX_{0,2} \cdot CCX_{0,1} \cdot \overline{CCX_{0,2} \cdot CZ_{0,2}} \cdot X_1 \cdot CCX_{0,1} \cdot X_1 \cdot CZ_{0,2} \cdot CZ_{0,1} \cdot r_5 \cdot r_6 \\
&\xleftarrow{B_{35}} X_1 \cdot CZ_{0,1} \cdot X_1 \cdot Z_0 \cdot CCX_{0,2} \cdot CCX_{0,1} \cdot CCX_{0,2} \cdot \overline{X_1 \cdot CZ_{0,2}} \cdot CCX_{0,1} \cdot \overline{X_1 \cdot CZ_{0,2}} \cdot CZ_{0,1} \cdot r_5 \cdot r_6 \\
&\xrightarrow{B_{35}} X_1 \cdot CZ_{0,1} \cdot X_1 \cdot Z_0 \cdot CCX_{0,2} \cdot CCX_{0,1} \cdot CCX_{0,2} \cdot X_1 \cdot \overline{CZ_{0,2} \cdot CCX_{0,1}} \cdot \overline{CZ_{0,2} \cdot X_1} \cdot CZ_{0,1} \cdot r_5 \cdot r_6 \\
&\xrightarrow{C_{81}} X_1 \cdot CZ_{0,1} \cdot X_1 \cdot Z_0 \cdot CCX_{0,2} \cdot CCX_{0,1} \cdot CCX_{0,2} \cdot X_1 \cdot \overline{CCX_{0,1} \cdot CZ_{0,1} \cdot CZ_{0,2}} \cdot CZ_{0,2} \cdot X_1 \cdot CZ_{0,1} \cdot r_5 \cdot r_6 \\
&\xrightarrow{E_{11}} X_1 \cdot CZ_{0,1} \cdot X_1 \cdot Z_0 \cdot CCX_{0,2} \cdot CCX_{0,1} \cdot CCX_{0,2} \cdot X_1 \cdot CCX_{0,1} \cdot \overline{CZ_{0,1} \cdot X_1} \cdot CZ_{0,1} \cdot r_5 \cdot r_6 \\
&\xleftarrow{C_{112}} X_1 \cdot CZ_{0,1} \cdot X_1 \cdot Z_0 \cdot CCX_{0,2} \cdot CCX_{0,1} \cdot CCX_{0,2} \cdot X_1 \cdot CCX_{0,1} \cdot \overline{X_1 \cdot Z_0 \cdot CZ_{0,1} \cdot CZ_{0,1}} \cdot r_5 \cdot r_6 \\
&\xrightarrow{E_2} X_1 \cdot CZ_{0,1} \cdot X_1 \cdot Z_0 \cdot CCX_{0,2} \cdot CCX_{0,1} \cdot CCX_{0,2} \cdot \overline{X_1 \cdot CCX_{0,1}} \cdot X_1 \cdot Z_0 \cdot r_5 \cdot r_6 \\
&\xrightarrow{C_{35}} X_1 \cdot CZ_{0,1} \cdot X_1 \cdot Z_0 \cdot CCX_{0,2} \cdot CCX_{0,1} \cdot CCX_{0,2} \cdot \overline{CCX_{0,1} \cdot CX_{0,2} \cdot X_1 \cdot X_1} \cdot Z_0 \cdot r_5 \cdot r_6 \\
&\xrightarrow{E_{13}} X_1 \cdot CZ_{0,1} \cdot X_1 \cdot Z_0 \cdot \overline{CCX_{0,2} \cdot CCX_{0,1} \cdot CCX_{0,2}} \cdot CCX_{0,1} \cdot CX_{0,2} \cdot Z_0 \cdot r_5 \cdot r_6 \\
&\xrightarrow{X_9} X_1 \cdot CZ_{0,1} \cdot X_1 \cdot Z_0 \cdot \overline{CCX_{0,1} \cdot CCX_{0,2} \cdot CCX_{0,1} \cdot CCX_{0,1}} \cdot CX_{0,2} \cdot Z_0 \cdot r_5 \cdot r_6 \\
&\xrightarrow{E_{18}} X_1 \cdot CZ_{0,1} \cdot X_1 \cdot Z_0 \cdot \overline{CCX_{0,1}} \cdot CCX_{0,2} \cdot CX_{0,2} \cdot Z_0 \cdot r_5 \cdot r_6 \\
&\xrightarrow{C_{54}} X_1 \cdot CZ_{0,1} \cdot X_1 \cdot \overline{CCX_{0,1} \cdot Z_0} \cdot CCX_{0,2} \cdot CX_{0,2} \cdot Z_0 \cdot r_5 \cdot r_6 \\
&\xrightarrow{C_{58}} X_1 \cdot CZ_{0,1} \cdot X_1 \cdot CCX_{0,1} \cdot \overline{CCX_{0,2} \cdot Z_0} \cdot CX_{0,2} \cdot Z_0 \cdot r_5 \cdot r_6 \\
&\xrightarrow{C_{90}} X_1 \cdot CZ_{0,1} \cdot X_1 \cdot CCX_{0,1} \cdot CCX_{0,2} \cdot \overline{Z_0 \cdot Z_0} \cdot CX_{0,2} \cdot r_5 \cdot r_6 \\
&\xrightarrow{E_3} X_1 \cdot CZ_{0,1} \cdot X_1 \cdot CCX_{0,1} \cdot CCX_{0,2} \cdot CX_{0,2} \cdot r_5 \cdot r_6 \xrightarrow{D_6} X_1 \cdot CZ_{0,1} \cdot X_1 \cdot CCX_{0,1} \cdot CCX_{0,2} \cdot CX_{0,2} \cdot \overline{X_1 \cdot CCX_{0,1} \cdot X_1} \cdot r_6 \\
&\xrightarrow{C_{35}} X_1 \cdot CZ_{0,1} \cdot X_1 \cdot CCX_{0,1} \cdot CCX_{0,2} \cdot CX_{0,2} \cdot \overline{CCX_{0,1} \cdot CX_{0,2} \cdot X_1 \cdot X_1} \cdot r_6 \\
&\xrightarrow{E_{13}} X_1 \cdot CZ_{0,1} \cdot X_1 \cdot CCX_{0,1} \cdot CCX_{0,2} \cdot CX_{0,2} \cdot \overline{CCX_{0,1} \cdot CX_{0,2}} \cdot r_6 \\
&\xrightarrow{C_{105}} X_1 \cdot CZ_{0,1} \cdot X_1 \cdot CCX_{0,1} \cdot CCX_{0,2} \cdot \overline{CX_{0,2} \cdot CX_{0,2}} \cdot CCX_{0,1} \cdot r_6 \\
&\xrightarrow{E_{15}} X_1 \cdot CZ_{0,1} \cdot X_1 \cdot \overline{CCX_{0,1} \cdot CCX_{0,2} \cdot CCX_{0,1}} \cdot r_6 \xleftarrow{X_9} X_1 \cdot CZ_{0,1} \cdot X_1 \cdot \overline{CCX_{0,2} \cdot CCX_{0,1} \cdot CCX_{0,2}} \cdot r_6 \\
&\xleftarrow{X_6} X_1 \cdot CZ_{0,1} \cdot X_1 \cdot \overline{CX_{2,1} \cdot CCX_{0,1} \cdot CX_{2,1}} \cdot r_6 \xleftarrow{D_6} X_1 \cdot CZ_{0,1} \cdot X_1 \cdot \overline{r_6 \cdot r_6} \xrightarrow{(6,6)} X_1 \cdot CZ_{0,1} \cdot X_1
\end{aligned}$$

$$\begin{aligned}
(\omega_6) : CZ_{0,1} \cdot \underline{r_6} &\xrightarrow{D_6} \underline{CZ_{0,1} \cdot \overline{CX_{2,1}} \cdot CCX_{0,1} \cdot CX_{2,1}} \\
&\xrightarrow{C_{121}} \overline{CX_{2,1} \cdot CZ_{0,1} \cdot CZ_{0,2}} \cdot CCX_{0,1} \cdot CX_{2,1} \\
&\xrightarrow{C_{60}} CX_{2,1} \cdot \overline{CZ_{0,2} \cdot CZ_{0,1}} \cdot CCX_{0,1} \cdot CX_{2,1} \\
&\xrightarrow{C_{110}} CX_{2,1} \cdot \overline{CCX_{0,1} \cdot CZ_{0,2}} \cdot CX_{2,1} \\
&\xleftarrow{C_{66}} \underline{CX_{2,1} \cdot CCX_{0,1} \cdot \overline{CX_{2,1}} \cdot CZ_{0,2}} \xleftarrow{D_6} \underline{r_6} \cdot CZ_{0,2}
\end{aligned}
\qquad
\begin{aligned}
(\omega_7) : CZ_{0,2} \cdot r_6 &\xleftarrow{(6;6)} \underline{r_6 \cdot \overline{r_6} \cdot CZ_{0,2} \cdot r_6} \\
&\xleftarrow{E_2} r_6 \cdot \overline{CZ_{0,1} \cdot CZ_{0,1}} \cdot r_6 \cdot CZ_{0,2} \cdot r_6 \\
&\xrightarrow{\omega_6} r_6 \cdot CZ_{0,1} \cdot r_6 \cdot \overline{CZ_{0,2}} \cdot CZ_{0,2} \cdot r_6 \\
&\xrightarrow{E_{11}} r_6 \cdot CZ_{0,1} \cdot \underline{r_6 \cdot r_6} \xrightarrow{(6;6)} r_6 \cdot CZ_{0,1}
\end{aligned}$$

$$\begin{aligned}
(\omega_8) : r_4 \cdot \underline{r_5} &\xrightarrow{D_6} \underline{r_4} \cdot \overline{X_1 \cdot CCX_{0,1} \cdot X_1} \xrightarrow{D_4} \overline{CX_{0,1} \cdot CX_{0,2} \cdot CCX_{1,2} \cdot CX_{0,2} \cdot CX_{0,1}} \cdot X_1 \cdot CCX_{0,1} \cdot X_1 \\
&\xrightarrow{\chi_4} CX_{0,1} \cdot \overline{CCX_{0,1} \cdot CCX_{1,2} \cdot CCX_{0,1}} \cdot CX_{0,1} \cdot X_1 \cdot CCX_{0,1} \cdot X_1 \\
&\xrightarrow{\chi_{11}} CX_{0,1} \cdot \overline{CCX_{1,2} \cdot CCX_{0,1} \cdot CCX_{1,2}} \cdot CX_{0,1} \cdot X_1 \cdot CCX_{0,1} \cdot X_1 \\
&\xleftarrow{\chi_3} CX_{0,1} \cdot CCX_{1,2} \cdot CCX_{0,1} \cdot CCX_{1,2} \cdot \underline{CX_{0,1} \cdot \overline{CX_{0,1}} \cdot CCX_{0,1} \cdot \overline{CX_{0,1}}} \\
&\xrightarrow{(22)} CX_{0,1} \cdot CCX_{1,2} \cdot \underline{CCX_{0,1} \cdot CCX_{1,2} \cdot CCX_{0,1}} \cdot CX_{0,1} \\
&\xrightarrow{\chi_{11}} CX_{0,1} \cdot \underline{CCX_{1,2} \cdot \overline{CCX_{1,2}} \cdot CCX_{0,1} \cdot \overline{CCX_{1,2}}} \cdot CX_{0,1} \xrightarrow{(24)} CX_{0,1} \cdot CCX_{0,1} \cdot CCX_{1,2} \cdot CX_{0,1}
\end{aligned}$$

$$\begin{aligned}
(\omega_9) : X_1 \cdot \underline{r_4 \cdot r_5} &\xrightarrow{\omega_8} X_1 \cdot \overline{CX_{0,1} \cdot CCX_{0,1} \cdot CCX_{1,2} \cdot CX_{0,1}} \xleftarrow{(22)} X_1 \cdot CX_{0,1} \cdot CCX_{0,1} \cdot \overline{CX_{0,1} \cdot CX_{0,1}} \cdot CCX_{1,2} \cdot CX_{0,1} \\
&\xrightarrow{\chi_1} X_1 \cdot CX_{0,1} \cdot CCX_{0,1} \cdot CX_{0,1} \cdot \overline{CCX_{0,2} \cdot CCX_{1,2} \cdot CCX_{0,2}} \\
&\xrightarrow{\chi_{12}} X_1 \cdot \underline{CX_{0,1} \cdot CCX_{0,1} \cdot CX_{0,1}} \cdot \overline{CCX_{1,2} \cdot CCX_{0,2} \cdot CCX_{1,2}} \\
&\xrightarrow{\chi_3} X_1 \cdot \underline{X_1} \cdot \overline{CCX_{0,1} \cdot X_1} \cdot CCX_{1,2} \cdot CCX_{0,2} \cdot CCX_{1,2} \\
&\xrightarrow{E_{13}} CCX_{0,1} \cdot \underline{X_1 \cdot CCX_{1,2}} \cdot CCX_{0,2} \cdot CCX_{1,2} \\
&\xrightarrow{C_8} CCX_{0,1} \cdot \overline{CCX_{1,2} \cdot CX_{2,0} \cdot X_1} \cdot \underline{CCX_{0,2}} \cdot CCX_{1,2} \\
&\xrightarrow{C_{37}} CCX_{0,1} \cdot CCX_{1,2} \cdot CX_{2,0} \cdot \overline{CCX_{0,2} \cdot X_1} \cdot CCX_{1,2}
\end{aligned}$$

$$\begin{aligned}
(\omega_{10}) : CCX_{1,2} \cdot X_1 \cdot CCX_{0,2} \cdot CX_{2,0} \cdot CCX_{1,2} \cdot CCX_{0,1} \\
&\xleftarrow{(5;5)} \underline{r_5 \cdot r_5} \cdot CCX_{1,2} \cdot X_1 \cdot CCX_{0,2} \cdot CX_{2,0} \cdot CCX_{1,2} \cdot CCX_{0,1} \\
&\xleftarrow{(4;4)} r_5 \cdot \underline{r_4 \cdot r_4} \cdot r_5 \cdot CCX_{1,2} \cdot X_1 \cdot CCX_{0,2} \cdot CX_{2,0} \cdot CCX_{1,2} \cdot CCX_{0,1} \\
&\xleftarrow{E_{13}} r_5 \cdot r_4 \cdot \overline{X_1 \cdot X_1} \cdot r_4 \cdot r_5 \cdot CCX_{1,2} \cdot X_1 \cdot CCX_{0,2} \cdot CX_{2,0} \cdot CCX_{1,2} \cdot CCX_{0,1} \\
&\xrightarrow{\omega_9} r_5 \cdot r_4 \cdot X_1 \cdot \overline{CCX_{0,1} \cdot CCX_{1,2} \cdot CX_{2,0} \cdot CCX_{0,2} \cdot X_1 \cdot \underline{CCX_{1,2} \cdot CCX_{1,2}}} \cdot X_1 \cdot CCX_{0,2} \cdot CX_{2,0} \cdot CCX_{1,2} \cdot CCX_{0,1} \\
&\xrightarrow{(24)} r_5 \cdot r_4 \cdot X_1 \cdot CCX_{0,1} \cdot CCX_{1,2} \cdot CX_{2,0} \cdot CCX_{0,2} \cdot \underline{X_1 \cdot X_1} \cdot CCX_{0,2} \cdot CX_{2,0} \cdot CCX_{1,2} \cdot CCX_{0,1} \\
&\xrightarrow{E_{13}} r_5 \cdot r_4 \cdot X_1 \cdot CCX_{0,1} \cdot CCX_{1,2} \cdot CX_{2,0} \cdot \underline{CCX_{0,2} \cdot CCX_{0,2}} \cdot CX_{2,0} \cdot CCX_{1,2} \cdot CCX_{0,1} \\
&\xrightarrow{E_7} r_5 \cdot r_4 \cdot X_1 \cdot CCX_{0,1} \cdot CCX_{1,2} \cdot \underline{CX_{2,0} \cdot CX_{2,0}} \cdot CCX_{1,2} \cdot CCX_{0,1} \\
&\xrightarrow{E_{14}} r_5 \cdot r_4 \cdot X_1 \cdot CCX_{0,1} \cdot \underline{CCX_{1,2} \cdot CCX_{1,2}} \cdot CCX_{0,1} \\
&\xrightarrow{(24)} r_5 \cdot r_4 \cdot X_1 \cdot \underline{CCX_{0,1} \cdot CCX_{0,1}} \xrightarrow{E_{18}} r_5 \cdot r_4 \cdot X_1
\end{aligned}$$

$$\begin{aligned}
(\omega_{11}) : \underline{w_3} &\xrightarrow{W_3} \overline{r_5 \cdot r_4 \cdot \underline{w_2} \cdot r_4 \cdot r_5} \xrightarrow{\omega_5} r_5 \cdot r_4 \cdot \overline{X_1 \cdot CZ_{0,1} \cdot \underline{X_1} \cdot r_4 \cdot r_5} \\
&\xrightarrow{\omega_9} r_5 \cdot r_4 \cdot X_1 \cdot CZ_{0,1} \cdot \overline{CCX_{0,1} \cdot CCX_{1,2} \cdot CX_{2,0} \cdot CCX_{0,2} \cdot X_1 \cdot CCX_{1,2}} \\
&\xleftarrow{\omega_{10}} \overline{CCX_{1,2} \cdot X_1 \cdot CCX_{0,2} \cdot CX_{2,0} \cdot CCX_{1,2} \cdot CCX_{0,1} \cdot CZ_{0,1} \cdot CCX_{0,1} \cdot CCX_{1,2} \cdot CX_{2,0} \cdot CCX_{0,2} \cdot X_1 \cdot CCX_{1,2}} \\
&\xrightarrow{C_{95}} CCX_{1,2} \cdot X_1 \cdot CCX_{0,2} \cdot CX_{2,0} \cdot CCX_{1,2} \cdot \overline{CCX_{0,1} \cdot CCX_{0,1} \cdot CZ_{0,1}} \cdot CCX_{1,2} \cdot CX_{2,0} \cdot CCX_{0,2} \cdot X_1 \cdot CCX_{1,2} \\
&\xrightarrow{E_{18}} CCX_{1,2} \cdot X_1 \cdot CCX_{0,2} \cdot CX_{2,0} \cdot CCX_{1,2} \cdot \overline{CZ_{0,1} \cdot CCX_{1,2} \cdot CX_{2,0} \cdot CCX_{0,2} \cdot X_1 \cdot CCX_{1,2}} \\
&\xrightarrow{C_{77}} CCX_{1,2} \cdot X_1 \cdot CCX_{0,2} \cdot CX_{2,0} \cdot \overline{CCX_{1,2} \cdot CCX_{1,2} \cdot CZ_{1,2} \cdot CZ_{0,1} \cdot CX_{2,0} \cdot CCX_{0,2} \cdot X_1 \cdot CCX_{1,2}} \\
&\xrightarrow{(24)} CCX_{1,2} \cdot X_1 \cdot CCX_{0,2} \cdot CX_{2,0} \cdot \overline{CZ_{1,2} \cdot CZ_{0,1} \cdot CX_{2,0} \cdot CCX_{0,2} \cdot X_1 \cdot CCX_{1,2}} \\
&\xleftarrow{(40)} CCX_{1,2} \cdot X_1 \cdot CCX_{0,2} \cdot CX_{2,0} \cdot \overline{CZ_{0,1} \cdot CZ_{1,2} \cdot CX_{2,0} \cdot CCX_{0,2} \cdot X_1 \cdot CCX_{1,2}} \\
&\xleftarrow{C_{52}} CCX_{1,2} \cdot X_1 \cdot CCX_{0,2} \cdot \overline{CX_{2,0} \cdot CX_{2,0} \cdot CZ_{0,1}} \cdot CCX_{0,2} \cdot X_1 \cdot CCX_{1,2} \\
&\xrightarrow{E_{14}} CCX_{1,2} \cdot X_1 \cdot CCX_{0,2} \cdot CZ_{0,1} \cdot CCX_{0,2} \cdot X_1 \cdot CCX_{1,2} \\
\\
(\omega_{12}) : \underline{w_4} &\xrightarrow{W_4} \overline{r_4 \cdot r_3 \cdot \underline{w_3} \cdot r_3 \cdot r_4} \xrightarrow{\omega_{11}} r_4 \cdot r_3 \cdot \overline{CCX_{1,2} \cdot X_1 \cdot CCX_{0,2} \cdot CZ_{0,1} \cdot CCX_{0,2} \cdot X_1 \cdot CCX_{1,2} \cdot r_3 \cdot r_4} \\
&\xleftarrow{C_{37}} r_4 \cdot r_3 \cdot CCX_{1,2} \cdot X_1 \cdot \overline{CCX_{0,2} \cdot CZ_{0,1} \cdot X_1 \cdot CCX_{0,2}} \cdot CCX_{1,2} \cdot r_3 \cdot r_4 \\
&\xrightarrow{C_{37}} r_4 \cdot r_3 \cdot CCX_{1,2} \cdot \overline{CCX_{0,2} \cdot X_1 \cdot CZ_{0,1}} \cdot X_1 \cdot CCX_{0,2} \cdot CCX_{1,2} \cdot r_3 \cdot r_4 \\
&\xrightarrow{C_{70}} r_4 \cdot r_3 \cdot CCX_{1,2} \cdot CCX_{0,2} \cdot \overline{CZ_{0,1} \cdot Z_0 \cdot X_1 \cdot X_1 \cdot CCX_{0,2}} \cdot CCX_{1,2} \cdot r_3 \cdot r_4 \\
&\xrightarrow{E_{13}} r_4 \cdot r_3 \cdot CCX_{1,2} \cdot CCX_{0,2} \cdot CZ_{0,1} \cdot \overline{Z_0 \cdot CCX_{0,2} \cdot CCX_{1,2} \cdot r_3 \cdot r_4} \\
&\xrightarrow{C_{58}} r_4 \cdot r_3 \cdot CCX_{1,2} \cdot CCX_{0,2} \cdot \overline{CZ_{0,1} \cdot CCX_{0,2} \cdot Z_0} \cdot CCX_{1,2} \cdot r_3 \cdot r_4 \\
&\xrightarrow{C_{80}} r_4 \cdot r_3 \cdot CCX_{1,2} \cdot \overline{CCX_{0,2} \cdot CCX_{0,2} \cdot CZ_{0,1} \cdot CZ_{0,2}} \cdot Z_0 \cdot CCX_{1,2} \cdot r_3 \cdot r_4 \\
&\xrightarrow{E_7} r_4 \cdot r_3 \cdot CCX_{1,2} \cdot CZ_{0,1} \cdot CZ_{0,2} \cdot \overline{Z_0 \cdot CCX_{1,2} \cdot r_3 \cdot r_4} \\
&\xrightarrow{C_{49}} r_4 \cdot r_3 \cdot CCX_{1,2} \cdot CZ_{0,1} \cdot \overline{CZ_{0,2} \cdot CCX_{1,2} \cdot CZ_{1,2} \cdot Z_0} \cdot r_3 \cdot r_4 \\
&\xrightarrow{C_{100}} r_4 \cdot r_3 \cdot CCX_{1,2} \cdot CZ_{0,1} \cdot \overline{CCX_{1,2} \cdot CZ_{1,2} \cdot CZ_{0,2} \cdot CZ_{1,2}} \cdot Z_0 \cdot r_3 \cdot r_4 \\
&\xrightarrow{C_{71}} r_4 \cdot r_3 \cdot CCX_{1,2} \cdot CZ_{0,1} \cdot CCX_{1,2} \cdot \overline{CZ_{1,2} \cdot CZ_{1,2} \cdot CZ_{0,2}} \cdot Z_0 \cdot r_3 \cdot r_4 \\
&\xrightarrow{E_{12}} r_4 \cdot r_3 \cdot CCX_{1,2} \cdot \overline{CZ_{0,1} \cdot CCX_{1,2} \cdot CZ_{0,2} \cdot Z_0} \cdot r_3 \cdot r_4 \\
&\xrightarrow{C_{77}} r_4 \cdot r_3 \cdot \overline{CCX_{1,2} \cdot CCX_{1,2} \cdot CZ_{1,2} \cdot CZ_{0,1} \cdot CZ_{0,2} \cdot Z_0} \cdot r_3 \cdot r_4 \\
&\xrightarrow{(24)} r_4 \cdot r_3 \cdot CZ_{1,2} \cdot CZ_{0,1} \cdot CZ_{0,2} \cdot Z_0 \cdot \underline{r_3} \cdot r_4 \xrightarrow{\omega_2} r_4 \cdot \underline{r_3} \cdot CZ_{1,2} \cdot CZ_{0,1} \cdot CZ_{0,2} \cdot Z_0 \cdot \overline{CX_{1,2} \cdot CCX_{0,1}} \cdot r_4 \\
&\xrightarrow{\omega_2} r_4 \cdot \overline{CX_{1,2} \cdot CCX_{0,1}} \cdot CZ_{1,2} \cdot CZ_{0,1} \cdot CZ_{0,2} \cdot \underline{Z_0 \cdot CX_{1,2}} \cdot CCX_{0,1} \cdot r_4 \\
&\xrightarrow{B_7} r_4 \cdot CX_{1,2} \cdot CCX_{0,1} \cdot CZ_{1,2} \cdot CZ_{0,1} \cdot \overline{CZ_{0,2} \cdot CX_{1,2} \cdot Z_0} \cdot CCX_{0,1} \cdot r_4 \\
&\xrightarrow{C_{102}} r_4 \cdot CX_{1,2} \cdot CCX_{0,1} \cdot CZ_{1,2} \cdot CZ_{0,1} \cdot \overline{CX_{1,2} \cdot CZ_{0,1} \cdot CZ_{0,2}} \cdot Z_0 \cdot CCX_{0,1} \cdot r_4 \\
&\xrightarrow{C_{60}} r_4 \cdot CX_{1,2} \cdot CCX_{0,1} \cdot CZ_{1,2} \cdot \overline{CZ_{0,1} \cdot CX_{1,2} \cdot CZ_{0,2} \cdot CZ_{0,1}} \cdot Z_0 \cdot CCX_{0,1} \cdot r_4 \\
&\xleftarrow{C_{21}} r_4 \cdot CX_{1,2} \cdot CCX_{0,1} \cdot CZ_{1,2} \cdot \overline{CX_{1,2} \cdot CZ_{0,1} \cdot CZ_{0,2}} \cdot CZ_{0,1} \cdot Z_0 \cdot CCX_{0,1} \cdot r_4
\end{aligned}$$

$$\begin{aligned}
& \xrightarrow{C_{60}} r_4 \cdot CX_{1,2} \cdot CCX_{0,1} \cdot CZ_{1,2} \cdot CX_{1,2} \cdot \overline{CZ_{0,2}} \cdot \overline{CZ_{0,1}} \cdot CZ_{0,1} \cdot Z_0 \cdot CCX_{0,1} \cdot r_4 \\
& \xrightarrow{E_2} r_4 \cdot CX_{1,2} \cdot CCX_{0,1} \cdot CZ_{1,2} \cdot CX_{1,2} \cdot CZ_{0,2} \cdot Z_0 \cdot CCX_{0,1} \cdot r_4 \\
& \xleftarrow{E_{12}} r_4 \cdot CX_{1,2} \cdot CCX_{0,1} \cdot CZ_{1,2} \cdot \overline{CX_{1,2}} \cdot \overline{CZ_{1,2}} \cdot CZ_{0,2} \cdot Z_0 \cdot CCX_{0,1} \cdot r_4 \\
& \xleftarrow{C_{64}} r_4 \cdot CX_{1,2} \cdot CCX_{0,1} \cdot \overline{CZ_{1,2}} \cdot \overline{CZ_{1,2}} \cdot \overline{CX_{1,2}} \cdot CZ_{1,2} \cdot CZ_{0,2} \cdot Z_0 \cdot CCX_{0,1} \cdot r_4 \\
& \xrightarrow{E_{12}} r_4 \cdot CX_{1,2} \cdot CCX_{0,1} \cdot \overline{Z_1} \cdot CX_{1,2} \cdot CZ_{1,2} \cdot CZ_{0,2} \cdot Z_0 \cdot CCX_{0,1} \cdot r_4 \\
& \xleftarrow{C_{87}} r_4 \cdot CX_{1,2} \cdot CCX_{0,1} \cdot \overline{CX_{1,2}} \cdot \overline{Z_1} \cdot CZ_{1,2} \cdot CZ_{0,2} \cdot Z_0 \cdot CCX_{0,1} \cdot r_4 \\
& \xleftarrow{C_{107}} r_4 \cdot \overline{CCX_{0,1}} \cdot \overline{CX_{1,2}} \cdot CX_{1,2} \cdot Z_1 \cdot CZ_{1,2} \cdot CZ_{0,2} \cdot Z_0 \cdot CCX_{0,1} \cdot r_4 \\
& \xrightarrow{E_8} r_4 \cdot CCX_{0,1} \cdot Z_1 \cdot CZ_{1,2} \cdot CZ_{0,2} \cdot \overline{Z_0} \cdot \overline{CCX_{0,1}} \cdot r_4 \\
& \xrightarrow{C_{54}} r_4 \cdot CCX_{0,1} \cdot Z_1 \cdot CZ_{1,2} \cdot \overline{CZ_{0,2}} \cdot \overline{CCX_{0,1}} \cdot \overline{Z_0} \cdot r_4 \\
& \xrightarrow{C_{81}} r_4 \cdot CCX_{0,1} \cdot Z_1 \cdot CZ_{1,2} \cdot \overline{CCX_{0,1}} \cdot \overline{CZ_{0,1}} \cdot \overline{CZ_{0,2}} \cdot Z_0 \cdot r_4 \\
& \xrightarrow{C_{60}} r_4 \cdot CCX_{0,1} \cdot Z_1 \cdot \overline{CZ_{1,2}} \cdot \overline{CCX_{0,1}} \cdot \overline{CZ_{0,2}} \cdot \overline{CZ_{0,1}} \cdot Z_0 \cdot r_4 \\
& \xrightarrow{C_{82}} r_4 \cdot CCX_{0,1} \cdot Z_1 \cdot \overline{CCX_{0,1}} \cdot \overline{CZ_{0,1}} \cdot \overline{CZ_{1,2}} \cdot CZ_{0,2} \cdot CZ_{0,1} \cdot Z_0 \cdot r_4 \\
& \xrightarrow{(40)} r_4 \cdot CCX_{0,1} \cdot Z_1 \cdot CCX_{0,1} \cdot \overline{CZ_{1,2}} \cdot \overline{CZ_{0,1}} \cdot \overline{CZ_{0,2}} \cdot CZ_{0,1} \cdot Z_0 \cdot r_4 \\
& \xrightarrow{C_{60}} r_4 \cdot CCX_{0,1} \cdot Z_1 \cdot CCX_{0,1} \cdot CZ_{1,2} \cdot \overline{CZ_{0,2}} \cdot \overline{CZ_{0,1}} \cdot \overline{CZ_{0,2}} \cdot Z_0 \cdot r_4 \\
& \xrightarrow{E_2} r_4 \cdot CCX_{0,1} \cdot \overline{Z_1} \cdot \overline{CCX_{0,1}} \cdot CZ_{1,2} \cdot CZ_{0,2} \cdot Z_0 \cdot r_4 \\
& \xrightarrow{C_{47}} r_4 \cdot \overline{CCX_{0,1}} \cdot \overline{CCX_{0,1}} \cdot \overline{Z_1} \cdot CZ_{1,2} \cdot CZ_{0,2} \cdot Z_0 \cdot r_4 \xrightarrow{E_{18}} r_4 \cdot Z_1 \cdot CZ_{1,2} \cdot CZ_{0,2} \cdot Z_0 \cdot \overline{r_4} \\
& \xrightarrow{D_4} r_4 \cdot Z_1 \cdot CZ_{1,2} \cdot CZ_{0,2} \cdot \overline{Z_0} \cdot \overline{CX_{0,1}} \cdot \overline{CX_{0,2}} \cdot \overline{CCX_{1,2}} \cdot \overline{CX_{0,2}} \cdot \overline{CX_{0,1}} \\
& \xleftarrow{C_{85}} r_4 \cdot Z_1 \cdot CZ_{1,2} \cdot \overline{CZ_{0,2}} \cdot \overline{CX_{0,1}} \cdot \overline{Z_0} \cdot CX_{0,2} \cdot CCX_{1,2} \cdot CX_{0,2} \cdot CX_{0,1} \\
& \xleftarrow{C_{23}} r_4 \cdot Z_1 \cdot \overline{CZ_{1,2}} \cdot \overline{CX_{0,1}} \cdot \overline{CZ_{0,2}} \cdot Z_0 \cdot CX_{0,2} \cdot CCX_{1,2} \cdot CX_{0,2} \cdot CX_{0,1} \\
& \xrightarrow{C_{75}} r_4 \cdot Z_1 \cdot \overline{CX_{0,1}} \cdot \overline{CZ_{0,2}} \cdot \overline{CZ_{1,2}} \cdot CZ_{0,2} \cdot Z_0 \cdot CX_{0,2} \cdot CCX_{1,2} \cdot CX_{0,2} \cdot CX_{0,1} \\
& \xrightarrow{C_{71}} r_4 \cdot Z_1 \cdot CX_{0,1} \cdot \overline{CZ_{1,2}} \cdot \overline{CZ_{0,2}} \cdot \overline{CZ_{0,2}} \cdot Z_0 \cdot CX_{0,2} \cdot CCX_{1,2} \cdot CX_{0,2} \cdot CX_{0,1} \\
& \xrightarrow{E_{11}} r_4 \cdot Z_1 \cdot \overline{CX_{0,1}} \cdot CZ_{1,2} \cdot Z_0 \cdot CX_{0,2} \cdot CCX_{1,2} \cdot CX_{0,2} \cdot CX_{0,1} \\
& \xrightarrow{C_{68}} r_4 \cdot \overline{CX_{0,1}} \cdot \overline{Z_0} \cdot \overline{Z_1} \cdot CZ_{1,2} \cdot Z_0 \cdot CX_{0,2} \cdot CCX_{1,2} \cdot CX_{0,2} \cdot CX_{0,1} \\
& \xrightarrow{B_{29}} r_4 \cdot CX_{0,1} \cdot \overline{Z_1} \cdot \overline{Z_0} \cdot \overline{CZ_{1,2}} \cdot Z_0 \cdot CX_{0,2} \cdot CCX_{1,2} \cdot CX_{0,2} \cdot CX_{0,1} \\
& \xleftarrow{B_{31}} r_4 \cdot CX_{0,1} \cdot Z_1 \cdot \overline{CZ_{1,2}} \cdot \overline{Z_0} \cdot \overline{Z_0} \cdot CX_{0,2} \cdot CCX_{1,2} \cdot CX_{0,2} \cdot CX_{0,1} \\
& \xrightarrow{E_3} r_4 \cdot CX_{0,1} \cdot Z_1 \cdot \overline{CZ_{1,2}} \cdot \overline{CX_{0,2}} \cdot CCX_{1,2} \cdot CX_{0,2} \cdot CX_{0,1} \\
& \xrightarrow{C_{84}} r_4 \cdot CX_{0,1} \cdot \overline{Z_1} \cdot \overline{CX_{0,2}} \cdot \overline{CZ_{0,1}} \cdot \overline{CZ_{1,2}} \cdot CCX_{1,2} \cdot CX_{0,2} \cdot CX_{0,1} \\
& \xrightarrow{B_{10}} r_4 \cdot CX_{0,1} \cdot \overline{CX_{0,2}} \cdot \overline{Z_1} \cdot CZ_{0,1} \cdot \overline{CZ_{1,2}} \cdot \overline{CCX_{1,2}} \cdot CX_{0,2} \cdot CX_{0,1} \\
& \xrightarrow{C_{97}} r_4 \cdot CX_{0,1} \cdot CX_{0,2} \cdot Z_1 \cdot \overline{CZ_{0,1}} \cdot \overline{CCX_{1,2}} \cdot \overline{CZ_{1,2}} \cdot CX_{0,2} \cdot CX_{0,1}
\end{aligned}$$

$$\begin{aligned}
& \xrightarrow{C_{77}} r_4 \cdot CX_{0,1} \cdot CX_{0,2} \cdot Z_1 \cdot \overline{CCX_{1,2} \cdot CZ_{1,2} \cdot CZ_{0,1}} \cdot CX_{0,2} \cdot CX_{0,1} \\
& \xrightarrow{(40)} r_4 \cdot CX_{0,1} \cdot CX_{0,2} \cdot Z_1 \cdot \overline{CCX_{1,2} \cdot CZ_{1,2} \cdot CZ_{0,1}} \cdot CX_{0,2} \cdot CX_{0,1} \\
& \xrightarrow{E_{12}} r_4 \cdot CX_{0,1} \cdot CX_{0,2} \cdot \underline{Z_1 \cdot CCX_{1,2}} \cdot CZ_{0,1} \cdot CX_{0,2} \cdot CX_{0,1} \\
& \xrightarrow{C_{59}} r_4 \cdot CX_{0,1} \cdot CX_{0,2} \cdot \overline{CCX_{1,2} \cdot Z_1} \cdot \underline{CZ_{0,1} \cdot CX_{0,2}} \cdot CX_{0,1} \\
& \xleftarrow{C_{24}} r_4 \cdot CX_{0,1} \cdot CX_{0,2} \cdot \overline{CCX_{1,2} \cdot Z_1} \cdot \underline{CX_{0,2} \cdot CZ_{0,1}} \cdot CX_{0,1} \\
& \xrightarrow{B_{10}} r_4 \cdot CX_{0,1} \cdot CX_{0,2} \cdot \overline{CCX_{1,2} \cdot CX_{0,2} \cdot Z_1} \cdot \underline{CZ_{0,1} \cdot CX_{0,1}} \\
& \xleftarrow{C_{76}} r_4 \cdot CX_{0,1} \cdot CX_{0,2} \cdot \overline{CCX_{1,2} \cdot CX_{0,2} \cdot Z_1} \cdot \underline{CX_{0,1} \cdot Z_0 \cdot CZ_{0,1}} \\
& \xrightarrow{C_{68}} r_4 \cdot CX_{0,1} \cdot CX_{0,2} \cdot \overline{CCX_{1,2} \cdot CX_{0,2} \cdot CX_{0,1} \cdot Z_0 \cdot CZ_{0,1}} \\
& \xrightarrow{B_{29}} r_4 \cdot CX_{0,1} \cdot CX_{0,2} \cdot \overline{CCX_{1,2} \cdot CX_{0,2} \cdot CX_{0,1} \cdot Z_1 \cdot Z_0 \cdot CZ_{0,1}} \\
& \xrightarrow{E_3} r_4 \cdot \underline{CX_{0,1} \cdot CX_{0,2} \cdot CCX_{1,2} \cdot CX_{0,2} \cdot CX_{0,1} \cdot Z_1 \cdot CZ_{0,1}} \\
& \xleftarrow{D_4} \underline{r_4 \cdot \overline{r_4}} \cdot Z_1 \cdot CZ_{0,1} \xrightarrow{(4;4)} Z_1 \cdot CZ_{0,1} \\
\\
& (\omega_{13}) : \underline{w_5} \xrightarrow{W_5} \overline{r_3 \cdot r_2 \cdot w_4 \cdot r_2 \cdot r_3} \xrightarrow{\omega_4} r_3 \cdot r_2 \cdot \underline{w_4} \cdot \overline{X_0 \cdot CCX_{0,1} \cdot CCX_{0,2} \cdot X_0} \\
& \xrightarrow{\omega_{12}} r_3 \cdot r_2 \cdot \underline{Z_1 \cdot CZ_{0,1} \cdot X_0} \cdot \overline{CCX_{0,1} \cdot CCX_{0,2} \cdot X_0} \\
& \xleftarrow{C_{69}} r_3 \cdot r_2 \cdot \underline{Z_1 \cdot X_0 \cdot Z_1 \cdot CZ_{0,1}} \cdot \overline{CCX_{0,1} \cdot CCX_{0,2} \cdot X_0} \\
& \xleftarrow{B_{14}} r_3 \cdot r_2 \cdot \overline{X_0 \cdot Z_1 \cdot Z_1 \cdot CZ_{0,1}} \cdot \overline{CCX_{0,1} \cdot CCX_{0,2} \cdot X_0} \\
& \xrightarrow{E_5} r_3 \cdot r_2 \cdot X_0 \cdot \underline{CZ_{0,1} \cdot CCX_{0,1} \cdot CCX_{0,2} \cdot X_0} \\
& \xrightarrow{C_{95}} r_3 \cdot r_2 \cdot X_0 \cdot \overline{CCX_{0,1} \cdot CZ_{0,1} \cdot CCX_{0,2} \cdot X_0} \\
& \xrightarrow{C_{80}} r_3 \cdot r_2 \cdot X_0 \cdot \overline{CCX_{0,1} \cdot CCX_{0,2} \cdot CZ_{0,1} \cdot CZ_{0,2} \cdot X_0} \\
& \xleftarrow{C_{117}} r_3 \cdot r_2 \cdot X_0 \cdot \overline{CCX_{0,1} \cdot CCX_{0,2} \cdot CZ_{0,1} \cdot X_0 \cdot Z_2 \cdot CZ_{0,2}} \\
& \xleftarrow{C_{69}} r_3 \cdot r_2 \cdot X_0 \cdot \overline{CCX_{0,1} \cdot CCX_{0,2} \cdot X_0 \cdot Z_1 \cdot CZ_{0,1} \cdot Z_2 \cdot CZ_{0,2}} \\
& \xrightarrow{B_{27}} r_3 \cdot r_2 \cdot \underline{X_0 \cdot CCX_{0,1} \cdot CCX_{0,2} \cdot X_0 \cdot Z_1 \cdot Z_2 \cdot CZ_{0,1} \cdot CZ_{0,2}} \\
& \xleftarrow{\omega_4} r_3 \cdot \underline{r_2 \cdot \overline{r_2} \cdot r_3} \cdot Z_1 \cdot Z_2 \cdot CZ_{0,1} \cdot CZ_{0,2} \xrightarrow{(2;2)} \underline{r_3 \cdot r_3} \cdot Z_1 \cdot Z_2 \cdot CZ_{0,1} \cdot CZ_{0,2} \xrightarrow{(3;3)} Z_1 \cdot Z_2 \cdot CZ_{0,1} \cdot CZ_{0,2} \\
\\
& (\omega_{14}) : \underline{r_1} \cdot r_2 \xrightarrow{D_1} \overline{X_0 \cdot X_1 \cdot CCX_{0,1} \cdot X_1 \cdot X_0 \cdot r_2} \xrightarrow{C_{35}} X_0 \cdot \overline{CCX_{0,1} \cdot CX_{0,2} \cdot X_1 \cdot X_1 \cdot X_0 \cdot r_2} \xrightarrow{E_{13}} X_0 \cdot \overline{CCX_{0,1} \cdot CX_{0,2} \cdot X_0 \cdot r_2} \\
& \xrightarrow{D_2} X_0 \cdot \overline{CCX_{0,1} \cdot CX_{0,2} \cdot X_0 \cdot X_0 \cdot CX_{2,1} \cdot CCX_{0,1} \cdot CX_{2,1} \cdot X_0} \\
& \xrightarrow{(21)} X_0 \cdot \overline{CCX_{0,1} \cdot CX_{0,2} \cdot CX_{2,1} \cdot CCX_{0,1} \cdot CX_{2,1} \cdot X_0} \\
& \xrightarrow{C_{105}} X_0 \cdot \overline{CX_{0,2} \cdot CCX_{0,1} \cdot CX_{2,1} \cdot CCX_{0,1} \cdot CX_{2,1} \cdot X_0} \\
& \xrightarrow{X_6} X_0 \cdot CX_{0,2} \cdot \overline{CCX_{0,1} \cdot CCX_{0,2} \cdot CCX_{0,1} \cdot CCX_{0,2} \cdot X_0} \\
& \xrightarrow{X_9} X_0 \cdot CX_{0,2} \cdot \overline{CCX_{0,1} \cdot CCX_{0,2} \cdot CCX_{0,1} \cdot X_0} \xrightarrow{E_{18}} X_0 \cdot CX_{0,2} \cdot \overline{CCX_{0,1} \cdot CCX_{0,2} \cdot CCX_{0,1} \cdot X_0}
\end{aligned}$$

$$\begin{aligned}
(\omega_{15}) : w_6 &\xrightarrow{W_6} \overline{r_2 \cdot r_1 \cdot w_5 \cdot r_1 \cdot r_2} \\
&\xrightarrow{\omega_{14}} r_2 \cdot r_1 \cdot \underline{w_5} \cdot \overline{X_0 \cdot CX_{0,2} \cdot CCX_{0,2} \cdot CCX_{0,1} \cdot X_0} \\
&\xrightarrow{\omega_{13}} r_2 \cdot r_1 \cdot \overline{Z_1 \cdot Z_2 \cdot CZ_{0,1} \cdot CZ_{0,2} \cdot X_0} \cdot CX_{0,2} \cdot CCX_{0,2} \cdot CCX_{0,1} \cdot X_0 \\
&\xleftarrow{C_{117}} r_2 \cdot r_1 \cdot Z_1 \cdot \overline{Z_2 \cdot CZ_{0,1} \cdot X_0 \cdot Z_2 \cdot CZ_{0,2}} \cdot CX_{0,2} \cdot CCX_{0,2} \cdot CCX_{0,1} \cdot X_0 \\
&\xleftarrow{B_{27}} r_2 \cdot r_1 \cdot Z_1 \cdot \overline{CZ_{0,1} \cdot Z_2 \cdot X_0 \cdot Z_2 \cdot CZ_{0,2}} \cdot CX_{0,2} \cdot CCX_{0,2} \cdot CCX_{0,1} \cdot X_0 \\
&\xleftarrow{B_{26}} r_2 \cdot r_1 \cdot Z_1 \cdot CZ_{0,1} \cdot \overline{X_0 \cdot Z_2 \cdot Z_2 \cdot CZ_{0,2}} \cdot CX_{0,2} \cdot CCX_{0,2} \cdot CCX_{0,1} \cdot X_0 \\
&\xrightarrow{E_{19}} r_2 \cdot r_1 \cdot Z_1 \cdot \overline{CZ_{0,1} \cdot X_0 \cdot CZ_{0,2}} \cdot CX_{0,2} \cdot CCX_{0,2} \cdot CCX_{0,1} \cdot X_0 \\
&\xleftarrow{C_{69}} r_2 \cdot r_1 \cdot Z_1 \cdot \overline{X_0 \cdot Z_1 \cdot CZ_{0,1}} \cdot CZ_{0,2} \cdot CX_{0,2} \cdot CCX_{0,2} \cdot CCX_{0,1} \cdot X_0 \\
&\xrightarrow{B_{14}} r_2 \cdot r_1 \cdot \underline{Z_1 \cdot X_0} \cdot CZ_{0,1} \cdot CZ_{0,2} \cdot CX_{0,2} \cdot CCX_{0,2} \cdot CCX_{0,1} \cdot X_0 \\
&\xrightarrow{E_5} r_2 \cdot r_1 \cdot X_0 \cdot CZ_{0,1} \cdot CZ_{0,2} \cdot CX_{0,2} \cdot CCX_{0,2} \cdot CCX_{0,1} \cdot X_0 \\
&\xleftarrow{E_{11}} r_2 \cdot r_1 \cdot X_0 \cdot CZ_{0,1} \cdot CZ_{0,2} \cdot \overline{CX_{0,2} \cdot CZ_{0,2} \cdot CZ_{0,2}} \cdot CCX_{0,2} \cdot CCX_{0,1} \cdot X_0 \\
&\xleftarrow{C_{63}} r_2 \cdot r_1 \cdot X_0 \cdot CZ_{0,1} \cdot \overline{CZ_{0,2} \cdot CZ_{0,2} \cdot Z_0 \cdot CX_{0,2}} \cdot CZ_{0,2} \cdot CCX_{0,2} \cdot CCX_{0,1} \cdot X_0 \\
&\xrightarrow{E_{11}} r_2 \cdot r_1 \cdot X_0 \cdot CZ_{0,1} \cdot \underline{Z_0 \cdot CX_{0,2}} \cdot CZ_{0,2} \cdot CCX_{0,2} \cdot CCX_{0,1} \cdot X_0 \\
&\xleftarrow{C_{90}} r_2 \cdot r_1 \cdot X_0 \cdot \overline{CZ_{0,1} \cdot CX_{0,2} \cdot Z_0} \cdot CZ_{0,2} \cdot CCX_{0,2} \cdot CCX_{0,1} \cdot X_0 \\
&\xleftarrow{C_{24}} r_2 \cdot r_1 \cdot X_0 \cdot \overline{CX_{0,2} \cdot CZ_{0,1} \cdot Z_0 \cdot CZ_{0,2}} \cdot CCX_{0,2} \cdot CCX_{0,1} \cdot X_0 \\
&\xrightarrow{C_{96}} r_2 \cdot r_1 \cdot X_0 \cdot CX_{0,2} \cdot CZ_{0,1} \cdot \underline{Z_0 \cdot CCX_{0,2} \cdot CZ_{0,2}} \cdot CCX_{0,1} \cdot X_0 \\
&\xrightarrow{C_{58}} r_2 \cdot r_1 \cdot X_0 \cdot CX_{0,2} \cdot \overline{CZ_{0,1} \cdot CCX_{0,2} \cdot Z_0} \cdot CZ_{0,2} \cdot CCX_{0,1} \cdot X_0 \\
&\xrightarrow{C_{80}} r_2 \cdot r_1 \cdot X_0 \cdot CX_{0,2} \cdot \overline{CCX_{0,2} \cdot CZ_{0,1} \cdot CZ_{0,2} \cdot Z_0} \cdot CZ_{0,2} \cdot CCX_{0,1} \cdot X_0 \\
&\xrightarrow{C_{103}} r_2 \cdot r_1 \cdot X_0 \cdot CX_{0,2} \cdot CCX_{0,2} \cdot CZ_{0,1} \cdot \overline{Z_0 \cdot CZ_{0,2} \cdot CZ_{0,2}} \cdot CCX_{0,1} \cdot X_0 \\
&\xrightarrow{E_{11}} r_2 \cdot r_1 \cdot X_0 \cdot CX_{0,2} \cdot CCX_{0,2} \cdot CZ_{0,1} \cdot \underline{Z_0 \cdot CCX_{0,1}} \cdot X_0 \\
&\xrightarrow{C_{54}} r_2 \cdot r_1 \cdot X_0 \cdot CX_{0,2} \cdot CCX_{0,2} \cdot \overline{CZ_{0,1} \cdot CCX_{0,1} \cdot Z_0} \cdot X_0 \\
&\xrightarrow{C_{95}} r_2 \cdot r_1 \cdot X_0 \cdot CX_{0,2} \cdot CCX_{0,2} \cdot \overline{CCX_{0,1} \cdot CZ_{0,1}} \cdot Z_0 \cdot X_0 \\
&\xleftarrow{(21)} r_2 \cdot r_1 \cdot \underline{X_0 \cdot CX_{0,2} \cdot CCX_{0,2} \cdot CCX_{0,1} \cdot X_0} \cdot \overline{X_0 \cdot X_0} \cdot CZ_{0,1} \cdot Z_0 \cdot X_0 \\
&\xleftarrow{\omega_{14}} r_2 \cdot r_1 \cdot \overline{r_1 \cdot r_2} \cdot X_0 \cdot CZ_{0,1} \cdot Z_0 \cdot X_0 \\
&\xrightarrow{(1;1)} r_2 \cdot r_2 \cdot X_0 \cdot CZ_{0,1} \cdot Z_0 \cdot X_0 \\
&\xrightarrow{(2;2)} X_0 \cdot CZ_{0,1} \cdot Z_0 \cdot X_0
\end{aligned}$$

$$\begin{aligned}
(\omega_{16}) : w_6 \cdot w_4 \cdot \underline{w_2} &\xrightarrow{\omega_5} w_6 \cdot \underline{w_4} \cdot \overline{X_1 \cdot CZ_{0,1} \cdot X_1} \\
&\xrightarrow{\omega_{12}} w_6 \cdot \overline{Z_1 \cdot CZ_{0,1} \cdot X_1} \cdot CZ_{0,1} \cdot X_1 \\
&\xleftarrow{C_{112}} w_6 \cdot Z_1 \cdot \overline{X_1 \cdot Z_0 \cdot CZ_{0,1} \cdot CZ_{0,1} \cdot X_1} \\
&\xrightarrow{E_2} w_6 \cdot Z_1 \cdot \underline{X_1 \cdot Z_0} \cdot X_1 \\
&\xrightarrow{B_{15}} w_6 \cdot Z_1 \cdot \overline{Z_0 \cdot X_1} \cdot X_1 \\
&\xrightarrow{E_{13}} \underline{w_6} \cdot Z_1 \cdot Z_0 \\
&\xrightarrow{\omega_{15}} \overline{X_0 \cdot CZ_{0,1} \cdot Z_0 \cdot X_0} \cdot Z_1 \cdot Z_0 \\
&\xrightarrow{C_{53}} \overline{CZ_{0,1} \cdot Z_1 \cdot X_0 \cdot Z_0 \cdot X_0 \cdot Z_1 \cdot Z_0} \\
&\xleftarrow{B_{29}} \overline{CZ_{0,1} \cdot Z_1 \cdot X_0 \cdot Z_0 \cdot X_0 \cdot Z_0 \cdot Z_1} \\
&\xleftarrow{P_1} \overline{CZ_{0,1} \cdot Z_1 \cdot (-I) \cdot Z_1} \\
&\xrightarrow{\gamma_6} \overline{CZ_{0,1} \cdot Z_1 \cdot \overline{Z_1} \cdot (-I)} \\
&\xrightarrow{E_5} \overline{CZ_{0,1} \cdot (-I)}
\end{aligned}$$

$$\begin{aligned}
(\omega_{17}) : CZ_{0,2} \cdot X_2 \cdot X_1 \cdot \underline{K_{1,2} \cdot CZ_{0,2}} \cdot K_{1,2} \cdot X_1 \cdot X_2 \cdot CZ_{0,2} \\
&\xrightarrow{C_{28}} CZ_{0,2} \cdot X_2 \cdot X_1 \cdot \overline{CX_{0,2} \cdot K_{1,2}} \cdot K_{1,2} \cdot X_1 \cdot X_2 \cdot CZ_{0,2} \\
&\xrightarrow{(23)} CZ_{0,2} \cdot X_2 \cdot X_1 \cdot \underline{CX_{0,2} \cdot X_1} \cdot X_2 \cdot CZ_{0,2} \\
&\xrightarrow{B_3} CZ_{0,2} \cdot X_2 \cdot \underline{X_1 \cdot \overline{X_1}} \cdot \overline{CX_{0,2}} \cdot X_2 \cdot CZ_{0,2} \\
&\xrightarrow{E_{13}} CZ_{0,2} \cdot X_2 \cdot \underline{CX_{0,2} \cdot X_2} \cdot CZ_{0,2} \\
&\xrightarrow{C_{65}} CZ_{0,2} \cdot \underline{X_2 \cdot \overline{X_2}} \cdot \overline{CX_{0,2}} \cdot CZ_{0,2} \\
&\xrightarrow{E_{17}} CZ_{0,2} \cdot \underline{CX_{0,2} \cdot CZ_{0,2}} \\
&\xleftarrow{C_{63}} \overline{CZ_{0,2} \cdot \overline{CZ_{0,2}} \cdot Z_0 \cdot CX_{0,2}} \\
&\xrightarrow{E_{11}} Z_0 \cdot CX_{0,2}
\end{aligned}$$

$$\begin{aligned}
(\omega_{18}) : (-I) \cdot \underline{r_8} &\xrightarrow{D_8} (-I) \cdot \overline{K_{1,2} \cdot X_1 \cdot X_2 \cdot CZ_{0,2} \cdot CCX_{1,2} \cdot CZ_{0,2} \cdot X_2 \cdot X_1 \cdot K_{1,2}} \\
&\xrightarrow{\gamma_1} \overline{K_{1,2} \cdot (-I) \cdot X_1 \cdot X_2 \cdot CZ_{0,2} \cdot CCX_{1,2} \cdot CZ_{0,2} \cdot X_2 \cdot X_1 \cdot K_{1,2}} \\
&\xrightarrow{\gamma_2} K_{1,2} \cdot \overline{X_1 \cdot (-I) \cdot X_2} \cdot CZ_{0,2} \cdot CCX_{1,2} \cdot CZ_{0,2} \cdot X_2 \cdot X_1 \cdot K_{1,2} \\
&\xrightarrow{\gamma_3} K_{1,2} \cdot X_1 \cdot \overline{X_2 \cdot (-I) \cdot CZ_{0,2}} \cdot CCX_{1,2} \cdot CZ_{0,2} \cdot X_2 \cdot X_1 \cdot K_{1,2} \\
&\xrightarrow{\gamma_{16}} K_{1,2} \cdot X_1 \cdot X_2 \cdot \overline{CZ_{0,2} \cdot (-I) \cdot CCX_{1,2}} \cdot CZ_{0,2} \cdot X_2 \cdot X_1 \cdot K_{1,2} \\
&\xrightarrow{\gamma_{17}} K_{1,2} \cdot X_1 \cdot X_2 \cdot CZ_{0,2} \cdot \overline{CCX_{1,2} \cdot (-I) \cdot CZ_{0,2}} \cdot X_2 \cdot X_1 \cdot K_{1,2} \\
&\xrightarrow{\gamma_{16}} K_{1,2} \cdot X_1 \cdot X_2 \cdot CZ_{0,2} \cdot CCX_{1,2} \cdot \overline{CZ_{0,2} \cdot (-I) \cdot X_2} \cdot X_1 \cdot K_{1,2} \\
&\xrightarrow{\gamma_3} K_{1,2} \cdot X_1 \cdot X_2 \cdot CZ_{0,2} \cdot CCX_{1,2} \cdot CZ_{0,2} \cdot \overline{X_2 \cdot (-I) \cdot X_1} \cdot K_{1,2} \\
&\xrightarrow{\gamma_2} K_{1,2} \cdot X_1 \cdot X_2 \cdot CZ_{0,2} \cdot CCX_{1,2} \cdot CZ_{0,2} \cdot X_2 \cdot \overline{X_1 \cdot (-I) \cdot K_{1,2}} \\
&\xrightarrow{\gamma_1} \overline{K_{1,2} \cdot X_1 \cdot X_2 \cdot CZ_{0,2} \cdot CCX_{1,2} \cdot CZ_{0,2} \cdot X_2 \cdot X_1 \cdot \overline{K_{1,2} \cdot (-I)}} \\
&\xleftarrow{D_8} \overline{r_8 \cdot (-I)}
\end{aligned}$$

$$\begin{aligned}
(\omega_{19}) : r_8 \cdot CZ_{0,2} \cdot \underline{r_8} \cdot CZ_{0,2} \cdot r_8 \\
&\xrightarrow{D_8} \overline{r_8 \cdot CZ_{0,2} \cdot K_{1,2} \cdot X_1 \cdot X_2 \cdot CZ_{0,2} \cdot CCX_{1,2} \cdot CZ_{0,2} \cdot X_2 \cdot X_1 \cdot K_{1,2} \cdot CZ_{0,2} \cdot r_8} \\
&\xrightarrow{D_8} \overline{K_{1,2} \cdot X_1 \cdot X_2 \cdot CZ_{0,2} \cdot CCX_{1,2} \cdot CZ_{0,2} \cdot X_2 \cdot X_1 \cdot K_{1,2} \cdot CZ_{0,2} \cdot K_{1,2} \cdot X_1 \cdot X_2 \cdot CZ_{0,2} \cdot CCX_{1,2} \cdot CZ_{0,2} \cdot X_2 \cdot X_1 \cdot K_{1,2} \cdot CZ_{0,2} \cdot r_8} \\
&\xrightarrow{\omega_{17}} K_{1,2} \cdot X_1 \cdot X_2 \cdot CZ_{0,2} \cdot CCX_{1,2} \cdot \overline{Z_0 \cdot CX_{0,2}} \cdot CCX_{1,2} \cdot CZ_{0,2} \cdot X_2 \cdot X_1 \cdot K_{1,2} \cdot CZ_{0,2} \cdot \underline{r_8} \\
&\xrightarrow{D_8} \overline{K_{1,2} \cdot X_1 \cdot X_2 \cdot CZ_{0,2} \cdot CCX_{1,2} \cdot Z_0 \cdot CX_{0,2} \cdot CCX_{1,2} \cdot CZ_{0,2} \cdot X_2 \cdot X_1 \cdot K_{1,2} \cdot CZ_{0,2} \cdot \overline{K_{1,2} \cdot X_1 \cdot X_2 \cdot CZ_{0,2} \cdot CCX_{1,2} \cdot CZ_{0,2} \cdot X_2 \cdot X_1 \cdot K_{1,2}}}
\end{aligned}$$

$$\begin{aligned}
& \xrightarrow{\omega_{17}} K_{1,2} \cdot X_1 \cdot X_2 \cdot CZ_{0,2} \cdot CCX_{1,2} \cdot Z_0 \cdot CX_{0,2} \cdot CCX_{1,2} \cdot \overline{Z_0 \cdot CX_{0,2}} \cdot CCX_{1,2} \cdot CZ_{0,2} \cdot X_2 \cdot X_1 \cdot K_{1,2} \\
& \xleftarrow{C_{90}} K_{1,2} \cdot X_1 \cdot X_2 \cdot CZ_{0,2} \cdot CCX_{1,2} \cdot Z_0 \cdot CX_{0,2} \cdot CCX_{1,2} \cdot \overline{CX_{0,2} \cdot Z_0} \cdot CCX_{1,2} \cdot CZ_{0,2} \cdot X_2 \cdot X_1 \cdot K_{1,2} \\
& \xrightarrow{C_{49}} K_{1,2} \cdot X_1 \cdot X_2 \cdot CZ_{0,2} \cdot \overline{CCX_{1,2} \cdot Z_0} \cdot CX_{0,2} \cdot CCX_{1,2} \cdot CX_{0,2} \cdot \overline{CCX_{1,2} \cdot CZ_{1,2} \cdot Z_0} \cdot CZ_{0,2} \cdot X_2 \cdot X_1 \cdot K_{1,2} \\
& \xrightarrow{C_{57}} K_{1,2} \cdot X_1 \cdot X_2 \cdot CZ_{0,2} \cdot \overline{Z_0 \cdot CZ_{1,2} \cdot CCX_{1,2}} \cdot \overline{CX_{0,2} \cdot CCX_{1,2} \cdot CX_{0,2}} \cdot CCX_{1,2} \cdot CZ_{1,2} \cdot Z_0 \cdot CZ_{0,2} \cdot X_2 \cdot X_1 \cdot K_{1,2} \\
& \xrightarrow{X_4} K_{1,2} \cdot X_1 \cdot X_2 \cdot CZ_{0,2} \cdot Z_0 \cdot CZ_{1,2} \cdot CCX_{1,2} \cdot \overline{CCX_{0,1} \cdot CCX_{1,2} \cdot CCX_{0,1}} \cdot CCX_{1,2} \cdot CZ_{1,2} \cdot Z_0 \cdot CZ_{0,2} \cdot X_2 \cdot X_1 \cdot K_{1,2} \\
& \xrightarrow{X_{11}} K_{1,2} \cdot X_1 \cdot X_2 \cdot CZ_{0,2} \cdot Z_0 \cdot CZ_{1,2} \cdot CCX_{1,2} \cdot \overline{CCX_{1,2} \cdot CCX_{0,1} \cdot CCX_{1,2}} \cdot CCX_{1,2} \cdot CZ_{1,2} \cdot Z_0 \cdot CZ_{0,2} \cdot X_2 \cdot X_1 \cdot K_{1,2} \\
& \xrightarrow{(24)} K_{1,2} \cdot X_1 \cdot X_2 \cdot CZ_{0,2} \cdot Z_0 \cdot CZ_{1,2} \cdot \overline{CCX_{1,2} \cdot CCX_{1,2}} \cdot CCX_{0,1} \cdot CZ_{1,2} \cdot Z_0 \cdot CZ_{0,2} \cdot X_2 \cdot X_1 \cdot K_{1,2} \\
& \xrightarrow{(24)} K_{1,2} \cdot X_1 \cdot X_2 \cdot CZ_{0,2} \cdot Z_0 \cdot \overline{CZ_{1,2} \cdot CCX_{0,1}} \cdot CZ_{1,2} \cdot Z_0 \cdot CZ_{0,2} \cdot X_2 \cdot X_1 \cdot K_{1,2} \\
& \xrightarrow{C_{82}} K_{1,2} \cdot X_1 \cdot X_2 \cdot CZ_{0,2} \cdot Z_0 \cdot \overline{CCX_{0,1} \cdot CZ_{0,1} \cdot CZ_{1,2}} \cdot CZ_{1,2} \cdot Z_0 \cdot CZ_{0,2} \cdot X_2 \cdot X_1 \cdot K_{1,2} \\
& \xrightarrow{E_{12}} K_{1,2} \cdot X_1 \cdot X_2 \cdot \overline{CZ_{0,2} \cdot Z_0} \cdot CCX_{0,1} \cdot CZ_{0,1} \cdot Z_0 \cdot CZ_{0,2} \cdot X_2 \cdot X_1 \cdot K_{1,2} \\
& \xrightarrow{C_{103}} K_{1,2} \cdot X_1 \cdot X_2 \cdot \overline{Z_0 \cdot CZ_{0,2}} \cdot CCX_{0,1} \cdot CZ_{0,1} \cdot Z_0 \cdot CZ_{0,2} \cdot X_2 \cdot X_1 \cdot K_{1,2} \\
& \xrightarrow{C_{81}} K_{1,2} \cdot X_1 \cdot X_2 \cdot Z_0 \cdot \overline{CCX_{0,1} \cdot CZ_{0,1} \cdot CZ_{0,2}} \cdot CZ_{0,1} \cdot Z_0 \cdot CZ_{0,2} \cdot X_2 \cdot X_1 \cdot K_{1,2} \\
& \xrightarrow{C_{60}} K_{1,2} \cdot X_1 \cdot X_2 \cdot Z_0 \cdot CCX_{0,1} \cdot \overline{CZ_{0,2} \cdot CZ_{0,1} \cdot CZ_{0,1}} \cdot Z_0 \cdot CZ_{0,2} \cdot X_2 \cdot X_1 \cdot K_{1,2} \\
& \xrightarrow{E_2} K_{1,2} \cdot X_1 \cdot X_2 \cdot Z_0 \cdot CCX_{0,1} \cdot \overline{CZ_{0,2} \cdot Z_0} \cdot CZ_{0,2} \cdot X_2 \cdot X_1 \cdot K_{1,2} \\
& \xrightarrow{C_{103}} K_{1,2} \cdot X_1 \cdot X_2 \cdot Z_0 \cdot CCX_{0,1} \cdot \overline{Z_0 \cdot CZ_{0,2} \cdot CZ_{0,2}} \cdot X_2 \cdot X_1 \cdot K_{1,2} \\
& \xrightarrow{E_{11}} K_{1,2} \cdot X_1 \cdot X_2 \cdot \overline{Z_0 \cdot CCX_{0,1}} \cdot Z_0 \cdot X_2 \cdot X_1 \cdot K_{1,2} \\
& \xrightarrow{C_{54}} K_{1,2} \cdot X_1 \cdot X_2 \cdot \overline{CCX_{0,1} \cdot Z_0} \cdot Z_0 \cdot X_2 \cdot X_1 \cdot K_{1,2} \\
& \xrightarrow{E_3} K_{1,2} \cdot X_1 \cdot X_2 \cdot \overline{CCX_{0,1} \cdot X_2} \cdot X_1 \cdot K_{1,2} \\
& \xrightarrow{C_{39}} K_{1,2} \cdot X_1 \cdot \overline{CCX_{0,1} \cdot X_2} \cdot X_2 \cdot X_1 \cdot K_{1,2} \\
& \xrightarrow{E_{17}} K_{1,2} \cdot X_1 \cdot CCX_{0,1} \cdot X_1 \cdot K_{1,2} \\
& \xrightarrow{C_{27}} \overline{Z_1 \cdot K_{1,2}} \cdot CCX_{0,1} \cdot X_1 \cdot K_{1,2} \xrightarrow{C_{44}} Z_1 \cdot \overline{CCX_{0,2} \cdot K_{1,2} \cdot X_1} \cdot K_{1,2} \xrightarrow{C_{27}} Z_1 \cdot CCX_{0,2} \cdot \overline{Z_1 \cdot K_{1,2} \cdot K_{1,2}} \xrightarrow{(23)} Z_1 \cdot CCX_{0,2} \cdot Z_1
\end{aligned}$$

$$\begin{aligned}
(\omega_{20}) : \underline{w_7} & \xrightarrow{W_7} \overline{r_7 \cdot r_8 \cdot r_6 \cdot w_6 \cdot w_4 \cdot w_2 \cdot r_8 \cdot w_6 \cdot w_4 \cdot w_2 \cdot r_6 \cdot r_8 \cdot r_7} \xrightarrow{\omega_{16}} r_7 \cdot r_8 \cdot r_6 \cdot \overline{w_6 \cdot w_4 \cdot w_2 \cdot r_8} \cdot \overline{CZ_{0,1} \cdot (-I)} \cdot r_6 \cdot r_8 \cdot r_7 \\
& \xrightarrow{\omega_{16}} r_7 \cdot r_8 \cdot r_6 \cdot \overline{CZ_{0,1} \cdot (-I)} \cdot r_8 \cdot \overline{CZ_{0,1} \cdot (-I)} \cdot r_6 \cdot r_8 \cdot r_7 \\
& \xleftarrow{\gamma_{15}} r_7 \cdot r_8 \cdot r_6 \cdot CZ_{0,1} \cdot \overline{(-I)} \cdot r_8 \cdot \overline{(-I)} \cdot CZ_{0,1} \cdot r_6 \cdot r_8 \cdot r_7 \\
& \xrightarrow{\omega_{18}} r_7 \cdot r_8 \cdot r_6 \cdot CZ_{0,1} \cdot \overline{r_8 \cdot (-I)} \cdot \overline{(-I)} \cdot CZ_{0,1} \cdot r_6 \cdot r_8 \cdot r_7 \\
& \xrightarrow{\eta_{12}} r_7 \cdot r_8 \cdot r_6 \cdot CZ_{0,1} \cdot r_8 \cdot \overline{CZ_{0,1} \cdot r_6 \cdot r_8 \cdot r_7} \\
& \xrightarrow{\omega_6} r_7 \cdot r_8 \cdot \overline{r_6 \cdot CZ_{0,1}} \cdot r_8 \cdot \overline{r_6 \cdot CZ_{0,2}} \cdot r_8 \cdot r_7 \\
& \xleftarrow{\omega_7} r_7 \cdot r_8 \cdot \overline{CZ_{0,2} \cdot r_6 \cdot r_8 \cdot r_6 \cdot CZ_{0,2}} \cdot r_8 \cdot r_7 \\
& \xleftarrow{(8;8)} r_7 \cdot r_8 \cdot CZ_{0,2} \cdot \overline{r_6 \cdot r_8 \cdot r_6 \cdot r_8 \cdot r_8} \cdot CZ_{0,2} \cdot r_8 \cdot r_7 \\
& \xrightarrow{(6;8)} r_7 \cdot r_8 \cdot \overline{CZ_{0,2} \cdot r_8 \cdot CZ_{0,2} \cdot r_8 \cdot r_7} \\
& \xrightarrow{\omega_{19}} \underline{r_7} \cdot \overline{Z_1 \cdot CCX_{0,2} \cdot Z_1} \cdot r_7
\end{aligned}$$

$$\begin{aligned}
& \xrightarrow{D_7} \overline{CZ_{0,1} \cdot CX_{2,1} \cdot CCX_{0,1} \cdot CX_{2,1} \cdot CZ_{0,1}} \cdot \underline{Z_1 \cdot CCX_{0,2} \cdot Z_1 \cdot r_7} \\
& \xrightarrow{C_{40}} CZ_{0,1} \cdot CX_{2,1} \cdot CCX_{0,1} \cdot CX_{2,1} \cdot CZ_{0,1} \cdot \overline{CCX_{0,2} \cdot CZ_{0,2} \cdot \underline{Z_1 \cdot Z_1} \cdot r_7} \\
& \xrightarrow{E_5} CZ_{0,1} \cdot CX_{2,1} \cdot CCX_{0,1} \cdot CX_{2,1} \cdot CZ_{0,1} \cdot \underline{CCX_{0,2} \cdot CZ_{0,2} \cdot r_7} \\
& \xrightarrow{C_{80}} CZ_{0,1} \cdot CX_{2,1} \cdot CCX_{0,1} \cdot CX_{2,1} \cdot \overline{CCX_{0,2} \cdot CZ_{0,1} \cdot \underline{CZ_{0,2} \cdot CZ_{0,2}} \cdot r_7} \\
& \xrightarrow{E_{11}} CZ_{0,1} \cdot CX_{2,1} \cdot CCX_{0,1} \cdot CX_{2,1} \cdot \underline{CCX_{0,2} \cdot CZ_{0,1} \cdot r_7} \\
& \xrightarrow{\chi_6} CZ_{0,1} \cdot \overline{CCX_{0,2} \cdot CCX_{0,1} \cdot \underline{CCX_{0,2} \cdot CCX_{0,2}} \cdot CZ_{0,1} \cdot r_7} \\
& \xrightarrow{E_7} CZ_{0,1} \cdot \underline{CCX_{0,2} \cdot CCX_{0,1} \cdot CZ_{0,1} \cdot \underline{r_7}} \\
& \xrightarrow{D_7} CZ_{0,1} \cdot \underline{CCX_{0,2} \cdot CCX_{0,1} \cdot \underline{CZ_{0,1} \cdot CX_{2,1} \cdot CCX_{0,1} \cdot CX_{2,1} \cdot CZ_{0,1}}} \\
& \xrightarrow{E_2} CZ_{0,1} \cdot \underline{CCX_{0,2} \cdot CCX_{0,1} \cdot \underline{CX_{2,1} \cdot CCX_{0,1} \cdot CX_{2,1} \cdot CZ_{0,1}}} \\
& \xrightarrow{\chi_6} CZ_{0,1} \cdot \underline{CCX_{0,2} \cdot CCX_{0,1} \cdot \overline{CCX_{0,2} \cdot CCX_{0,1} \cdot \underline{CCX_{0,2}} \cdot CZ_{0,1}}} \\
& \xrightarrow{\chi_9} CZ_{0,1} \cdot \overline{CCX_{0,1} \cdot \underline{CCX_{0,2} \cdot \underline{CCX_{0,1}} \cdot CCX_{0,1} \cdot CCX_{0,2} \cdot CZ_{0,1}}} \\
& \xrightarrow{E_{18}} CZ_{0,1} \cdot \underline{CCX_{0,1} \cdot \underline{CCX_{0,2} \cdot CCX_{0,2} \cdot CZ_{0,1}}} \\
& \xrightarrow{E_7} \underline{CZ_{0,1} \cdot \underline{CCX_{0,1} \cdot CZ_{0,1}}} \xrightarrow{C_{95}} \overline{\underline{CCX_{0,1} \cdot \underline{CZ_{0,1} \cdot CZ_{0,1}}}} \xrightarrow{E_2} CCX_{0,1}
\end{aligned}$$

$$\begin{aligned}
(\omega_{21}) : \underline{w_{10}} & \xrightarrow{w_{10}} \underline{r_1 \cdot r_3} \\
& \xrightarrow{D_3} \underline{r_1 \cdot \underline{X_0 \cdot CCX_{0,1} \cdot X_0}} \\
& \xrightarrow{D_1} \underline{X_0 \cdot X_1 \cdot \underline{CCX_{0,1} \cdot X_1 \cdot \underline{X_0 \cdot X_0 \cdot CCX_{0,1} \cdot X_0}}} \\
& \xrightarrow{(21)} X_0 \cdot X_1 \cdot \underline{CCX_{0,1} \cdot X_1 \cdot \underline{CCX_{0,1} \cdot X_0}} \\
& \xrightarrow{C_{35}} X_0 \cdot X_1 \cdot \underline{CCX_{0,1} \cdot \overline{CCX_{0,1} \cdot CX_{0,2} \cdot X_1} \cdot X_0} \\
& \xrightarrow{E_{18}} X_0 \cdot X_1 \cdot \underline{CX_{0,2} \cdot X_1 \cdot X_0} \\
& \xrightarrow{B_3} X_0 \cdot \underline{X_1 \cdot \underline{X_1 \cdot \overline{CX_{0,2} \cdot X_0}}} \\
& \xrightarrow{E_{13}} X_0 \cdot \underline{CX_{0,2} \cdot X_0} \\
(\omega_{22}) : \underline{w_8} & \xrightarrow{w_8} \underline{r_1 \cdot r_3 \cdot r_5 \cdot w_7} \\
& \xleftarrow{w_{10}} \underline{w_{10} \cdot r_5 \cdot w_7} \\
& \xrightarrow{\omega_{20}} w_{10} \cdot \underline{r_5 \cdot \overline{CCX_{0,1}}} \\
& \xrightarrow{D_6} w_{10} \cdot \underline{X_1 \cdot \overline{CCX_{0,1} \cdot X_1} \cdot CCX_{0,1}} \\
& \xrightarrow{\omega_{21}} \underline{X_0 \cdot CX_{0,2} \cdot X_0 \cdot X_1 \cdot \underline{CCX_{0,1} \cdot X_1 \cdot \underline{CCX_{0,1}}}} \\
& \xrightarrow{C_{35}} X_0 \cdot CX_{0,2} \cdot X_0 \cdot X_1 \cdot \underline{CCX_{0,1} \cdot \overline{CCX_{0,1} \cdot CX_{0,2} \cdot X_1}} \\
& \xrightarrow{E_{18}} X_0 \cdot CX_{0,2} \cdot X_0 \cdot X_1 \cdot \underline{CX_{0,2} \cdot X_1} \\
& \xrightarrow{B_3} X_0 \cdot CX_{0,2} \cdot X_0 \cdot \underline{X_1 \cdot \underline{X_1 \cdot \overline{CX_{0,2}}}} \\
& \xrightarrow{E_{13}} X_0 \cdot CX_{0,2} \cdot \underline{X_0 \cdot \underline{CX_{0,2}}} \\
& \xrightarrow{C_{118}} X_0 \cdot CX_{0,2} \cdot \overline{CX_{0,2} \cdot X_2 \cdot X_0} \\
& \xleftarrow{B_{13}} X_0 \cdot \underline{CX_{0,2} \cdot CX_{0,2} \cdot \overline{X_0 \cdot X_2}} \xrightarrow{E_{15}} \underline{X_0 \cdot X_0 \cdot X_2} \xrightarrow{(21)} X_2
\end{aligned}$$

$$\begin{aligned}
(\omega_{23}) : \underline{w_{11}} & \xrightarrow{w_{11}} \underline{w_{10} \cdot r_4 \cdot w_8 \cdot \underline{r_4 \cdot w_{10} \cdot w_8}} \xrightarrow{D_4} w_{10} \cdot r_4 \cdot \underline{w_8 \cdot \overline{CX_{0,1} \cdot CX_{0,2} \cdot CCX_{1,2} \cdot CX_{0,2} \cdot CX_{0,1}}} \cdot w_{10} \cdot w_8 \\
& \xrightarrow{\omega_{22}} w_{10} \cdot \underline{r_4 \cdot \overline{X_2} \cdot CX_{0,1} \cdot CX_{0,2} \cdot CCX_{1,2} \cdot CX_{0,2} \cdot CX_{0,1} \cdot w_{10} \cdot w_8} \\
& \xrightarrow{D_4} w_{10} \cdot \overline{CX_{0,1} \cdot CX_{0,2} \cdot \underline{CCX_{1,2} \cdot CX_{0,2} \cdot \overline{CX_{0,1} \cdot X_2 \cdot CX_{0,1} \cdot CX_{0,2} \cdot CCX_{1,2} \cdot CX_{0,2} \cdot CX_{0,1} \cdot w_{10} \cdot w_8}}} \\
& \xleftarrow{B_{16}} w_{10} \cdot CX_{0,1} \cdot CX_{0,2} \cdot \underline{CCX_{1,2} \cdot CX_{0,2} \cdot CX_{0,1} \cdot \overline{CX_{0,1} \cdot X_2 \cdot CX_{0,2} \cdot CCX_{1,2} \cdot CX_{0,2} \cdot CX_{0,1} \cdot w_{10} \cdot w_8}} \\
& \xleftarrow{C_{65}} w_{10} \cdot CX_{0,1} \cdot CX_{0,2} \cdot \underline{CCX_{1,2} \cdot CX_{0,2} \cdot \underline{CX_{0,1} \cdot CX_{0,1} \cdot \overline{CX_{0,2} \cdot X_2 \cdot CCX_{1,2} \cdot CX_{0,2} \cdot CX_{0,1} \cdot w_{10} \cdot w_8}}} \\
& \xrightarrow{(22)} w_{10} \cdot CX_{0,1} \cdot CX_{0,2} \cdot \underline{CCX_{1,2} \cdot CX_{0,2} \cdot \underline{CX_{0,2} \cdot X_2 \cdot CCX_{1,2} \cdot CX_{0,2} \cdot CX_{0,1} \cdot w_{10} \cdot w_8}} \\
& \xrightarrow{E_{15}} w_{10} \cdot CX_{0,1} \cdot CX_{0,2} \cdot \underline{CCX_{1,2} \cdot X_2 \cdot \underline{CCX_{1,2} \cdot CX_{0,2} \cdot CX_{0,1} \cdot w_{10} \cdot w_8}}
\end{aligned}$$

$$\begin{aligned}
& \xrightarrow{C_{83}} w_{10} \cdot CX_{0,1} \cdot CX_{0,2} \cdot \overline{CCX_{1,2} \cdot CX_{1,0} \cdot X_2} \cdot CX_{0,2} \cdot CX_{0,1} \cdot w_{10} \cdot w_8 \\
& \xrightarrow{(24)} \overline{w_{10} \cdot CX_{0,1} \cdot CX_{0,2} \cdot CX_{1,0} \cdot X_2 \cdot CX_{0,2} \cdot CX_{0,1} \cdot w_{10} \cdot w_8} \\
& \xrightarrow{\omega_{21}} \overline{X_0 \cdot CX_{0,2} \cdot X_0} \cdot CX_{0,1} \cdot CX_{0,2} \cdot CX_{1,0} \cdot X_2 \cdot CX_{0,2} \cdot CX_{0,1} \cdot w_{10} \cdot w_8 \\
& \xleftarrow{C_{120}} \overline{X_0 \cdot X_0 \cdot X_2 \cdot CX_{0,2} \cdot CX_{0,1} \cdot CX_{0,2} \cdot CX_{1,0} \cdot X_2 \cdot CX_{0,2} \cdot CX_{0,1} \cdot w_{10} \cdot w_8} \\
& \xrightarrow{(21)} X_2 \cdot CX_{0,2} \cdot \overline{CX_{0,1} \cdot CX_{0,2}} \cdot CX_{1,0} \cdot X_2 \cdot CX_{0,2} \cdot CX_{0,1} \cdot w_{10} \cdot w_8 \\
& \xrightarrow{C_{22}} X_2 \cdot \overline{CX_{0,2} \cdot CX_{0,1}} \cdot CX_{1,0} \cdot X_2 \cdot CX_{0,2} \cdot CX_{0,1} \cdot w_{10} \cdot w_8 \\
& \xrightarrow{E_{15}} X_2 \cdot \overline{CX_{0,1}} \cdot CX_{1,0} \cdot X_2 \cdot CX_{0,2} \cdot CX_{0,1} \cdot w_{10} \cdot w_8 \\
& \xleftarrow{B_{16}} \overline{CX_{0,1} \cdot X_2 \cdot CX_{1,0} \cdot X_2 \cdot CX_{0,2} \cdot CX_{0,1} \cdot w_{10} \cdot w_8} \\
& \xleftarrow{B_{21}} CX_{0,1} \cdot \overline{CX_{1,0} \cdot X_2 \cdot X_2} \cdot CX_{0,2} \cdot CX_{0,1} \cdot w_{10} \cdot w_8 \\
& \xrightarrow{E_{17}} CX_{0,1} \cdot CX_{1,0} \cdot \overline{CX_{0,2} \cdot CX_{0,1}} \cdot w_{10} \cdot w_8 \\
& \xleftarrow{C_{22}} \overline{CX_{0,1} \cdot CX_{1,0} \cdot CX_{0,1} \cdot CX_{0,2}} \cdot w_{10} \cdot w_8 \\
& \xleftarrow{(13)} \overline{\sigma_{0,1} \cdot CX_{0,2} \cdot w_{10} \cdot w_8} \\
& \xrightarrow{\omega_{21}} \sigma_{0,1} \cdot CX_{0,2} \cdot \overline{X_0 \cdot CX_{0,2} \cdot X_0} \cdot w_8 \\
& \xrightarrow{C_{118}} \sigma_{0,1} \cdot CX_{0,2} \cdot \overline{CX_{0,2} \cdot X_2 \cdot X_0 \cdot X_0} \cdot w_8 \\
& \xrightarrow{(21)} \sigma_{0,1} \cdot CX_{0,2} \cdot CX_{0,2} \cdot X_2 \cdot \overline{w_8} \\
& \xrightarrow{\omega_{22}} \sigma_{0,1} \cdot CX_{0,2} \cdot CX_{0,2} \cdot \overline{X_2 \cdot X_2} \\
& \xrightarrow{E_{17}} \sigma_{0,1} \cdot \overline{CX_{0,2} \cdot CX_{0,2}} \\
& \xrightarrow{E_{15}} \sigma_{0,1}
\end{aligned}$$
  

$$\begin{aligned}
(\omega_{24}) : \underline{w_{12}} & \xrightarrow{W_{12}} \overline{r_2 \cdot r_6} \xrightarrow{D_6} r_2 \cdot \overline{CX_{2,1} \cdot CCX_{0,1} \cdot CX_{2,1}} \\
& \xrightarrow{D_2} \overline{X_0 \cdot CX_{2,1} \cdot CCX_{0,1} \cdot CX_{2,1} \cdot X_0 \cdot CX_{2,1} \cdot CCX_{0,1} \cdot CX_{2,1}} \\
& \xleftarrow{B_1} X_0 \cdot CX_{2,1} \cdot CCX_{0,1} \cdot CX_{2,1} \cdot \overline{CX_{2,1} \cdot X_0 \cdot CCX_{0,1} \cdot CX_{2,1}} \\
& \xrightarrow{(42)} X_0 \cdot CX_{2,1} \cdot CCX_{0,1} \cdot \overline{CX_{2,1} \cdot CX_{2,1} \cdot CCX_{0,1} \cdot CX_{1,2} \cdot X_0} \cdot CX_{2,1} \\
& \xrightarrow{E_9} X_0 \cdot CX_{2,1} \cdot \overline{CCX_{0,1} \cdot CCX_{0,1}} \cdot CX_{1,2} \cdot X_0 \cdot CX_{2,1} \\
& \xrightarrow{E_{18}} \overline{X_0 \cdot CX_{2,1} \cdot CX_{1,2} \cdot X_0 \cdot CX_{2,1}} \\
& \xleftarrow{B_1} \overline{CX_{2,1} \cdot X_0 \cdot CX_{1,2} \cdot X_0 \cdot CX_{2,1}} \\
& \xleftarrow{(26)} CX_{2,1} \cdot \overline{CX_{1,2} \cdot X_0 \cdot X_0} \cdot CX_{2,1} \\
& \xrightarrow{(21)} CX_{2,1} \cdot \overline{CX_{1,2} \cdot CX_{2,1}} \\
& \xrightarrow{C_9} CX_{2,1} \cdot \overline{CX_{2,1} \cdot \sigma_{1,2}} \\
& \xrightarrow{E_9} \sigma_{1,2}
\end{aligned}$$
  

$$(\omega_{25}) : \underline{w_{13}} \xrightarrow{W_{13}} \overline{w_{11} \cdot w_{12} \cdot w_{11}} \xrightarrow{\omega_{23}} w_{11} \cdot \overline{w_{12} \cdot \sigma_{0,1}} \xrightarrow{\omega_{24}} \overline{w_{11} \cdot \sigma_{1,2} \cdot \sigma_{0,1}} \xrightarrow{\omega_{23}} \overline{\sigma_{0,1} \cdot \sigma_{1,2} \cdot \sigma_{0,1}} \xleftarrow{S_3} \overline{\sigma_{0,2}}$$

## 1.5 Elimination of the Circuit Definitions

This section derives the relations for  $X_0$ ,  $CX_{0,1}$ ,  $CCX_{1,2}$ , and  $K_{1,2}$ , as introduced in Section 4.1 of the main paper.

### 1.5.1 Deriving the X-Operator

$$w_{13} \cdot w_8 \cdot \underline{w_{13}} \xrightarrow{\omega_{25}} w_{13} \cdot \underline{w_8} \cdot \underline{\sigma_{0,2}} \xrightarrow{\omega_{22}} \underline{w_{13}} \cdot \underline{\overline{X_2}} \cdot \sigma_{0,2} \xrightarrow{\omega_{25}} \underline{\sigma_{0,2}} \cdot \underline{X_2} \cdot \sigma_{0,2} \xrightarrow{(15)} \sigma_{0,2} \cdot \underline{\sigma_{0,2}} \cdot \underline{X_0} \cdot \underline{\sigma_{0,2}} \cdot \sigma_{0,2} \xrightarrow{E_{16}} \underline{\sigma_{0,2}} \cdot \underline{\sigma_{0,2}} \cdot X_0 \xrightarrow{E_{16}} X_0$$

### 1.5.2 Deriving the Controlled X-Operator

$$\begin{aligned} w_{12} \cdot X_0 \cdot \underline{w_{10}} \cdot X_0 \cdot w_{12} &\xrightarrow{\omega_{21}} w_{12} \cdot X_0 \cdot \underline{\overline{CX_{0,2}} \cdot \overline{X_0} \cdot X_0} \cdot w_{12} \xrightarrow{(21)} w_{12} \cdot \underline{X_0} \cdot \underline{X_0} \cdot CX_{0,2} \cdot w_{12} \xrightarrow{(21)} w_{12} \cdot CX_{0,2} \cdot \underline{w_{12}} \\ &\xrightarrow{\omega_{24}} \underline{w_{12}} \cdot CX_{0,2} \cdot \underline{\sigma_{1,2}} \\ &\xrightarrow{\omega_{24}} \underline{\sigma_{1,2}} \cdot CX_{0,2} \cdot \sigma_{1,2} \\ &\xrightarrow{(9)} \sigma_{1,2} \cdot \underline{\sigma_{1,2}} \cdot \underline{CX_{0,1}} \cdot \underline{\sigma_{1,2}} \cdot \sigma_{1,2} \\ &\xrightarrow{E_{10}} \sigma_{1,2} \cdot \underline{\sigma_{1,2}} \cdot CX_{0,1} \\ &\xrightarrow{E_{10}} CX_{0,1} \end{aligned}$$

### 1.5.3 Deriving the Doubly Controlled X-Operator

$$w_{13} \cdot w_7 \cdot \underline{w_{13}} \xrightarrow{\omega_{25}} w_{13} \cdot \underline{w_7} \cdot \underline{\sigma_{0,2}} \xrightarrow{\omega_{20}} \underline{w_{13}} \cdot \underline{CCX_{0,1}} \cdot \sigma_{0,2} \xrightarrow{\omega_{25}} \underline{\sigma_{0,2}} \cdot \underline{CCX_{0,1}} \cdot \sigma_{0,2} \xrightarrow{(32)} \sigma_{0,2} \cdot \underline{\sigma_{0,2}} \cdot \underline{CCX_{1,2}} \cdot \underline{\sigma_{0,2}} \cdot \sigma_{0,2} \xrightarrow{E_{16}} \underline{\sigma_{0,2}} \cdot \underline{\sigma_{0,2}} \cdot CCX_{1,2} \xrightarrow{E_{16}} CCX_{1,2}$$

### 1.5.4 Deriving the K-Operator

This section introduces several lemmas to derive the  $K_{1,2}$  gate. These lemmas are not used in other sections, and are denoted  $K_1$  through to  $K_5$ .

$$\begin{aligned} (K_1) : \underline{w_9} &\xrightarrow{W_6} r_6 \cdot \underline{w_7} \cdot \underline{w_1} \cdot \underline{w_7} \cdot r_6 \xrightarrow{\omega_{20}} r_6 \cdot \underline{w_7} \cdot \underline{w_1} \cdot \underline{CCX_{0,1}} \cdot r_6 \xrightarrow{\omega_3} r_6 \cdot \underline{w_7} \cdot \underline{\overline{CZ_{0,2}} \cdot \overline{CZ_{0,1}}} \cdot CCX_{0,1} \cdot r_6 \\ &\xrightarrow{\omega_{20}} r_6 \cdot \underline{\overline{CCX_{0,1}}} \cdot \underline{CZ_{0,2}} \cdot \underline{CZ_{0,1}} \cdot CCX_{0,1} \cdot r_6 \\ &\xleftarrow{C_{110}} r_6 \cdot \underline{\overline{CZ_{0,2}} \cdot \overline{CZ_{0,1}} \cdot \overline{CCX_{0,1}}} \cdot CZ_{0,1} \cdot CCX_{0,1} \cdot r_6 \\ &\xrightarrow{C_{95}} r_6 \cdot CZ_{0,2} \cdot \underline{\overline{CCX_{0,1}}} \cdot \underline{\overline{CZ_{0,1}}} \cdot \underline{CZ_{0,1}} \cdot CCX_{0,1} \cdot r_6 \\ &\xrightarrow{E_2} r_6 \cdot CZ_{0,2} \cdot \underline{CCX_{0,1}} \cdot \underline{CCX_{0,1}} \cdot r_6 \\ &\xrightarrow{E_{18}} r_6 \cdot CZ_{0,2} \cdot r_6 \\ &\xrightarrow{D_6} r_6 \cdot \underline{CZ_{0,2}} \cdot \underline{\overline{CX_{2,1}}} \cdot \underline{CCX_{0,1}} \cdot \underline{CX_{2,1}} \\ &\xrightarrow{D_6} \underline{CX_{2,1}} \cdot \underline{CCX_{0,1}} \cdot \underline{CX_{2,1}} \cdot \underline{CZ_{0,2}} \cdot CX_{2,1} \cdot CCX_{0,1} \cdot CX_{2,1} \\ &\xrightarrow{C_{66}} CX_{2,1} \cdot CCX_{0,1} \cdot \underline{\overline{CZ_{0,2}}} \cdot \underline{\overline{CX_{2,1}}} \cdot CX_{2,1} \cdot CCX_{0,1} \cdot CX_{2,1} \end{aligned}$$

$$\begin{aligned}
& \xrightarrow{E_9} CX_{2,1} \cdot CCX_{0,1} \cdot \overline{CZ_{0,2} \cdot CCX_{0,1} \cdot CX_{2,1}} \\
& \xrightarrow{C_{81}} CX_{2,1} \cdot \overline{CCX_{0,1} \cdot \overline{CCX_{0,1} \cdot CZ_{0,1} \cdot CZ_{0,2} \cdot CX_{2,1}}} \\
& \xrightarrow{E_{18}} CX_{2,1} \cdot CZ_{0,1} \cdot \overline{CZ_{0,2} \cdot CX_{2,1}} \\
& \xleftarrow{C_{66}} CX_{2,1} \cdot \overline{CZ_{0,1} \cdot \overline{CX_{2,1} \cdot CZ_{0,2}}} \\
& \xrightarrow{C_{121}} CX_{2,1} \cdot \overline{CX_{2,1} \cdot CZ_{0,1} \cdot \overline{CZ_{0,2} \cdot CZ_{0,2}}} \\
& \xrightarrow{E_{11}} \overline{CX_{2,1} \cdot CX_{2,1}} \cdot CZ_{0,1} \xrightarrow{E_9} CZ_{0,1}
\end{aligned}$$
  

$$\begin{aligned}
(K_2) : \underline{w_3} \cdot w_5 & \xrightarrow{\omega_{11}} \overline{CCX_{1,2} \cdot X_1 \cdot \overline{CCX_{0,2} \cdot CZ_{0,1} \cdot CCX_{0,2} \cdot X_1 \cdot CCX_{1,2}} \cdot w_5} \\
& \xleftarrow{C_{111}} \overline{CCX_{1,2} \cdot X_1 \cdot \overline{CZ_{0,1} \cdot CZ_{0,2} \cdot \overline{CCX_{0,2} \cdot CCX_{0,2} \cdot X_1 \cdot CCX_{1,2}} \cdot w_5}} \\
& \xrightarrow{E_7} \overline{CCX_{1,2} \cdot X_1 \cdot \overline{CZ_{0,1} \cdot CZ_{0,2} \cdot X_1 \cdot CCX_{1,2}} \cdot w_5} \\
& \xrightarrow{C_{60}} \overline{CCX_{1,2} \cdot X_1 \cdot \overline{CZ_{0,2} \cdot \overline{CZ_{0,1} \cdot X_1 \cdot CCX_{1,2}} \cdot w_5}} \\
& \xrightarrow{B_{35}} \overline{CCX_{1,2} \cdot \overline{CZ_{0,2} \cdot X_1 \cdot CZ_{0,1}} \cdot X_1 \cdot CCX_{1,2} \cdot w_5} \\
& \xrightarrow{C_{70}} \overline{CCX_{1,2} \cdot CZ_{0,2} \cdot \overline{CZ_{0,1} \cdot Z_0 \cdot X_1 \cdot X_1} \cdot CCX_{1,2} \cdot w_5} \\
& \xrightarrow{E_{13}} \overline{CCX_{1,2} \cdot CZ_{0,2} \cdot CZ_{0,1} \cdot \overline{Z_0 \cdot CCX_{1,2}} \cdot w_5} \\
& \xrightarrow{C_{49}} \overline{CCX_{1,2} \cdot CZ_{0,2} \cdot \overline{CZ_{0,1} \cdot \overline{CCX_{1,2} \cdot CZ_{1,2} \cdot Z_0} \cdot w_5}} \\
& \xrightarrow{C_{77}} \overline{CCX_{1,2} \cdot CZ_{0,2} \cdot \overline{CCX_{1,2} \cdot CZ_{1,2} \cdot \overline{CZ_{0,1} \cdot CZ_{1,2}} \cdot Z_0} \cdot w_5} \\
& \xrightarrow{(40)} \overline{CCX_{1,2} \cdot CZ_{0,2} \cdot \overline{CCX_{1,2} \cdot \overline{CZ_{1,2} \cdot \overline{CZ_{1,2} \cdot CZ_{0,1}} \cdot Z_0} \cdot w_5}} \\
& \xrightarrow{E_{12}} \overline{CCX_{1,2} \cdot \overline{CZ_{0,2} \cdot \overline{CCX_{1,2} \cdot CZ_{0,1} \cdot Z_0} \cdot w_5}} \\
& \xrightarrow{C_{100}} \overline{CCX_{1,2} \cdot \overline{CCX_{1,2} \cdot CZ_{1,2} \cdot \overline{CZ_{0,2} \cdot CZ_{0,1} \cdot Z_0} \cdot w_5}} \\
& \xrightarrow{(24)} \overline{CZ_{1,2} \cdot CZ_{0,2} \cdot CZ_{0,1} \cdot Z_0 \cdot w_5} \\
& \xrightarrow{\omega_{13}} \overline{CZ_{1,2} \cdot CZ_{0,2} \cdot \overline{CZ_{0,1} \cdot Z_0 \cdot \overline{Z_1 \cdot Z_2 \cdot \overline{CZ_{0,1} \cdot CZ_{0,2}}}}} \\
& \xrightarrow{C_{88}} \overline{CZ_{1,2} \cdot CZ_{0,2} \cdot \overline{Z_0 \cdot \overline{CZ_{0,1} \cdot Z_1 \cdot Z_2 \cdot CZ_{0,1} \cdot CZ_{0,2}}}} \\
& \xrightarrow{C_{55}} \overline{CZ_{1,2} \cdot CZ_{0,2} \cdot Z_0 \cdot \overline{Z_1 \cdot \overline{CZ_{0,1} \cdot Z_2 \cdot CZ_{0,1} \cdot CZ_{0,2}}}} \\
& \xrightarrow{B_{27}} \overline{CZ_{1,2} \cdot CZ_{0,2} \cdot Z_0 \cdot Z_1 \cdot \overline{Z_2 \cdot \overline{CZ_{0,1} \cdot CZ_{0,1} \cdot CZ_{0,2}}}} \\
& \xrightarrow{E_2} \overline{CZ_{1,2} \cdot \overline{CZ_{0,2} \cdot Z_0 \cdot Z_1 \cdot Z_2 \cdot CZ_{0,2}}} \\
& \xrightarrow{C_{103}} \overline{CZ_{1,2} \cdot \overline{Z_0 \cdot \overline{CZ_{0,2} \cdot Z_1 \cdot Z_2 \cdot CZ_{0,2}}}} \\
& \xrightarrow{B_{20}} \overline{CZ_{1,2} \cdot Z_0 \cdot \overline{Z_1 \cdot \overline{CZ_{0,2} \cdot Z_2 \cdot CZ_{0,2}}}} \\
& \xrightarrow{C_{78}} \overline{CZ_{1,2} \cdot Z_0 \cdot Z_1 \cdot \overline{Z_2 \cdot \overline{CZ_{0,2} \cdot CZ_{0,2}}}} \\
& \xrightarrow{E_{11}} \overline{CZ_{1,2} \cdot Z_0 \cdot Z_1 \cdot Z_2}
\end{aligned}$$

$$(K_3) : \underline{w_2} \cdot w_9 \xrightarrow{\omega_5} \overline{X_1 \cdot CZ_{0,1} \cdot X_1} \cdot w_9 \xrightarrow{C_{70}} \overline{CZ_{0,1} \cdot Z_0 \cdot X_1 \cdot X_1} \cdot w_9 \xrightarrow{E_{13}} CZ_{0,1} \cdot Z_0 \cdot \underline{w_9} \xrightarrow{K_1} \underline{CZ_{0,1} \cdot Z_0} \cdot \overline{CZ_{0,1}} \xrightarrow{C_{88}} \overline{Z_0 \cdot CZ_{0,1} \cdot CZ_{0,1}} \xrightarrow{E_2} Z_0$$

$$(K_4) : w_3 \cdot w_5 \cdot \underline{w_2} \cdot w_9 \xrightarrow{K_3} \underline{w_3 \cdot w_5} \cdot \overline{Z_0} \xrightarrow{K_2} \overline{CZ_{1,2} \cdot Z_0 \cdot Z_1 \cdot Z_2} \cdot Z_0 \xrightarrow{B_{29}} CZ_{1,2} \cdot \overline{Z_1 \cdot Z_0} \cdot Z_2 \cdot Z_0 \xrightarrow{B_{28}} CZ_{1,2} \cdot Z_1 \cdot \overline{Z_2 \cdot Z_0} \cdot Z_0 \xrightarrow{E_3} CZ_{1,2} \cdot Z_1 \cdot Z_2$$

$$\begin{aligned} (K_5) : r_8 \cdot \underline{w_2} \cdot w_9 \cdot r_8 &\xrightarrow{K_3} r_8 \cdot \overline{Z_0} \cdot r_8 \\ &\xrightarrow{D_8} \overline{r_8 \cdot Z_0 \cdot \overline{K_{1,2} \cdot X_1 \cdot X_2 \cdot CZ_{0,2} \cdot CCX_{1,2} \cdot CZ_{0,2} \cdot X_2 \cdot X_1 \cdot K_{1,2}}} \\ &\xrightarrow{D_8} \overline{K_{1,2} \cdot X_1 \cdot X_2 \cdot CZ_{0,2} \cdot CCX_{1,2} \cdot CZ_{0,2} \cdot X_2 \cdot X_1 \cdot \overline{K_{1,2} \cdot Z_0} \cdot K_{1,2} \cdot X_1 \cdot X_2 \cdot CZ_{0,2} \cdot CCX_{1,2} \cdot CZ_{0,2} \cdot X_2 \cdot X_1 \cdot K_{1,2}} \\ &\xleftarrow{B_6} K_{1,2} \cdot X_1 \cdot X_2 \cdot CZ_{0,2} \cdot CCX_{1,2} \cdot CZ_{0,2} \cdot X_2 \cdot X_1 \cdot \overline{Z_0 \cdot \overline{K_{1,2} \cdot K_{1,2}}} \cdot X_1 \cdot X_2 \cdot CZ_{0,2} \cdot CCX_{1,2} \cdot CZ_{0,2} \cdot X_2 \cdot X_1 \cdot K_{1,2} \\ &\xrightarrow{(23)} K_{1,2} \cdot X_1 \cdot X_2 \cdot CZ_{0,2} \cdot CCX_{1,2} \cdot CZ_{0,2} \cdot X_2 \cdot \overline{X_1 \cdot Z_0} \cdot X_1 \cdot X_2 \cdot CZ_{0,2} \cdot CCX_{1,2} \cdot CZ_{0,2} \cdot X_2 \cdot X_1 \cdot K_{1,2} \\ &\xrightarrow{B_{15}} K_{1,2} \cdot X_1 \cdot X_2 \cdot CZ_{0,2} \cdot CCX_{1,2} \cdot CZ_{0,2} \cdot X_2 \cdot \overline{Z_0 \cdot \overline{X_1 \cdot X_1}} \cdot X_2 \cdot CZ_{0,2} \cdot CCX_{1,2} \cdot CZ_{0,2} \cdot X_2 \cdot X_1 \cdot K_{1,2} \\ &\xrightarrow{E_{13}} K_{1,2} \cdot X_1 \cdot X_2 \cdot CZ_{0,2} \cdot CCX_{1,2} \cdot CZ_{0,2} \cdot \underline{X_2 \cdot Z_0} \cdot X_2 \cdot CZ_{0,2} \cdot CCX_{1,2} \cdot CZ_{0,2} \cdot X_2 \cdot X_1 \cdot K_{1,2} \\ &\xrightarrow{B_{23}} K_{1,2} \cdot X_1 \cdot X_2 \cdot CZ_{0,2} \cdot CCX_{1,2} \cdot CZ_{0,2} \cdot \overline{Z_0 \cdot \overline{X_2 \cdot X_2}} \cdot CZ_{0,2} \cdot CCX_{1,2} \cdot CZ_{0,2} \cdot X_2 \cdot X_1 \cdot K_{1,2} \\ &\xrightarrow{E_{17}} K_{1,2} \cdot X_1 \cdot X_2 \cdot CZ_{0,2} \cdot CCX_{1,2} \cdot \underline{CZ_{0,2} \cdot Z_0} \cdot CZ_{0,2} \cdot CCX_{1,2} \cdot CZ_{0,2} \cdot X_2 \cdot X_1 \cdot K_{1,2} \\ &\xrightarrow{C_{103}} K_{1,2} \cdot X_1 \cdot X_2 \cdot CZ_{0,2} \cdot CCX_{1,2} \cdot \overline{Z_0 \cdot CZ_{0,2}} \cdot CZ_{0,2} \cdot CCX_{1,2} \cdot CZ_{0,2} \cdot X_2 \cdot X_1 \cdot K_{1,2} \\ &\xrightarrow{E_{11}} K_{1,2} \cdot X_1 \cdot X_2 \cdot CZ_{0,2} \cdot CCX_{1,2} \cdot \underline{Z_0 \cdot CCX_{1,2}} \cdot CZ_{0,2} \cdot X_2 \cdot X_1 \cdot K_{1,2} \\ &\xrightarrow{C_{49}} K_{1,2} \cdot X_1 \cdot X_2 \cdot CZ_{0,2} \cdot \underline{CCX_{1,2} \cdot \overline{CCX_{1,2}}} \cdot \overline{CZ_{1,2} \cdot Z_0} \cdot CZ_{0,2} \cdot X_2 \cdot X_1 \cdot K_{1,2} \\ &\xrightarrow{(24)} K_{1,2} \cdot X_1 \cdot X_2 \cdot \underline{CZ_{0,2} \cdot CZ_{1,2}} \cdot Z_0 \cdot CZ_{0,2} \cdot X_2 \cdot X_1 \cdot K_{1,2} \\ &\xrightarrow{C_{71}} K_{1,2} \cdot X_1 \cdot X_2 \cdot \overline{CZ_{1,2} \cdot CZ_{0,2}} \cdot Z_0 \cdot CZ_{0,2} \cdot X_2 \cdot X_1 \cdot K_{1,2} \\ &\xrightarrow{C_{103}} K_{1,2} \cdot X_1 \cdot X_2 \cdot CZ_{1,2} \cdot \overline{Z_0 \cdot CZ_{0,2}} \cdot CZ_{0,2} \cdot X_2 \cdot X_1 \cdot K_{1,2} \\ &\xrightarrow{E_{11}} K_{1,2} \cdot X_1 \cdot X_2 \cdot CZ_{1,2} \cdot Z_0 \cdot X_2 \cdot X_1 \cdot K_{1,2} \end{aligned}$$

$$\begin{aligned} \underline{r_2 \cdot r_6} \cdot w_3 \cdot w_5 \cdot r_8 \cdot w_2 \cdot w_9 \cdot r_8 \cdot w_3 \cdot w_5 \cdot w_2 \cdot w_9 &\xleftarrow{W_{12}} \overline{w_{12} \cdot w_3 \cdot w_5 \cdot r_8 \cdot w_2 \cdot w_9 \cdot r_8 \cdot w_3 \cdot w_5 \cdot w_2 \cdot w_9} \\ &\xrightarrow{K_5} \overline{w_{12} \cdot \underline{w_3 \cdot w_5} \cdot \overline{K_{1,2} \cdot X_1 \cdot X_2 \cdot CZ_{1,2} \cdot Z_0 \cdot X_2 \cdot X_1 \cdot K_{1,2}}} \cdot w_3 \cdot w_5 \cdot w_2 \cdot w_9 \\ &\xrightarrow{K_2} w_{12} \cdot \overline{CZ_{1,2} \cdot Z_0 \cdot Z_1 \cdot \underline{Z_2} \cdot K_{1,2}} \cdot X_1 \cdot X_2 \cdot CZ_{1,2} \cdot Z_0 \cdot X_2 \cdot X_1 \cdot K_{1,2} \cdot w_3 \cdot w_5 \cdot w_2 \cdot w_9 \\ &\xleftarrow{C_{26}} w_{12} \cdot CZ_{1,2} \cdot Z_0 \cdot Z_1 \cdot \overline{K_{1,2} \cdot \underline{X_2} \cdot X_1 \cdot X_2} \cdot CZ_{1,2} \cdot Z_0 \cdot X_2 \cdot X_1 \cdot K_{1,2} \cdot w_3 \cdot w_5 \cdot w_2 \cdot w_9 \\ &\xleftarrow{B_{19}} w_{12} \cdot CZ_{1,2} \cdot Z_0 \cdot Z_1 \cdot K_{1,2} \cdot \overline{X_1 \cdot \underline{X_2} \cdot X_2} \cdot CZ_{1,2} \cdot Z_0 \cdot X_2 \cdot X_1 \cdot K_{1,2} \cdot w_3 \cdot w_5 \cdot w_2 \cdot w_9 \\ &\xrightarrow{E_{17}} w_{12} \cdot CZ_{1,2} \cdot Z_0 \cdot \underline{Z_1 \cdot K_{1,2}} \cdot X_1 \cdot CZ_{1,2} \cdot Z_0 \cdot X_2 \cdot X_1 \cdot K_{1,2} \cdot w_3 \cdot w_5 \cdot w_2 \cdot w_9 \\ &\xleftarrow{C_{27}} w_{12} \cdot CZ_{1,2} \cdot Z_0 \cdot \overline{K_{1,2} \cdot \underline{X_1} \cdot X_1} \cdot CZ_{1,2} \cdot Z_0 \cdot X_2 \cdot X_1 \cdot K_{1,2} \cdot w_3 \cdot w_5 \cdot w_2 \cdot w_9 \\ &\xrightarrow{E_{13}} w_{12} \cdot CZ_{1,2} \cdot \underline{Z_0 \cdot K_{1,2}} \cdot CZ_{1,2} \cdot Z_0 \cdot X_2 \cdot X_1 \cdot K_{1,2} \cdot w_3 \cdot w_5 \cdot w_2 \cdot w_9 \\ &\xrightarrow{B_6} w_{12} \cdot CZ_{1,2} \cdot \overline{K_{1,2} \cdot Z_0} \cdot \underline{CZ_{1,2}} \cdot Z_0 \cdot X_2 \cdot X_1 \cdot K_{1,2} \cdot w_3 \cdot w_5 \cdot w_2 \cdot w_9 \end{aligned}$$

$$\begin{aligned}
& \xleftarrow{B_{31}} w_{12} \cdot CZ_{1,2} \cdot K_{1,2} \cdot \overline{CZ_{1,2} \cdot Z_0 \cdot X_2 \cdot X_1 \cdot K_{1,2} \cdot w_3 \cdot w_5 \cdot w_2 \cdot w_9} \\
& \xrightarrow{E_3} w_{12} \cdot CZ_{1,2} \cdot K_{1,2} \cdot CZ_{1,2} \cdot X_2 \cdot X_1 \cdot K_{1,2} \cdot w_3 \cdot w_5 \cdot w_2 \cdot w_9 \\
& \xrightarrow{K_4} w_{12} \cdot CZ_{1,2} \cdot K_{1,2} \cdot CZ_{1,2} \cdot X_2 \cdot X_1 \cdot K_{1,2} \cdot \overline{CZ_{1,2} \cdot Z_1 \cdot Z_2} \\
& \xrightarrow{C_2} w_{12} \cdot CZ_{1,2} \cdot K_{1,2} \cdot CZ_{1,2} \cdot X_2 \cdot \overline{K_{1,2} \cdot Z_1 \cdot CZ_{1,2} \cdot Z_1 \cdot Z_2} \\
& \xrightarrow{C_{124}} w_{12} \cdot CZ_{1,2} \cdot K_{1,2} \cdot CZ_{1,2} \cdot X_2 \cdot K_{1,2} \cdot \overline{CZ_{1,2} \cdot Z_1 \cdot Z_1 \cdot Z_2} \\
& \xrightarrow{E_5} w_{12} \cdot CZ_{1,2} \cdot K_{1,2} \cdot CZ_{1,2} \cdot \underline{X_2 \cdot K_{1,2}} \cdot CZ_{1,2} \cdot Z_2 \\
& \xrightarrow{C_{16}} w_{12} \cdot CZ_{1,2} \cdot K_{1,2} \cdot CZ_{1,2} \cdot \overline{K_{1,2} \cdot Z_2} \cdot CZ_{1,2} \cdot Z_2 \\
& \xleftarrow{C_{91}} w_{12} \cdot CZ_{1,2} \cdot K_{1,2} \cdot CZ_{1,2} \cdot K_{1,2} \cdot \overline{CZ_{1,2} \cdot Z_2 \cdot Z_2} \\
& \xrightarrow{E_{19}} w_{12} \cdot CZ_{1,2} \cdot K_{1,2} \cdot CZ_{1,2} \cdot K_{1,2} \cdot CZ_{1,2} \\
& \xrightarrow{\omega_{24}} \overline{\sigma_{1,2}} \cdot CZ_{1,2} \cdot K_{1,2} \cdot CZ_{1,2} \cdot K_{1,2} \cdot CZ_{1,2} \\
& \xleftarrow{(23)} \sigma_{1,2} \cdot \underline{CZ_{1,2} \cdot K_{1,2} \cdot CZ_{1,2} \cdot K_{1,2} \cdot CZ_{1,2} \cdot \overline{K_{1,2} \cdot K_{1,2}}} \\
& \xleftarrow{(20)} \underline{\sigma_{1,2} \cdot \overline{\sigma_{1,2}}} \cdot K_{1,2} \xrightarrow{E_{10}} K_{1,2}
\end{aligned}$$

## 1.6 Some Lemmas to Eliminate the Coxeter Relations

This section derives lemmas to help eliminate the relations in  $R_{E8}$ . The  $n$ -th lemma in this section is denoted  $\xi_n$ . Note that relations of the form  $(k; j)$  do not appear in any of the derivations in this section.

$$\begin{aligned}
(\xi_2) : \underline{r_7} & \xrightarrow{D_7} \overline{CZ_{0,1} \cdot CX_{2,1} \cdot CCX_{0,1} \cdot CX_{2,1} \cdot CZ_{0,1}} & (\xi_3) : \underline{r_6} \cdot CZ_{0,2} \cdot CZ_{0,1} & \xrightarrow{D_6} \overline{CX_{2,1} \cdot CCX_{0,1} \cdot CX_{2,1} \cdot CZ_{0,2} \cdot CZ_{0,1}} \\
& \xrightarrow{C_{121}} \overline{CX_{2,1} \cdot CZ_{0,1} \cdot CZ_{0,2} \cdot CCX_{0,1} \cdot CX_{2,1} \cdot CZ_{0,1}} & & \xleftarrow{C_{60}} CX_{2,1} \cdot CCX_{0,1} \cdot \underline{CX_{2,1} \cdot CZ_{0,1} \cdot CZ_{0,2}} \\
& \xrightarrow{C_{60}} CX_{2,1} \cdot \overline{CZ_{0,2} \cdot CZ_{0,1} \cdot CCX_{0,1} \cdot CX_{2,1} \cdot CZ_{0,1}} & & \xleftarrow{C_{121}} CX_{2,1} \cdot \underline{CCX_{0,1} \cdot CZ_{0,1} \cdot CX_{2,1}} \\
& \xrightarrow{C_{110}} CX_{2,1} \cdot \overline{CCX_{0,1} \cdot CZ_{0,2} \cdot CX_{2,1} \cdot CZ_{0,1}} & & \xleftarrow{C_{95}} CX_{2,1} \cdot \overline{CZ_{0,1} \cdot CCX_{0,1} \cdot CX_{2,1}} \\
& \xleftarrow{C_{66}} \underline{CX_{2,1} \cdot CCX_{0,1} \cdot \overline{CX_{2,1} \cdot CZ_{0,2} \cdot CZ_{0,1}}} & & \xleftarrow{E_{11}} \underline{CX_{2,1} \cdot CZ_{0,1} \cdot \overline{CZ_{0,2} \cdot CZ_{0,2} \cdot CCX_{0,1} \cdot CX_{2,1}}} \\
& \xleftarrow{D_6} \overline{r_6} \cdot CZ_{0,2} \cdot CZ_{0,1} & & \xleftarrow{C_{121}} \overline{CZ_{0,1} \cdot CX_{2,1} \cdot CZ_{0,2} \cdot CCX_{0,1} \cdot CX_{2,1}} \\
& & & \xrightarrow{C_{66}} \underline{CZ_{0,1} \cdot CZ_{0,2} \cdot CX_{2,1} \cdot CCX_{0,1} \cdot CX_{2,1}} \\
& & & \xrightarrow{C_{60}} \overline{CZ_{0,2} \cdot CZ_{0,1} \cdot CX_{2,1} \cdot CCX_{0,1} \cdot CX_{2,1}} \\
& & & \xleftarrow{D_6} CZ_{0,2} \cdot CZ_{0,1} \cdot \overline{r_6} \\
(\xi_3) : \underline{r_7} & \xrightarrow{D_7} \overline{CZ_{0,1} \cdot CX_{2,1} \cdot CCX_{0,1} \cdot CX_{2,1} \cdot CZ_{0,1}} \xleftarrow{D_6} CZ_{0,1} \cdot \overline{r_6} \cdot CZ_{0,1} \\
(\xi_4) : X_0 \cdot \underline{r_8} & \xrightarrow{D_8} \underline{X_0 \cdot \overline{K_{1,2} \cdot X_1 \cdot X_2 \cdot CZ_{0,2} \cdot CCX_{1,2} \cdot CZ_{0,2} \cdot X_2 \cdot X_1 \cdot K_{1,2}}} \\
& \xrightarrow{(27)} \overline{K_{1,2} \cdot X_0 \cdot X_1 \cdot X_2 \cdot CZ_{0,2} \cdot CCX_{1,2} \cdot CZ_{0,2} \cdot X_2 \cdot X_1 \cdot K_{1,2}}
\end{aligned}$$

$$\begin{aligned}
& \xrightarrow{B_2} K_{1,2} \cdot \overline{X_1 \cdot X_0} \cdot X_2 \cdot CZ_{0,2} \cdot CCX_{1,2} \cdot CZ_{0,2} \cdot X_2 \cdot X_1 \cdot K_{1,2} \\
& \xrightarrow{B_{13}} K_{1,2} \cdot X_1 \cdot \overline{X_2 \cdot X_0} \cdot CZ_{0,2} \cdot CCX_{1,2} \cdot CZ_{0,2} \cdot X_2 \cdot X_1 \cdot K_{1,2} \\
& \xrightarrow{C_{108}} K_{1,2} \cdot X_1 \cdot X_2 \cdot \overline{CZ_{0,2} \cdot Z_2 \cdot X_0} \cdot CCX_{1,2} \cdot CZ_{0,2} \cdot X_2 \cdot X_1 \cdot K_{1,2} \\
& \xrightarrow{(37)} K_{1,2} \cdot X_1 \cdot X_2 \cdot CZ_{0,2} \cdot Z_2 \cdot \overline{CCX_{1,2} \cdot X_0} \cdot CZ_{0,2} \cdot X_2 \cdot X_1 \cdot K_{1,2} \\
& \xrightarrow{C_{108}} K_{1,2} \cdot X_1 \cdot X_2 \cdot CZ_{0,2} \cdot Z_2 \cdot CCX_{1,2} \cdot \overline{CZ_{0,2} \cdot Z_2 \cdot X_0} \cdot X_2 \cdot X_1 \cdot K_{1,2} \\
& \xrightarrow{C_{78}} K_{1,2} \cdot X_1 \cdot X_2 \cdot CZ_{0,2} \cdot \overline{Z_2 \cdot CCX_{1,2}} \cdot \overline{Z_2 \cdot CZ_{0,2}} \cdot X_0 \cdot X_2 \cdot X_1 \cdot K_{1,2} \\
& \xrightarrow{C_{50}} K_{1,2} \cdot X_1 \cdot X_2 \cdot CZ_{0,2} \cdot \overline{CCX_{1,2} \cdot Z_2 \cdot Z_2} \cdot CZ_{0,2} \cdot X_0 \cdot X_2 \cdot X_1 \cdot K_{1,2} \\
& \xrightarrow{E_{19}} K_{1,2} \cdot X_1 \cdot X_2 \cdot CZ_{0,2} \cdot CCX_{1,2} \cdot CZ_{0,2} \cdot \overline{X_0 \cdot X_2} \cdot X_1 \cdot K_{1,2} \\
& \xrightarrow{B_{13}} K_{1,2} \cdot X_1 \cdot X_2 \cdot CZ_{0,2} \cdot CCX_{1,2} \cdot CZ_{0,2} \cdot \overline{X_2 \cdot X_0} \cdot X_1 \cdot K_{1,2} \\
& \xrightarrow{B_2} K_{1,2} \cdot X_1 \cdot X_2 \cdot CZ_{0,2} \cdot CCX_{1,2} \cdot CZ_{0,2} \cdot X_2 \cdot \overline{X_1 \cdot X_0} \cdot K_{1,2} \\
& \xrightarrow{(27)} K_{1,2} \cdot X_1 \cdot X_2 \cdot CZ_{0,2} \cdot CCX_{1,2} \cdot CZ_{0,2} \cdot X_2 \cdot X_1 \cdot \overline{K_{1,2} \cdot X_0} \\
& \xleftarrow{D_8} \overline{r_8} \cdot X_0
\end{aligned}$$

$$\begin{aligned}
(\xi_5) : CCX_{1,2} \cdot \overline{CCX_{0,1} \cdot CCX_{0,2} \cdot CCX_{0,1}} \cdot CCX_{1,2} & \xleftarrow{X_7} CCX_{1,2} \cdot \overline{CX_{1,2} \cdot CCX_{0,2} \cdot CX_{1,2}} \cdot CCX_{1,2} \\
& \xrightarrow{(44)} CCX_{1,2} \cdot CX_{1,2} \cdot CCX_{0,2} \cdot \overline{CCX_{1,2} \cdot CX_{1,0} \cdot CX_{1,2}} \\
& \xrightarrow{(36)} CCX_{1,2} \cdot CX_{1,2} \cdot CCX_{0,2} \cdot \overline{CX_{1,0} \cdot CCX_{1,2}} \cdot CX_{1,2} \\
& \xleftarrow{E_1} CCX_{1,2} \cdot \overline{CX_{1,0} \cdot CX_{1,2}} \cdot CCX_{0,2} \cdot CX_{1,0} \cdot CCX_{1,2} \cdot CX_{1,2} \\
& \xrightarrow{C_{94}} \overline{CCX_{1,2} \cdot CX_{1,0} \cdot CX_{1,2} \cdot CX_{1,0}} \cdot CCX_{0,2} \cdot CX_{1,0} \cdot CCX_{1,2} \cdot CX_{1,2} \\
& \xleftarrow{(44)} \overline{CX_{1,2} \cdot CCX_{1,2} \cdot CX_{1,0} \cdot CCX_{0,2} \cdot CX_{1,0} \cdot CCX_{1,2} \cdot CX_{1,2}} \\
& \xrightarrow{X_8} CX_{1,2} \cdot CCX_{1,2} \cdot \overline{CCX_{1,2} \cdot CCX_{0,2} \cdot CCX_{1,2} \cdot CCX_{1,2}} \cdot CX_{1,2} \\
& \xrightarrow{(24)} CX_{1,2} \cdot \overline{CCX_{1,2} \cdot CCX_{1,2}} \cdot CCX_{0,2} \cdot CX_{1,2} \\
& \xrightarrow{(24)} \overline{CX_{1,2} \cdot CCX_{0,2} \cdot CX_{1,2}} \\
& \xrightarrow{X_7} \overline{CCX_{0,1} \cdot CCX_{0,2} \cdot CCX_{0,1}}
\end{aligned}$$

$$\begin{aligned}
(\xi_6) : r_1 \cdot r_6 & \xrightarrow{D_6} r_1 \cdot \overline{CX_{2,1} \cdot CCX_{0,1} \cdot CX_{2,1}} \\
& \xrightarrow{D_1} \overline{X_0 \cdot X_1 \cdot CCX_{0,1} \cdot X_1 \cdot X_0} \cdot CX_{2,1} \cdot CCX_{0,1} \cdot CX_{2,1} \\
& \xrightarrow{C_{35}} X_0 \cdot \overline{CCX_{0,1} \cdot CX_{0,2} \cdot X_1 \cdot X_0} \cdot CX_{2,1} \cdot CCX_{0,1} \cdot CX_{2,1} \\
& \xrightarrow{E_{13}} \overline{X_0 \cdot CCX_{0,1} \cdot CX_{0,2} \cdot X_0 \cdot CX_{2,1} \cdot CCX_{0,1} \cdot CX_{2,1}} \\
& \xrightarrow{(42)} \overline{CCX_{0,1} \cdot CX_{1,2} \cdot X_0 \cdot CX_{0,2}} \cdot X_0 \cdot CX_{2,1} \cdot CCX_{0,1} \cdot CX_{2,1} \\
& \xrightarrow{C_{118}} CCX_{0,1} \cdot CX_{1,2} \cdot \overline{CX_{0,2} \cdot X_2 \cdot X_0 \cdot X_0} \cdot CX_{2,1} \cdot CCX_{0,1} \cdot CX_{2,1}
\end{aligned}$$

$$\begin{aligned}
& \xrightarrow{(21)} CCX_{0,1} \cdot CX_{1,2} \cdot CX_{0,2} \cdot X_2 \cdot CX_{2,1} \cdot CCX_{0,1} \cdot CX_{2,1} \\
& \xleftarrow{E_9} CCX_{0,1} \cdot \overline{CX_{2,1} \cdot CX_{2,1}} \cdot CX_{1,2} \cdot CX_{0,2} \cdot X_2 \cdot CX_{2,1} \cdot CCX_{0,1} \cdot CX_{2,1} \\
& \xleftarrow{E_9} \overline{CX_{2,1} \cdot CX_{2,1} \cdot CCX_{0,1} \cdot CX_{2,1}} \cdot CX_{2,1} \cdot CX_{1,2} \cdot CX_{0,2} \cdot X_2 \cdot CX_{2,1} \cdot CCX_{0,1} \cdot CX_{2,1} \\
& \xrightarrow{X_6} CX_{2,1} \cdot \overline{CCX_{0,2} \cdot CCX_{0,1} \cdot CCX_{0,2}} \cdot CX_{2,1} \cdot CX_{1,2} \cdot CX_{0,2} \cdot X_2 \cdot CX_{2,1} \cdot CCX_{0,1} \cdot CX_{2,1} \\
& \xrightarrow{X_9} CX_{2,1} \cdot \overline{CCX_{0,1} \cdot CCX_{0,2} \cdot CCX_{0,1}} \cdot CX_{2,1} \cdot CX_{1,2} \cdot CX_{0,2} \cdot X_2 \cdot CX_{2,1} \cdot CCX_{0,1} \cdot CX_{2,1} \\
& \xleftarrow{E_9} \overline{CX_{2,1} \cdot CCX_{0,1} \cdot CX_{2,1} \cdot CX_{2,1}} \cdot CCX_{0,2} \cdot CCX_{0,1} \cdot CX_{2,1} \cdot CX_{1,2} \cdot CX_{0,2} \cdot X_2 \cdot CX_{2,1} \cdot CCX_{0,1} \cdot CX_{2,1} \\
& \xleftarrow{D_6} \overline{r_6 \cdot CX_{2,1} \cdot CCX_{0,2} \cdot CCX_{0,1} \cdot CX_{2,1} \cdot CX_{1,2} \cdot CX_{0,2} \cdot X_2 \cdot CX_{2,1} \cdot CCX_{0,1} \cdot CX_{2,1}} \\
& \xleftarrow{C_{106}} r_6 \cdot \overline{CCX_{0,2} \cdot CX_{2,1} \cdot CCX_{0,1} \cdot CX_{2,1}} \cdot CX_{1,2} \cdot CX_{0,2} \cdot X_2 \cdot CX_{2,1} \cdot CCX_{0,1} \cdot CX_{2,1} \\
& \xrightarrow{X_6} r_6 \cdot \overline{CCX_{0,2} \cdot CCX_{0,2} \cdot CCX_{0,1} \cdot CCX_{0,2} \cdot CX_{1,2} \cdot CX_{0,2} \cdot X_2 \cdot CX_{2,1} \cdot CCX_{0,1} \cdot CX_{2,1}} \\
& \xrightarrow{E_7} r_6 \cdot CCX_{0,1} \cdot CCX_{0,2} \cdot \overline{CX_{1,2} \cdot CX_{0,2} \cdot X_2 \cdot CX_{2,1} \cdot CCX_{0,1} \cdot CX_{2,1}} \\
& \xrightarrow{C_{33}} r_6 \cdot CCX_{0,1} \cdot CCX_{0,2} \cdot \overline{CX_{0,2} \cdot CX_{1,2} \cdot X_2 \cdot CX_{2,1} \cdot CCX_{0,1} \cdot CX_{2,1}} \\
& \xleftarrow{C_{11}} r_6 \cdot CCX_{0,1} \cdot CCX_{0,2} \cdot CX_{0,2} \cdot \overline{X_2 \cdot CX_{1,2} \cdot CX_{2,1} \cdot CCX_{0,1} \cdot CX_{2,1}} \\
& \xrightarrow{X_{10}} r_6 \cdot CCX_{0,1} \cdot CCX_{0,2} \cdot CX_{0,2} \cdot X_2 \cdot \overline{CX_{1,2} \cdot CX_{1,2} \cdot CCX_{0,2} \cdot CX_{1,2}} \\
& \xrightarrow{E_8} r_6 \cdot CCX_{0,1} \cdot CCX_{0,2} \cdot CX_{0,2} \cdot \overline{X_2 \cdot CCX_{0,2} \cdot CX_{1,2}} \\
& \xrightarrow{C_{104}} r_6 \cdot CCX_{0,1} \cdot CCX_{0,2} \cdot \overline{CX_{0,2} \cdot CCX_{0,2} \cdot CX_{0,1} \cdot X_2 \cdot CX_{1,2}} \\
& \xrightarrow{C_{34}} r_6 \cdot CCX_{0,1} \cdot CCX_{0,2} \cdot \overline{CCX_{0,2} \cdot CX_{0,1} \cdot CX_{0,2} \cdot CX_{0,1} \cdot X_2 \cdot CX_{1,2}} \\
& \xrightarrow{C_{22}} r_6 \cdot CCX_{0,1} \cdot CCX_{0,2} \cdot \overline{CCX_{0,2} \cdot CX_{0,1} \cdot CX_{0,1} \cdot X_2 \cdot CX_{1,2}} \\
& \xrightarrow{(22)} r_6 \cdot CCX_{0,1} \cdot \overline{CCX_{0,2} \cdot CCX_{0,2} \cdot CX_{0,2} \cdot X_2 \cdot CX_{1,2}} \\
& \xrightarrow{E_7} r_6 \cdot CCX_{0,1} \cdot CX_{0,2} \cdot X_2 \cdot CX_{1,2} \\
& \xleftarrow{(21)} r_6 \cdot \overline{X_0 \cdot X_0} \cdot CCX_{0,1} \cdot CX_{0,2} \cdot X_2 \cdot CX_{1,2} \\
& \xleftarrow{E_{13}} r_6 \cdot X_0 \cdot \overline{X_1 \cdot X_1} \cdot \overline{X_0 \cdot CCX_{0,1} \cdot CX_{0,2} \cdot X_2 \cdot CX_{1,2}} \\
& \xrightarrow{(42)} r_6 \cdot X_0 \cdot X_1 \cdot X_1 \cdot \overline{CCX_{0,1} \cdot CX_{1,2} \cdot X_0} \cdot CX_{0,2} \cdot X_2 \cdot CX_{1,2} \\
& \xrightarrow{(26)} r_6 \cdot X_0 \cdot X_1 \cdot X_1 \cdot CCX_{0,1} \cdot \overline{X_0 \cdot CX_{1,2} \cdot CX_{0,2} \cdot X_2 \cdot CX_{1,2}} \\
& \xrightarrow{C_{33}} r_6 \cdot X_0 \cdot X_1 \cdot X_1 \cdot CCX_{0,1} \cdot X_0 \cdot \overline{CX_{0,2} \cdot CX_{1,2} \cdot X_2 \cdot CX_{1,2}} \\
& \xrightarrow{C_{11}} r_6 \cdot X_0 \cdot X_1 \cdot X_1 \cdot CCX_{0,1} \cdot X_0 \cdot CX_{0,2} \cdot \overline{CX_{1,2} \cdot CX_{1,2} \cdot X_2} \\
& \xrightarrow{E_8} r_6 \cdot X_0 \cdot X_1 \cdot X_1 \cdot \overline{CCX_{0,1} \cdot X_0 \cdot CX_{0,2} \cdot X_2} \\
& \xrightarrow{C_{35}} r_6 \cdot X_0 \cdot X_1 \cdot \overline{CCX_{0,1} \cdot CX_{0,2} \cdot X_1} \cdot X_0 \cdot CX_{0,2} \cdot X_2 \\
& \xrightarrow{B_3} r_6 \cdot X_0 \cdot X_1 \cdot CCX_{0,1} \cdot \overline{X_1 \cdot CX_{0,2} \cdot X_0} \cdot CX_{0,2} \cdot X_2 \\
& \xrightarrow{C_{65}} r_6 \cdot X_0 \cdot X_1 \cdot CCX_{0,1} \cdot X_1 \cdot CX_{0,2} \cdot \overline{X_0 \cdot X_2 \cdot CX_{0,2}} \\
& \xrightarrow{B_{13}} r_6 \cdot X_0 \cdot X_1 \cdot CCX_{0,1} \cdot X_1 \cdot \overline{CX_{0,2} \cdot X_2 \cdot X_0} \cdot CX_{0,2} \\
& \xleftarrow{C_{118}} r_6 \cdot \overline{X_0 \cdot X_1 \cdot CCX_{0,1} \cdot X_1 \cdot X_0 \cdot CX_{0,2} \cdot CX_{0,2}}
\end{aligned}$$

$$\begin{array}{c} \xleftarrow{D_1} r_6 \cdot \overline{r_1} \cdot \underline{CX_{0,2}} \cdot CX_{0,2} \\ \xrightarrow{E_{15}} r_6 \cdot r_1 \end{array}$$

$$\begin{aligned} (\xi_7) : X_1 \cdot r_8 &\xrightarrow{D_8} \underline{X_1 \cdot \overline{K_{1,2}} \cdot X_1 \cdot X_2 \cdot CZ_{0,2} \cdot CCX_{1,2} \cdot CZ_{0,2} \cdot X_2 \cdot X_1 \cdot K_{1,2}} \\ &\xrightarrow{C_2} \overline{K_{1,2} \cdot \underline{Z_1} \cdot X_1 \cdot X_2 \cdot CZ_{0,2} \cdot CCX_{1,2} \cdot CZ_{0,2} \cdot X_2 \cdot X_1 \cdot K_{1,2}} \\ &\xrightarrow{\gamma_{13}} K_{1,2} \cdot \overline{X_1 \cdot Z_1 \cdot (-I) \cdot X_2 \cdot CZ_{0,2} \cdot CCX_{1,2} \cdot CZ_{0,2} \cdot X_2 \cdot X_1 \cdot K_{1,2}} \\ &\xrightarrow{\gamma_3} K_{1,2} \cdot X_1 \cdot Z_1 \cdot \overline{X_2 \cdot (-I) \cdot CZ_{0,2} \cdot CCX_{1,2} \cdot CZ_{0,2} \cdot X_2 \cdot X_1 \cdot K_{1,2}} \\ &\xrightarrow{\gamma_{16}} K_{1,2} \cdot X_1 \cdot Z_1 \cdot X_2 \cdot \overline{CZ_{0,2} \cdot (-I) \cdot CCX_{1,2} \cdot CZ_{0,2} \cdot X_2 \cdot X_1 \cdot K_{1,2}} \\ &\xrightarrow{\gamma_{17}} K_{1,2} \cdot X_1 \cdot Z_1 \cdot X_2 \cdot CZ_{0,2} \cdot \overline{CCX_{1,2} \cdot (-I) \cdot CZ_{0,2} \cdot X_2 \cdot X_1 \cdot K_{1,2}} \\ &\xrightarrow{\gamma_{16}} K_{1,2} \cdot X_1 \cdot Z_1 \cdot X_2 \cdot CZ_{0,2} \cdot CCX_{1,2} \cdot \overline{CZ_{0,2} \cdot (-I) \cdot X_2 \cdot X_1 \cdot K_{1,2}} \\ &\xrightarrow{\gamma_3} K_{1,2} \cdot X_1 \cdot \underline{Z_1 \cdot X_2} \cdot CZ_{0,2} \cdot CCX_{1,2} \cdot CZ_{0,2} \cdot \overline{X_2 \cdot (-I) \cdot X_1 \cdot K_{1,2}} \\ &\xleftarrow{B_{24}} K_{1,2} \cdot X_1 \cdot \overline{X_2 \cdot Z_1 \cdot CZ_{0,2} \cdot CCX_{1,2} \cdot CZ_{0,2} \cdot X_2 \cdot (-I) \cdot X_1 \cdot K_{1,2}} \\ &\xleftarrow{B_{20}} K_{1,2} \cdot X_1 \cdot X_2 \cdot \overline{CZ_{0,2} \cdot Z_1 \cdot CCX_{1,2} \cdot CZ_{0,2} \cdot X_2 \cdot (-I) \cdot X_1 \cdot K_{1,2}} \\ &\xrightarrow{C_{59}} K_{1,2} \cdot X_1 \cdot X_2 \cdot CZ_{0,2} \cdot \overline{CCX_{1,2} \cdot Z_1 \cdot CZ_{0,2} \cdot X_2 \cdot (-I) \cdot X_1 \cdot K_{1,2}} \\ &\xleftarrow{B_{20}} K_{1,2} \cdot X_1 \cdot X_2 \cdot CZ_{0,2} \cdot CCX_{1,2} \cdot \overline{CZ_{0,2} \cdot Z_1 \cdot X_2 \cdot (-I) \cdot X_1 \cdot K_{1,2}} \\ &\xleftarrow{B_{24}} K_{1,2} \cdot X_1 \cdot X_2 \cdot CZ_{0,2} \cdot CCX_{1,2} \cdot CZ_{0,2} \cdot \overline{X_2 \cdot Z_1 \cdot (-I) \cdot X_1 \cdot K_{1,2}} \\ &\xleftarrow{\gamma_6} K_{1,2} \cdot X_1 \cdot X_2 \cdot CZ_{0,2} \cdot CCX_{1,2} \cdot CZ_{0,2} \cdot X_2 \cdot \overline{(-I) \cdot Z_1 \cdot X_1 \cdot K_{1,2}} \\ &\xleftarrow{\gamma_{11}} K_{1,2} \cdot X_1 \cdot X_2 \cdot CZ_{0,2} \cdot CCX_{1,2} \cdot CZ_{0,2} \cdot X_2 \cdot \overline{X_1 \cdot Z_1 \cdot K_{1,2}} \\ &\xleftarrow{C_{27}} \underline{K_{1,2} \cdot X_1 \cdot X_2 \cdot CZ_{0,2} \cdot CCX_{1,2} \cdot CZ_{0,2} \cdot X_2 \cdot X_1 \cdot \overline{K_{1,2} \cdot X_1}} \\ &\xleftarrow{D_8} \overline{r_8} \cdot X_1 \end{aligned}$$

$$\begin{aligned} (\xi_8) : CCX_{0,1} \cdot r_8 &\xrightarrow{D_8} \underline{CCX_{0,1} \cdot \overline{K_{1,2}} \cdot X_1 \cdot X_2 \cdot CZ_{0,2} \cdot CCX_{1,2} \cdot CZ_{0,2} \cdot X_2 \cdot X_1 \cdot K_{1,2}} \\ &\xrightarrow{C_{38}} \overline{K_{1,2} \cdot \underline{CCX_{0,2}} \cdot X_1 \cdot X_2 \cdot CZ_{0,2} \cdot CCX_{1,2} \cdot CZ_{0,2} \cdot X_2 \cdot X_1 \cdot K_{1,2}} \\ &\xleftarrow{C_{37}} K_{1,2} \cdot \overline{X_1 \cdot \underline{CCX_{0,2}} \cdot X_2 \cdot CZ_{0,2} \cdot CCX_{1,2} \cdot CZ_{0,2} \cdot X_2 \cdot X_1 \cdot K_{1,2}} \\ &\xleftarrow{C_{109}} K_{1,2} \cdot X_1 \cdot \overline{X_2 \cdot CX_{0,1} \cdot \underline{CCX_{0,2}} \cdot CZ_{0,2} \cdot CCX_{1,2} \cdot CZ_{0,2} \cdot X_2 \cdot X_1 \cdot K_{1,2}} \\ &\xleftarrow{C_{96}} K_{1,2} \cdot X_1 \cdot X_2 \cdot \underline{CX_{0,1} \cdot \overline{CZ_{0,2} \cdot CCX_{0,2}}} \cdot CCX_{1,2} \cdot CZ_{0,2} \cdot X_2 \cdot X_1 \cdot K_{1,2} \\ &\xrightarrow{C_{23}} K_{1,2} \cdot X_1 \cdot X_2 \cdot \overline{CZ_{0,2} \cdot CX_{0,1}} \cdot CCX_{0,2} \cdot CCX_{1,2} \cdot CZ_{0,2} \cdot X_2 \cdot X_1 \cdot K_{1,2} \\ &\xleftarrow{E_7} K_{1,2} \cdot X_1 \cdot X_2 \cdot CZ_{0,2} \cdot CX_{0,1} \cdot \underline{CCX_{0,2} \cdot CCX_{1,2} \cdot \overline{CCX_{0,2} \cdot CCX_{0,2}}} \cdot CZ_{0,2} \cdot X_2 \cdot X_1 \cdot K_{1,2} \\ &\xleftarrow{X_1} K_{1,2} \cdot X_1 \cdot X_2 \cdot CZ_{0,2} \cdot \underline{CX_{0,1} \cdot \overline{CX_{0,1} \cdot CCX_{1,2} \cdot CX_{0,1}}} \cdot CCX_{0,2} \cdot CZ_{0,2} \cdot X_2 \cdot X_1 \cdot K_{1,2} \end{aligned}$$

$$\begin{aligned}
& \xrightarrow{(22)} K_{1,2} \cdot X_1 \cdot X_2 \cdot CZ_{0,2} \cdot CCX_{1,2} \cdot CX_{0,1} \cdot \overline{CCX_{0,2} \cdot CZ_{0,2}} \cdot X_2 \cdot X_1 \cdot K_{1,2} \\
& \xleftarrow{C_{96}} K_{1,2} \cdot X_1 \cdot X_2 \cdot CZ_{0,2} \cdot CCX_{1,2} \cdot \overline{CX_{0,1} \cdot CZ_{0,2} \cdot CCX_{0,2}} \cdot X_2 \cdot X_1 \cdot K_{1,2} \\
& \xrightarrow{C_{23}} K_{1,2} \cdot X_1 \cdot X_2 \cdot CZ_{0,2} \cdot CCX_{1,2} \cdot \overline{CZ_{0,2} \cdot CX_{0,1}} \cdot \overline{CCX_{0,2} \cdot X_2 \cdot X_1} \cdot K_{1,2} \\
& \xleftarrow{C_{109}} K_{1,2} \cdot X_1 \cdot X_2 \cdot CZ_{0,2} \cdot CCX_{1,2} \cdot CZ_{0,2} \cdot CX_{0,1} \cdot \overline{X_2 \cdot CX_{0,1} \cdot CCX_{0,2}} \cdot X_1 \cdot K_{1,2} \\
& \xleftarrow{B_{16}} K_{1,2} \cdot X_1 \cdot X_2 \cdot CZ_{0,2} \cdot CCX_{1,2} \cdot CZ_{0,2} \cdot \overline{CX_{0,1} \cdot CX_{0,1} \cdot X_2} \cdot CCX_{0,2} \cdot X_1 \cdot K_{1,2} \\
& \xrightarrow{(22)} K_{1,2} \cdot X_1 \cdot X_2 \cdot CZ_{0,2} \cdot CCX_{1,2} \cdot CZ_{0,2} \cdot X_2 \cdot \overline{CCX_{0,2} \cdot X_1} \cdot K_{1,2} \\
& \xleftarrow{C_{37}} K_{1,2} \cdot X_1 \cdot X_2 \cdot CZ_{0,2} \cdot CCX_{1,2} \cdot CZ_{0,2} \cdot X_2 \cdot \overline{X_1 \cdot CCX_{0,2}} \cdot K_{1,2} \\
& \xleftarrow{C_{44}} K_{1,2} \cdot X_1 \cdot X_2 \cdot CZ_{0,2} \cdot CCX_{1,2} \cdot CZ_{0,2} \cdot X_2 \cdot X_1 \cdot \overline{K_{1,2} \cdot CCX_{0,1}} \\
& \xleftarrow{D_8} \overline{r_8} \cdot CCX_{0,1}
\end{aligned}$$

## 1.7 Elimination of the Coxeter Relations

This section derives the Coxeter relations in  $R_{E8}$ , as described in Section 4.3 of the main paper. When necessary, the  $n$ -th labelled derivation in this section is denoted  $\delta_n$ . Note that relations of the form  $(j;k)$ , which belong to  $R_{E8}$ , appear in the lemmas  $\omega_5$ ,  $\omega_7$ ,  $\omega_{10}$ ,  $\omega_{12}$ ,  $\omega_{13}$ ,  $\omega_{15}$ , and  $\omega_{20}$ . To ensure that this proof is not cyclic, each derivation has been validated in TIETZE with all primitive relations of the form  $(j;k)$  and  $W_j$  omitted.

It is important to note that all Coxeter matrices are symmetric. That is, if  $(j;k)$  denotes  $(r_j \cdot r_k)^n \approx \varepsilon$  for some  $n \in \mathbb{N}$ , then  $(k;j)$  denotes  $(r_k \cdot r_j)^n \approx \varepsilon$ . Since all Coxeter matrices contain only ones along their diagonal, then  $(j;j)$  denotes  $r_j^2 \approx \varepsilon$ . Given  $r_j^2 \approx \varepsilon$  and  $r_k^2 \approx \varepsilon$ , it is also possible to derive the relation  $(k;j)$  from  $(j;k)$ . Then it suffices to only derive the relations  $(j;k)$  for  $j, k \in \{1, 2, \dots, 8\}$  with  $j \leq k$ .

### 1.7.1 Deriving the Coxeter Relation ( 1 ; 1 )

$$\begin{aligned}
(1;1) : r_1 \cdot \underline{r_1} & \xrightarrow{D_1} \underline{r_1} \cdot \overline{X_0 \cdot X_1 \cdot CCX_{0,1} \cdot X_1 \cdot X_0} \xrightarrow{D_1} \overline{X_0 \cdot X_1 \cdot CCX_{0,1} \cdot X_1 \cdot X_0} \cdot X_0 \cdot X_1 \cdot CCX_{0,1} \cdot X_1 \cdot X_0 \\
& \xrightarrow{(21)} X_0 \cdot X_1 \cdot CCX_{0,1} \cdot \overline{X_1 \cdot X_1} \cdot CCX_{0,1} \cdot X_1 \cdot X_0 \\
& \xrightarrow{E_{13}} X_0 \cdot X_1 \cdot \overline{CCX_{0,1} \cdot CCX_{0,1}} \cdot X_1 \cdot X_0 \\
& \xrightarrow{E_{18}} X_0 \cdot \overline{X_1 \cdot X_1} \cdot X_0 \xrightarrow{E_{13}} \overline{X_0 \cdot X_0} \xrightarrow{(21)} \varepsilon
\end{aligned}$$

### 1.7.2 Deriving the Coxeter Relation ( 2 ; 2 )

$$\begin{aligned}
(2;2) : r_2 \cdot \underline{r_2} & \xrightarrow{D_2} \underline{r_2} \cdot \overline{X_0 \cdot CX_{2,1} \cdot CCX_{0,1} \cdot CX_{2,1} \cdot X_0} \xrightarrow{D_2} \overline{X_0 \cdot CX_{2,1} \cdot CCX_{0,1} \cdot CX_{2,1} \cdot X_0} \cdot X_0 \cdot CX_{2,1} \cdot CCX_{0,1} \cdot CX_{2,1} \cdot X_0 \\
& \xrightarrow{(21)} X_0 \cdot CX_{2,1} \cdot CCX_{0,1} \cdot \overline{CX_{2,1} \cdot CX_{2,1}} \cdot CCX_{0,1} \cdot CX_{2,1} \cdot X_0 \\
& \xrightarrow{E_9} X_0 \cdot CX_{2,1} \cdot \overline{CCX_{0,1} \cdot CCX_{0,1}} \cdot CX_{2,1} \cdot X_0 \\
& \xrightarrow{E_{18}} X_0 \cdot \overline{CX_{2,1} \cdot CX_{2,1}} \cdot X_0 \xrightarrow{E_9} \overline{X_0 \cdot X_0} \xrightarrow{(21)} \varepsilon
\end{aligned}$$

### 1.7.3 Deriving the Coxeter Relation ( 3 ; 3 )

$$(3;3) : r_3 \cdot \underline{r_3} \xrightarrow{D_3} \underline{r_3} \cdot \overline{X_0 \cdot CCX_{0,1} \cdot X_0} \xrightarrow{D_3} \overline{X_0 \cdot CCX_{0,1} \cdot X_0} \cdot \underline{X_0} \cdot CCX_{0,1} \cdot X_0 \xrightarrow{(21)} X_0 \cdot \underline{CCX_{0,1} \cdot CCX_{0,1}} \cdot X_0 \xrightarrow{E_{18}} \underline{X_0 \cdot X_0} \xrightarrow{(21)} \varepsilon$$

### 1.7.4 Deriving the Coxeter Relation ( 4 ; 4 )

$$(4;4) : r_4 \cdot \underline{r_4} \xrightarrow{D_4} \underline{r_4} \cdot \overline{CX_{0,1} \cdot CX_{0,2} \cdot CCX_{1,2} \cdot CX_{0,2} \cdot CX_{0,1}} \xrightarrow{D_4} \overline{CX_{0,1} \cdot CX_{0,2} \cdot CCX_{1,2} \cdot CX_{0,2} \cdot CX_{0,1}} \cdot CX_{0,1} \cdot CX_{0,2} \cdot CCX_{1,2} \cdot CX_{0,2} \cdot CX_{0,1} \\ \xrightarrow{(22)} CX_{0,1} \cdot CX_{0,2} \cdot CCX_{1,2} \cdot \underline{CX_{0,2} \cdot CX_{0,2}} \cdot CCX_{1,2} \cdot CX_{0,2} \cdot CX_{0,1} \\ \xrightarrow{E_{15}} CX_{0,1} \cdot CX_{0,2} \cdot \underline{CCX_{1,2} \cdot CCX_{1,2}} \cdot CX_{0,2} \cdot CX_{0,1} \\ \xrightarrow{(24)} CX_{0,1} \cdot \underline{CX_{0,2} \cdot CX_{0,2}} \cdot CX_{0,1} \xrightarrow{E_{15}} \underline{CX_{0,1} \cdot CX_{0,1}} \xrightarrow{(22)} \varepsilon$$

### 1.7.5 Deriving the Coxeter Relation ( 5 ; 5 )

$$(5;5) : r_5 \cdot \underline{r_5} \xrightarrow{D_6} \underline{r_5} \cdot \overline{X_1 \cdot CCX_{0,1} \cdot X_1} \xrightarrow{D_6} \overline{X_1 \cdot CCX_{0,1} \cdot X_1} \cdot X_1 \cdot CCX_{0,1} \cdot X_1 \xrightarrow{E_{13}} X_1 \cdot \underline{CCX_{0,1} \cdot CCX_{0,1}} \cdot X_1 \xrightarrow{E_{18}} \underline{X_1 \cdot X_1} \xrightarrow{E_{13}} \varepsilon$$

### 1.7.6 Deriving the Coxeter Relation ( 6 ; 6 )

$$(6;6) : r_6 \cdot \underline{r_6} \xrightarrow{D_6} \underline{r_6} \cdot \overline{CX_{2,1} \cdot CCX_{0,1} \cdot CX_{2,1}} \xrightarrow{D_6} \overline{CX_{2,1} \cdot CCX_{0,1} \cdot CX_{2,1}} \cdot CX_{2,1} \cdot CCX_{0,1} \cdot CX_{2,1} \\ \xrightarrow{E_9} CX_{2,1} \cdot \underline{CCX_{0,1} \cdot CCX_{0,1}} \cdot CX_{2,1} \xrightarrow{E_{18}} \underline{CX_{2,1} \cdot CX_{2,1}} \xrightarrow{E_9} \varepsilon$$

### 1.7.7 Deriving the Coxeter Relation ( 7 ; 7 )

$$(7;7) : r_7 \cdot \underline{r_7} \xrightarrow{D_7} \underline{r_7} \cdot \overline{CZ_{0,1} \cdot CX_{2,1} \cdot CCX_{0,1} \cdot CX_{2,1} \cdot CZ_{0,1}} \xrightarrow{D_7} \overline{CZ_{0,1} \cdot CX_{2,1} \cdot CCX_{0,1} \cdot CX_{2,1} \cdot CZ_{0,1}} \cdot CZ_{0,1} \cdot CX_{2,1} \cdot CCX_{0,1} \cdot CX_{2,1} \cdot CZ_{0,1} \\ \xrightarrow{E_2} CZ_{0,1} \cdot CX_{2,1} \cdot CCX_{0,1} \cdot \underline{CX_{2,1} \cdot CX_{2,1}} \cdot CCX_{0,1} \cdot CX_{2,1} \cdot CZ_{0,1} \\ \xrightarrow{E_9} CZ_{0,1} \cdot CX_{2,1} \cdot \underline{CCX_{0,1} \cdot CCX_{0,1}} \cdot CX_{2,1} \cdot CZ_{0,1} \\ \xrightarrow{E_{18}} CZ_{0,1} \cdot \underline{CX_{2,1} \cdot CX_{2,1}} \cdot CZ_{0,1} \xrightarrow{E_9} \underline{CZ_{0,1} \cdot CZ_{0,1}} \xrightarrow{E_2} \varepsilon$$

### 1.7.8 Deriving the Coxeter Relation ( 8 ; 8 )

$$(8,8) : r_8 \cdot \underline{r_8} \xrightarrow{D_8} \underline{r_8} \cdot \overline{K_{1,2} \cdot X_1 \cdot X_2 \cdot CZ_{0,2} \cdot CCX_{1,2} \cdot CZ_{0,2} \cdot X_2 \cdot X_1 \cdot K_{1,2}} \\ \xrightarrow{D_8} \overline{K_{1,2} \cdot X_1 \cdot X_2 \cdot CZ_{0,2} \cdot CCX_{1,2} \cdot CZ_{0,2} \cdot X_2 \cdot X_1 \cdot K_{1,2}} \cdot K_{1,2} \cdot X_1 \cdot X_2 \cdot CZ_{0,2} \cdot CCX_{1,2} \cdot CZ_{0,2} \cdot X_2 \cdot X_1 \cdot K_{1,2} \\ \xrightarrow{(23)} K_{1,2} \cdot X_1 \cdot X_2 \cdot CZ_{0,2} \cdot CCX_{1,2} \cdot CZ_{0,2} \cdot X_2 \cdot \underline{X_1 \cdot X_1} \cdot X_2 \cdot CZ_{0,2} \cdot CCX_{1,2} \cdot CZ_{0,2} \cdot X_2 \cdot X_1 \cdot K_{1,2} \\ \xrightarrow{E_{13}} K_{1,2} \cdot X_1 \cdot X_2 \cdot CZ_{0,2} \cdot CCX_{1,2} \cdot CZ_{0,2} \cdot \underline{X_2 \cdot X_2} \cdot CZ_{0,2} \cdot CCX_{1,2} \cdot CZ_{0,2} \cdot X_2 \cdot X_1 \cdot K_{1,2} \\ \xrightarrow{E_{17}} K_{1,2} \cdot X_1 \cdot X_2 \cdot CZ_{0,2} \cdot CCX_{1,2} \cdot \underline{CZ_{0,2} \cdot CZ_{0,2}} \cdot CCX_{1,2} \cdot CZ_{0,2} \cdot X_2 \cdot X_1 \cdot K_{1,2} \\ \xrightarrow{E_{11}} K_{1,2} \cdot X_1 \cdot X_2 \cdot CZ_{0,2} \cdot \underline{CCX_{1,2} \cdot CCX_{1,2}} \cdot CZ_{0,2} \cdot X_2 \cdot X_1 \cdot K_{1,2} \\ \xrightarrow{(24)} K_{1,2} \cdot X_1 \cdot X_2 \cdot \underline{CZ_{0,2} \cdot CZ_{0,2}} \cdot X_2 \cdot X_1 \cdot K_{1,2} \\ \xrightarrow{E_{11}} K_{1,2} \cdot X_1 \cdot \underline{X_2 \cdot X_2} \cdot X_1 \cdot K_{1,2}$$

$$\begin{aligned}
& \xrightarrow{E_{17}} K_{1,2} \cdot \underline{X_1 \cdot X_1} \cdot K_{1,2} \\
& \xrightarrow{E_{13}} \underline{K_{1,2} \cdot K_{1,2}} \\
& \xrightarrow{(23)} \varepsilon
\end{aligned}$$

### 1.7.9 Deriving the Coxeter Relation ( 1 ; 2 )

$$\begin{aligned}
(1;2) : r_1 \cdot r_2 \cdot r_1 \cdot r_2 \cdot \underline{r_1 \cdot r_2} & \xrightarrow{\theta_{14}} r_1 \cdot r_2 \cdot r_1 \cdot r_2 \cdot \overline{X_0 \cdot CX_{0,2} \cdot CCX_{0,2} \cdot CCX_{0,1} \cdot X_0} \\
& \xrightarrow{\theta_{14}} r_1 \cdot r_2 \cdot \overline{X_0 \cdot CX_{0,2} \cdot CCX_{0,2} \cdot CCX_{0,1} \cdot X_0} \cdot X_0 \cdot CX_{0,2} \cdot CCX_{0,2} \cdot CCX_{0,1} \cdot X_0 \\
& \xrightarrow{(21)} r_1 \cdot r_2 \cdot X_0 \cdot CX_{0,2} \cdot CCX_{0,2} \cdot \underline{CCX_{0,1} \cdot CX_{0,2}} \cdot CCX_{0,2} \cdot CCX_{0,1} \cdot X_0 \\
& \xrightarrow{C_{105}} r_1 \cdot r_2 \cdot X_0 \cdot \underline{CX_{0,2} \cdot CCX_{0,2}} \cdot \overline{CX_{0,2} \cdot CCX_{0,1}} \cdot CCX_{0,2} \cdot CCX_{0,1} \cdot X_0 \\
& \xrightarrow{C_{34}} r_1 \cdot r_2 \cdot X_0 \cdot \overline{CCX_{0,2} \cdot CX_{0,1}} \cdot \underline{CX_{0,2} \cdot CX_{0,2}} \cdot CCX_{0,1} \cdot CCX_{0,2} \cdot CCX_{0,1} \cdot X_0 \\
& \xrightarrow{E_{15}} r_1 \cdot r_2 \cdot X_0 \cdot \underline{CCX_{0,2} \cdot CX_{0,1}} \cdot CCX_{0,1} \cdot CCX_{0,2} \cdot CCX_{0,1} \cdot X_0 \\
& \xrightarrow{C_{89}} r_1 \cdot r_2 \cdot X_0 \cdot \overline{CX_{0,1} \cdot CCX_{0,2}} \cdot CCX_{0,1} \cdot \underline{CCX_{0,2} \cdot CCX_{0,1}} \cdot X_0 \\
& \xrightarrow{X_9} r_1 \cdot r_2 \cdot X_0 \cdot CX_{0,1} \cdot \overline{CCX_{0,1} \cdot CCX_{0,2} \cdot CCX_{0,1}} \cdot \underline{CCX_{0,1} \cdot X_0} \\
& \xrightarrow{E_{18}} r_1 \cdot r_2 \cdot X_0 \cdot CX_{0,1} \cdot CCX_{0,1} \cdot CCX_{0,2} \cdot X_0 \\
& \xrightarrow{\theta_{14}} \overline{X_0 \cdot CX_{0,2} \cdot CCX_{0,2} \cdot CCX_{0,1} \cdot X_0} \cdot X_0 \cdot CX_{0,1} \cdot CCX_{0,1} \cdot CCX_{0,2} \cdot X_0 \\
& \xrightarrow{(21)} X_0 \cdot CX_{0,2} \cdot CCX_{0,2} \cdot \underline{CCX_{0,1} \cdot CX_{0,1}} \cdot CCX_{0,1} \cdot CCX_{0,2} \cdot X_0 \\
& \xrightarrow{C_{122}} X_0 \cdot CX_{0,2} \cdot CCX_{0,2} \cdot \overline{CX_{0,1} \cdot CX_{0,2}} \cdot \underline{CCX_{0,1} \cdot CCX_{0,1}} \cdot CCX_{0,2} \cdot X_0 \\
& \xrightarrow{E_{18}} X_0 \cdot CX_{0,2} \cdot \underline{CCX_{0,2} \cdot CX_{0,1} \cdot CX_{0,2}} \cdot CCX_{0,2} \cdot X_0 \\
& \xleftarrow{C_{34}} X_0 \cdot CX_{0,2} \cdot \overline{CX_{0,2} \cdot CCX_{0,2} \cdot CCX_{0,2}} \cdot X_0 \xrightarrow{E_7} X_0 \cdot \underline{CX_{0,2} \cdot CX_{0,2}} \cdot X_0 \xrightarrow{E_{15}} \underline{X_0 \cdot X_0} \xrightarrow{(21)} \varepsilon
\end{aligned}$$

### 1.7.10 Deriving the Coxeter Relation ( 1 ; 3 )

$$\begin{aligned}
(\delta_1) : \underline{r_1} & \xrightarrow{D_1} \overline{X_0 \cdot X_1 \cdot CCX_{0,1} \cdot X_1 \cdot X_0} \xrightarrow{B_2} \overline{X_1 \cdot X_0 \cdot CCX_{0,1} \cdot X_1 \cdot X_0} \xleftarrow{B_2} X_1 \cdot X_0 \cdot \underline{CCX_{0,1} \cdot X_0} \cdot X_1 \cdot X_0 \xleftarrow{D_3} X_1 \cdot \overline{X_0 \cdot X_1} \cdot X_1 \\
(\delta_2) : X_1 \cdot r_3 & \xrightarrow{D_3} \underline{X_1 \cdot X_0} \cdot \overline{CCX_{0,1} \cdot X_0} \xleftarrow{B_2} \overline{X_0 \cdot X_1 \cdot CCX_{0,1} \cdot X_0} \xrightarrow{C_{35}} X_0 \cdot \overline{CCX_{0,1} \cdot CX_{0,2} \cdot X_1 \cdot X_0} \xleftarrow{B_2} X_0 \cdot CCX_{0,1} \cdot \underline{CX_{0,2} \cdot X_0} \cdot X_1 \\
& \xleftarrow{C_{120}} \underline{X_0 \cdot CCX_{0,1} \cdot X_0 \cdot X_2 \cdot CX_{0,2} \cdot X_1} \\
& \xleftarrow{D_3} \overline{r_3} \cdot X_2 \cdot CX_{0,2} \cdot X_1 \\
r_1 \cdot r_3 \cdot \underline{r_1} \cdot r_3 & \xrightarrow{\delta_1} \underline{r_1} \cdot r_3 \cdot \overline{X_1 \cdot r_3 \cdot X_1} \cdot r_3 \xrightarrow{\delta_1} \overline{X_1 \cdot r_3 \cdot X_1} \cdot r_3 \cdot X_1 \cdot r_3 \cdot \underline{X_1 \cdot r_3} \xrightarrow{\delta_2} X_1 \cdot r_3 \cdot X_1 \cdot r_3 \cdot X_1 \cdot \underline{r_3 \cdot X_2 \cdot CX_{0,2} \cdot X_1} \\
& \xrightarrow{(3;3)} X_1 \cdot r_3 \cdot \underline{X_1 \cdot r_3} \cdot X_1 \cdot X_2 \cdot CX_{0,2} \cdot X_1 \\
& \xrightarrow{\delta_2} X_1 \cdot \underline{r_3 \cdot r_3} \cdot X_2 \cdot \overline{CX_{0,2} \cdot X_1} \cdot X_1 \cdot X_2 \cdot CX_{0,2} \cdot X_1 \\
& \xrightarrow{(3;3)} X_1 \cdot \underline{X_2 \cdot CX_{0,2}} \cdot X_1 \cdot X_1 \cdot X_2 \cdot CX_{0,2} \cdot X_1
\end{aligned}$$

$$\begin{aligned}
& \xleftarrow{C_{65}} X_1 \cdot \overline{CX_{0,2} \cdot X_2} \cdot X_1 \cdot X_1 \cdot X_2 \cdot CX_{0,2} \cdot X_1 \\
& \xrightarrow{E_{13}} X_1 \cdot CX_{0,2} \cdot \overline{X_2 \cdot X_2} \cdot CX_{0,2} \cdot X_1 \\
& \xrightarrow{E_{17}} X_1 \cdot \overline{CX_{0,2} \cdot CX_{0,2}} \cdot X_1 \\
& \xrightarrow{E_{15}} \overline{X_1 \cdot X_1} \\
& \xrightarrow{E_{13}} \varepsilon
\end{aligned}$$

### 1.7.11 Deriving the Coxeter Relation ( 1 ; 4 )

$$\begin{aligned}
(\delta_3) : \underline{CX_{1,2}} & \xrightarrow{S_8} \overline{\sigma_{1,2} \cdot CX_{2,1} \cdot \sigma_{1,2}} \xrightarrow{(6)} \sigma_{1,2} \cdot \overline{CX_{2,0} \cdot CX_{0,1} \cdot CX_{2,0} \cdot CX_{0,1}} \cdot \sigma_{1,2} \xrightarrow{S_{14}} \sigma_{1,2} \cdot CX_{2,0} \cdot CX_{0,1} \cdot \overline{\sigma_{1,2} \cdot CX_{1,0} \cdot \sigma_{1,2} \cdot CX_{0,1} \cdot \sigma_{1,2}} \\
& \xleftarrow{(9)} \sigma_{1,2} \cdot \overline{CX_{2,0} \cdot CX_{0,1} \cdot \sigma_{1,2} \cdot CX_{1,0} \cdot \overline{CX_{0,2}}} \\
& \xrightarrow{S_{14}} \overline{\sigma_{1,2} \cdot \sigma_{1,2} \cdot CX_{1,0} \cdot \sigma_{1,2} \cdot CX_{0,1} \cdot \sigma_{1,2} \cdot CX_{1,0} \cdot CX_{0,2}} \\
& \xrightarrow{E_{10}} CX_{1,0} \cdot \overline{\sigma_{1,2} \cdot CX_{0,1} \cdot \sigma_{1,2}} \cdot CX_{1,0} \cdot CX_{0,2} \\
& \xleftarrow{(9)} CX_{1,0} \cdot \overline{CX_{0,2}} \cdot CX_{1,0} \cdot CX_{0,2}
\end{aligned}$$

$$\begin{aligned}
(\delta_4) : r_1 \cdot \underline{r_4} & \xrightarrow{D_4} \overline{r_1 \cdot CX_{0,1} \cdot CX_{0,2} \cdot CCX_{1,2} \cdot CX_{0,2} \cdot CX_{0,1}} \\
& \xrightarrow{D_1} \overline{X_0 \cdot X_1 \cdot CCX_{0,1} \cdot X_1 \cdot X_0} \cdot CX_{0,1} \cdot CX_{0,2} \cdot CCX_{1,2} \cdot CX_{0,2} \cdot CX_{0,1} \\
& \xleftarrow{B_2} X_0 \cdot X_1 \cdot CCX_{0,1} \cdot \overline{X_0 \cdot X_1} \cdot CX_{0,1} \cdot CX_{0,2} \cdot CCX_{1,2} \cdot CX_{0,2} \cdot CX_{0,1} \\
& \xrightarrow{C_{79}} X_0 \cdot X_1 \cdot CCX_{0,1} \cdot \overline{CX_{0,1} \cdot X_0 \cdot CX_{0,2}} \cdot CCX_{1,2} \cdot CX_{0,2} \cdot CX_{0,1} \\
& \xrightarrow{C_{118}} X_0 \cdot X_1 \cdot CCX_{0,1} \cdot CX_{0,1} \cdot \overline{CX_{0,2} \cdot X_2 \cdot X_0} \cdot CCX_{1,2} \cdot CX_{0,2} \cdot CX_{0,1} \\
& \xleftarrow{B_{13}} X_0 \cdot X_1 \cdot CCX_{0,1} \cdot CX_{0,1} \cdot CX_{0,2} \cdot \overline{X_0 \cdot X_2} \cdot CCX_{1,2} \cdot CX_{0,2} \cdot CX_{0,1} \\
& \xrightarrow{C_{83}} X_0 \cdot X_1 \cdot CCX_{0,1} \cdot CX_{0,1} \cdot CX_{0,2} \cdot \overline{X_0 \cdot CCX_{1,2} \cdot CX_{1,0} \cdot X_2} \cdot CX_{0,2} \cdot CX_{0,1} \\
& \xrightarrow{(37)} X_0 \cdot X_1 \cdot CCX_{0,1} \cdot CX_{0,1} \cdot CX_{0,2} \cdot \overline{CCX_{1,2} \cdot X_0 \cdot CX_{1,0} \cdot X_2} \cdot CX_{0,2} \cdot CX_{0,1} \\
& \xrightarrow{(38)} X_0 \cdot X_1 \cdot CCX_{0,1} \cdot CX_{0,1} \cdot CX_{0,2} \cdot CCX_{1,2} \cdot \overline{CX_{1,0} \cdot X_0 \cdot X_2 \cdot CX_{0,2}} \cdot CX_{0,1} \\
& \xrightarrow{C_{120}} X_0 \cdot X_1 \cdot CCX_{0,1} \cdot CX_{0,1} \cdot CX_{0,2} \cdot CCX_{1,2} \cdot CX_{1,0} \cdot \overline{CX_{0,2} \cdot X_0} \cdot CX_{0,1} \\
& \xrightarrow{C_3} X_0 \cdot X_1 \cdot \overline{CCX_{0,1} \cdot CX_{0,1}} \cdot CX_{0,2} \cdot CCX_{1,2} \cdot CX_{1,0} \cdot CX_{0,2} \cdot \overline{CX_{0,1} \cdot X_1 \cdot X_0} \\
& \xrightarrow{C_{122}} X_0 \cdot X_1 \cdot \overline{CX_{0,1} \cdot CX_{0,2} \cdot CCX_{0,1}} \cdot CX_{0,2} \cdot CCX_{1,2} \cdot CX_{1,0} \cdot CX_{0,2} \cdot CX_{0,1} \cdot X_1 \cdot X_0 \\
& \xleftarrow{E_{15}} X_0 \cdot X_1 \cdot CX_{0,1} \cdot CX_{0,2} \cdot CCX_{0,1} \cdot \overline{CX_{0,2} \cdot CCX_{1,2} \cdot CX_{0,2}} \cdot CX_{1,0} \cdot CX_{0,2} \cdot CX_{0,1} \cdot X_1 \cdot X_0 \\
& \xrightarrow{X_4} X_0 \cdot X_1 \cdot CX_{0,1} \cdot CX_{0,2} \cdot \overline{CCX_{0,1} \cdot CCX_{1,2} \cdot CCX_{0,1}} \cdot CX_{0,2} \cdot CX_{1,0} \cdot CX_{0,2} \cdot CX_{0,1} \cdot X_1 \cdot X_0 \\
& \xrightarrow{E_{18}} X_0 \cdot X_1 \cdot CX_{0,1} \cdot CX_{0,2} \cdot CCX_{1,2} \cdot \overline{CCX_{0,1} \cdot CX_{0,2}} \cdot CX_{1,0} \cdot CX_{0,2} \cdot CX_{0,1} \cdot X_1 \cdot X_0 \\
& \xrightarrow{C_{105}} X_0 \cdot X_1 \cdot \overline{CX_{0,1}} \cdot CX_{0,2} \cdot CCX_{1,2} \cdot \overline{CX_{0,2} \cdot CCX_{0,1}} \cdot CX_{1,0} \cdot CX_{0,2} \cdot CX_{0,1} \cdot X_1 \cdot X_0 \\
& \xrightarrow{C_{79}} \overline{CX_{0,1} \cdot X_0 \cdot CX_{0,2}} \cdot CCX_{1,2} \cdot CX_{0,2} \cdot CCX_{0,1} \cdot CX_{1,0} \cdot CX_{0,2} \cdot CX_{0,1} \cdot X_1 \cdot X_0 \\
& \xrightarrow{C_{118}} CX_{0,1} \cdot \overline{CX_{0,2} \cdot X_2 \cdot X_0} \cdot CCX_{1,2} \cdot CX_{0,2} \cdot CCX_{0,1} \cdot CX_{1,0} \cdot CX_{0,2} \cdot CX_{0,1} \cdot X_1 \cdot X_0
\end{aligned}$$

$$\begin{aligned}
& \xleftarrow{B_{13}} CX_{0,1} \cdot CX_{0,2} \cdot \overline{X_0} \cdot \overline{X_2} \cdot \overline{CCX_{1,2}} \cdot CX_{0,2} \cdot CCX_{0,1} \cdot CX_{1,0} \cdot CX_{0,2} \cdot CX_{0,1} \cdot X_1 \cdot X_0 \\
& \xrightarrow{C_{83}} CX_{0,1} \cdot CX_{0,2} \cdot X_0 \cdot \overline{CCX_{1,2}} \cdot \overline{CX_{1,0}} \cdot \overline{X_2} \cdot CX_{0,2} \cdot CCX_{0,1} \cdot CX_{1,0} \cdot CX_{0,2} \cdot CX_{0,1} \cdot X_1 \cdot X_0 \\
& \xleftarrow{E_1} CX_{0,1} \cdot CX_{0,2} \cdot X_0 \cdot CCX_{1,2} \cdot CX_{1,0} \cdot X_2 \cdot CX_{0,2} \cdot \overline{CX_{1,0}} \cdot \overline{CX_{1,0}} \cdot \overline{CCX_{0,1}} \cdot CX_{1,0} \cdot CX_{0,2} \cdot CX_{0,1} \cdot X_1 \cdot X_0 \\
& \xrightarrow{X_2} CX_{0,1} \cdot CX_{0,2} \cdot X_0 \cdot \overline{CCX_{1,2}} \cdot CX_{1,0} \cdot X_2 \cdot CX_{0,2} \cdot CX_{1,0} \cdot \overline{X_0} \cdot \overline{CCX_{0,1}} \cdot \overline{X_0} \cdot CX_{0,2} \cdot CX_{0,1} \cdot X_1 \cdot X_0 \\
& \xrightarrow{(37)} CX_{0,1} \cdot CX_{0,2} \cdot \overline{CCX_{1,2}} \cdot \overline{X_0} \cdot \overline{CX_{1,0}} \cdot X_2 \cdot CX_{0,2} \cdot CX_{1,0} \cdot X_0 \cdot CCX_{0,1} \cdot X_0 \cdot CX_{0,2} \cdot CX_{0,1} \cdot X_1 \cdot X_0 \\
& \xrightarrow{(38)} CX_{0,1} \cdot CX_{0,2} \cdot CCX_{1,2} \cdot \overline{CX_{1,0}} \cdot \overline{X_0} \cdot \overline{X_2} \cdot \overline{CX_{0,2}} \cdot CX_{1,0} \cdot X_0 \cdot CCX_{0,1} \cdot X_0 \cdot CX_{0,2} \cdot CX_{0,1} \cdot X_1 \cdot X_0 \\
& \xrightarrow{C_{120}} CX_{0,1} \cdot CX_{0,2} \cdot CCX_{1,2} \cdot CX_{1,0} \cdot \overline{CX_{0,2}} \cdot \overline{X_0} \cdot \overline{CX_{1,0}} \cdot X_0 \cdot CCX_{0,1} \cdot X_0 \cdot CX_{0,2} \cdot CX_{0,1} \cdot X_1 \cdot X_0 \\
& \xrightarrow{(38)} CX_{0,1} \cdot CX_{0,2} \cdot CCX_{1,2} \cdot CX_{1,0} \cdot CX_{0,2} \cdot \overline{CX_{1,0}} \cdot \overline{X_0} \cdot \overline{X_0} \cdot CCX_{0,1} \cdot X_0 \cdot CX_{0,2} \cdot CX_{0,1} \cdot X_1 \cdot X_0 \\
& \xrightarrow{(21)} CX_{0,1} \cdot CX_{0,2} \cdot CCX_{1,2} \cdot CX_{1,0} \cdot CX_{0,2} \cdot CX_{1,0} \cdot CCX_{0,1} \cdot X_0 \cdot CX_{0,2} \cdot CX_{0,1} \cdot X_1 \cdot X_0 \\
& \xleftarrow{E_{15}} CX_{0,1} \cdot CX_{0,2} \cdot CCX_{1,2} \cdot \overline{CX_{1,0}} \cdot \overline{CX_{0,2}} \cdot \overline{CX_{1,0}} \cdot \overline{CX_{0,2}} \cdot CCX_{0,1} \cdot X_0 \cdot CX_{0,2} \cdot CX_{0,1} \cdot X_1 \cdot X_0 \\
& \xleftarrow{\delta_3} CX_{0,1} \cdot CX_{0,2} \cdot CCX_{1,2} \cdot \overline{CX_{1,2}} \cdot \overline{CX_{0,2}} \cdot CCX_{0,1} \cdot X_0 \cdot CX_{0,2} \cdot CX_{0,1} \cdot X_1 \cdot X_0 \\
& \xrightarrow{C_{33}} CX_{0,1} \cdot CX_{0,2} \cdot CCX_{1,2} \cdot \overline{CX_{0,2}} \cdot \overline{CX_{1,2}} \cdot CCX_{0,1} \cdot X_0 \cdot CX_{0,2} \cdot CX_{0,1} \cdot X_1 \cdot X_0 \\
& \xleftarrow{(22)} CX_{0,1} \cdot CX_{0,2} \cdot CCX_{1,2} \cdot \overline{CX_{0,2}} \cdot \overline{CX_{0,1}} \cdot \overline{CX_{1,2}} \cdot CCX_{0,1} \cdot X_0 \cdot CX_{0,2} \cdot CX_{0,1} \cdot X_1 \cdot X_0 \\
& \xleftarrow{D_4} \overline{r_4} \cdot CX_{0,1} \cdot CX_{1,2} \cdot \overline{CCX_{0,1}} \cdot \overline{X_0} \cdot CX_{0,2} \cdot CX_{0,1} \cdot X_1 \cdot X_0 \\
& \xleftarrow{C_{56}} r_4 \cdot CX_{0,1} \cdot \overline{CX_{1,2}} \cdot \overline{X_0} \cdot \overline{CX_{1,2}} \cdot \overline{CCX_{0,1}} \cdot CX_{0,2} \cdot CX_{0,1} \cdot X_1 \cdot X_0 \\
& \xrightarrow{(26)} r_4 \cdot CX_{0,1} \cdot \overline{X_0} \cdot \overline{CX_{1,2}} \cdot \overline{CX_{1,2}} \cdot CCX_{0,1} \cdot CX_{0,2} \cdot CX_{0,1} \cdot X_1 \cdot X_0 \\
& \xrightarrow{E_8} r_4 \cdot CX_{0,1} \cdot X_0 \cdot \overline{CCX_{0,1}} \cdot \overline{CX_{0,2}} \cdot \overline{CX_{0,1}} \cdot X_1 \cdot X_0 \xleftarrow{C_{119}} r_4 \cdot CX_{0,1} \cdot \overline{X_0} \cdot \overline{CX_{0,1}} \cdot \overline{CCX_{0,1}} \cdot X_1 \cdot X_0 \\
& \xrightarrow{C_3} r_4 \cdot \overline{CX_{0,1}} \cdot \overline{CX_{0,1}} \cdot \overline{X_1} \cdot \overline{X_0} \cdot CCX_{0,1} \cdot X_1 \cdot X_0 \xrightarrow{(22)} r_4 \cdot \overline{X_1} \cdot \overline{X_0} \cdot CCX_{0,1} \cdot X_1 \cdot X_0 \xleftarrow{B_2} r_4 \cdot \overline{X_0} \cdot \overline{X_1} \cdot \overline{CCX_{0,1}} \cdot X_1 \cdot X_0 \xleftarrow{D_1} r_4 \cdot \overline{r_1}
\end{aligned}$$

$$\begin{aligned}
& \xrightarrow{\delta_4} \overline{r_4} \cdot \overline{r_1} \cdot r_1 \cdot r_4 \xrightarrow{(1;1)} \overline{r_4} \cdot r_4 \xrightarrow{(4;4)} \varepsilon
\end{aligned}$$

### 1.7.12 Deriving the Coxeter Relation ( 1 ; 5 )

$$\begin{aligned}
(\delta_5) : r_1 \cdot r_5 & \xrightarrow{D_6} \overline{r_1} \cdot \overline{X_1} \cdot \overline{CCX_{0,1}} \cdot \overline{X_1} \xrightarrow{D_1} \overline{X_0} \cdot \overline{X_1} \cdot \overline{CCX_{0,1}} \cdot \overline{X_1} \cdot \overline{X_0} \cdot X_1 \cdot CCX_{0,1} \cdot X_1 \xrightarrow{B_2} \overline{X_1} \cdot \overline{X_0} \cdot \overline{CCX_{0,1}} \cdot \overline{X_1} \cdot \overline{X_0} \cdot X_1 \cdot CCX_{0,1} \cdot X_1 \\
& \xleftarrow{B_2} X_1 \cdot X_0 \cdot \overline{CCX_{0,1}} \cdot \overline{X_0} \cdot \overline{X_1} \cdot X_1 \cdot CCX_{0,1} \cdot X_1 \\
& \xleftarrow{X_2} X_1 \cdot \overline{CX_{1,0}} \cdot \overline{CCX_{0,1}} \cdot \overline{CX_{1,0}} \cdot X_1 \cdot X_1 \cdot CCX_{0,1} \cdot X_1 \\
& \xrightarrow{C_{72}} X_1 \cdot \overline{CCX_{0,1}} \cdot \overline{CX_{1,2}} \cdot \overline{CX_{1,0}} \cdot CX_{1,0} \cdot X_1 \cdot X_1 \cdot CCX_{0,1} \cdot X_1 \\
& \xrightarrow{E_1} X_1 \cdot CCX_{0,1} \cdot \overline{CX_{1,2}} \cdot X_1 \cdot X_1 \cdot CCX_{0,1} \cdot X_1 \\
& \xrightarrow{C_{15}} X_1 \cdot \overline{CCX_{0,1}} \cdot \overline{X_1} \cdot \overline{X_2} \cdot \overline{CX_{1,2}} \cdot X_1 \cdot CCX_{0,1} \cdot X_1 \\
& \xleftarrow{D_6} \overline{r_5} \cdot X_2 \cdot \overline{CX_{1,2}} \cdot X_1 \cdot CCX_{0,1} \cdot X_1 \\
& \xrightarrow{C_{15}} r_5 \cdot X_2 \cdot \overline{X_1} \cdot \overline{X_2} \cdot \overline{CX_{1,2}} \cdot CCX_{0,1} \cdot X_1
\end{aligned}$$

$$\begin{aligned}
& \xrightarrow{B_{19}} r_5 \cdot \underline{X_2 \cdot \overline{X_2 \cdot X_1}} \cdot CX_{1,2} \cdot CCX_{0,1} \cdot X_1 \\
& \xrightarrow{E_{17}} r_5 \cdot X_1 \cdot CX_{1,2} \cdot CCX_{0,1} \cdot X_1 \\
& \xleftarrow{(21)} r_5 \cdot X_1 \cdot \overline{X_0 \cdot \overline{X_0}} \cdot CX_{1,2} \cdot CCX_{0,1} \cdot X_1 \\
& \xrightarrow{C_{56}} r_5 \cdot X_1 \cdot X_0 \cdot \overline{CCX_{0,1} \cdot \overline{X_0 \cdot X_1}} \xrightarrow{B_2} r_5 \cdot \underline{X_1 \cdot X_0} \cdot CCX_{0,1} \cdot \overline{X_1 \cdot X_0} \\
& \xleftarrow{B_2} r_5 \cdot \overline{X_0 \cdot X_1} \cdot CCX_{0,1} \cdot X_1 \cdot X_0 \xleftarrow{D_1} r_5 \cdot \overline{r_1}
\end{aligned}$$

$$(1;5) : \underline{r_1 \cdot r_5} \cdot r_1 \cdot r_5 \xrightarrow{\delta_5} \overline{r_5 \cdot \underline{r_1}} \cdot r_1 \cdot r_5 \xrightarrow{(1;1)} \underline{r_5 \cdot r_5} \xrightarrow{(5;5)} \varepsilon$$

### 1.7.13 Deriving the Coxeter Relation ( 1 ; 6 )

$$(1;6) : \underline{r_1 \cdot r_6} \cdot r_1 \cdot r_6 \xrightarrow{\xi_6} \overline{r_6 \cdot \underline{r_1}} \cdot r_1 \cdot r_6 \xrightarrow{(1;1)} \underline{r_6 \cdot r_6} \xrightarrow{(6;6)} \varepsilon$$

### 1.7.14 Deriving the Coxeter Relation ( 1 ; 7 )

$$\begin{aligned}
(\delta_6) : CZ_{0,1} \cdot \underline{r_1} & \xrightarrow{D_1} \underline{CZ_{0,1} \cdot \overline{X_0 \cdot X_1 \cdot CCX_{0,1} \cdot X_1 \cdot X_0}} \xleftarrow{C_{69}} \overline{X_0 \cdot Z_1 \cdot \underline{CZ_{0,1} \cdot X_1 \cdot CCX_{0,1} \cdot X_1 \cdot X_0}} \\
& \xleftarrow{C_{112}} X_0 \cdot Z_1 \cdot \overline{X_1 \cdot Z_0 \cdot \underline{CZ_{0,1} \cdot CCX_{0,1} \cdot X_1 \cdot X_0}} \\
& \xrightarrow{C_{95}} X_0 \cdot Z_1 \cdot X_1 \cdot Z_0 \cdot \overline{CCX_{0,1} \cdot \underline{CZ_{0,1} \cdot X_1 \cdot X_0}} \\
& \xleftarrow{C_{112}} X_0 \cdot Z_1 \cdot X_1 \cdot Z_0 \cdot CCX_{0,1} \cdot \overline{X_1 \cdot Z_0 \cdot \underline{CZ_{0,1} \cdot X_0}} \\
& \xleftarrow{C_{69}} X_0 \cdot Z_1 \cdot X_1 \cdot Z_0 \cdot CCX_{0,1} \cdot \underline{X_1 \cdot Z_0 \cdot \overline{X_0 \cdot Z_1 \cdot CZ_{0,1}}} \\
& \xrightarrow{B_{15}} X_0 \cdot Z_1 \cdot X_1 \cdot \underline{Z_0 \cdot CCX_{0,1}} \cdot \overline{Z_0 \cdot X_1 \cdot X_0 \cdot Z_1 \cdot CZ_{0,1}} \\
& \xrightarrow{C_{54}} X_0 \cdot Z_1 \cdot X_1 \cdot \overline{CCX_{0,1} \cdot \underline{Z_0 \cdot Z_0 \cdot X_1 \cdot X_0 \cdot Z_1 \cdot CZ_{0,1}}} \\
& \xrightarrow{E_3} X_0 \cdot \underline{Z_1 \cdot X_1} \cdot CCX_{0,1} \cdot X_1 \cdot X_0 \cdot Z_1 \cdot CZ_{0,1} \\
& \xrightarrow{\gamma_{13}} X_0 \cdot \overline{X_1 \cdot Z_1 \cdot (-I)} \cdot \underline{CCX_{0,1} \cdot X_1 \cdot X_0 \cdot Z_1 \cdot CZ_{0,1}} \\
& \xrightarrow{\gamma_{18}} X_0 \cdot X_1 \cdot Z_1 \cdot \overline{CCX_{0,1} \cdot (-I)} \cdot X_1 \cdot \underline{X_0 \cdot Z_1 \cdot CZ_{0,1}} \\
& \xrightarrow{B_{14}} X_0 \cdot X_1 \cdot Z_1 \cdot CCX_{0,1} \cdot (-I) \cdot \underline{X_1 \cdot \overline{Z_1 \cdot X_0}} \cdot CZ_{0,1} \\
& \xrightarrow{\gamma_{11}} X_0 \cdot X_1 \cdot Z_1 \cdot CCX_{0,1} \cdot (-I) \cdot \overline{(-I) \cdot Z_1 \cdot X_1 \cdot X_0 \cdot CZ_{0,1}} \\
& \xrightarrow{\gamma_{12}} X_0 \cdot X_1 \cdot \underline{Z_1 \cdot CCX_{0,1}} \cdot Z_1 \cdot X_1 \cdot X_0 \cdot CZ_{0,1} \\
& \xrightarrow{C_{47}} X_0 \cdot X_1 \cdot \overline{CCX_{0,1} \cdot \underline{Z_1 \cdot Z_1 \cdot X_1 \cdot X_0 \cdot CZ_{0,1}}} \\
& \xrightarrow{E_5} \underline{X_0 \cdot X_1 \cdot CCX_{0,1} \cdot X_1 \cdot X_0 \cdot CZ_{0,1}} \xleftarrow{D_1} \overline{r_1} \cdot CZ_{0,1} \\
(\delta_7) : CZ_{0,2} \cdot \underline{r_1} & \xrightarrow{D_1} \underline{CZ_{0,2} \cdot \overline{X_0 \cdot X_1 \cdot CCX_{0,1} \cdot X_1 \cdot X_0}} \xleftarrow{C_{117}} \overline{X_0 \cdot Z_2 \cdot \underline{CZ_{0,2} \cdot X_1 \cdot CCX_{0,1} \cdot X_1 \cdot X_0}} \\
& \xleftarrow{B_{35}} X_0 \cdot Z_2 \cdot \overline{X_1 \cdot \underline{CZ_{0,2} \cdot CCX_{0,1} \cdot X_1 \cdot X_0}}
\end{aligned}$$

$$\begin{aligned}
& \xrightarrow{C_{81}} X_0 \cdot Z_2 \cdot X_1 \cdot \overline{CCX_{0,1} \cdot CZ_{0,1} \cdot CZ_{0,2}} \cdot X_1 \cdot X_0 \\
& \xleftarrow{B_{35}} X_0 \cdot Z_2 \cdot X_1 \cdot CCX_{0,1} \cdot CZ_{0,1} \cdot \overline{X_1 \cdot CZ_{0,2}} \cdot X_0 \\
& \xleftarrow{C_{117}} X_0 \cdot Z_2 \cdot X_1 \cdot CCX_{0,1} \cdot CZ_{0,1} \cdot X_1 \cdot \overline{X_0 \cdot Z_2 \cdot CZ_{0,2}} \\
& \xleftarrow{B_{25}} X_0 \cdot \overline{X_1 \cdot Z_2} \cdot CCX_{0,1} \cdot CZ_{0,1} \cdot X_1 \cdot X_0 \cdot Z_2 \cdot CZ_{0,2} \\
& \xrightarrow{C_{125}} X_0 \cdot X_1 \cdot \overline{CCX_{0,1} \cdot CZ_{0,1} \cdot Z_2 \cdot CZ_{0,1}} \cdot X_1 \cdot X_0 \cdot Z_2 \cdot CZ_{0,2} \\
& \xleftarrow{B_{27}} X_0 \cdot X_1 \cdot CCX_{0,1} \cdot CZ_{0,1} \cdot \overline{CZ_{0,1} \cdot Z_2 \cdot X_1} \cdot X_0 \cdot Z_2 \cdot CZ_{0,2} \\
& \xleftarrow{B_{25}} X_0 \cdot X_1 \cdot CCX_{0,1} \cdot CZ_{0,1} \cdot CZ_{0,1} \cdot \overline{X_1 \cdot Z_2 \cdot X_0} \cdot Z_2 \cdot CZ_{0,2} \\
& \xleftarrow{B_{26}} X_0 \cdot X_1 \cdot CCX_{0,1} \cdot CZ_{0,1} \cdot CZ_{0,1} \cdot X_1 \cdot \overline{X_0 \cdot Z_2 \cdot Z_2} \cdot CZ_{0,2} \\
& \xrightarrow{E_{19}} X_0 \cdot X_1 \cdot CCX_{0,1} \cdot \overline{CZ_{0,1} \cdot CZ_{0,1}} \cdot X_1 \cdot X_0 \cdot CZ_{0,2} \\
& \xrightarrow{E_2} X_0 \cdot X_1 \cdot \overline{CCX_{0,1} \cdot X_1 \cdot X_0} \cdot CZ_{0,2} \xleftarrow{D_1} \overline{r_1} \cdot CZ_{0,2} \\
\\
& r_1 \cdot \underline{r_7} \cdot r_1 \cdot r_7 \xrightarrow{\xi_2} r_1 \cdot \overline{r_6 \cdot CZ_{0,2} \cdot CZ_{0,1}} \cdot r_1 \cdot r_7 \xrightarrow{\delta_6} r_1 \cdot r_6 \cdot \overline{CZ_{0,2} \cdot r_1 \cdot CZ_{0,1}} \cdot r_7 \xrightarrow{\delta_7} r_1 \cdot r_6 \cdot \overline{r_1 \cdot CZ_{0,2}} \cdot CZ_{0,1} \cdot \underline{r_7} \\
& \xrightarrow{\xi_2} r_1 \cdot r_6 \cdot r_1 \cdot CZ_{0,2} \cdot CZ_{0,1} \cdot \overline{r_6 \cdot CZ_{0,2} \cdot CZ_{0,1}} \\
& \xrightarrow{\xi_3} r_1 \cdot r_6 \cdot r_1 \cdot CZ_{0,2} \cdot \overline{CZ_{0,1} \cdot CZ_{0,2} \cdot CZ_{0,1}} \cdot r_6 \\
& \xrightarrow{C_{60}} r_1 \cdot r_6 \cdot r_1 \cdot CZ_{0,2} \cdot \overline{CZ_{0,2} \cdot CZ_{0,1}} \cdot CZ_{0,1} \cdot r_6 \\
& \xrightarrow{E_2} r_1 \cdot r_6 \cdot r_1 \cdot \overline{CZ_{0,2} \cdot CZ_{0,2}} \cdot r_6 \xrightarrow{E_{11}} \underline{r_1 \cdot r_6 \cdot r_1 \cdot r_6} \xrightarrow{(1;6)} \varepsilon
\end{aligned}$$

### 1.7.15 Deriving the Coxeter Relation ( 1 ; 8 )

$$\begin{aligned}
(1;8) : r_1 \cdot r_8 \cdot \underline{r_1} \cdot r_8 & \xrightarrow{D_1} r_1 \cdot r_8 \cdot \overline{X_0 \cdot X_1 \cdot CCX_{0,1} \cdot X_1 \cdot X_0} \cdot r_8 \xrightarrow{\xi_4} r_1 \cdot r_8 \cdot X_0 \cdot X_1 \cdot CCX_{0,1} \cdot \overline{X_1 \cdot r_8} \cdot X_0 \\
& \xrightarrow{\xi_7} r_1 \cdot r_8 \cdot X_0 \cdot X_1 \cdot CCX_{0,1} \cdot \overline{r_8 \cdot X_1} \cdot X_0 \\
& \xleftarrow{\xi_4} r_1 \cdot \overline{X_0 \cdot r_8} \cdot X_1 \cdot CCX_{0,1} \cdot r_8 \cdot X_1 \cdot X_0 \\
& \xleftarrow{\xi_7} r_1 \cdot X_0 \cdot \overline{X_1 \cdot r_8} \cdot CCX_{0,1} \cdot r_8 \cdot X_1 \cdot X_0 \\
& \xrightarrow{\xi_8} r_1 \cdot X_0 \cdot X_1 \cdot \overline{r_8 \cdot r_8} \cdot \overline{CCX_{0,1}} \cdot X_1 \cdot X_0 \\
& \xrightarrow{(8,8)} r_1 \cdot X_0 \cdot X_1 \cdot \overline{CCX_{0,1} \cdot X_1 \cdot X_0} \xleftarrow{D_1} \underline{r_1 \cdot r_1} \xrightarrow{(1;1)} \varepsilon
\end{aligned}$$

### 1.7.16 Deriving the Coxeter Relation ( 2 ; 3 )

$$\begin{aligned}
r_2 \cdot r_3 \cdot \underline{r_2 \cdot r_3} \cdot r_2 \cdot r_3 & \xrightarrow{\omega_4} \underline{r_2 \cdot r_3} \cdot \overline{X_0 \cdot CCX_{0,1} \cdot CCX_{0,2} \cdot X_0} \cdot r_2 \cdot r_3 \xrightarrow{\omega_4} \overline{X_0 \cdot CCX_{0,1} \cdot CCX_{0,2} \cdot X_0 \cdot X_0} \cdot CCX_{0,1} \cdot CCX_{0,2} \cdot X_0 \cdot r_2 \cdot r_3 \\
& \xrightarrow{(21)} X_0 \cdot CCX_{0,1} \cdot \overline{CCX_{0,2} \cdot CCX_{0,1} \cdot CCX_{0,2}} \cdot X_0 \cdot r_2 \cdot r_3 \\
& \xrightarrow{\chi_9} X_0 \cdot \overline{CCX_{0,1} \cdot CCX_{0,1}} \cdot \overline{CCX_{0,2} \cdot CCX_{0,1}} \cdot X_0 \cdot r_2 \cdot r_3
\end{aligned}$$

$$\begin{aligned}
& \xrightarrow{E_{18}} X_0 \cdot CCX_{0,2} \cdot CCX_{0,1} \cdot X_0 \cdot \underline{r_2 \cdot r_3} \\
& \xrightarrow{\omega_4} X_0 \cdot CCX_{0,2} \cdot CCX_{0,1} \cdot \underline{X_0 \cdot \bar{X}_0 \cdot CCX_{0,1} \cdot CCX_{0,2} \cdot X_0} \\
& \xrightarrow{(21)} X_0 \cdot CCX_{0,2} \cdot \underline{CCX_{0,1} \cdot CCX_{0,1} \cdot CCX_{0,2} \cdot X_0} \\
& \xrightarrow{E_{18}} X_0 \cdot \underline{CCX_{0,2} \cdot CCX_{0,2} \cdot X_0} \xrightarrow{E_7} \underline{X_0 \cdot X_0} \xrightarrow{(21)} \varepsilon
\end{aligned}$$

### 1.7.17 Deriving the Coxeter Relation ( 2 ; 4 )

$$\begin{aligned}
(\delta_8) : CCX_{0,1} \cdot CCX_{0,2} \cdot CCX_{1,2} \cdot \underline{CCX_{0,2}} \cdot CCX_{0,1} & \xrightarrow{(14)} CCX_{0,1} \cdot \underline{CCX_{0,2} \cdot CCX_{1,2} \cdot \sigma_{0,1} \cdot \overline{CCX_{1,2} \cdot \sigma_{0,1}}} \cdot CCX_{0,1} \\
& \xrightarrow{(14)} CCX_{0,1} \cdot \overline{\sigma_{0,1} \cdot \overline{CCX_{1,2} \cdot \sigma_{0,1} \cdot CCX_{1,2} \cdot \sigma_{0,1}}} \cdot CCX_{1,2} \cdot \sigma_{0,1} \cdot CCX_{0,1} \\
& \xleftarrow{(14)} CCX_{0,1} \cdot \sigma_{0,1} \cdot CCX_{1,2} \cdot \overline{CCX_{0,2}} \cdot CCX_{1,2} \cdot \sigma_{0,1} \cdot \underline{CCX_{0,1}} \\
& \xrightarrow{S_{17}} CCX_{0,1} \cdot \sigma_{0,1} \cdot CCX_{1,2} \cdot CCX_{0,2} \cdot CCX_{1,2} \cdot \underline{\sigma_{0,1} \cdot \overline{\sigma_{0,1} \cdot \overline{CCX_{0,1} \cdot \sigma_{0,1}}}} \\
& \xrightarrow{E_4} \underline{CCX_{0,1}} \cdot \sigma_{0,1} \cdot CCX_{1,2} \cdot CCX_{0,2} \cdot CCX_{1,2} \cdot CCX_{0,1} \cdot \sigma_{0,1} \\
& \xrightarrow{S_{17}} \overline{\sigma_{0,1} \cdot \overline{CCX_{0,1} \cdot \sigma_{0,1} \cdot \overline{\sigma_{0,1}}}} \cdot CCX_{1,2} \cdot CCX_{0,2} \cdot CCX_{1,2} \cdot CCX_{0,1} \cdot \sigma_{0,1} \\
& \xrightarrow{E_4} \sigma_{0,1} \cdot \underline{CCX_{0,1}} \cdot CCX_{1,2} \cdot CCX_{0,2} \cdot CCX_{1,2} \cdot CCX_{0,1} \cdot \sigma_{0,1} \\
& \xrightarrow{(32)} \sigma_{0,1} \cdot \overline{\sigma_{0,2} \cdot \overline{CCX_{1,2} \cdot \sigma_{0,2} \cdot CCX_{1,2} \cdot \underline{CCX_{0,2}} \cdot CCX_{1,2} \cdot CCX_{0,1} \cdot \sigma_{0,1}}} \\
& \xrightarrow{S_{19}} \sigma_{0,1} \cdot \sigma_{0,2} \cdot CCX_{1,2} \cdot \underline{\sigma_{0,2} \cdot \overline{CCX_{1,2} \cdot \sigma_{0,2} \cdot \overline{CCX_{0,2} \cdot \sigma_{0,2} \cdot CCX_{1,2} \cdot CCX_{0,1} \cdot \sigma_{0,1}}}} \\
& \xleftarrow{(32)} \sigma_{0,1} \cdot \sigma_{0,2} \cdot CCX_{1,2} \cdot \overline{CCX_{0,1}} \cdot CCX_{0,2} \cdot \sigma_{0,2} \cdot CCX_{1,2} \cdot \underline{CCX_{0,1} \cdot \sigma_{0,1}} \\
& \xrightarrow{(32)} \sigma_{0,1} \cdot \sigma_{0,2} \cdot CCX_{1,2} \cdot CCX_{0,1} \cdot CCX_{0,2} \cdot \underline{\sigma_{0,2} \cdot \overline{CCX_{1,2} \cdot \sigma_{0,2} \cdot \overline{CCX_{1,2} \cdot \sigma_{0,2} \cdot \sigma_{0,1}}}} \\
& \xleftarrow{(32)} \sigma_{0,1} \cdot \sigma_{0,2} \cdot \underline{CCX_{1,2} \cdot CCX_{0,1} \cdot CCX_{0,2} \cdot \overline{CCX_{0,1} \cdot CCX_{1,2} \cdot \sigma_{0,2} \cdot \sigma_{0,1}}} \\
& \xrightarrow{\xi_5} \sigma_{0,1} \cdot \sigma_{0,2} \cdot \overline{CCX_{0,1} \cdot \overline{CCX_{0,2} \cdot \underline{CCX_{0,1}}}} \cdot \sigma_{0,2} \cdot \sigma_{0,1} \\
& \xrightarrow{(32)} \sigma_{0,1} \cdot \sigma_{0,2} \cdot CCX_{0,1} \cdot CCX_{0,2} \cdot \overline{\sigma_{0,2} \cdot \overline{CCX_{1,2} \cdot \sigma_{0,2} \cdot \underline{\sigma_{0,2} \cdot \sigma_{0,1}}}} \\
& \xrightarrow{E_{16}} \sigma_{0,1} \cdot \sigma_{0,2} \cdot \underline{CCX_{0,1} \cdot CCX_{0,2} \cdot \sigma_{0,2} \cdot CCX_{1,2} \cdot \sigma_{0,1}} \\
& \xrightarrow{(32)} \sigma_{0,1} \cdot \underline{\sigma_{0,2} \cdot \overline{\sigma_{0,2} \cdot \overline{CCX_{1,2} \cdot \sigma_{0,2} \cdot CCX_{0,2} \cdot \sigma_{0,2} \cdot CCX_{1,2} \cdot \sigma_{0,1}}}} \\
& \xrightarrow{E_{16}} \sigma_{0,1} \cdot CCX_{1,2} \cdot \underline{\sigma_{0,2} \cdot \overline{CCX_{0,2} \cdot \sigma_{0,2} \cdot CCX_{1,2} \cdot \sigma_{0,1}}} \\
& \xleftarrow{S_{19}} \sigma_{0,1} \cdot CCX_{1,2} \cdot \overline{CCX_{0,2}} \cdot CCX_{1,2} \cdot \sigma_{0,1} \\
& \xrightarrow{(14)} \sigma_{0,1} \cdot CCX_{1,2} \cdot \overline{\sigma_{0,1} \cdot \overline{CCX_{1,2} \cdot \sigma_{0,1} \cdot CCX_{1,2} \cdot \sigma_{0,1}}} \\
& \xleftarrow{(14)} \underline{\sigma_{0,1} \cdot \overline{CCX_{1,2} \cdot \sigma_{0,1} \cdot CCX_{1,2} \cdot \overline{CCX_{0,2}}}} \xleftarrow{(14)} \overline{CCX_{0,2} \cdot CCX_{1,2} \cdot CCX_{0,2}}
\end{aligned}$$

$$\begin{aligned}
(\delta_9) : \underline{r_2} & \xrightarrow{D_2} \overline{X_0 \cdot CX_{2,1} \cdot CCX_{0,1} \cdot CX_{2,1} \cdot X_0} \xrightarrow{B_1} \underline{X_0 \cdot CX_{2,1} \cdot CCX_{0,1} \cdot \bar{X}_0 \cdot CX_{2,1}} \\
& \xleftarrow{B_1} \overline{CX_{2,1} \cdot \bar{X}_0 \cdot CCX_{0,1} \cdot X_0 \cdot CX_{2,1}} \\
& \xleftarrow{X_2} CX_{2,1} \cdot \overline{CX_{1,0} \cdot \overline{CCX_{0,1} \cdot CX_{1,0}}} \cdot CX_{2,1} \\
& \xrightarrow{C_{72}} CX_{2,1} \cdot \overline{CCX_{0,1} \cdot CX_{1,2} \cdot \underline{CX_{1,0} \cdot CX_{1,0}}} \cdot CX_{2,1}
\end{aligned}$$

$$\begin{aligned}
& \xrightarrow{E_1} CX_{2,1} \cdot CCX_{0,1} \cdot CX_{1,2} \cdot CX_{2,1} \\
& \xleftarrow{E_8} CX_{2,1} \cdot CCX_{0,1} \cdot \underline{CX_{1,2} \cdot CX_{2,1} \cdot \overline{CX_{1,2}} \cdot CX_{1,2}} \\
& \xleftarrow{(8)} CX_{2,1} \cdot CCX_{0,1} \cdot \overline{\sigma_{1,2}} \cdot \underline{CX_{1,2}} \\
& \xrightarrow{S_8} CX_{2,1} \cdot CCX_{0,1} \cdot \underline{\sigma_{1,2}} \cdot \overline{\sigma_{1,2}} \cdot \underline{CX_{2,1}} \cdot \sigma_{1,2} \xrightarrow{E_{10}} CX_{2,1} \cdot CCX_{0,1} \cdot CX_{2,1} \cdot \sigma_{1,2} \\
\\
(\delta_{10}) : \sigma_{1,2} \cdot \underline{r_4} \xrightarrow{D_4} \sigma_{1,2} \cdot \overline{CX_{0,1} \cdot \underline{CX_{0,2}} \cdot CCX_{1,2} \cdot CX_{0,2} \cdot CX_{0,1}} \xrightarrow{(9)} \underline{\sigma_{1,2} \cdot CX_{0,1} \cdot \overline{\sigma_{1,2}} \cdot CX_{0,1}} \cdot CCX_{1,2} \cdot CX_{0,2} \cdot CX_{0,1} \\
& \xleftarrow{(9)} \overline{CX_{0,2}} \cdot CX_{0,1} \cdot \sigma_{1,2} \cdot \underline{CCX_{1,2}} \cdot CX_{0,2} \cdot CX_{0,1} \\
& \xrightarrow{S_{20}} CX_{0,2} \cdot CX_{0,1} \cdot \underline{\sigma_{1,2} \cdot \overline{\sigma_{1,2}} \cdot CCX_{1,2} \cdot \sigma_{1,2}} \cdot CX_{0,2} \cdot CX_{0,1} \\
& \xrightarrow{E_{10}} CX_{0,2} \cdot CX_{0,1} \cdot CCX_{1,2} \cdot \sigma_{1,2} \cdot \underline{CX_{0,2}} \cdot CX_{0,1} \\
& \xrightarrow{(9)} CX_{0,2} \cdot CX_{0,1} \cdot CCX_{1,2} \cdot \underline{\sigma_{1,2} \cdot \overline{\sigma_{1,2}}} \cdot \overline{CX_{0,1}} \cdot \sigma_{1,2} \cdot CX_{0,1} \\
& \xrightarrow{E_{10}} CX_{0,2} \cdot CX_{0,1} \cdot CCX_{1,2} \cdot CX_{0,1} \cdot \sigma_{1,2} \cdot CX_{0,1} \\
& \xleftarrow{E_{10}} CX_{0,2} \cdot CX_{0,1} \cdot CCX_{1,2} \cdot CX_{0,1} \cdot \underline{\sigma_{1,2} \cdot CX_{0,1} \cdot \overline{\sigma_{1,2}} \cdot \sigma_{1,2}} \\
& \xleftarrow{(9)} CX_{0,2} \cdot CX_{0,1} \cdot CCX_{1,2} \cdot \underline{CX_{0,1} \cdot \overline{CX_{0,2}}} \cdot \sigma_{1,2} \\
& \xrightarrow{C_{22}} \underline{CX_{0,2} \cdot CX_{0,1}} \cdot CCX_{1,2} \cdot \overline{CX_{0,2} \cdot CX_{0,1}} \cdot \sigma_{1,2} \\
& \xleftarrow{C_{22}} \underline{\overline{CX_{0,1} \cdot CX_{0,2}} \cdot CCX_{1,2} \cdot CX_{0,2} \cdot CX_{0,1}} \cdot \sigma_{1,2} \xleftarrow{D_4} \overline{r_4} \cdot \sigma_{1,2} \\
\\
(\delta_{11}) : CX_{2,1} \cdot CCX_{0,1} \cdot CX_{2,1} \cdot \underline{r_4} \\
& \xrightarrow{D_4} CX_{2,1} \cdot CCX_{0,1} \cdot CX_{2,1} \cdot \overline{CX_{0,1} \cdot \underline{CX_{0,2}} \cdot CCX_{1,2} \cdot CX_{0,2} \cdot CX_{0,1}} \\
& \xrightarrow{C_{22}} CX_{2,1} \cdot CCX_{0,1} \cdot \underline{CX_{2,1} \cdot \overline{CX_{0,2} \cdot CX_{0,1}}} \cdot CCX_{1,2} \cdot CX_{0,2} \cdot CX_{0,1} \\
& \xleftarrow{C_{18}} CX_{2,1} \cdot CCX_{0,1} \cdot \overline{CX_{0,2} \cdot CX_{2,1}} \cdot CCX_{1,2} \cdot CX_{0,2} \cdot CX_{0,1} \\
& \xrightarrow{C_{61}} CX_{2,1} \cdot CCX_{0,1} \cdot CX_{0,2} \cdot \overline{CCX_{1,2} \cdot CX_{2,0} \cdot \underline{CX_{2,1}}} \cdot CX_{0,2} \cdot CX_{0,1} \\
& \xleftarrow{C_{18}} CX_{2,1} \cdot CCX_{0,1} \cdot CX_{0,2} \cdot \underline{CCX_{1,2} \cdot CX_{2,0}} \cdot \overline{CX_{0,2} \cdot CX_{2,1}} \\
& \xrightarrow{C_{101}} CX_{2,1} \cdot CCX_{0,1} \cdot CX_{0,2} \cdot \overline{CX_{2,0} \cdot CCX_{1,2}} \cdot CX_{0,2} \cdot CX_{2,1} \\
& \xleftarrow{E_{15}} CX_{2,1} \cdot CCX_{0,1} \cdot CX_{0,2} \cdot CX_{2,0} \cdot \overline{CX_{0,2} \cdot \underline{CX_{0,2}} \cdot CCX_{1,2} \cdot CX_{0,2}} \cdot CX_{2,1} \\
& \xrightarrow{X_4} CX_{2,1} \cdot CCX_{0,1} \cdot CX_{0,2} \cdot CX_{2,0} \cdot CX_{0,2} \cdot \overline{CCX_{0,1} \cdot CCX_{1,2} \cdot CCX_{0,1}} \cdot CX_{2,1} \\
& \xleftarrow{E_9} CX_{2,1} \cdot CCX_{0,1} \cdot CX_{0,2} \cdot CX_{2,0} \cdot CX_{0,2} \cdot CCX_{0,1} \cdot \overline{CX_{2,1} \cdot \underline{CX_{2,1}} \cdot CCX_{1,2}} \cdot CCX_{0,1} \cdot CX_{2,1} \\
& \xrightarrow{C_{61}} CX_{2,1} \cdot CCX_{0,1} \cdot CX_{0,2} \cdot CX_{2,0} \cdot CX_{0,2} \cdot CCX_{0,1} \cdot CX_{2,1} \cdot \overline{CCX_{1,2} \cdot CX_{2,0} \cdot CX_{2,1}} \cdot CCX_{0,1} \cdot CX_{2,1} \\
& \xleftarrow{(22)} \overline{CX_{0,1} \cdot \underline{CX_{0,1}}} \cdot CX_{2,1} \cdot \underline{CCX_{0,1} \cdot CX_{0,2}} \cdot CX_{2,0} \cdot CX_{0,2} \cdot CCX_{0,1} \cdot CX_{2,1} \cdot CCX_{1,2} \cdot CX_{2,0} \cdot CX_{2,1} \cdot CCX_{0,1} \cdot CX_{2,1} \\
& \xrightarrow{C_{105}} CX_{0,1} \cdot \underline{CX_{0,1} \cdot CX_{2,1}} \cdot \overline{CX_{0,2} \cdot CCX_{0,1}} \cdot CX_{2,0} \cdot CX_{0,2} \cdot CCX_{0,1} \cdot CX_{2,1} \cdot CCX_{1,2} \cdot CX_{2,0} \cdot CX_{2,1} \cdot CCX_{0,1} \cdot CX_{2,1} \\
& \xrightarrow{C_{20}} CX_{0,1} \cdot \underline{\overline{CX_{2,1}} \cdot \underline{CX_{0,1}}} \cdot CX_{0,2} \cdot CCX_{0,1} \cdot CX_{2,0} \cdot CX_{0,2} \cdot CCX_{0,1} \cdot CX_{2,1} \cdot CCX_{1,2} \cdot CX_{2,0} \cdot CX_{2,1} \cdot CCX_{0,1} \cdot CX_{2,1} \\
& \xrightarrow{C_{45}} CX_{0,1} \cdot \overline{CX_{0,2} \cdot CX_{2,1}} \cdot CCX_{0,1} \cdot CX_{2,0} \cdot CX_{0,2} \cdot CCX_{0,1} \cdot CX_{2,1} \cdot \underline{CCX_{1,2} \cdot CX_{2,0} \cdot CX_{2,1}} \cdot CCX_{0,1} \cdot CX_{2,1} \\
& \xleftarrow{C_{61}} CX_{0,1} \cdot CX_{0,2} \cdot CX_{2,1} \cdot CCX_{0,1} \cdot CX_{2,0} \cdot CX_{0,2} \cdot CCX_{0,1} \cdot \underline{CX_{2,1} \cdot \overline{CX_{2,1}} \cdot CCX_{1,2}} \cdot CCX_{0,1} \cdot CX_{2,1}
\end{aligned}$$

$$\begin{aligned}
& \xrightarrow{E_9} CX_{0,1} \cdot CX_{0,2} \cdot CX_{2,1} \cdot CCX_{0,1} \cdot CX_{2,0} \cdot CX_{0,2} \cdot CCX_{0,1} \cdot CCX_{1,2} \cdot CCX_{0,1} \cdot CX_{2,1} \\
& \xleftarrow{E_{15}} CX_{0,1} \cdot CX_{0,2} \cdot CX_{2,1} \cdot CCX_{0,1} \cdot CX_{2,0} \cdot \overline{CX_{0,2} \cdot CCX_{0,1}} \cdot CCX_{1,2} \cdot \overline{CX_{0,2} \cdot CX_{0,2}} \cdot CCX_{0,1} \cdot CX_{2,1} \\
& \xleftarrow{C_{105}} CX_{0,1} \cdot CX_{0,2} \cdot CX_{2,1} \cdot CCX_{0,1} \cdot CX_{2,0} \cdot \overline{CCX_{0,1} \cdot CX_{0,2}} \cdot CCX_{1,2} \cdot \overline{CX_{0,2}} \cdot CX_{0,2} \cdot CCX_{0,1} \cdot CX_{2,1} \\
& \xrightarrow{X_4} CX_{0,1} \cdot CX_{0,2} \cdot CX_{2,1} \cdot CCX_{0,1} \cdot CX_{2,0} \cdot \overline{CCX_{0,1} \cdot CCX_{0,1}} \cdot \overline{CCX_{1,2} \cdot CCX_{0,1}} \cdot CX_{0,2} \cdot CCX_{0,1} \cdot CX_{2,1} \\
& \xrightarrow{E_{18}} CX_{0,1} \cdot CX_{0,2} \cdot CX_{2,1} \cdot CCX_{0,1} \cdot CX_{2,0} \cdot CCX_{1,2} \cdot CCX_{0,1} \cdot CX_{0,2} \cdot CCX_{0,1} \cdot CX_{2,1} \\
& \xleftarrow{E_9} CX_{0,1} \cdot CX_{0,2} \cdot \overline{CX_{2,1} \cdot CCX_{0,1}} \cdot \overline{CX_{2,1} \cdot CX_{2,1}} \cdot CX_{2,0} \cdot CCX_{1,2} \cdot CCX_{0,1} \cdot CX_{0,2} \cdot CCX_{0,1} \cdot CX_{2,1} \\
& \xrightarrow{X_6} CX_{0,1} \cdot CX_{0,2} \cdot \overline{CCX_{0,2} \cdot CCX_{0,1}} \cdot \overline{CCX_{0,2} \cdot CX_{2,1}} \cdot \overline{CX_{2,0} \cdot CCX_{1,2}} \cdot CCX_{0,1} \cdot CX_{0,2} \cdot CCX_{0,1} \cdot CX_{2,1} \\
& \xleftarrow{C_{101}} CX_{0,1} \cdot CX_{0,2} \cdot CCX_{0,2} \cdot CCX_{0,1} \cdot CCX_{0,2} \cdot \overline{CX_{2,1} \cdot CCX_{1,2}} \cdot \overline{CX_{2,0} \cdot CCX_{0,1}} \cdot CX_{0,2} \cdot CCX_{0,1} \cdot CX_{2,1} \\
& \xrightarrow{C_{61}} CX_{0,1} \cdot CX_{0,2} \cdot CCX_{0,2} \cdot CCX_{0,1} \cdot CCX_{0,2} \cdot \overline{CCX_{1,2} \cdot CX_{2,0}} \cdot \overline{CX_{2,1} \cdot CX_{2,0}} \cdot CCX_{0,1} \cdot CX_{0,2} \cdot CCX_{0,1} \cdot CX_{2,1} \\
& \xrightarrow{C_{67}} CX_{0,1} \cdot CX_{0,2} \cdot CCX_{0,2} \cdot CCX_{0,1} \cdot CCX_{0,2} \cdot CCX_{1,2} \cdot \overline{CX_{2,0} \cdot CX_{2,0}} \cdot \overline{CX_{2,1} \cdot CX_{2,1}} \cdot CCX_{0,1} \cdot CX_{0,2} \cdot CCX_{0,1} \cdot CX_{2,1} \\
& \xrightarrow{E_{14}} CX_{0,1} \cdot CX_{0,2} \cdot CCX_{0,2} \cdot CCX_{0,1} \cdot CCX_{0,2} \cdot CCX_{1,2} \cdot CX_{2,1} \cdot CCX_{0,1} \cdot CX_{0,2} \cdot CCX_{0,1} \cdot CX_{2,1} \\
& \xleftarrow{E_9} CX_{0,1} \cdot CX_{0,2} \cdot CCX_{0,2} \cdot CCX_{0,1} \cdot CCX_{0,2} \cdot CCX_{1,2} \cdot \overline{CX_{2,1} \cdot CCX_{0,1}} \cdot \overline{CX_{2,1} \cdot CX_{2,1}} \cdot CX_{0,2} \cdot CCX_{0,1} \cdot CX_{2,1} \\
& \xrightarrow{X_6} CX_{0,1} \cdot CX_{0,2} \cdot CCX_{0,2} \cdot \overline{CCX_{0,1} \cdot CCX_{0,2}} \cdot \overline{CCX_{1,2} \cdot CCX_{0,2}} \cdot \overline{CCX_{0,2} \cdot CCX_{0,1}} \cdot \overline{CCX_{0,2} \cdot CX_{2,1}} \cdot CX_{0,2} \cdot CCX_{0,1} \cdot CX_{2,1} \\
& \xrightarrow{\delta_8} CX_{0,1} \cdot CX_{0,2} \cdot CCX_{0,2} \cdot \overline{CCX_{0,2} \cdot CCX_{1,2}} \cdot \overline{CCX_{0,2} \cdot CCX_{0,2}} \cdot CX_{2,1} \cdot CX_{0,2} \cdot CCX_{0,1} \cdot CX_{2,1} \\
& \xrightarrow{E_7} CX_{0,1} \cdot CX_{0,2} \cdot \overline{CCX_{0,2} \cdot CCX_{0,2}} \cdot CCX_{1,2} \cdot CX_{2,1} \cdot CX_{0,2} \cdot CCX_{0,1} \cdot CX_{2,1} \\
& \xrightarrow{E_7} CX_{0,1} \cdot CX_{0,2} \cdot CCX_{1,2} \cdot \overline{CX_{2,1} \cdot CX_{0,2}} \cdot CCX_{0,1} \cdot CX_{2,1} \\
& \xrightarrow{C_{19}} CX_{0,1} \cdot CX_{0,2} \cdot CCX_{1,2} \cdot \overline{CX_{0,2} \cdot CX_{2,1}} \cdot \overline{CX_{0,1} \cdot CX_{0,1}} \cdot CCX_{0,1} \cdot CX_{2,1} \\
& \xleftarrow{C_{20}} CX_{0,1} \cdot CX_{0,2} \cdot CCX_{1,2} \cdot \overline{CX_{0,2} \cdot CX_{0,1}} \cdot \overline{CX_{2,1} \cdot CX_{2,1}} \cdot CCX_{0,1} \cdot CX_{2,1} \\
& \xleftarrow{C_{22}} CX_{0,1} \cdot CX_{0,2} \cdot CCX_{1,2} \cdot \overline{CX_{0,1} \cdot CX_{0,2}} \cdot CX_{2,1} \cdot CCX_{0,1} \cdot CX_{2,1} \\
& \xrightarrow{C_{22}} \overline{CX_{0,1} \cdot CX_{0,2} \cdot CCX_{1,2} \cdot CX_{0,2} \cdot CX_{0,1}} \cdot CX_{2,1} \cdot CCX_{0,1} \cdot CX_{2,1} \quad \xleftarrow{D_4} \overline{r_4} \cdot CX_{2,1} \cdot CCX_{0,1} \cdot CX_{2,1}
\end{aligned}$$

$$(\delta_{12}) : \underline{r_2} \cdot r_4 \xrightarrow{\delta_9} \overline{CX_{2,1} \cdot CCX_{0,1} \cdot CX_{2,1} \cdot \sigma_{1,2} \cdot r_4} \xrightarrow{\delta_{10}} \overline{CX_{2,1} \cdot CCX_{0,1} \cdot CX_{2,1} \cdot \overline{r_4} \cdot \sigma_{1,2}} \xrightarrow{\delta_{11}} \overline{r_4 \cdot CX_{2,1} \cdot CCX_{0,1} \cdot CX_{2,1} \cdot \sigma_{1,2}} \xleftarrow{\delta_9} r_4 \cdot \overline{r_2}$$

$$\underline{r_2} \cdot \underline{r_4} \cdot r_2 \cdot r_4 \xrightarrow{\delta_{12}} \overline{\overline{r_4} \cdot \overline{r_2} \cdot r_2 \cdot r_4} \xrightarrow{(2;2)} \underline{r_4} \cdot \underline{r_4} \xrightarrow{(4;4)} \mathcal{E}$$

### 1.7.18 Deriving the Coxeter Relation ( 2 ; 5 )

$$\begin{aligned}
r_2 \cdot r_5 \cdot r_2 \cdot r_5 & \xleftarrow{(21)} r_2 \cdot r_5 \cdot r_2 \cdot \underline{r_5} \cdot \overline{X_0 \cdot X_0} \xrightarrow{D_6} r_2 \cdot r_5 \cdot \underline{r_2} \cdot \overline{X_1 \cdot CCX_{0,1} \cdot X_1} \cdot X_0 \cdot X_0 \\
& \xrightarrow{D_2} r_2 \cdot r_5 \cdot \overline{X_0 \cdot CX_{2,1} \cdot CCX_{0,1} \cdot CX_{2,1} \cdot X_0} \cdot X_1 \cdot \overline{CCX_{0,1} \cdot X_1 \cdot X_0 \cdot X_0} \\
& \xleftarrow{D_1} r_2 \cdot r_5 \cdot X_0 \cdot \overline{CX_{2,1} \cdot CCX_{0,1} \cdot CX_{2,1}} \cdot \overline{r_1} \cdot X_0 \\
& \xleftarrow{D_6} r_2 \cdot \underline{r_5} \cdot X_0 \cdot \overline{r_6} \cdot r_1 \cdot X_0 \\
& \xrightarrow{D_6} \underline{r_2} \cdot \overline{X_1 \cdot CCX_{0,1} \cdot X_1} \cdot X_0 \cdot r_6 \cdot r_1 \cdot X_0
\end{aligned}$$

$$\begin{aligned}
& \xrightarrow{D_2} \overline{X_0 \cdot CX_{2,1} \cdot CCX_{0,1} \cdot CX_{2,1} \cdot \overline{X_0} \cdot X_1 \cdot CCX_{0,1} \cdot X_1 \cdot X_0 \cdot r_6 \cdot r_1 \cdot X_0} \\
& \xleftarrow{D_1} X_0 \cdot \overline{CX_{2,1} \cdot CCX_{0,1} \cdot CX_{2,1} \cdot \overline{r_1} \cdot r_6 \cdot r_1 \cdot X_0} \\
& \xleftarrow{D_6} X_0 \cdot \overline{r_6 \cdot r_1 \cdot r_6 \cdot r_1 \cdot X_0} \xleftarrow{\xi_6} X_0 \cdot \overline{r_1 \cdot \overline{r_6} \cdot r_6 \cdot r_1 \cdot X_0} \xrightarrow{(6;6)} X_0 \cdot \overline{r_1 \cdot r_1 \cdot X_0} \xrightarrow{(1;1)} \overline{X_0 \cdot X_0} \xrightarrow{(21)} \varepsilon
\end{aligned}$$

### 1.7.19 Deriving the Coxeter Relation ( 2 ; 6 )

$$\begin{aligned}
(\delta_{13}) : r_2 \cdot r_6 & \xrightarrow{D_6} \overline{r_2 \cdot CX_{2,1} \cdot CCX_{0,1} \cdot CX_{2,1}} \xrightarrow{D_2} \overline{X_0 \cdot CX_{2,1} \cdot CCX_{0,1} \cdot CX_{2,1} \cdot \overline{X_0} \cdot CX_{2,1} \cdot CCX_{0,1} \cdot CX_{2,1}} \\
& \xleftarrow{B_1} \overline{X_0 \cdot CX_{2,1} \cdot CCX_{0,1} \cdot CX_{2,1} \cdot \overline{CX_{2,1} \cdot \overline{X_0} \cdot CCX_{0,1} \cdot CX_{2,1}}} \\
& \xleftarrow{B_1} \overline{CX_{2,1} \cdot \overline{X_0} \cdot CCX_{0,1} \cdot CX_{2,1} \cdot CX_{2,1} \cdot X_0 \cdot CCX_{0,1} \cdot CX_{2,1}} \\
& \xrightarrow{E_9} CX_{2,1} \cdot X_0 \cdot CCX_{0,1} \cdot X_0 \cdot CCX_{0,1} \cdot CX_{2,1} \\
& \xleftarrow{E_{13}} CX_{2,1} \cdot X_0 \cdot CCX_{0,1} \cdot X_0 \cdot CCX_{0,1} \cdot \overline{X_1 \cdot \overline{X_1}} \cdot CX_{2,1} \\
& \xleftarrow{E_{13}} CX_{2,1} \cdot X_0 \cdot CCX_{0,1} \cdot X_0 \cdot \overline{X_1 \cdot \overline{X_1} \cdot CCX_{0,1} \cdot X_1 \cdot X_1 \cdot CX_{2,1}} \\
& \xleftarrow{D_6} CX_{2,1} \cdot X_0 \cdot CCX_{0,1} \cdot X_0 \cdot X_1 \cdot \overline{r_5} \cdot X_1 \cdot CX_{2,1} \\
& \xleftarrow{E_{13}} CX_{2,1} \cdot \overline{X_1 \cdot \overline{X_1}} \cdot X_0 \cdot CCX_{0,1} \cdot \overline{X_0 \cdot X_1 \cdot r_5 \cdot X_1 \cdot CX_{2,1}} \\
& \xrightarrow{B_2} CX_{2,1} \cdot X_1 \cdot \overline{X_1 \cdot X_0 \cdot CCX_{0,1} \cdot \overline{X_1 \cdot X_0} \cdot r_5 \cdot X_1 \cdot CX_{2,1}} \\
& \xleftarrow{B_2} CX_{2,1} \cdot X_1 \cdot \overline{X_0 \cdot \overline{X_1} \cdot CCX_{0,1} \cdot X_1 \cdot X_0 \cdot r_5 \cdot X_1 \cdot CX_{2,1}} \xleftarrow{D_1} CX_{2,1} \cdot X_1 \cdot \overline{r_1 \cdot r_5 \cdot X_1 \cdot CX_{2,1}} \\
r_2 \cdot r_6 \cdot r_2 \cdot r_6 & \xrightarrow{\delta_{13}} \overline{r_2 \cdot r_6 \cdot CX_{2,1} \cdot X_1 \cdot r_1 \cdot r_5 \cdot X_1 \cdot CX_{2,1}} \xrightarrow{\delta_{13}} \overline{CX_{2,1} \cdot X_1 \cdot r_1 \cdot r_5 \cdot X_1 \cdot CX_{2,1} \cdot CX_{2,1} \cdot X_1 \cdot r_1 \cdot r_5 \cdot X_1 \cdot CX_{2,1}} \\
& \xrightarrow{E_9} CX_{2,1} \cdot X_1 \cdot r_1 \cdot r_5 \cdot \overline{X_1 \cdot X_1 \cdot r_1 \cdot r_5 \cdot X_1 \cdot CX_{2,1}} \\
& \xrightarrow{E_{13}} CX_{2,1} \cdot X_1 \cdot \overline{r_1 \cdot r_5 \cdot r_1 \cdot r_5 \cdot X_1 \cdot CX_{2,1}} \xrightarrow{(1;5)} CX_{2,1} \cdot \overline{X_1 \cdot X_1 \cdot CX_{2,1}} \xrightarrow{E_{13}} \overline{CX_{2,1} \cdot CX_{2,1}} \xrightarrow{E_9} \varepsilon
\end{aligned}$$

### 1.7.20 Deriving the Coxeter Relation ( 2 ; 7 )

$$\begin{aligned}
(\delta_{14}) : CZ_{0,1} \cdot CX_{2,1} \cdot CCX_{0,1} \cdot CX_{2,1} & \xrightarrow{X_6} \overline{CZ_{0,1} \cdot \overline{CCX_{0,2} \cdot CCX_{0,1} \cdot CCX_{0,2}}} \xrightarrow{C_{80}} \overline{CCX_{0,2} \cdot CZ_{0,1} \cdot \overline{CZ_{0,2} \cdot CCX_{0,1} \cdot CCX_{0,2}}} \\
& \xrightarrow{C_{81}} \overline{CCX_{0,2} \cdot CZ_{0,1} \cdot \overline{CCX_{0,1} \cdot CZ_{0,1} \cdot CZ_{0,2} \cdot CCX_{0,2}}} \\
& \xrightarrow{C_{95}} \overline{CCX_{0,2} \cdot \overline{CCX_{0,1} \cdot \overline{CZ_{0,1} \cdot CZ_{0,2} \cdot CCX_{0,2}}}} \\
& \xrightarrow{E_2} \overline{CCX_{0,2} \cdot CCX_{0,1} \cdot \overline{CZ_{0,2} \cdot CCX_{0,2}}} \\
& \xrightarrow{C_{96}} \overline{CCX_{0,2} \cdot CCX_{0,1} \cdot \overline{CCX_{0,2} \cdot CZ_{0,2}}} \xleftarrow{X_6} \overline{CX_{2,1} \cdot CCX_{0,1} \cdot CX_{2,1} \cdot CZ_{0,2}} \\
(\delta_{15}) : CZ_{0,2} \cdot CX_{2,1} \cdot CCX_{0,1} \cdot CX_{2,1} & \xleftarrow{E_9} \overline{CX_{2,1} \cdot CX_{2,1} \cdot CZ_{0,2} \cdot CX_{2,1} \cdot CCX_{0,1} \cdot CX_{2,1}} \\
& \xleftarrow{E_{18}} \overline{CX_{2,1} \cdot \overline{CCX_{0,1} \cdot \overline{CCX_{0,1} \cdot CX_{2,1} \cdot CZ_{0,2} \cdot CX_{2,1} \cdot CCX_{0,1} \cdot CX_{2,1}}}} \\
& \xleftarrow{E_9} \overline{CX_{2,1} \cdot CCX_{0,1} \cdot \overline{CX_{2,1} \cdot CX_{2,1} \cdot CCX_{0,1} \cdot CX_{2,1} \cdot CZ_{0,2} \cdot CX_{2,1} \cdot CCX_{0,1} \cdot CX_{2,1}}} \\
& \xleftarrow{E_2} \overline{CX_{2,1} \cdot CCX_{0,1} \cdot CX_{2,1} \cdot \overline{CZ_{0,1} \cdot \overline{CZ_{0,1} \cdot CX_{2,1} \cdot CCX_{0,1} \cdot CX_{2,1} \cdot CZ_{0,2} \cdot CX_{2,1} \cdot CCX_{0,1} \cdot CX_{2,1}}}}
\end{aligned}$$

$$\begin{aligned}
& \xrightarrow{\delta_{14}} CX_{2,1} \cdot CCX_{0,1} \cdot CX_{2,1} \cdot CZ_{0,1} \cdot \overline{CX_{2,1} \cdot CCX_{0,1} \cdot CX_{2,1} \cdot CZ_{0,2}} \cdot CZ_{0,2} \cdot CX_{2,1} \cdot CCX_{0,1} \cdot CX_{2,1} \\
& \xrightarrow{E_{11}} CX_{2,1} \cdot CCX_{0,1} \cdot CX_{2,1} \cdot CZ_{0,1} \cdot CX_{2,1} \cdot CCX_{0,1} \cdot \overline{CX_{2,1} \cdot CX_{2,1}} \cdot CCX_{0,1} \cdot CX_{2,1} \\
& \xrightarrow{E_9} CX_{2,1} \cdot CCX_{0,1} \cdot CX_{2,1} \cdot CZ_{0,1} \cdot CX_{2,1} \cdot \overline{CCX_{0,1} \cdot CCX_{0,1}} \cdot CX_{2,1} \\
& \xrightarrow{E_{18}} CX_{2,1} \cdot CCX_{0,1} \cdot CX_{2,1} \cdot CZ_{0,1} \cdot \overline{CX_{2,1} \cdot CX_{2,1}} \xrightarrow{E_9} CX_{2,1} \cdot CCX_{0,1} \cdot CX_{2,1} \cdot CZ_{0,1} \\
\\
(\delta_{16}) : \underline{r_2} \cdot r_7 & \xrightarrow{D_2} \overline{X_0 \cdot CX_{2,1} \cdot CCX_{0,1} \cdot CX_{2,1} \cdot X_0} \cdot r_7 \xrightarrow{B_1} \overline{X_0 \cdot CX_{2,1} \cdot CCX_{0,1} \cdot X_0 \cdot CX_{2,1}} \cdot r_7 \\
& \xleftarrow{B_1} \overline{CX_{2,1} \cdot X_0 \cdot CCX_{0,1} \cdot X_0 \cdot CX_{2,1}} \cdot r_7 \\
& \xleftarrow{X_2} CX_{2,1} \cdot \overline{CX_{1,0} \cdot CCX_{0,1} \cdot CX_{1,0}} \cdot CX_{2,1} \cdot r_7 \\
& \xrightarrow{C_{72}} CX_{2,1} \cdot \overline{CCX_{0,1} \cdot CX_{1,2} \cdot CX_{1,0} \cdot CX_{1,0}} \cdot CX_{2,1} \cdot r_7 \\
\\
& \xrightarrow{E_1} CX_{2,1} \cdot CCX_{0,1} \cdot \overline{CX_{1,2} \cdot CX_{2,1}} \cdot r_7 \\
& \xrightarrow{C_9} CX_{2,1} \cdot CCX_{0,1} \cdot \overline{CX_{2,1} \cdot \sigma_{1,2}} \cdot \underline{r_7} \\
& \xrightarrow{D_7} CX_{2,1} \cdot CCX_{0,1} \cdot CX_{2,1} \cdot \sigma_{1,2} \cdot \overline{CZ_{0,1} \cdot CX_{2,1} \cdot CCX_{0,1} \cdot CX_{2,1} \cdot CZ_{0,1}} \\
& \xleftarrow{\delta_{15}} CX_{2,1} \cdot CCX_{0,1} \cdot CX_{2,1} \cdot \sigma_{1,2} \cdot CZ_{0,1} \cdot \overline{CZ_{0,2} \cdot CX_{2,1} \cdot CCX_{0,1} \cdot CX_{2,1}} \\
& \xleftarrow{E_{10}} CX_{2,1} \cdot CCX_{0,1} \cdot CX_{2,1} \cdot \sigma_{1,2} \cdot CZ_{0,1} \cdot \overline{\sigma_{1,2} \cdot \sigma_{1,2}} \cdot CZ_{0,2} \cdot CX_{2,1} \cdot CCX_{0,1} \cdot CX_{2,1} \\
\\
& \xleftarrow{(18)} CX_{2,1} \cdot CCX_{0,1} \cdot CX_{2,1} \cdot \overline{CZ_{0,2} \cdot \sigma_{1,2} \cdot CZ_{0,2}} \cdot CX_{2,1} \cdot CCX_{0,1} \cdot CX_{2,1} \\
& \xrightarrow{(18)} CX_{2,1} \cdot CCX_{0,1} \cdot CX_{2,1} \cdot CZ_{0,2} \cdot \sigma_{1,2} \cdot \overline{\sigma_{1,2} \cdot CZ_{0,1} \cdot \sigma_{1,2}} \cdot CX_{2,1} \cdot CCX_{0,1} \cdot CX_{2,1} \\
\\
& \xrightarrow{E_{10}} CX_{2,1} \cdot CCX_{0,1} \cdot CX_{2,1} \cdot CZ_{0,2} \cdot CZ_{0,1} \cdot \sigma_{1,2} \cdot CX_{2,1} \cdot CCX_{0,1} \cdot CX_{2,1} \\
& \xleftarrow{\delta_{14}} \overline{CZ_{0,1} \cdot CX_{2,1} \cdot CCX_{0,1} \cdot CX_{2,1} \cdot CZ_{0,1}} \cdot \sigma_{1,2} \cdot CX_{2,1} \cdot CCX_{0,1} \cdot CX_{2,1} \\
& \xleftarrow{D_7} \overline{r_7} \cdot \sigma_{1,2} \cdot CX_{2,1} \cdot CCX_{0,1} \cdot CX_{2,1} \\
& \xleftarrow{E_9} r_7 \cdot \overline{CX_{2,1} \cdot CX_{2,1} \cdot \sigma_{1,2}} \cdot CX_{2,1} \cdot CCX_{0,1} \cdot CX_{2,1} \\
\\
& \xleftarrow{C_9} r_7 \cdot CX_{2,1} \cdot \overline{CX_{1,2} \cdot CX_{2,1} \cdot CX_{2,1}} \cdot CCX_{0,1} \cdot CX_{2,1} \\
\\
& \xrightarrow{E_9} r_7 \cdot CX_{2,1} \cdot CX_{1,2} \cdot CCX_{0,1} \cdot CX_{2,1} \\
& \xleftarrow{(21)} r_7 \cdot CX_{2,1} \cdot \overline{X_0 \cdot X_0 \cdot CX_{1,2} \cdot CCX_{0,1}} \cdot CX_{2,1} \\
\\
& \xrightarrow{C_{56}} r_7 \cdot CX_{2,1} \cdot X_0 \cdot \overline{CCX_{0,1} \cdot X_0 \cdot CX_{2,1}} \\
\\
& \xleftarrow{B_1} r_7 \cdot \overline{CX_{2,1} \cdot X_0 \cdot CCX_{0,1} \cdot CX_{2,1} \cdot X_0} \xrightarrow{B_1} r_7 \cdot \overline{X_0 \cdot CX_{2,1} \cdot CCX_{0,1} \cdot CX_{2,1} \cdot X_0} \xleftarrow{D_2} r_7 \cdot \overline{r_2} \\
\\
\underline{r_2} \cdot r_7 \cdot r_2 \cdot r_7 & \xrightarrow{\delta_{16}} \overline{r_7 \cdot \underline{r_2} \cdot r_2 \cdot r_7} \xrightarrow{(2;2)} \underline{r_7 \cdot r_7} \xrightarrow{(7;7)} \varepsilon
\end{aligned}$$

### 1.7.21 Deriving the Coxeter Relation ( 2 ; 8 )

$$\begin{aligned}
(\delta_{17}) : CX_{2,1} \cdot r_8 & \xleftarrow{E_9} CX_{2,1} \cdot \underline{r_8} \cdot \overline{CX_{2,1} \cdot CX_{2,1}} \\
& \xrightarrow{D_8} CX_{2,1} \cdot \overline{K_{1,2} \cdot X_1 \cdot X_2 \cdot CZ_{0,2} \cdot CCX_{1,2} \cdot CZ_{0,2} \cdot X_2 \cdot X_1 \cdot K_{1,2}} \cdot CX_{2,1} \cdot CX_{2,1} \\
\\
& \xrightarrow{C_4} \overline{CX_{2,1} \cdot K_{1,2} \cdot X_1 \cdot X_2 \cdot CZ_{0,2} \cdot CCX_{1,2} \cdot CZ_{0,2} \cdot X_2 \cdot X_1 \cdot CX_{1,2} \cdot K_{1,2}} \cdot CX_{2,1}
\end{aligned}$$

$$\begin{aligned}
& \xrightarrow{C_{10}} \overline{K_{1,2} \cdot CX_{1,2}} \cdot X_1 \cdot X_2 \cdot CZ_{0,2} \cdot CCX_{1,2} \cdot CZ_{0,2} \cdot X_2 \cdot X_1 \cdot CX_{1,2} \cdot K_{1,2} \cdot CX_{2,1} \\
& \xrightarrow{C_{14}} K_{1,2} \cdot \overline{CX_{1,2}} \cdot X_1 \cdot X_2 \cdot CZ_{0,2} \cdot CCX_{1,2} \cdot CZ_{0,2} \cdot X_2 \cdot \overline{CX_{1,2} \cdot X_2 \cdot X_1} \cdot K_{1,2} \cdot CX_{2,1} \\
& \xrightarrow{C_{15}} K_{1,2} \cdot \overline{X_1 \cdot X_2 \cdot CX_{1,2}} \cdot X_2 \cdot CZ_{0,2} \cdot CCX_{1,2} \cdot CZ_{0,2} \cdot X_2 \cdot CX_{1,2} \cdot X_2 \cdot X_1 \cdot K_{1,2} \cdot CX_{2,1} \\
& \xrightarrow{C_{114}} K_{1,2} \cdot X_1 \cdot X_2 \cdot CX_{1,2} \cdot \overline{CZ_{0,2} \cdot Z_0 \cdot X_2} \cdot CCX_{1,2} \cdot \overline{CZ_{0,2} \cdot X_2} \cdot CX_{1,2} \cdot X_2 \cdot X_1 \cdot K_{1,2} \cdot CX_{2,1} \\
& \xleftarrow{C_{115}} K_{1,2} \cdot X_1 \cdot X_2 \cdot CX_{1,2} \cdot CZ_{0,2} \cdot Z_0 \cdot \overline{X_2 \cdot CCX_{1,2} \cdot X_2 \cdot Z_0 \cdot CZ_{0,2}} \cdot CX_{1,2} \cdot X_2 \cdot X_1 \cdot K_{1,2} \cdot CX_{2,1} \\
& \xrightarrow{C_{83}} K_{1,2} \cdot X_1 \cdot X_2 \cdot CX_{1,2} \cdot CZ_{0,2} \cdot Z_0 \cdot \overline{CCX_{1,2} \cdot CX_{1,0} \cdot X_2 \cdot X_2} \cdot Z_0 \cdot CZ_{0,2} \cdot CX_{1,2} \cdot X_2 \cdot X_1 \cdot K_{1,2} \cdot CX_{2,1} \\
& \xrightarrow{E_{17}} K_{1,2} \cdot X_1 \cdot X_2 \cdot CX_{1,2} \cdot CZ_{0,2} \cdot Z_0 \cdot \overline{CCX_{1,2} \cdot CX_{1,0} \cdot Z_0 \cdot CZ_{0,2}} \cdot CX_{1,2} \cdot X_2 \cdot X_1 \cdot K_{1,2} \cdot CX_{2,1} \\
& \xrightarrow{C_{49}} K_{1,2} \cdot X_1 \cdot X_2 \cdot CX_{1,2} \cdot CZ_{0,2} \cdot \overline{CCX_{1,2} \cdot CZ_{1,2} \cdot Z_0 \cdot CX_{1,0}} \cdot Z_0 \cdot CZ_{0,2} \cdot CX_{1,2} \cdot X_2 \cdot X_1 \cdot K_{1,2} \cdot CX_{2,1} \\
& \xrightarrow{C_{32}} K_{1,2} \cdot X_1 \cdot X_2 \cdot CX_{1,2} \cdot CZ_{0,2} \cdot CCX_{1,2} \cdot CZ_{1,2} \cdot \overline{CX_{1,0} \cdot Z_1 \cdot Z_0 \cdot Z_0} \cdot CZ_{0,2} \cdot CX_{1,2} \cdot X_2 \cdot X_1 \cdot K_{1,2} \cdot CX_{2,1} \\
& \xrightarrow{E_3} K_{1,2} \cdot X_1 \cdot X_2 \cdot \overline{CX_{1,2} \cdot CZ_{0,2}} \cdot CCX_{1,2} \cdot CZ_{1,2} \cdot CX_{1,0} \cdot Z_1 \cdot CZ_{0,2} \cdot CX_{1,2} \cdot X_2 \cdot X_1 \cdot K_{1,2} \cdot CX_{2,1} \\
& \xrightarrow{C_{51}} K_{1,2} \cdot X_1 \cdot X_2 \cdot \overline{CZ_{0,2} \cdot CZ_{0,1} \cdot CX_{1,2}} \cdot CCX_{1,2} \cdot CZ_{1,2} \cdot CX_{1,0} \cdot Z_1 \cdot CZ_{0,2} \cdot CX_{1,2} \cdot X_2 \cdot X_1 \cdot K_{1,2} \cdot CX_{2,1} \\
& \xleftarrow{C_{21}} K_{1,2} \cdot X_1 \cdot X_2 \cdot CZ_{0,2} \cdot \overline{CX_{1,2} \cdot CZ_{0,1} \cdot CCX_{1,2}} \cdot CZ_{1,2} \cdot CX_{1,0} \cdot Z_1 \cdot CZ_{0,2} \cdot CX_{1,2} \cdot X_2 \cdot X_1 \cdot K_{1,2} \cdot CX_{2,1} \\
& \xrightarrow{C_{77}} K_{1,2} \cdot X_1 \cdot X_2 \cdot CZ_{0,2} \cdot CX_{1,2} \cdot \overline{CCX_{1,2} \cdot CZ_{1,2} \cdot CZ_{0,1} \cdot CZ_{1,2}} \cdot CX_{1,0} \cdot Z_1 \cdot CZ_{0,2} \cdot CX_{1,2} \cdot X_2 \cdot X_1 \cdot K_{1,2} \cdot CX_{2,1} \\
& \xrightarrow{(40)} K_{1,2} \cdot X_1 \cdot X_2 \cdot CZ_{0,2} \cdot CX_{1,2} \cdot CCX_{1,2} \cdot \overline{CZ_{1,2} \cdot CZ_{1,2} \cdot CZ_{0,1}} \cdot CX_{1,0} \cdot Z_1 \cdot CZ_{0,2} \cdot CX_{1,2} \cdot X_2 \cdot X_1 \cdot K_{1,2} \cdot CX_{2,1} \\
& \xrightarrow{E_{12}} K_{1,2} \cdot X_1 \cdot X_2 \cdot CZ_{0,2} \cdot CX_{1,2} \cdot CCX_{1,2} \cdot CZ_{0,1} \cdot \overline{CX_{1,0} \cdot Z_1} \cdot CZ_{0,2} \cdot CX_{1,2} \cdot X_2 \cdot X_1 \cdot K_{1,2} \cdot CX_{2,1} \\
& \xrightarrow{C_{48}} K_{1,2} \cdot X_1 \cdot X_2 \cdot CZ_{0,2} \cdot CX_{1,2} \cdot CCX_{1,2} \cdot \overline{CZ_{0,1} \cdot Z_1 \cdot CX_{1,0}} \cdot CZ_{0,2} \cdot CX_{1,2} \cdot X_2 \cdot X_1 \cdot K_{1,2} \cdot CX_{2,1} \\
& \xrightarrow{C_{62}} K_{1,2} \cdot X_1 \cdot X_2 \cdot CZ_{0,2} \cdot CX_{1,2} \cdot CCX_{1,2} \cdot \overline{CX_{1,0} \cdot CZ_{0,1}} \cdot \overline{CZ_{0,2} \cdot CX_{1,2}} \cdot X_2 \cdot X_1 \cdot K_{1,2} \cdot CX_{2,1} \\
& \xrightarrow{C_{102}} K_{1,2} \cdot X_1 \cdot X_2 \cdot CZ_{0,2} \cdot CX_{1,2} \cdot CCX_{1,2} \cdot CX_{1,0} \cdot CZ_{0,1} \cdot \overline{CX_{1,2} \cdot CZ_{0,1} \cdot CZ_{0,2}} \cdot X_2 \cdot X_1 \cdot K_{1,2} \cdot CX_{2,1} \\
& \xrightarrow{C_{21}} K_{1,2} \cdot X_1 \cdot X_2 \cdot CZ_{0,2} \cdot CX_{1,2} \cdot CCX_{1,2} \cdot CX_{1,0} \cdot \overline{CZ_{0,1} \cdot CZ_{0,1}} \cdot \overline{CX_{1,2}} \cdot CZ_{0,2} \cdot X_2 \cdot X_1 \cdot K_{1,2} \cdot CX_{2,1} \\
& \xrightarrow{E_2} K_{1,2} \cdot X_1 \cdot X_2 \cdot CZ_{0,2} \cdot \overline{CX_{1,2} \cdot CCX_{1,2}} \cdot CX_{1,0} \cdot CX_{1,2} \cdot CZ_{0,2} \cdot X_2 \cdot X_1 \cdot K_{1,2} \cdot CX_{2,1} \\
& \xrightarrow{(44)} K_{1,2} \cdot X_1 \cdot X_2 \cdot CZ_{0,2} \cdot \overline{CCX_{1,2} \cdot CX_{1,0} \cdot CX_{1,2}} \cdot CX_{1,0} \cdot CX_{1,2} \cdot CZ_{0,2} \cdot X_2 \cdot X_1 \cdot K_{1,2} \cdot CX_{2,1} \\
& \xrightarrow{C_{94}} K_{1,2} \cdot X_1 \cdot X_2 \cdot CZ_{0,2} \cdot CCX_{1,2} \cdot \overline{CX_{1,2} \cdot CX_{1,0} \cdot CX_{1,0}} \cdot CX_{1,2} \cdot CZ_{0,2} \cdot X_2 \cdot X_1 \cdot K_{1,2} \cdot CX_{2,1} \\
& \xrightarrow{E_1} K_{1,2} \cdot X_1 \cdot X_2 \cdot CZ_{0,2} \cdot CCX_{1,2} \cdot \overline{CX_{1,2} \cdot CX_{1,2}} \cdot CZ_{0,2} \cdot X_2 \cdot X_1 \cdot K_{1,2} \cdot CX_{2,1} \\
& \xrightarrow{E_8} \overline{K_{1,2} \cdot X_1 \cdot X_2 \cdot CZ_{0,2} \cdot CCX_{1,2} \cdot CZ_{0,2} \cdot X_2 \cdot X_1 \cdot K_{1,2} \cdot CX_{2,1}} \xleftarrow{D_8} \overline{r_8} \cdot CX_{2,1}
\end{aligned}$$

$$\begin{aligned}
(2; 8) : r_2 \cdot r_8 \cdot \underline{r_2} \cdot r_8 & \xrightarrow{D_2} \underline{r_2} \cdot r_8 \cdot \overline{X_0 \cdot CX_{2,1} \cdot CCX_{0,1} \cdot CX_{2,1} \cdot X_0} \cdot r_8 \\
& \xrightarrow{D_2} \overline{X_0 \cdot CX_{2,1} \cdot CCX_{0,1} \cdot CX_{2,1} \cdot X_0} \cdot r_8 \cdot X_0 \cdot CX_{2,1} \cdot CCX_{0,1} \cdot CX_{2,1} \cdot \underline{X_0} \cdot r_8 \\
& \xrightarrow{\xi_4} X_0 \cdot CX_{2,1} \cdot CCX_{0,1} \cdot CX_{2,1} \cdot \underline{X_0} \cdot r_8 \cdot X_0 \cdot CX_{2,1} \cdot CCX_{0,1} \cdot CX_{2,1} \cdot \overline{X_0} \\
& \xrightarrow{\xi_4} X_0 \cdot CX_{2,1} \cdot CCX_{0,1} \cdot CX_{2,1} \cdot \overline{r_8 \cdot X_0} \cdot X_0 \cdot CX_{2,1} \cdot CCX_{0,1} \cdot CX_{2,1} \cdot r_8 \cdot X_0 \\
& \xrightarrow{(21)} X_0 \cdot CX_{2,1} \cdot CCX_{0,1} \cdot CX_{2,1} \cdot r_8 \cdot CX_{2,1} \cdot CCX_{0,1} \cdot \overline{CX_{2,1} \cdot r_8} \cdot X_0 \\
& \xrightarrow{\delta_{17}} X_0 \cdot CX_{2,1} \cdot CCX_{0,1} \cdot \overline{CX_{2,1} \cdot r_8} \cdot CX_{2,1} \cdot CCX_{0,1} \cdot \overline{r_8 \cdot CX_{2,1}} \cdot X_0 \\
& \xrightarrow{\delta_{17}} X_0 \cdot CX_{2,1} \cdot CCX_{0,1} \cdot \overline{r_8 \cdot CX_{2,1}} \cdot \overline{CX_{2,1}} \cdot CCX_{0,1} \cdot r_8 \cdot CX_{2,1} \cdot X_0
\end{aligned}$$

$$\begin{aligned}
& \xrightarrow{E_9} X_0 \cdot CX_{2,1} \cdot CCX_{0,1} \cdot r_8 \cdot \overline{CCX_{0,1} \cdot r_8} \cdot CX_{2,1} \cdot X_0 \\
& \xrightarrow{\xi_8} X_0 \cdot CX_{2,1} \cdot CCX_{0,1} \cdot \overline{r_8 \cdot r_8} \cdot \overline{CCX_{0,1}} \cdot CX_{2,1} \cdot X_0 \\
& \xrightarrow{(8,8)} X_0 \cdot CX_{2,1} \cdot \overline{CCX_{0,1} \cdot CCX_{0,1}} \cdot CX_{2,1} \cdot X_0 \\
& \xrightarrow{E_{18}} X_0 \cdot \overline{CX_{2,1} \cdot CX_{2,1}} \cdot X_0 \xrightarrow{E_9} \overline{X_0 \cdot X_0} \xrightarrow{(21)} \varepsilon
\end{aligned}$$

### 1.7.22 Deriving the Coxeter Relation ( 3 ; 4 )

$$\begin{aligned}
(\delta_{18}) : r_3 \cdot r_4 & \xrightarrow{D_3} \overline{X_0 \cdot CCX_{0,1} \cdot X_0} \cdot r_4 \xleftarrow{\chi_2} \overline{CX_{1,0} \cdot CCX_{0,1} \cdot CX_{1,0}} \cdot r_4 \xrightarrow{C_{72}} \overline{CCX_{0,1} \cdot CX_{1,2} \cdot CX_{1,0}} \cdot CX_{1,0} \cdot r_4 \\
& \xrightarrow{E_1} \overline{CCX_{0,1} \cdot CX_{1,2} \cdot r_4} \\
& \xrightarrow{D_4} \overline{CCX_{0,1} \cdot CX_{1,2} \cdot \overline{CX_{0,1} \cdot CX_{0,2}} \cdot CCX_{1,2} \cdot CX_{0,2} \cdot CX_{0,1}} \\
& \xleftarrow{C_{17}} \overline{CCX_{0,1} \cdot \overline{CX_{0,1}} \cdot CX_{1,2} \cdot CCX_{1,2} \cdot CX_{0,2} \cdot CX_{0,1}} \\
& \xrightarrow{C_{122}} \overline{CX_{0,1} \cdot CX_{0,2} \cdot \overline{CCX_{0,1} \cdot CX_{1,2}} \cdot CCX_{1,2} \cdot CX_{0,2} \cdot CX_{0,1}} \\
& \xrightarrow{C_{107}} \overline{CX_{0,1} \cdot CX_{0,2} \cdot \overline{CX_{1,2} \cdot CCX_{0,1}} \cdot CCX_{1,2} \cdot CX_{0,2} \cdot CX_{0,1}} \\
& \xleftarrow{C_{33}} \overline{CX_{0,1} \cdot \overline{CX_{1,2} \cdot CX_{0,2}} \cdot \overline{CCX_{0,1}} \cdot CCX_{1,2} \cdot CX_{0,2} \cdot CX_{0,1}} \\
& \xleftarrow{C_{105}} \overline{CX_{0,1} \cdot CX_{1,2} \cdot \overline{CCX_{0,1} \cdot CX_{0,2}} \cdot \overline{CCX_{1,2} \cdot CX_{0,2}} \cdot CX_{0,1}} \\
& \xrightarrow{\chi_4} \overline{CX_{0,1} \cdot CX_{1,2} \cdot \overline{CCX_{0,1} \cdot \overline{CCX_{0,1}} \cdot \overline{CCX_{1,2} \cdot CCX_{0,1}}} \cdot CX_{0,1}} \\
& \xrightarrow{E_{18}} \overline{CX_{0,1} \cdot CX_{1,2} \cdot CCX_{1,2} \cdot CCX_{0,1} \cdot CX_{0,1}} \\
\\
r_3 \cdot r_4 \cdot r_3 \cdot r_4 \cdot \overline{r_3 \cdot r_4} & \xrightarrow{\delta_{18}} r_3 \cdot r_4 \cdot r_3 \cdot r_4 \cdot \overline{CX_{0,1} \cdot CX_{1,2} \cdot \overline{CCX_{1,2} \cdot CCX_{0,1} \cdot CX_{0,1}}} \\
& \xrightarrow{\delta_{18}} r_3 \cdot r_4 \cdot \overline{CX_{0,1} \cdot CX_{1,2} \cdot \overline{CCX_{1,2} \cdot CCX_{0,1} \cdot CX_{0,1}}} \cdot \overline{CX_{0,1} \cdot CX_{0,1}} \cdot CX_{1,2} \cdot \overline{CCX_{1,2} \cdot CCX_{0,1} \cdot CX_{0,1}} \\
& \xrightarrow{(22)} r_3 \cdot r_4 \cdot \overline{CX_{0,1} \cdot CX_{1,2} \cdot \overline{CCX_{1,2} \cdot CCX_{0,1} \cdot CX_{1,2} \cdot \overline{CCX_{1,2} \cdot CCX_{0,1} \cdot CX_{0,1}}}} \\
& \xrightarrow{(44)} r_3 \cdot r_4 \cdot \overline{CX_{0,1} \cdot \overline{CCX_{1,2} \cdot CX_{1,0} \cdot CX_{1,2}} \cdot \overline{CCX_{0,1} \cdot CX_{1,2}} \cdot \overline{CCX_{1,2} \cdot CCX_{0,1} \cdot CX_{0,1}}} \\
& \xrightarrow{C_{107}} r_3 \cdot r_4 \cdot \overline{CX_{0,1} \cdot \overline{CCX_{1,2} \cdot CX_{1,0} \cdot CX_{1,2} \cdot \overline{CX_{1,2} \cdot \overline{CCX_{0,1}} \cdot CCX_{1,2} \cdot CCX_{0,1} \cdot CX_{0,1}}}} \\
& \xrightarrow{E_8} r_3 \cdot r_4 \cdot \overline{CX_{0,1} \cdot \overline{CCX_{1,2} \cdot CX_{1,0} \cdot CCX_{0,1} \cdot \overline{CCX_{1,2} \cdot CCX_{0,1} \cdot CX_{0,1}}}} \\
& \xrightarrow{C_{98}} r_3 \cdot r_4 \cdot \overline{CX_{0,1} \cdot \overline{CX_{1,0} \cdot \overline{CCX_{1,2}} \cdot \overline{CCX_{0,1} \cdot CCX_{1,2} \cdot CCX_{0,1}}} \cdot CX_{0,1}} \\
& \xrightarrow{\chi_{11}} r_3 \cdot r_4 \cdot \overline{CX_{0,1} \cdot CX_{1,0} \cdot \overline{CCX_{1,2} \cdot \overline{CCX_{1,2}} \cdot CCX_{0,1} \cdot \overline{CCX_{1,2} \cdot CX_{0,1}}}} \\
& \xrightarrow{(24)} r_3 \cdot r_4 \cdot \overline{CX_{0,1} \cdot CX_{1,0} \cdot \overline{CCX_{0,1} \cdot \overline{CCX_{1,2} \cdot CX_{0,1}}}} \\
& \xrightarrow{\delta_{18}} \overline{CX_{0,1} \cdot CX_{1,2} \cdot \overline{CCX_{1,2} \cdot CCX_{0,1} \cdot CX_{0,1}} \cdot CX_{0,1} \cdot CX_{1,0} \cdot \overline{CCX_{0,1} \cdot \overline{CCX_{1,2} \cdot CX_{0,1}}}} \\
& \xrightarrow{(22)} \overline{CX_{0,1} \cdot CX_{1,2} \cdot \overline{CCX_{1,2} \cdot CCX_{0,1} \cdot CX_{1,0} \cdot \overline{CCX_{0,1} \cdot \overline{CCX_{1,2} \cdot CX_{0,1}}}} \\
& \xleftarrow{E_1} \overline{CX_{0,1} \cdot CX_{1,2} \cdot \overline{CCX_{1,2} \cdot \overline{CX_{1,0} \cdot \overline{CCX_{0,1}} \cdot CX_{1,0} \cdot \overline{CCX_{0,1} \cdot \overline{CCX_{1,2} \cdot CX_{0,1}}}} \\
& \xrightarrow{C_{72}} \overline{CX_{0,1} \cdot CX_{1,2} \cdot \overline{CCX_{1,2} \cdot CX_{1,0} \cdot \overline{CCX_{0,1} \cdot \overline{CX_{1,2} \cdot \overline{CX_{1,0} \cdot CX_{1,0} \cdot \overline{CCX_{0,1} \cdot \overline{CCX_{1,2} \cdot CX_{0,1}}}}}}
\end{aligned}$$

$$\begin{aligned}
& \xrightarrow{E_1} CX_{0,1} \cdot CX_{1,2} \cdot CCX_{1,2} \cdot CX_{1,0} \cdot \overline{CCX_{0,1} \cdot CX_{1,2}} \cdot CCX_{0,1} \cdot CCX_{1,2} \cdot CX_{0,1} \\
& \xrightarrow{C_{107}} CX_{0,1} \cdot CX_{1,2} \cdot CCX_{1,2} \cdot \overline{CX_{1,0} \cdot \overline{CX_{1,2}} \cdot CCX_{0,1}} \cdot CCX_{0,1} \cdot CCX_{1,2} \cdot CX_{0,1} \\
& \xrightarrow{C_{94}} CX_{0,1} \cdot CX_{1,2} \cdot CCX_{1,2} \cdot \overline{CX_{1,2} \cdot CX_{1,0}} \cdot \overline{CCX_{0,1} \cdot CCX_{0,1}} \cdot CCX_{1,2} \cdot CX_{0,1} \\
& \xrightarrow{E_{18}} CX_{0,1} \cdot \overline{CX_{1,2} \cdot CCX_{1,2}} \cdot CX_{1,2} \cdot CX_{1,0} \cdot CCX_{1,2} \cdot CX_{0,1} \\
& \xrightarrow{(44)} CX_{0,1} \cdot \overline{CCX_{1,2} \cdot CX_{1,0} \cdot \overline{CX_{1,2}} \cdot CX_{1,2}} \cdot CX_{1,0} \cdot CCX_{1,2} \cdot CX_{0,1} \\
& \xrightarrow{E_8} CX_{0,1} \cdot CCX_{1,2} \cdot \overline{CX_{1,0} \cdot CX_{1,0}} \cdot CCX_{1,2} \cdot CX_{0,1} \xrightarrow{E_1} CX_{0,1} \cdot \overline{CCX_{1,2} \cdot CCX_{1,2}} \cdot CX_{0,1} \xrightarrow{(24)} \overline{CX_{0,1} \cdot CX_{0,1}} \xrightarrow{(22)} \varepsilon
\end{aligned}$$

### 1.7.23 Deriving the Coxeter Relation ( 3 ; 5 )

$$\begin{aligned}
(\delta_{19}) : r_3 \cdot r_5 & \xrightarrow{D_3} \overline{X_0 \cdot CCX_{0,1} \cdot X_0} \cdot r_5 \xleftarrow{X_2} \overline{CX_{1,0} \cdot CCX_{0,1} \cdot CX_{1,0}} \cdot r_5 \xrightarrow{C_{72}} \overline{CCX_{0,1} \cdot CX_{1,2} \cdot CX_{1,0}} \cdot r_5 \\
& \xrightarrow{E_1} \overline{CCX_{0,1} \cdot CX_{1,2} \cdot r_5} \\
& \xrightarrow{D_6} \overline{CCX_{0,1} \cdot CX_{1,2} \cdot \overline{X_1 \cdot CCX_{0,1} \cdot X_1}} \\
& \xleftarrow{X_3} \overline{CCX_{0,1} \cdot CX_{1,2} \cdot \overline{CX_{0,1} \cdot \overline{CCX_{0,1} \cdot CX_{0,1}}}} \\
& \xrightarrow{C_{122}} \overline{CCX_{0,1} \cdot CX_{1,2} \cdot \overline{CX_{0,1} \cdot \overline{CX_{0,2} \cdot CCX_{0,1}}}} \\
& \xrightarrow{(22)} \overline{CCX_{0,1} \cdot \overline{CX_{1,2} \cdot CX_{0,2} \cdot CCX_{0,1}}} \\
& \xrightarrow{C_{33}} \overline{CCX_{0,1} \cdot \overline{CX_{0,2} \cdot CX_{1,2} \cdot CCX_{0,1}}} \\
& \xleftarrow{(22)} \overline{CCX_{0,1} \cdot \overline{CX_{0,2} \cdot \overline{CX_{0,1} \cdot CX_{1,2} \cdot CCX_{0,1}}}} \\
& \xleftarrow{C_{119}} \overline{\overline{CX_{0,1} \cdot \overline{CCX_{0,1} \cdot CX_{0,1} \cdot CX_{1,2} \cdot CCX_{0,1}}}} \\
& \xrightarrow{X_3} \overline{\overline{X_1 \cdot \overline{CCX_{0,1} \cdot X_1} \cdot CX_{1,2} \cdot CCX_{0,1}}} \\
& \xleftarrow{D_6} \overline{\overline{r_5 \cdot \overline{CX_{1,2} \cdot CCX_{0,1}}}} \\
& \xleftarrow{C_{107}} \overline{\overline{r_5 \cdot \overline{CCX_{0,1} \cdot CX_{1,2}}}} \\
& \xleftarrow{E_1} \overline{\overline{r_5 \cdot \overline{CCX_{0,1} \cdot CX_{1,2} \cdot \overline{CX_{1,0} \cdot CX_{1,0}}}}} \\
& \xleftarrow{C_{72}} \overline{\overline{r_5 \cdot \overline{CX_{1,0} \cdot \overline{CCX_{0,1} \cdot CX_{1,0}}}}} \xrightarrow{X_2} \overline{\overline{r_5 \cdot \overline{X_0 \cdot \overline{CCX_{0,1} \cdot X_0}}}} \xleftarrow{D_3} \overline{\overline{r_5 \cdot \overline{r_3}}} \\
& \xrightarrow{\delta_{19}} \overline{\overline{r_3 \cdot \overline{r_5} \cdot r_3 \cdot r_5}} \xrightarrow{(3;3)} \overline{\overline{r_5 \cdot \overline{r_3} \cdot r_3 \cdot r_5}} \xrightarrow{(5;5)} \varepsilon
\end{aligned}$$

### 1.7.24 Deriving the Coxeter Relation ( 3 ; 6 )

$$\begin{aligned}
(\delta_{20}) : r_3 \cdot r_6 & \xrightarrow{D_6} \overline{r_3 \cdot \overline{CX_{2,1} \cdot CCX_{0,1} \cdot CX_{2,1}}} \xrightarrow{D_3} \overline{\overline{X_0 \cdot \overline{CCX_{0,1} \cdot X_0} \cdot CX_{2,1} \cdot CCX_{0,1} \cdot CX_{2,1}}} \\
& \xleftarrow{X_2} \overline{\overline{CX_{1,0} \cdot \overline{CCX_{0,1} \cdot CX_{1,0}} \cdot CX_{2,1} \cdot CCX_{0,1} \cdot CX_{2,1}}} \\
& \xrightarrow{C_{72}} \overline{\overline{CCX_{0,1} \cdot \overline{CX_{1,2} \cdot \overline{CX_{1,0} \cdot CX_{1,0}} \cdot CX_{2,1} \cdot CCX_{0,1} \cdot CX_{2,1}}} \\
& \xrightarrow{E_1} \overline{\overline{CCX_{0,1} \cdot \overline{CX_{1,2} \cdot \overline{CX_{2,1} \cdot \overline{CCX_{0,1} \cdot CX_{2,1}}}}} \\
& \xrightarrow{X_{10}} \overline{\overline{CCX_{0,1} \cdot \overline{CX_{1,2} \cdot \overline{CX_{1,2} \cdot \overline{CCX_{0,2} \cdot CX_{1,2}}}}} \\
& \xrightarrow{E_8} \overline{\overline{CCX_{0,1} \cdot \overline{CCX_{0,2} \cdot CX_{1,2}}}
\end{aligned}$$

$$\begin{aligned}
& \xleftarrow{E_{18}} \overline{CCX_{0,1} \cdot CCX_{0,2} \cdot \overline{CCX_{0,1} \cdot CCX_{0,1}} \cdot CX_{1,2}} \\
& \xleftarrow{\chi_9} \overline{CCX_{0,2} \cdot CCX_{0,1} \cdot \overline{CCX_{0,2}} \cdot CCX_{0,1} \cdot CX_{1,2}} \\
& \xleftarrow{\chi_6} \overline{CX_{2,1} \cdot \overline{CCX_{0,1} \cdot CX_{2,1}} \cdot CCX_{0,1} \cdot CX_{1,2}} \\
& \xleftarrow{E_1} CX_{2,1} \cdot CCX_{0,1} \cdot CX_{2,1} \cdot \overline{CCX_{0,1} \cdot CX_{1,2} \cdot \overline{CX_{1,0}} \cdot CX_{1,0}} \\
& \xleftarrow{C_{72}} CX_{2,1} \cdot CCX_{0,1} \cdot CX_{2,1} \cdot \overline{CX_{1,0} \cdot \overline{CCX_{0,1}} \cdot CX_{1,0}} \\
& \xrightarrow{\chi_2} \overline{CX_{2,1} \cdot CCX_{0,1} \cdot CX_{2,1} \cdot \overline{X_0 \cdot CCX_{0,1} \cdot X_0}} \xleftarrow{D_6} \overline{r_6 \cdot X_0 \cdot CCX_{0,1} \cdot X_0} \xleftarrow{D_3} r_6 \cdot \overline{r_3} \\
(3;6) : & \underline{r_3 \cdot r_6} \cdot r_3 \cdot r_6 \xrightarrow{\delta_{20}} \overline{r_6 \cdot \underline{r_3} \cdot r_3} \cdot r_6 \xrightarrow{(3;3)} \underline{r_6 \cdot r_6} \xrightarrow{(6;6)} \varepsilon
\end{aligned}$$

### 1.7.25 Deriving the Coxeter Relation ( 3 ; 7 )

$$\begin{aligned}
(\delta_{21}) : & CZ_{0,1} \cdot \underline{r_3} \xrightarrow{D_3} \overline{CZ_{0,1} \cdot \overline{X_0 \cdot CCX_{0,1}} \cdot X_0} \\
& \xleftarrow{C_{69}} \overline{X_0 \cdot \underline{Z_1} \cdot \overline{CZ_{0,1}} \cdot CCX_{0,1} \cdot X_0} \\
& \xrightarrow{C_{95}} X_0 \cdot \underline{Z_1} \cdot \overline{CCX_{0,1} \cdot \overline{CZ_{0,1}} \cdot X_0} \\
& \xleftarrow{C_{69}} X_0 \cdot \underline{Z_1} \cdot CCX_{0,1} \cdot \overline{X_0 \cdot \underline{Z_1} \cdot CZ_{0,1}} \\
& \xrightarrow{B_{14}} X_0 \cdot \underline{Z_1} \cdot \overline{CCX_{0,1} \cdot \underline{Z_1} \cdot X_0} \cdot CZ_{0,1} \\
& \xrightarrow{C_{47}} X_0 \cdot \overline{CCX_{0,1} \cdot \underline{Z_1} \cdot Z_1} \cdot X_0 \cdot CZ_{0,1} \\
& \xrightarrow{E_5} X_0 \cdot \overline{CCX_{0,1} \cdot X_0} \cdot CZ_{0,1} \xleftarrow{D_3} \overline{r_3 \cdot CZ_{0,1}} \\
& r_3 \cdot r_7 \cdot r_3 \cdot \underline{r_7} \xrightarrow{\xi_3} r_3 \cdot \underline{r_7} \cdot r_3 \cdot \overline{CZ_{0,1} \cdot r_6 \cdot CZ_{0,1}} \\
& \xrightarrow{\xi_3} r_3 \cdot \overline{CZ_{0,1} \cdot r_6 \cdot \overline{CZ_{0,1}}} \cdot r_3 \cdot CZ_{0,1} \cdot r_6 \cdot CZ_{0,1} \\
& \xrightarrow{\delta_{21}} r_3 \cdot CZ_{0,1} \cdot r_6 \cdot \overline{r_3 \cdot \overline{CZ_{0,1}}} \cdot CZ_{0,1} \cdot r_6 \cdot CZ_{0,1} \\
& \xleftarrow{\delta_{21}} \overline{CZ_{0,1} \cdot r_3 \cdot r_6 \cdot r_3 \cdot \overline{CZ_{0,1} \cdot CZ_{0,1}}} \cdot r_6 \cdot CZ_{0,1} \\
& \xrightarrow{E_2} CZ_{0,1} \cdot \underline{r_3 \cdot r_6 \cdot r_3 \cdot r_6} \cdot CZ_{0,1} \\
& \xrightarrow{(3;6)} \underline{CZ_{0,1} \cdot CZ_{0,1}} \\
& \xrightarrow{E_2} \varepsilon
\end{aligned}$$

### 1.7.26 Deriving the Coxeter Relation ( 3 ; 8 )

$$\begin{aligned}
(\delta_{22}) : & r_3 \xleftarrow{E_{13}} \underline{r_3} \cdot \overline{X_1 \cdot X_1} \\
& \xrightarrow{D_3} \overline{X_0 \cdot CCX_{0,1} \cdot X_0} \cdot X_1 \cdot X_1 \\
& \xleftarrow{E_{13}} \overline{X_1 \cdot \underline{X_1} \cdot X_0} \cdot CCX_{0,1} \cdot X_0 \cdot X_1 \cdot X_1 \\
& \xleftarrow{B_2} X_1 \cdot \overline{X_0 \cdot X_1} \cdot CCX_{0,1} \cdot \underline{X_0 \cdot X_1} \cdot X_1 \\
& \xrightarrow{B_2} X_1 \cdot \underline{X_0 \cdot X_1} \cdot \overline{CCX_{0,1} \cdot \overline{X_1 \cdot X_0}} \cdot X_1 \xleftarrow{D_1} X_1 \cdot \overline{r_1} \cdot X_1 \\
& r_3 \cdot r_8 \cdot \underline{r_3} \cdot r_8 \xrightarrow{\delta_{22}} \underline{r_3} \cdot r_8 \cdot \overline{X_1 \cdot r_1 \cdot X_1} \cdot r_8 \\
& \xrightarrow{\delta_{22}} \overline{X_1 \cdot r_1 \cdot X_1} \cdot r_8 \cdot X_1 \cdot r_1 \cdot \underline{X_1 \cdot r_8} \\
& \xrightarrow{\xi_7} X_1 \cdot r_1 \cdot \underline{X_1 \cdot r_8} \cdot X_1 \cdot r_1 \cdot \overline{r_8 \cdot X_1} \\
& \xrightarrow{\xi_7} X_1 \cdot r_1 \cdot \overline{r_8 \cdot X_1} \cdot X_1 \cdot r_1 \cdot r_8 \cdot X_1 \\
& \xrightarrow{E_{13}} X_1 \cdot \underline{r_1 \cdot r_8 \cdot r_1 \cdot r_8} \cdot X_1 \xrightarrow{(1;8)} \underline{X_1 \cdot X_1} \xrightarrow{E_{13}} \varepsilon
\end{aligned}$$

### 1.7.27 Deriving the Coxeter Relation ( 4 ; 5 )

$$\begin{aligned}
& r_4 \cdot r_5 \cdot r_4 \cdot r_5 \cdot \underline{r_4 \cdot r_5} \xrightarrow{\omega_8} r_4 \cdot r_5 \cdot \underline{r_4 \cdot r_5} \cdot \overline{CX_{0,1} \cdot CCX_{0,1} \cdot \overline{CCX_{1,2}} \cdot CX_{0,1}} \\
& \xrightarrow{\omega_8} r_4 \cdot r_5 \cdot \overline{CX_{0,1} \cdot CCX_{0,1} \cdot \overline{CCX_{1,2}} \cdot CX_{0,1}} \cdot CX_{0,1} \cdot CCX_{0,1} \cdot \overline{CCX_{1,2}} \cdot CX_{0,1} \\
& \xrightarrow{(22)} r_4 \cdot r_5 \cdot CX_{0,1} \cdot \overline{CCX_{0,1} \cdot \overline{CCX_{1,2}} \cdot \overline{CCX_{0,1}} \cdot CCX_{1,2}} \cdot CX_{0,1} \\
& \xrightarrow{\chi_{11}} r_4 \cdot r_5 \cdot CX_{0,1} \cdot \overline{CCX_{1,2} \cdot \overline{CCX_{0,1}} \cdot \overline{CCX_{1,2}} \cdot CCX_{1,2}} \cdot CX_{0,1}
\end{aligned}$$

$$\begin{aligned}
& \xrightarrow{(24)} r_4 \cdot r_5 \cdot CX_{0,1} \cdot CCX_{1,2} \cdot CCX_{0,1} \cdot CX_{0,1} \\
& \xrightarrow{\omega_8} \overline{CX_{0,1} \cdot CCX_{0,1} \cdot CCX_{1,2} \cdot CX_{0,1} \cdot CCX_{1,2} \cdot CCX_{0,1} \cdot CX_{0,1}} \\
& \xrightarrow{(22)} CX_{0,1} \cdot CCX_{0,1} \cdot \overline{CCX_{1,2} \cdot CCX_{1,2} \cdot CCX_{0,1} \cdot CX_{0,1}} \\
& \xrightarrow{(24)} CX_{0,1} \cdot \overline{CCX_{0,1} \cdot CCX_{0,1} \cdot CX_{0,1}} \xrightarrow{E_{18}} \overline{CX_{0,1} \cdot CX_{0,1}} \xrightarrow{(22)} \varepsilon
\end{aligned}$$

### 1.7.28 Deriving the Coxeter Relation ( 4 ; 6 )

$$\begin{aligned}
(\delta_{23}) : CCX_{0,1} \cdot CCX_{0,2} \cdot CCX_{0,1} \cdot CX_{0,1} & \xleftarrow{E_{15}} \overline{CX_{0,2} \cdot CX_{0,2} \cdot CCX_{0,1} \cdot CCX_{0,2} \cdot CCX_{0,1} \cdot CX_{0,1}} \\
& \xleftarrow{C_{105}} CX_{0,2} \cdot \overline{CCX_{0,1} \cdot CX_{0,2} \cdot CCX_{0,2} \cdot CCX_{0,1} \cdot CX_{0,1}} \\
& \xrightarrow{C_{34}} CX_{0,2} \cdot CCX_{0,1} \cdot \overline{CCX_{0,2} \cdot CX_{0,1} \cdot CX_{0,2} \cdot CCX_{0,1} \cdot CX_{0,1}} \\
& \xleftarrow{C_{105}} CX_{0,2} \cdot CCX_{0,1} \cdot CCX_{0,2} \cdot CX_{0,1} \cdot \overline{CCX_{0,1} \cdot CX_{0,2} \cdot CX_{0,1}} \\
& \xleftarrow{C_{22}} CX_{0,2} \cdot CCX_{0,1} \cdot CCX_{0,2} \cdot \overline{CX_{0,1} \cdot CCX_{0,1} \cdot CX_{0,1} \cdot CX_{0,2}} \\
& \xrightarrow{C_{119}} CX_{0,2} \cdot CCX_{0,1} \cdot CCX_{0,2} \cdot \overline{CCX_{0,1} \cdot CX_{0,2} \cdot CX_{0,1} \cdot CX_{0,1}} \cdot CX_{0,2} \\
& \xrightarrow{(22)} CX_{0,2} \cdot CCX_{0,1} \cdot CCX_{0,2} \cdot CCX_{0,1} \cdot \overline{CX_{0,2} \cdot CX_{0,2}} \xrightarrow{E_{15}} CX_{0,2} \cdot CCX_{0,1} \cdot CCX_{0,2} \cdot CCX_{0,1}
\end{aligned}$$

$$\begin{aligned}
(\delta_{24}) : CCX_{0,2} \cdot CCX_{0,1} \cdot CCX_{0,2} \cdot CX_{0,2} & \xleftarrow{(22)} \overline{CX_{0,1} \cdot CX_{0,1} \cdot CCX_{0,2} \cdot CCX_{0,1} \cdot CCX_{0,2} \cdot CX_{0,2}} \\
& \xleftarrow{C_{89}} CX_{0,1} \cdot \overline{CCX_{0,2} \cdot CX_{0,1} \cdot CCX_{0,1} \cdot CCX_{0,2} \cdot CX_{0,2}} \\
& \xrightarrow{C_{119}} CX_{0,1} \cdot CCX_{0,2} \cdot \overline{CCX_{0,1} \cdot CX_{0,2} \cdot CX_{0,1} \cdot CCX_{0,2} \cdot CX_{0,2}} \\
& \xleftarrow{C_{89}} CX_{0,1} \cdot CCX_{0,2} \cdot CCX_{0,1} \cdot \overline{CX_{0,2} \cdot CCX_{0,2} \cdot CX_{0,1} \cdot CX_{0,2}} \\
& \xrightarrow{C_{34}} CX_{0,1} \cdot CCX_{0,2} \cdot CCX_{0,1} \cdot \overline{CCX_{0,2} \cdot CX_{0,1} \cdot CX_{0,2} \cdot CX_{0,1} \cdot CX_{0,2}} \\
& \xrightarrow{C_{22}} CX_{0,1} \cdot CCX_{0,2} \cdot CCX_{0,1} \cdot CCX_{0,2} \cdot \overline{CX_{0,2} \cdot CX_{0,1} \cdot CX_{0,1} \cdot CX_{0,2}} \\
& \xrightarrow{(22)} CX_{0,1} \cdot CCX_{0,2} \cdot CCX_{0,1} \cdot CCX_{0,2} \cdot \overline{CX_{0,2} \cdot CX_{0,2}} \xrightarrow{E_{15}} CX_{0,1} \cdot CCX_{0,2} \cdot CCX_{0,1} \cdot CCX_{0,2}
\end{aligned}$$

$$\begin{aligned}
(\delta_{25}) : r_4 \cdot r_6 & \xrightarrow{D_6} r_4 \cdot \overline{CX_{2,1} \cdot CCX_{0,1} \cdot CX_{2,1}} \xrightarrow{D_4} \overline{CX_{0,1} \cdot CX_{0,2} \cdot CCX_{1,2} \cdot CX_{0,2} \cdot CX_{0,1} \cdot CX_{2,1} \cdot CCX_{0,1} \cdot CX_{2,1}} \\
& \xrightarrow{\chi_6} CX_{0,1} \cdot CX_{0,2} \cdot CCX_{1,2} \cdot CX_{0,2} \cdot CX_{0,1} \cdot \overline{CCX_{0,2} \cdot CCX_{0,1} \cdot CCX_{0,2}} \\
& \xleftarrow{\delta_{24}} CX_{0,1} \cdot CX_{0,2} \cdot CCX_{1,2} \cdot CX_{0,2} \cdot \overline{CCX_{0,2} \cdot CCX_{0,1} \cdot CCX_{0,2} \cdot CX_{0,2}} \\
& \xrightarrow{\chi_9} CX_{0,1} \cdot CX_{0,2} \cdot CCX_{1,2} \cdot \overline{CX_{0,2} \cdot CCX_{0,1} \cdot CCX_{0,2} \cdot CCX_{0,1}} \cdot CX_{0,2} \\
& \xleftarrow{\delta_{23}} CX_{0,1} \cdot CX_{0,2} \cdot CCX_{1,2} \cdot \overline{CCX_{0,1} \cdot CCX_{0,2} \cdot CCX_{0,1} \cdot CX_{0,1}} \cdot CX_{0,2} \\
& \xleftarrow{(24)} CX_{0,1} \cdot CX_{0,2} \cdot \overline{CCX_{1,2} \cdot CCX_{0,1} \cdot CCX_{0,2} \cdot CCX_{0,1} \cdot CCX_{1,2} \cdot CX_{0,1} \cdot CX_{0,2}} \\
& \xrightarrow{\xi_{55}} CX_{0,1} \cdot CX_{0,2} \cdot \overline{CCX_{0,1} \cdot CCX_{0,2} \cdot CCX_{0,1}} \cdot CCX_{1,2} \cdot CX_{0,1} \cdot CX_{0,2} \\
& \xleftarrow{\delta_{23}} CX_{0,1} \cdot \overline{CCX_{0,1} \cdot CCX_{0,2} \cdot CCX_{0,1} \cdot CX_{0,1} \cdot CCX_{1,2} \cdot CX_{0,1} \cdot CX_{0,2}}
\end{aligned}$$

$$\begin{aligned}
& \xleftarrow{\chi_9} CX_{0,1} \cdot \overline{CCX_{0,2} \cdot CCX_{0,1} \cdot CCX_{0,2}} \cdot CX_{0,1} \cdot CCX_{1,2} \cdot CX_{0,1} \cdot CX_{0,2} \\
& \xleftarrow{\delta_{24}} \overline{CCX_{0,2} \cdot CCX_{0,1} \cdot CCX_{0,2} \cdot CX_{0,2}} \cdot CX_{0,1} \cdot CCX_{1,2} \cdot \overline{CX_{0,1} \cdot CX_{0,2}} \\
& \xrightarrow{C_{22}} CCX_{0,2} \cdot CCX_{0,1} \cdot CCX_{0,2} \cdot \overline{CX_{0,2} \cdot CX_{0,1}} \cdot CCX_{1,2} \cdot \overline{CX_{0,2} \cdot CX_{0,1}} \\
& \xleftarrow{C_{22}} CCX_{0,2} \cdot CCX_{0,1} \cdot CCX_{0,2} \cdot \overline{CX_{0,1} \cdot CX_{0,2}} \cdot CCX_{1,2} \cdot CX_{0,2} \cdot CX_{0,1} \\
& \xleftarrow{D_4} \overline{CCX_{0,2} \cdot CCX_{0,1} \cdot CCX_{0,2}} \cdot \overline{r_4} \xleftarrow{\chi_6} \overline{CX_{2,1} \cdot CCX_{0,1} \cdot CX_{2,1}} \cdot r_4 \xleftarrow{D_6} \overline{r_6} \cdot r_4 \\
(4;6) : \underline{r_4 \cdot r_6} \cdot r_4 \cdot r_6 & \xrightarrow{\delta_{25}} \overline{r_6 \cdot \underline{r_4} \cdot r_4} \cdot r_6 \xrightarrow{(4;4)} \overline{r_6 \cdot r_6} \xrightarrow{(6;6)} \varepsilon
\end{aligned}$$

### 1.7.29 Deriving the Coxeter Relation ( 4 ; 7 )

$$\begin{aligned}
(\delta_{26}) : CZ_{0,1} \cdot \underline{r_4} & \xrightarrow{D_4} \overline{CZ_{0,1} \cdot \underline{CX_{0,1}} \cdot CX_{0,2} \cdot CCX_{1,2} \cdot \overline{CX_{0,2}} \cdot CX_{0,1}} \xleftarrow{C_{76}} \overline{CX_{0,1} \cdot Z_0 \cdot \underline{CZ_{0,1}} \cdot CX_{0,2}} \cdot CCX_{1,2} \cdot CX_{0,2} \cdot CX_{0,1} \\
& \xleftarrow{C_{24}} CX_{0,1} \cdot \underline{Z_0 \cdot \overline{CX_{0,2}} \cdot \overline{CZ_{0,1}}} \cdot CCX_{1,2} \cdot CX_{0,2} \cdot CX_{0,1} \\
& \xleftarrow{C_{90}} CX_{0,1} \cdot \overline{CX_{0,2} \cdot Z_0} \cdot \underline{CZ_{0,1}} \cdot CCX_{1,2} \cdot CX_{0,2} \cdot CX_{0,1} \\
& \xrightarrow{C_{77}} CX_{0,1} \cdot CX_{0,2} \cdot \underline{Z_0 \cdot \overline{CCX_{1,2}} \cdot \overline{CZ_{1,2}} \cdot \overline{CZ_{0,1}}} \cdot CX_{0,2} \cdot CX_{0,1} \\
& \xrightarrow{C_{49}} CX_{0,1} \cdot CX_{0,2} \cdot \overline{CCX_{1,2} \cdot \underline{CZ_{1,2}} \cdot Z_0} \cdot CZ_{1,2} \cdot CZ_{0,1} \cdot CX_{0,2} \cdot CX_{0,1} \\
& \xrightarrow{B_{31}} CX_{0,1} \cdot CX_{0,2} \cdot CCX_{1,2} \cdot \overline{Z_0 \cdot \underline{CZ_{1,2}} \cdot CZ_{1,2}} \cdot CZ_{0,1} \cdot CX_{0,2} \cdot CX_{0,1} \\
& \xrightarrow{E_{12}} CX_{0,1} \cdot CX_{0,2} \cdot CCX_{1,2} \cdot Z_0 \cdot \underline{CZ_{0,1}} \cdot \underline{CX_{0,2}} \cdot CX_{0,1} \\
& \xleftarrow{C_{24}} CX_{0,1} \cdot CX_{0,2} \cdot CCX_{1,2} \cdot \underline{Z_0 \cdot \overline{CX_{0,2}} \cdot \overline{CZ_{0,1}}} \cdot CX_{0,1} \\
& \xleftarrow{C_{90}} CX_{0,1} \cdot CX_{0,2} \cdot CCX_{1,2} \cdot \overline{CX_{0,2} \cdot Z_0} \cdot \underline{CZ_{0,1}} \cdot CX_{0,1} \\
& \xleftarrow{C_{88}} CX_{0,1} \cdot CX_{0,2} \cdot CCX_{1,2} \cdot CX_{0,2} \cdot \overline{CZ_{0,1}} \cdot \underline{Z_0} \cdot CX_{0,1} \\
& \xleftarrow{C_{85}} CX_{0,1} \cdot CX_{0,2} \cdot CCX_{1,2} \cdot CX_{0,2} \cdot \underline{CZ_{0,1}} \cdot \overline{CX_{0,1}} \cdot Z_0 \\
& \xleftarrow{C_{76}} CX_{0,1} \cdot CX_{0,2} \cdot CCX_{1,2} \cdot CX_{0,2} \cdot \overline{CX_{0,1} \cdot Z_0 \cdot \underline{CZ_{0,1}}} \cdot Z_0 \\
& \xleftarrow{C_{88}} CX_{0,1} \cdot CX_{0,2} \cdot CCX_{1,2} \cdot CX_{0,2} \cdot CX_{0,1} \cdot \overline{CZ_{0,1}} \cdot \underline{Z_0} \cdot Z_0 \\
& \xrightarrow{E_3} \overline{CX_{0,1} \cdot CX_{0,2} \cdot CCX_{1,2} \cdot CX_{0,2} \cdot CX_{0,1} \cdot CZ_{0,1}} \\
& \xleftarrow{D_4} \overline{r_4} \cdot CZ_{0,1} \\
r_4 \cdot r_7 \cdot r_4 \cdot \underline{r_7} & \xrightarrow{\xi_3} r_4 \cdot \underline{r_7} \cdot r_4 \cdot \overline{CZ_{0,1} \cdot r_6 \cdot \underline{CZ_{0,1}}} \xrightarrow{\xi_3} r_4 \cdot \overline{CZ_{0,1} \cdot r_6 \cdot \underline{CZ_{0,1}}} \cdot r_4 \cdot CZ_{0,1} \cdot r_6 \cdot CZ_{0,1} \\
& \xrightarrow{\delta_{26}} \overline{r_4 \cdot \underline{CZ_{0,1}} \cdot r_6 \cdot \overline{r_4 \cdot \underline{CZ_{0,1}}}} \cdot CZ_{0,1} \cdot r_6 \cdot CZ_{0,1} \\
& \xleftarrow{\delta_{26}} \overline{CZ_{0,1} \cdot r_4 \cdot r_6 \cdot r_4 \cdot \underline{CZ_{0,1}} \cdot CZ_{0,1}} \cdot r_6 \cdot CZ_{0,1} \\
& \xrightarrow{E_2} CZ_{0,1} \cdot \underline{r_4 \cdot r_6 \cdot r_4 \cdot r_6} \cdot CZ_{0,1} \xrightarrow{(4;6)} \overline{CZ_{0,1} \cdot CZ_{0,1}} \xrightarrow{E_2} \varepsilon
\end{aligned}$$

### 1.7.30 Deriving the Coxeter Relation ( 4 ; 8 )

$$(\delta_{27}) : CX_{0,1} \cdot \underline{r_8} \xrightarrow{D_8} \overline{CX_{0,1} \cdot \underline{K_{1,2}} \cdot X_1 \cdot X_2 \cdot CZ_{0,2} \cdot CCX_{1,2} \cdot CZ_{0,2} \cdot X_2 \cdot X_1 \cdot K_{1,2}}$$

$$\begin{aligned}
& \xleftarrow{C_{41}} \overline{K_{1,2} \cdot \underline{CZ_{0,1}} \cdot X_1 \cdot X_2 \cdot CZ_{0,2} \cdot CCX_{1,2} \cdot CZ_{0,2} \cdot X_2 \cdot X_1 \cdot K_{1,2}} \\
& \xleftarrow{C_{112}} K_{1,2} \cdot \overline{X_1 \cdot Z_0 \cdot \underline{CZ_{0,1}}} \cdot X_2 \cdot CZ_{0,2} \cdot CCX_{1,2} \cdot CZ_{0,2} \cdot X_2 \cdot X_1 \cdot K_{1,2} \\
& \xleftarrow{B_{37}} K_{1,2} \cdot X_1 \cdot \underline{Z_0 \cdot \overline{X_2} \cdot CZ_{0,1}} \cdot CZ_{0,2} \cdot CCX_{1,2} \cdot CZ_{0,2} \cdot X_2 \cdot X_1 \cdot K_{1,2} \\
& \xleftarrow{B_{23}} K_{1,2} \cdot X_1 \cdot \overline{X_2 \cdot Z_0} \cdot \underline{CZ_{0,1} \cdot CZ_{0,2}} \cdot CCX_{1,2} \cdot CZ_{0,2} \cdot X_2 \cdot X_1 \cdot K_{1,2} \\
& \xrightarrow{C_{60}} K_{1,2} \cdot X_1 \cdot X_2 \cdot \underline{Z_0 \cdot \overline{CZ_{0,2}} \cdot CZ_{0,1}} \cdot CCX_{1,2} \cdot CZ_{0,2} \cdot X_2 \cdot X_1 \cdot K_{1,2} \\
& \xleftarrow{C_{103}} K_{1,2} \cdot X_1 \cdot X_2 \cdot \overline{CZ_{0,2} \cdot Z_0} \cdot \underline{CZ_{0,1} \cdot CCX_{1,2}} \cdot CZ_{0,2} \cdot X_2 \cdot X_1 \cdot K_{1,2} \\
& \xrightarrow{C_{77}} K_{1,2} \cdot X_1 \cdot X_2 \cdot CZ_{0,2} \cdot \underline{Z_0 \cdot \overline{CCX_{1,2}}} \cdot \overline{CZ_{1,2} \cdot CZ_{0,1}} \cdot CZ_{0,2} \cdot X_2 \cdot X_1 \cdot K_{1,2} \\
& \xrightarrow{C_{49}} K_{1,2} \cdot X_1 \cdot X_2 \cdot CZ_{0,2} \cdot \overline{CCX_{1,2} \cdot \underline{CZ_{1,2} \cdot Z_0}} \cdot CZ_{1,2} \cdot CZ_{0,1} \cdot CZ_{0,2} \cdot X_2 \cdot X_1 \cdot K_{1,2} \\
& \xrightarrow{B_{31}} K_{1,2} \cdot X_1 \cdot X_2 \cdot CZ_{0,2} \cdot CCX_{1,2} \cdot \overline{Z_0 \cdot \underline{CZ_{1,2} \cdot CZ_{1,2}}} \cdot CZ_{0,1} \cdot CZ_{0,2} \cdot X_2 \cdot X_1 \cdot K_{1,2} \\
& \xrightarrow{E_{12}} K_{1,2} \cdot X_1 \cdot X_2 \cdot CZ_{0,2} \cdot CCX_{1,2} \cdot Z_0 \cdot \underline{CZ_{0,1} \cdot CZ_{0,2}} \cdot X_2 \cdot X_1 \cdot K_{1,2} \\
& \xrightarrow{C_{60}} K_{1,2} \cdot X_1 \cdot X_2 \cdot CZ_{0,2} \cdot CCX_{1,2} \cdot \underline{Z_0 \cdot \overline{CZ_{0,2} \cdot CZ_{0,1}}} \cdot X_2 \cdot X_1 \cdot K_{1,2} \\
& \xleftarrow{C_{103}} K_{1,2} \cdot X_1 \cdot X_2 \cdot CZ_{0,2} \cdot CCX_{1,2} \cdot \overline{CZ_{0,2} \cdot Z_0} \cdot \underline{CZ_{0,1} \cdot X_2} \cdot X_1 \cdot K_{1,2} \\
& \xleftarrow{B_{37}} K_{1,2} \cdot X_1 \cdot X_2 \cdot CZ_{0,2} \cdot CCX_{1,2} \cdot CZ_{0,2} \cdot \underline{Z_0 \cdot \overline{X_2} \cdot CZ_{0,1}} \cdot X_1 \cdot K_{1,2} \\
& \xleftarrow{B_{23}} K_{1,2} \cdot X_1 \cdot X_2 \cdot CZ_{0,2} \cdot CCX_{1,2} \cdot CZ_{0,2} \cdot \overline{X_2 \cdot Z_0} \cdot \underline{CZ_{0,1} \cdot X_1} \cdot K_{1,2} \\
& \xleftarrow{C_{112}} K_{1,2} \cdot X_1 \cdot X_2 \cdot CZ_{0,2} \cdot CCX_{1,2} \cdot CZ_{0,2} \cdot X_2 \cdot Z_0 \cdot \overline{X_1 \cdot Z_0 \cdot CZ_{0,1}} \cdot K_{1,2} \\
& \xrightarrow{B_{15}} K_{1,2} \cdot X_1 \cdot X_2 \cdot CZ_{0,2} \cdot CCX_{1,2} \cdot CZ_{0,2} \cdot X_2 \cdot \underline{Z_0 \cdot \overline{Z_0} \cdot X_1} \cdot CZ_{0,1} \cdot K_{1,2} \\
& \xrightarrow{E_3} K_{1,2} \cdot X_1 \cdot X_2 \cdot CZ_{0,2} \cdot CCX_{1,2} \cdot CZ_{0,2} \cdot X_2 \cdot X_1 \cdot \underline{CZ_{0,1} \cdot K_{1,2}} \\
& \xrightarrow{C_{46}} \underline{K_{1,2} \cdot X_1 \cdot X_2 \cdot CZ_{0,2} \cdot CCX_{1,2} \cdot CZ_{0,2} \cdot X_2 \cdot X_1 \cdot \overline{K_{1,2} \cdot CX_{0,1}}} \xleftarrow{D_8} \overline{r_8} \cdot CX_{0,1} \\
\\
(\delta_{28}) : CX_{0,2} \cdot \underline{r_8} & \xrightarrow{D_8} \underline{CX_{0,2} \cdot \overline{K_{1,2} \cdot X_1 \cdot X_2 \cdot CZ_{0,2} \cdot CCX_{1,2} \cdot CZ_{0,2} \cdot X_2 \cdot X_1 \cdot K_{1,2}}} \\
& \xleftarrow{C_{28}} \overline{K_{1,2} \cdot \underline{CZ_{0,2}} \cdot X_1 \cdot X_2 \cdot CZ_{0,2} \cdot CCX_{1,2} \cdot CZ_{0,2} \cdot X_2 \cdot X_1 \cdot K_{1,2}} \\
& \xleftarrow{B_{35}} K_{1,2} \cdot \overline{X_1 \cdot \underline{CZ_{0,2} \cdot X_2} \cdot CZ_{0,2} \cdot CCX_{1,2} \cdot CZ_{0,2} \cdot X_2 \cdot X_1 \cdot K_{1,2}} \\
& \xleftarrow{C_{115}} K_{1,2} \cdot X_1 \cdot \overline{X_2 \cdot Z_0 \cdot \underline{CZ_{0,2}}} \cdot CZ_{0,2} \cdot CCX_{1,2} \cdot CZ_{0,2} \cdot X_2 \cdot X_1 \cdot K_{1,2} \\
& \xleftarrow{C_{103}} K_{1,2} \cdot X_1 \cdot X_2 \cdot \overline{CZ_{0,2} \cdot Z_0} \cdot \underline{CZ_{0,2} \cdot CCX_{1,2}} \cdot CZ_{0,2} \cdot X_2 \cdot X_1 \cdot K_{1,2} \\
& \xrightarrow{C_{100}} K_{1,2} \cdot X_1 \cdot X_2 \cdot CZ_{0,2} \cdot \underline{Z_0 \cdot \overline{CCX_{1,2}}} \cdot \overline{CZ_{1,2} \cdot CZ_{0,2}} \cdot CZ_{0,2} \cdot X_2 \cdot X_1 \cdot K_{1,2} \\
& \xrightarrow{C_{49}} K_{1,2} \cdot X_1 \cdot X_2 \cdot CZ_{0,2} \cdot \overline{CCX_{1,2} \cdot \underline{CZ_{1,2} \cdot Z_0}} \cdot CZ_{1,2} \cdot CZ_{0,2} \cdot CZ_{0,2} \cdot X_2 \cdot X_1 \cdot K_{1,2} \\
& \xrightarrow{B_{31}} K_{1,2} \cdot X_1 \cdot X_2 \cdot CZ_{0,2} \cdot CCX_{1,2} \cdot \overline{Z_0 \cdot \underline{CZ_{1,2} \cdot CZ_{1,2}}} \cdot CZ_{0,2} \cdot CZ_{0,2} \cdot X_2 \cdot X_1 \cdot K_{1,2} \\
& \xrightarrow{E_{12}} K_{1,2} \cdot X_1 \cdot X_2 \cdot CZ_{0,2} \cdot CCX_{1,2} \cdot \underline{Z_0 \cdot CZ_{0,2}} \cdot CZ_{0,2} \cdot X_2 \cdot X_1 \cdot K_{1,2} \\
& \xleftarrow{C_{103}} K_{1,2} \cdot X_1 \cdot X_2 \cdot CZ_{0,2} \cdot CCX_{1,2} \cdot \overline{CZ_{0,2} \cdot Z_0} \cdot \underline{CZ_{0,2} \cdot X_2} \cdot X_1 \cdot K_{1,2} \\
& \xleftarrow{C_{115}} K_{1,2} \cdot X_1 \cdot X_2 \cdot CZ_{0,2} \cdot CCX_{1,2} \cdot CZ_{0,2} \cdot Z_0 \cdot \overline{X_2 \cdot Z_0 \cdot CZ_{0,2}} \cdot X_1 \cdot K_{1,2} \\
& \xrightarrow{B_{23}} K_{1,2} \cdot X_1 \cdot X_2 \cdot CZ_{0,2} \cdot CCX_{1,2} \cdot CZ_{0,2} \cdot \underline{Z_0 \cdot \overline{X_2} \cdot CZ_{0,2}} \cdot X_1 \cdot K_{1,2}
\end{aligned}$$

$$\begin{aligned}
& \xrightarrow{E_3} K_{1,2} \cdot X_1 \cdot X_2 \cdot CZ_{0,2} \cdot CCX_{1,2} \cdot CZ_{0,2} \cdot X_2 \cdot \overline{CZ_{0,2} \cdot X_1 \cdot K_{1,2}} \\
& \xleftarrow{B_{35}} K_{1,2} \cdot X_1 \cdot X_2 \cdot CZ_{0,2} \cdot CCX_{1,2} \cdot CZ_{0,2} \cdot X_2 \cdot \overline{X_1 \cdot CZ_{0,2} \cdot K_{1,2}} \\
& \xrightarrow{C_{29}} K_{1,2} \cdot X_1 \cdot X_2 \cdot CZ_{0,2} \cdot CCX_{1,2} \cdot CZ_{0,2} \cdot X_2 \cdot \overline{X_1 \cdot K_{1,2} \cdot CX_{0,2}} \xleftarrow{D_8} \overline{r_8} \cdot CX_{0,2} \\
\\
(\delta_{29}) : & \overline{K_{1,2} \cdot CX_{0,2}} \cdot CCX_{1,2} \cdot CX_{0,2} \cdot K_{1,2} \cdot CCX_{1,2} \xleftarrow{C_{29}} \overline{CZ_{0,2} \cdot K_{1,2}} \cdot CCX_{1,2} \cdot \overline{CX_{0,2} \cdot K_{1,2}} \cdot CCX_{1,2} \\
& \xleftarrow{C_{28}} CZ_{0,2} \cdot K_{1,2} \cdot CCX_{1,2} \cdot \overline{K_{1,2} \cdot CZ_{0,2}} \cdot CCX_{1,2} \\
& \xleftarrow{(25)} \overline{CZ_{0,2} \cdot K_{1,2} \cdot CCX_{1,2} \cdot K_{1,2} \cdot CZ_{0,2} \cdot CCX_{1,2} \cdot \overline{K_{0,1} \cdot K_{0,1}}} \\
& \xrightarrow{C_{42}} CZ_{0,2} \cdot K_{1,2} \cdot CCX_{1,2} \cdot K_{1,2} \cdot \overline{CZ_{0,2} \cdot \overline{K_{0,1} \cdot CCX_{0,2}}} \cdot K_{0,1} \\
& \xleftarrow{C_{73}} CZ_{0,2} \cdot K_{1,2} \cdot CCX_{1,2} \cdot K_{1,2} \cdot \overline{K_{0,1} \cdot CX_{2,0}} \cdot CCX_{0,2} \cdot K_{0,1} \\
& \xrightarrow{C_{93}} CZ_{0,2} \cdot K_{1,2} \cdot CCX_{1,2} \cdot K_{1,2} \cdot K_{0,1} \cdot \overline{CCX_{0,2} \cdot CX_{2,1} \cdot CX_{2,0}} \cdot K_{0,1} \\
& \xleftarrow{(25)} CZ_{0,2} \cdot K_{1,2} \cdot CCX_{1,2} \cdot K_{1,2} \cdot K_{0,1} \cdot CCX_{0,2} \cdot CX_{2,1} \cdot \overline{K_{0,1} \cdot K_{0,1} \cdot CX_{2,0}} \cdot K_{0,1} \\
& \xrightarrow{C_{73}} CZ_{0,2} \cdot K_{1,2} \cdot CCX_{1,2} \cdot K_{1,2} \cdot K_{0,1} \cdot CCX_{0,2} \cdot CX_{2,1} \cdot K_{0,1} \cdot \overline{CZ_{0,2} \cdot \overline{K_{0,1} \cdot K_{0,1}}} \\
& \xrightarrow{(25)} CZ_{0,2} \cdot K_{1,2} \cdot CCX_{1,2} \cdot \overline{K_{1,2} \cdot K_{0,1}} \cdot CCX_{0,2} \cdot CX_{2,1} \cdot K_{0,1} \cdot CZ_{0,2} \\
& \xleftarrow{(39)} CZ_{0,2} \cdot K_{1,2} \cdot CCX_{1,2} \cdot \overline{K_{0,1} \cdot K_{1,2}} \cdot CCX_{0,2} \cdot CX_{2,1} \cdot K_{0,1} \cdot CZ_{0,2} \\
& \xleftarrow{C_{38}} CZ_{0,2} \cdot K_{1,2} \cdot CCX_{1,2} \cdot K_{0,1} \cdot \overline{CCX_{0,1} \cdot K_{1,2} \cdot CX_{2,1}} \cdot K_{0,1} \cdot CZ_{0,2} \\
& \xrightarrow{C_4} CZ_{0,2} \cdot K_{1,2} \cdot CCX_{1,2} \cdot K_{0,1} \cdot CCX_{0,1} \cdot \overline{CX_{1,2} \cdot K_{1,2} \cdot K_{0,1}} \cdot CZ_{0,2} \\
& \xleftarrow{(39)} CZ_{0,2} \cdot K_{1,2} \cdot CCX_{1,2} \cdot K_{0,1} \cdot CCX_{0,1} \cdot CX_{1,2} \cdot \overline{K_{0,1} \cdot K_{1,2} \cdot CZ_{0,2}} \\
& \xrightarrow{C_{28}} CZ_{0,2} \cdot K_{1,2} \cdot \overline{CCX_{1,2} \cdot K_{0,1}} \cdot CCX_{0,1} \cdot CX_{1,2} \cdot K_{0,1} \cdot \overline{CX_{0,2} \cdot K_{1,2}} \\
& \xrightarrow{C_{42}} CZ_{0,2} \cdot K_{1,2} \cdot \overline{K_{0,1} \cdot CCX_{0,2}} \cdot \overline{CCX_{0,1} \cdot CX_{1,2}} \cdot K_{0,1} \cdot CX_{0,2} \cdot K_{1,2} \\
& \xrightarrow{C_{107}} CZ_{0,2} \cdot K_{1,2} \cdot K_{0,1} \cdot CCX_{0,2} \cdot \overline{CX_{1,2} \cdot CCX_{0,1}} \cdot K_{0,1} \cdot CX_{0,2} \cdot K_{1,2} \\
& \xleftarrow{E_8} CZ_{0,2} \cdot K_{1,2} \cdot K_{0,1} \cdot \overline{CX_{1,2} \cdot CX_{1,2}} \cdot CCX_{0,2} \cdot \overline{CX_{1,2} \cdot CCX_{0,1} \cdot K_{0,1} \cdot CX_{0,2} \cdot K_{1,2}} \\
& \xrightarrow{X_7} CZ_{0,2} \cdot K_{1,2} \cdot K_{0,1} \cdot CX_{1,2} \cdot \overline{CCX_{0,1} \cdot CCX_{0,2} \cdot CCX_{0,1} \cdot CCX_{0,1}} \cdot K_{0,1} \cdot CX_{0,2} \cdot K_{1,2} \\
& \xrightarrow{E_{18}} CZ_{0,2} \cdot K_{1,2} \cdot K_{0,1} \cdot CX_{1,2} \cdot CCX_{0,1} \cdot \overline{CCX_{0,2} \cdot K_{0,1} \cdot CX_{0,2} \cdot K_{1,2}} \\
& \xleftarrow{C_{36}} CZ_{0,2} \cdot \overline{K_{1,2} \cdot K_{0,1}} \cdot CX_{1,2} \cdot CCX_{0,1} \cdot \overline{K_{0,1} \cdot CCX_{1,2}} \cdot CX_{0,2} \cdot K_{1,2} \\
& \xleftarrow{(39)} CZ_{0,2} \cdot \overline{K_{0,1} \cdot K_{1,2}} \cdot CX_{1,2} \cdot CCX_{0,1} \cdot K_{0,1} \cdot CCX_{1,2} \cdot CX_{0,2} \cdot K_{1,2} \\
& \xleftarrow{C_{10}} CZ_{0,2} \cdot K_{0,1} \cdot \overline{CX_{2,1} \cdot K_{1,2}} \cdot CCX_{0,1} \cdot K_{0,1} \cdot CCX_{1,2} \cdot CX_{0,2} \cdot K_{1,2} \\
& \xrightarrow{C_{44}} CZ_{0,2} \cdot K_{0,1} \cdot CX_{2,1} \cdot \overline{CCX_{0,2} \cdot K_{1,2} \cdot K_{0,1}} \cdot CCX_{1,2} \cdot CX_{0,2} \cdot K_{1,2} \\
& \xleftarrow{(39)} CZ_{0,2} \cdot \overline{K_{0,1} \cdot CX_{2,1}} \cdot CCX_{0,2} \cdot \overline{K_{0,1} \cdot K_{1,2}} \cdot CCX_{1,2} \cdot CX_{0,2} \cdot K_{1,2} \\
& \xleftarrow{C_{74}} CZ_{0,2} \cdot \overline{CZ_{1,2} \cdot K_{0,1}} \cdot CCX_{0,2} \cdot K_{0,1} \cdot K_{1,2} \cdot CCX_{1,2} \cdot CX_{0,2} \cdot K_{1,2} \\
& \xleftarrow{C_{42}} CZ_{0,2} \cdot CZ_{1,2} \cdot \overline{CCX_{1,2} \cdot K_{0,1} \cdot K_{0,1}} \cdot K_{1,2} \cdot CCX_{1,2} \cdot CX_{0,2} \cdot K_{1,2}
\end{aligned}$$

$$\begin{aligned}
& \xrightarrow{(25)} \overline{CZ_{0,2} \cdot CZ_{1,2} \cdot CCX_{1,2} \cdot K_{1,2} \cdot CCX_{1,2} \cdot CX_{0,2} \cdot K_{1,2}} \\
& \xleftarrow{C_{101}} \overline{CCX_{1,2} \cdot CZ_{0,2} \cdot K_{1,2} \cdot CCX_{1,2} \cdot CX_{0,2} \cdot K_{1,2}} \xrightarrow{C_{29}} \overline{CCX_{1,2} \cdot \overline{K_{1,2}} \cdot \overline{CX_{0,2}} \cdot CCX_{1,2} \cdot CX_{0,2} \cdot K_{1,2}} \\
\\
(\delta_{30}) : CCX_{1,2} \cdot r_8 & \xrightarrow{D_8} CCX_{1,2} \cdot \overline{K_{1,2} \cdot X_1 \cdot X_2 \cdot CZ_{0,2} \cdot CCX_{1,2} \cdot CZ_{0,2} \cdot X_2 \cdot X_1 \cdot K_{1,2}} \\
& \xleftarrow{(23)} \overline{K_{1,2} \cdot \overline{K_{1,2}} \cdot CCX_{1,2} \cdot K_{1,2} \cdot X_1 \cdot X_2 \cdot CZ_{0,2} \cdot CCX_{1,2} \cdot CZ_{0,2} \cdot X_2 \cdot X_1 \cdot K_{1,2}} \\
& \xleftarrow{E_5} K_{1,2} \cdot K_{1,2} \cdot \overline{Z_1 \cdot \overline{Z_1}} \cdot \overline{CCX_{1,2}} \cdot K_{1,2} \cdot X_1 \cdot X_2 \cdot CZ_{0,2} \cdot CCX_{1,2} \cdot CZ_{0,2} \cdot X_2 \cdot X_1 \cdot K_{1,2} \\
& \xrightarrow{C_{59}} K_{1,2} \cdot K_{1,2} \cdot Z_1 \cdot \overline{CCX_{1,2} \cdot \overline{Z_1}} \cdot \overline{K_{1,2} \cdot X_1 \cdot X_2 \cdot CZ_{0,2} \cdot CCX_{1,2} \cdot CZ_{0,2} \cdot X_2 \cdot X_1 \cdot K_{1,2}} \\
& \xrightarrow{C_{27}} K_{1,2} \cdot K_{1,2} \cdot Z_1 \cdot CCX_{1,2} \cdot \overline{Z_1 \cdot \overline{K_{1,2}}} \cdot X_2 \cdot CZ_{0,2} \cdot CCX_{1,2} \cdot CZ_{0,2} \cdot X_2 \cdot X_1 \cdot K_{1,2} \\
& \xrightarrow{E_5} K_{1,2} \cdot \overline{K_{1,2}} \cdot Z_1 \cdot CCX_{1,2} \cdot K_{1,2} \cdot X_2 \cdot CZ_{0,2} \cdot CCX_{1,2} \cdot CZ_{0,2} \cdot X_2 \cdot X_1 \cdot K_{1,2} \\
& \xleftarrow{C_2} K_{1,2} \cdot \overline{X_1 \cdot \overline{K_{1,2}}} \cdot CCX_{1,2} \cdot \overline{K_{1,2} \cdot X_2 \cdot CZ_{0,2} \cdot CCX_{1,2} \cdot CZ_{0,2} \cdot X_2 \cdot X_1 \cdot K_{1,2}} \\
& \xrightarrow{C_{26}} K_{1,2} \cdot X_1 \cdot K_{1,2} \cdot \overline{CCX_{1,2} \cdot \overline{Z_2}} \cdot \overline{K_{1,2} \cdot CZ_{0,2} \cdot CCX_{1,2} \cdot CZ_{0,2} \cdot X_2 \cdot X_1 \cdot K_{1,2}} \\
& \xleftarrow{C_{50}} K_{1,2} \cdot X_1 \cdot \overline{K_{1,2} \cdot \overline{Z_2}} \cdot \overline{CCX_{1,2}} \cdot K_{1,2} \cdot CZ_{0,2} \cdot CCX_{1,2} \cdot CZ_{0,2} \cdot X_2 \cdot X_1 \cdot K_{1,2} \\
& \xleftarrow{C_{16}} K_{1,2} \cdot X_1 \cdot \overline{X_2 \cdot \overline{K_{1,2}}} \cdot CCX_{1,2} \cdot \overline{K_{1,2} \cdot CZ_{0,2}} \cdot CCX_{1,2} \cdot CZ_{0,2} \cdot X_2 \cdot X_1 \cdot K_{1,2} \\
& \xrightarrow{C_{28}} K_{1,2} \cdot X_1 \cdot X_2 \cdot K_{1,2} \cdot CCX_{1,2} \cdot \overline{CX_{0,2} \cdot \overline{K_{1,2}}} \cdot CCX_{1,2} \cdot CZ_{0,2} \cdot X_2 \cdot X_1 \cdot K_{1,2} \\
& \xleftarrow{E_{15}} K_{1,2} \cdot X_1 \cdot X_2 \cdot \overline{K_{1,2} \cdot \overline{CX_{0,2}}} \cdot \overline{CX_{0,2} \cdot CCX_{1,2} \cdot CX_{0,2} \cdot K_{1,2} \cdot CCX_{1,2} \cdot CZ_{0,2} \cdot X_2 \cdot X_1 \cdot K_{1,2}} \\
& \xleftarrow{C_{29}} K_{1,2} \cdot X_1 \cdot X_2 \cdot \overline{CZ_{0,2} \cdot \overline{K_{1,2}}} \cdot \overline{CX_{0,2} \cdot CCX_{1,2} \cdot CX_{0,2} \cdot K_{1,2} \cdot CCX_{1,2} \cdot CZ_{0,2} \cdot X_2 \cdot X_1 \cdot K_{1,2}} \\
& \xrightarrow{\delta_{29}} K_{1,2} \cdot X_1 \cdot X_2 \cdot CZ_{0,2} \cdot \overline{CCX_{1,2} \cdot K_{1,2} \cdot CX_{0,2} \cdot CCX_{1,2} \cdot CX_{0,2} \cdot \overline{K_{1,2}}} \cdot \overline{CZ_{0,2} \cdot X_2 \cdot X_1 \cdot K_{1,2}} \\
& \xrightarrow{C_{28}} K_{1,2} \cdot X_1 \cdot X_2 \cdot CZ_{0,2} \cdot CCX_{1,2} \cdot K_{1,2} \cdot CX_{0,2} \cdot CCX_{1,2} \cdot \overline{CX_{0,2} \cdot \overline{K_{1,2}}} \cdot \overline{CZ_{0,2} \cdot X_2 \cdot X_1 \cdot K_{1,2}} \\
& \xrightarrow{E_{15}} K_{1,2} \cdot X_1 \cdot X_2 \cdot CZ_{0,2} \cdot CCX_{1,2} \cdot \overline{K_{1,2} \cdot CX_{0,2}} \cdot CCX_{1,2} \cdot K_{1,2} \cdot X_2 \cdot X_1 \cdot K_{1,2} \\
& \xleftarrow{C_{29}} K_{1,2} \cdot X_1 \cdot X_2 \cdot CZ_{0,2} \cdot CCX_{1,2} \cdot \overline{CZ_{0,2} \cdot \overline{K_{1,2}}} \cdot CCX_{1,2} \cdot \overline{K_{1,2} \cdot X_2 \cdot X_1 \cdot K_{1,2}} \\
& \xrightarrow{C_{26}} K_{1,2} \cdot X_1 \cdot X_2 \cdot CZ_{0,2} \cdot CCX_{1,2} \cdot CZ_{0,2} \cdot K_{1,2} \cdot \overline{CCX_{1,2} \cdot \overline{Z_2}} \cdot \overline{K_{1,2} \cdot X_1 \cdot K_{1,2}} \\
& \xleftarrow{C_{50}} K_{1,2} \cdot X_1 \cdot X_2 \cdot CZ_{0,2} \cdot CCX_{1,2} \cdot CZ_{0,2} \cdot \overline{K_{1,2} \cdot \overline{Z_2}} \cdot \overline{CCX_{1,2}} \cdot K_{1,2} \cdot X_1 \cdot K_{1,2} \\
& \xleftarrow{C_{16}} K_{1,2} \cdot X_1 \cdot X_2 \cdot CZ_{0,2} \cdot CCX_{1,2} \cdot CZ_{0,2} \cdot \overline{X_2 \cdot \overline{K_{1,2}}} \cdot CCX_{1,2} \cdot K_{1,2} \cdot X_1 \cdot K_{1,2} \\
& \xleftarrow{E_5} K_{1,2} \cdot X_1 \cdot X_2 \cdot CZ_{0,2} \cdot CCX_{1,2} \cdot CZ_{0,2} \cdot X_2 \cdot K_{1,2} \cdot \overline{Z_1 \cdot \overline{Z_1}} \cdot \overline{CCX_{1,2}} \cdot K_{1,2} \cdot X_1 \cdot K_{1,2} \\
& \xrightarrow{C_{59}} K_{1,2} \cdot X_1 \cdot X_2 \cdot CZ_{0,2} \cdot CCX_{1,2} \cdot CZ_{0,2} \cdot X_2 \cdot K_{1,2} \cdot Z_1 \cdot \overline{CCX_{1,2} \cdot \overline{Z_1}} \cdot \overline{K_{1,2} \cdot X_1 \cdot K_{1,2}} \\
& \xleftarrow{C_{27}} K_{1,2} \cdot X_1 \cdot X_2 \cdot CZ_{0,2} \cdot CCX_{1,2} \cdot CZ_{0,2} \cdot X_2 \cdot K_{1,2} \cdot Z_1 \cdot CCX_{1,2} \cdot \overline{K_{1,2} \cdot \overline{X_1}} \cdot \overline{X_1 \cdot K_{1,2}} \\
& \xrightarrow{E_{13}} K_{1,2} \cdot X_1 \cdot X_2 \cdot CZ_{0,2} \cdot CCX_{1,2} \cdot CZ_{0,2} \cdot X_2 \cdot \overline{K_{1,2} \cdot Z_1} \cdot CCX_{1,2} \cdot K_{1,2} \cdot K_{1,2} \\
& \xleftarrow{C_2} K_{1,2} \cdot X_1 \cdot X_2 \cdot CZ_{0,2} \cdot CCX_{1,2} \cdot CZ_{0,2} \cdot X_2 \cdot \overline{X_1 \cdot \overline{K_{1,2}}} \cdot CCX_{1,2} \cdot \overline{K_{1,2} \cdot K_{1,2}} \\
& \xrightarrow{(23)} K_{1,2} \cdot X_1 \cdot X_2 \cdot CZ_{0,2} \cdot CCX_{1,2} \cdot CZ_{0,2} \cdot X_2 \cdot X_1 \cdot K_{1,2} \cdot CCX_{1,2} \\
& \xleftarrow{D_8} \overline{r_8} \cdot CCX_{1,2}
\end{aligned}$$

$$\begin{aligned}
r_4 \cdot r_8 \cdot \underline{r_4} \cdot r_8 &\xrightarrow{D_4} r_4 \cdot r_8 \cdot \overline{CX_{0,1} \cdot CX_{0,2} \cdot CCX_{1,2} \cdot CX_{0,2} \cdot CX_{0,1}} \cdot r_8 \\
&\xrightarrow{D_4} \overline{CX_{0,1} \cdot CX_{0,2} \cdot CCX_{1,2} \cdot CX_{0,2} \cdot CX_{0,1}} \cdot r_8 \cdot CX_{0,1} \cdot CX_{0,2} \cdot CCX_{1,2} \cdot CX_{0,2} \cdot \overline{CX_{0,1} \cdot r_8} \\
&\xrightarrow{\delta_{27}} CX_{0,1} \cdot CX_{0,2} \cdot CCX_{1,2} \cdot CX_{0,2} \cdot \overline{CX_{0,1} \cdot r_8} \cdot CX_{0,1} \cdot CX_{0,2} \cdot CCX_{1,2} \cdot CX_{0,2} \cdot \overline{r_8 \cdot CX_{0,1}} \\
&\xrightarrow{\delta_{27}} CX_{0,1} \cdot CX_{0,2} \cdot CCX_{1,2} \cdot CX_{0,2} \cdot \overline{r_8 \cdot CX_{0,1}} \cdot CX_{0,1} \cdot CX_{0,2} \cdot CCX_{1,2} \cdot CX_{0,2} \cdot r_8 \cdot CX_{0,1} \\
&\xrightarrow{(22)} CX_{0,1} \cdot CX_{0,2} \cdot CCX_{1,2} \cdot CX_{0,2} \cdot r_8 \cdot CX_{0,2} \cdot CCX_{1,2} \cdot \overline{CX_{0,2} \cdot r_8} \cdot CX_{0,1} \\
&\xrightarrow{\delta_{28}} CX_{0,1} \cdot CX_{0,2} \cdot CCX_{1,2} \cdot \overline{CX_{0,2} \cdot r_8} \cdot CX_{0,2} \cdot CCX_{1,2} \cdot \overline{r_8 \cdot CX_{0,2}} \cdot CX_{0,1} \\
&\xrightarrow{\delta_{28}} CX_{0,1} \cdot CX_{0,2} \cdot CCX_{1,2} \cdot \overline{r_8 \cdot CX_{0,2}} \cdot CX_{0,2} \cdot CCX_{1,2} \cdot r_8 \cdot CX_{0,2} \cdot CX_{0,1} \\
&\xrightarrow{E_{15}} CX_{0,1} \cdot CX_{0,2} \cdot \overline{CCX_{1,2} \cdot r_8} \cdot CCX_{1,2} \cdot r_8 \cdot CX_{0,2} \cdot CX_{0,1} \\
&\xrightarrow{\delta_{30}} CX_{0,1} \cdot CX_{0,2} \cdot r_8 \cdot \overline{CCX_{1,2} \cdot CCX_{1,2}} \cdot r_8 \cdot CX_{0,2} \cdot CX_{0,1} \\
&\xrightarrow{(24)} CX_{0,1} \cdot CX_{0,2} \cdot r_8 \cdot r_8 \cdot CX_{0,2} \cdot CX_{0,1} \\
&\xrightarrow{(8,8)} CX_{0,1} \cdot \overline{CX_{0,2} \cdot CX_{0,2}} \cdot CX_{0,1} \xrightarrow{E_{15}} \overline{CX_{0,1} \cdot CX_{0,1}} \xrightarrow{(22)} \varepsilon
\end{aligned}$$

### 1.7.31 Deriving the Coxeter Relation ( 5 ; 6 )

$$\begin{aligned}
(\delta_{31}) : r_5 \cdot r_6 &\xrightarrow{D_6} \underline{r_5} \cdot \overline{CX_{2,1} \cdot CCX_{0,1} \cdot CX_{2,1}} \xrightarrow{D_6} \overline{X_1 \cdot CCX_{0,1} \cdot X_1} \cdot CX_{2,1} \cdot CCX_{0,1} \cdot CX_{2,1} \\
&\xleftarrow{(21)} X_1 \cdot CCX_{0,1} \cdot X_1 \cdot CX_{2,1} \cdot CCX_{0,1} \cdot CX_{2,1} \cdot \overline{X_0 \cdot X_0} \\
&\xleftarrow{(21)} X_1 \cdot CCX_{0,1} \cdot X_1 \cdot \overline{X_0 \cdot X_0} \cdot CX_{2,1} \cdot \overline{CCX_{0,1} \cdot CX_{2,1} \cdot X_0 \cdot X_0} \\
&\xleftarrow{D_2} X_1 \cdot CCX_{0,1} \cdot X_1 \cdot X_0 \cdot \overline{r_2} \cdot X_0 \\
&\xleftarrow{(21)} \overline{X_0 \cdot X_0} \cdot X_1 \cdot \overline{CCX_{0,1} \cdot X_1 \cdot X_0} \cdot r_2 \cdot X_0 \xleftarrow{D_1} X_0 \cdot \overline{r_1} \cdot r_2 \cdot X_0 \\
\\
(5;6) : r_5 \cdot r_6 \cdot r_5 \cdot r_6 \cdot \underline{r_5} \cdot r_6 &\xrightarrow{\delta_{31}} r_5 \cdot r_6 \cdot \underline{r_5} \cdot r_6 \cdot \overline{X_0 \cdot r_1 \cdot r_2 \cdot X_0} \xrightarrow{\delta_{31}} r_5 \cdot r_6 \cdot \overline{X_0 \cdot r_1 \cdot r_2 \cdot X_0} \cdot X_0 \cdot r_1 \cdot r_2 \cdot X_0 \\
&\xrightarrow{(21)} \underline{r_5 \cdot r_6} \cdot X_0 \cdot r_1 \cdot r_2 \cdot r_1 \cdot r_2 \cdot X_0 \\
&\xrightarrow{\delta_{31}} \overline{X_0 \cdot r_1 \cdot r_2 \cdot X_0} \cdot X_0 \cdot r_1 \cdot r_2 \cdot r_1 \cdot r_2 \cdot X_0 \\
&\xrightarrow{(21)} X_0 \cdot \underline{r_1 \cdot r_2 \cdot r_1 \cdot r_2 \cdot X_0} \xrightarrow{(1;2)} \underline{X_0 \cdot X_0} \xrightarrow{(21)} \varepsilon
\end{aligned}$$

### 1.7.32 Deriving the Coxeter Relation ( 5 ; 7 )

$$\begin{aligned}
(\delta_{32}) : CZ_{0,1} \cdot \underline{r_5} &\xrightarrow{D_6} \underline{CZ_{0,1} \cdot X_1} \cdot \overline{CCX_{0,1} \cdot X_1} \xleftarrow{C_{112}} \overline{X_1 \cdot Z_0} \cdot \underline{CZ_{0,1} \cdot CCX_{0,1} \cdot X_1} \xrightarrow{C_{95}} X_1 \cdot Z_0 \cdot \overline{CCX_{0,1} \cdot CZ_{0,1} \cdot X_1} \\
&\xleftarrow{C_{112}} X_1 \cdot Z_0 \cdot CCX_{0,1} \cdot \overline{X_1 \cdot Z_0 \cdot CZ_{0,1}} \\
&\xrightarrow{B_{15}} X_1 \cdot \underline{Z_0 \cdot CCX_{0,1}} \cdot \overline{Z_0 \cdot X_1} \cdot CZ_{0,1} \\
&\xrightarrow{C_{54}} X_1 \cdot \overline{CCX_{0,1} \cdot Z_0 \cdot Z_0} \cdot X_1 \cdot CZ_{0,1} \\
&\xrightarrow{E_3} \underline{X_1 \cdot CCX_{0,1} \cdot X_1} \cdot CZ_{0,1} \xleftarrow{D_6} \overline{r_5} \cdot CZ_{0,1}
\end{aligned}$$

$$\begin{aligned}
r_5 \cdot r_7 \cdot r_5 \cdot r_7 \cdot r_5 \cdot \underline{r_7} &\xrightarrow{\xi_3} r_5 \cdot r_7 \cdot r_5 \cdot \underline{r_7} \cdot r_5 \cdot \overline{CZ_{0,1} \cdot r_6 \cdot CZ_{0,1}} \xrightarrow{\xi_3} r_5 \cdot r_7 \cdot r_5 \cdot \overline{CZ_{0,1} \cdot r_6 \cdot CZ_{0,1}} \cdot r_5 \cdot CZ_{0,1} \cdot r_6 \cdot CZ_{0,1} \\
&\xrightarrow{\delta_{32}} r_5 \cdot r_7 \cdot r_5 \cdot CZ_{0,1} \cdot r_6 \cdot \overline{r_5 \cdot CZ_{0,1} \cdot CZ_{0,1}} \cdot r_6 \cdot CZ_{0,1} \\
&\xrightarrow{E_2} r_5 \cdot \underline{r_7} \cdot r_5 \cdot CZ_{0,1} \cdot r_6 \cdot r_5 \cdot r_6 \cdot CZ_{0,1} \\
&\xrightarrow{\xi_3} r_5 \cdot \overline{CZ_{0,1} \cdot r_6 \cdot CZ_{0,1}} \cdot r_5 \cdot CZ_{0,1} \cdot r_6 \cdot r_5 \cdot r_6 \cdot CZ_{0,1} \\
&\xrightarrow{\delta_{32}} r_5 \cdot CZ_{0,1} \cdot r_6 \cdot \overline{r_5 \cdot CZ_{0,1}} \cdot CZ_{0,1} \cdot r_6 \cdot r_5 \cdot r_6 \cdot CZ_{0,1} \\
&\xleftarrow{\delta_{32}} \overline{CZ_{0,1} \cdot r_5 \cdot r_6 \cdot r_5 \cdot CZ_{0,1} \cdot CZ_{0,1}} \cdot r_6 \cdot r_5 \cdot r_6 \cdot CZ_{0,1} \\
&\xrightarrow{E_2} CZ_{0,1} \cdot \underline{r_5 \cdot r_6 \cdot r_5 \cdot r_6 \cdot r_5 \cdot r_6 \cdot CZ_{0,1}} \xrightarrow{(5;6)} \underline{CZ_{0,1} \cdot CZ_{0,1}} \xrightarrow{E_2} \varepsilon
\end{aligned}$$

### 1.7.33 Deriving the Coxeter Relation ( 5 ; 8 )

$$\begin{aligned}
(\delta_{33}) : r_5 &\xleftarrow{(21)} \underline{r_5} \cdot \overline{X_0 \cdot X_0} \xrightarrow{D_6} \overline{X_1 \cdot CCX_{0,1} \cdot X_1 \cdot X_0 \cdot X_0} \xleftarrow{(21)} \overline{X_0 \cdot X_0} \cdot X_1 \cdot \overline{CCX_{0,1} \cdot X_1 \cdot X_0 \cdot X_0} \xleftarrow{D_1} X_0 \cdot \overline{r_1} \cdot X_0 \\
r_5 \cdot r_8 \cdot \underline{r_5} \cdot r_8 &\xrightarrow{\delta_{33}} \underline{r_5} \cdot r_8 \cdot \overline{X_0 \cdot r_1 \cdot X_0} \cdot r_8 \xrightarrow{\delta_{33}} \overline{X_0 \cdot r_1 \cdot X_0} \cdot r_8 \cdot X_0 \cdot r_1 \cdot \underline{X_0} \cdot r_8 \xrightarrow{\xi_4} X_0 \cdot r_1 \cdot \underline{X_0 \cdot r_8} \cdot X_0 \cdot r_1 \cdot \overline{X_0} \\
&\xrightarrow{\xi_4} X_0 \cdot r_1 \cdot \overline{X_0 \cdot X_0} \cdot X_0 \cdot r_1 \cdot r_8 \cdot X_0 \\
&\xrightarrow{(21)} X_0 \cdot r_1 \cdot r_8 \cdot r_1 \cdot r_8 \cdot X_0 \xrightarrow{(1;8)} \underline{X_0 \cdot X_0} \xrightarrow{(21)} \varepsilon
\end{aligned}$$

### 1.7.34 Deriving the Coxeter Relation ( 6 ; 7 )

$$r_6 \cdot r_7 \cdot \underline{r_6} \cdot \underline{r_7} \xrightarrow{\omega_1} \underline{r_6 \cdot r_7} \cdot \overline{CZ_{0,2} \cdot CZ_{0,1}} \xrightarrow{\omega_1} \overline{CZ_{0,2} \cdot CZ_{0,1}} \cdot CZ_{0,2} \cdot CZ_{0,1} \xrightarrow{C_{60}} \underline{CZ_{0,2} \cdot CZ_{0,2} \cdot CZ_{0,1}} \cdot CZ_{0,1} \xrightarrow{E_{11}} \underline{CZ_{0,1} \cdot CZ_{0,1}} \xrightarrow{E_2} \varepsilon$$

### 1.7.35 Deriving the Coxeter Relation ( 6 ; 8 )

$$\begin{aligned}
(\delta_{34}) : r_6 &\xleftarrow{(21)} \underline{r_6} \cdot \overline{X_0 \cdot X_0} \xrightarrow{D_6} \overline{CX_{2,1} \cdot CCX_{0,1} \cdot CX_{2,1}} \cdot X_0 \cdot X_0 \xleftarrow{(21)} \overline{X_0 \cdot X_0} \cdot CX_{2,1} \cdot \overline{CCX_{0,1} \cdot CX_{2,1} \cdot X_0 \cdot X_0} \xleftarrow{D_2} X_0 \cdot \overline{r_2} \cdot X_0 \\
(6;8) : r_6 \cdot r_8 \cdot \underline{r_6} \cdot r_8 &\xrightarrow{\delta_{34}} \underline{r_6} \cdot r_8 \cdot \overline{X_0 \cdot r_2 \cdot X_0} \cdot r_8 \xrightarrow{\delta_{34}} \overline{X_0 \cdot r_2 \cdot X_0} \cdot r_8 \cdot X_0 \cdot r_2 \cdot \underline{X_0} \cdot r_8 \xrightarrow{\xi_4} X_0 \cdot r_2 \cdot \underline{X_0 \cdot r_8} \cdot X_0 \cdot r_2 \cdot \overline{r_8} \cdot \overline{X_0} \\
&\xrightarrow{\xi_4} X_0 \cdot r_2 \cdot \overline{X_0 \cdot X_0} \cdot X_0 \cdot r_2 \cdot r_8 \cdot X_0 \\
&\xrightarrow{(21)} X_0 \cdot r_2 \cdot r_8 \cdot r_2 \cdot r_8 \cdot X_0 \xrightarrow{(2;8)} \underline{X_0 \cdot X_0} \xrightarrow{(21)} \varepsilon
\end{aligned}$$

### 1.7.36 Deriving the Coxeter Relation ( 7 ; 8 )

$$\begin{aligned}
(\delta_{35}) : X_2 \cdot X_1 \cdot K_{1,2} \cdot CZ_{0,1} \cdot CZ_{0,2} \cdot \underline{r_8} &\xrightarrow{D_8} X_2 \cdot X_1 \cdot \underline{K_{1,2} \cdot CZ_{0,1}} \cdot CZ_{0,2} \cdot \overline{K_{1,2} \cdot X_1 \cdot X_2 \cdot CZ_{0,2} \cdot CCX_{1,2} \cdot CZ_{0,2} \cdot X_2 \cdot X_1 \cdot K_{1,2}} \\
&\xrightarrow{C_{41}} X_2 \cdot X_1 \cdot \overline{CX_{0,1} \cdot K_{1,2} \cdot CZ_{0,2}} \cdot K_{1,2} \cdot X_1 \cdot X_2 \cdot CZ_{0,2} \cdot CCX_{1,2} \cdot CZ_{0,2} \cdot X_2 \cdot X_1 \cdot K_{1,2} \\
&\xrightarrow{C_{28}} X_2 \cdot X_1 \cdot CX_{0,1} \cdot \overline{CX_{0,2} \cdot K_{1,2}} \cdot K_{1,2} \cdot X_1 \cdot X_2 \cdot CZ_{0,2} \cdot CCX_{1,2} \cdot CZ_{0,2} \cdot X_2 \cdot X_1 \cdot K_{1,2}
\end{aligned}$$

$$\begin{aligned}
& \xrightarrow{(23)} X_2 \cdot X_1 \cdot CX_{0,1} \cdot \overline{CX_{0,2} \cdot X_1 \cdot X_2 \cdot CZ_{0,2} \cdot CCX_{1,2} \cdot CZ_{0,2} \cdot X_2 \cdot X_1 \cdot K_{1,2}} \\
& \xrightarrow{B_3} X_2 \cdot X_1 \cdot \overline{CX_{0,1} \cdot X_1 \cdot CX_{0,2} \cdot X_2 \cdot CZ_{0,2} \cdot CCX_{1,2} \cdot CZ_{0,2} \cdot X_2 \cdot X_1 \cdot K_{1,2}} \\
& \xrightarrow{C_7} X_2 \cdot \overline{CX_{0,1} \cdot X_1 \cdot X_1} \cdot CX_{0,2} \cdot X_2 \cdot CZ_{0,2} \cdot CCX_{1,2} \cdot CZ_{0,2} \cdot X_2 \cdot X_1 \cdot K_{1,2} \\
& \xrightarrow{E_{13}} X_2 \cdot CX_{0,1} \cdot CX_{0,2} \cdot X_2 \cdot CZ_{0,2} \cdot CCX_{1,2} \cdot CZ_{0,2} \cdot X_2 \cdot X_1 \cdot K_{1,2} \\
& \xleftarrow{B_{16}} \overline{CX_{0,1} \cdot X_2 \cdot CX_{0,2} \cdot X_2 \cdot CZ_{0,2} \cdot CCX_{1,2} \cdot CZ_{0,2} \cdot X_2 \cdot X_1 \cdot K_{1,2}} \\
& \xrightarrow{C_{65}} CX_{0,1} \cdot \overline{X_2 \cdot X_2 \cdot CX_{0,2} \cdot CZ_{0,2} \cdot CCX_{1,2} \cdot CZ_{0,2} \cdot X_2 \cdot X_1 \cdot K_{1,2}} \\
& \xrightarrow{E_{17}} CX_{0,1} \cdot CX_{0,2} \cdot CZ_{0,2} \cdot CCX_{1,2} \cdot CZ_{0,2} \cdot X_2 \cdot X_1 \cdot K_{1,2}
\end{aligned}$$

$$\begin{aligned}
(\delta_{36}) : & CX_{0,1} \cdot CCX_{0,1} \cdot \overline{CZ_{1,2} \cdot CCX_{1,2} \cdot CCX_{0,1} \cdot CX_{0,1} \cdot CCX_{1,2}} \\
& \xrightarrow{C_{97}} CX_{0,1} \cdot CCX_{0,1} \cdot \overline{CCX_{1,2} \cdot CZ_{1,2} \cdot CCX_{0,1} \cdot CX_{0,1} \cdot CCX_{1,2}} \\
& \xrightarrow{C_{82}} CX_{0,1} \cdot CCX_{0,1} \cdot CCX_{1,2} \cdot \overline{CCX_{0,1} \cdot CZ_{0,1} \cdot CZ_{1,2}} \cdot CX_{0,1} \cdot CCX_{1,2} \\
& \xrightarrow{(40)} CX_{0,1} \cdot CCX_{0,1} \cdot CCX_{1,2} \cdot CCX_{0,1} \cdot \overline{CZ_{1,2} \cdot CZ_{0,1} \cdot CX_{0,1} \cdot CCX_{1,2}} \\
& \xleftarrow{C_{76}} CX_{0,1} \cdot CCX_{0,1} \cdot CCX_{1,2} \cdot CCX_{0,1} \cdot \overline{CZ_{1,2} \cdot CX_{0,1} \cdot Z_0 \cdot CZ_{0,1} \cdot CCX_{1,2}} \\
& \xrightarrow{C_{75}} CX_{0,1} \cdot CCX_{0,1} \cdot CCX_{1,2} \cdot CCX_{0,1} \cdot \overline{CX_{0,1} \cdot CZ_{0,2} \cdot CZ_{1,2} \cdot Z_0 \cdot CZ_{0,1} \cdot CCX_{1,2}} \\
& \xrightarrow{B_{31}} CX_{0,1} \cdot CCX_{0,1} \cdot CCX_{1,2} \cdot CCX_{0,1} \cdot CX_{0,1} \cdot CZ_{0,2} \cdot \overline{Z_0 \cdot CZ_{1,2} \cdot CZ_{0,1} \cdot CCX_{1,2}} \\
& \xleftarrow{(40)} CX_{0,1} \cdot CCX_{0,1} \cdot CCX_{1,2} \cdot CCX_{0,1} \cdot CX_{0,1} \cdot CZ_{0,2} \cdot Z_0 \cdot \overline{CZ_{0,1} \cdot CZ_{1,2} \cdot CCX_{1,2}} \\
& \xrightarrow{C_{116}} CX_{0,1} \cdot CCX_{0,1} \cdot CCX_{1,2} \cdot CCX_{0,1} \cdot CX_{0,1} \cdot CZ_{0,2} \cdot \overline{Z_0 \cdot CCX_{1,2} \cdot CZ_{0,1}} \\
& \xrightarrow{C_{49}} CX_{0,1} \cdot CCX_{0,1} \cdot CCX_{1,2} \cdot CCX_{0,1} \cdot CX_{0,1} \cdot CZ_{0,2} \cdot \overline{CCX_{1,2} \cdot CZ_{1,2} \cdot Z_0 \cdot CZ_{0,1}} \\
& \xleftarrow{C_{97}} CX_{0,1} \cdot CCX_{0,1} \cdot CCX_{1,2} \cdot CCX_{0,1} \cdot CX_{0,1} \cdot \overline{CZ_{0,2} \cdot CZ_{1,2} \cdot CCX_{1,2} \cdot Z_0 \cdot CZ_{0,1}} \\
& \xleftarrow{C_{101}} CX_{0,1} \cdot \overline{CCX_{0,1} \cdot CCX_{1,2} \cdot CCX_{0,1} \cdot CX_{0,1} \cdot CCX_{1,2} \cdot CZ_{0,2} \cdot Z_0 \cdot CZ_{0,1}} \\
& \xrightarrow{X_{11}} CX_{0,1} \cdot \overline{CCX_{1,2} \cdot CCX_{0,1} \cdot CCX_{1,2} \cdot CX_{0,1} \cdot CCX_{1,2} \cdot CZ_{0,2} \cdot Z_0 \cdot CZ_{0,1}} \\
& \xleftarrow{(22)} CX_{0,1} \cdot CCX_{1,2} \cdot \overline{CX_{0,1} \cdot CX_{0,1} \cdot CCX_{0,1} \cdot CCX_{1,2} \cdot CX_{0,1} \cdot CCX_{1,2} \cdot CZ_{0,2} \cdot Z_0 \cdot CZ_{0,1}} \\
& \xrightarrow{C_{119}} CX_{0,1} \cdot CCX_{1,2} \cdot CX_{0,1} \cdot \overline{CCX_{0,1} \cdot CX_{0,2} \cdot CX_{0,1} \cdot CCX_{1,2} \cdot CX_{0,1} \cdot CCX_{1,2} \cdot CZ_{0,2} \cdot Z_0 \cdot CZ_{0,1}} \\
& \xrightarrow{X_{11}} CX_{0,1} \cdot CCX_{1,2} \cdot CX_{0,1} \cdot CCX_{0,1} \cdot CX_{0,2} \cdot \overline{CCX_{0,2} \cdot CCX_{1,2} \cdot CCX_{0,2}} \cdot CCX_{1,2} \cdot CZ_{0,2} \cdot Z_0 \cdot CZ_{0,1} \\
& \xrightarrow{X_{12}} CX_{0,1} \cdot CCX_{1,2} \cdot CX_{0,1} \cdot CCX_{0,1} \cdot CX_{0,2} \cdot \overline{CCX_{1,2} \cdot CCX_{0,2} \cdot CCX_{1,2} \cdot CCX_{1,2}} \cdot CCX_{1,2} \cdot CZ_{0,2} \cdot Z_0 \cdot CZ_{0,1} \\
& \xrightarrow{(24)} CX_{0,1} \cdot CCX_{1,2} \cdot CX_{0,1} \cdot CCX_{0,1} \cdot CX_{0,2} \cdot CCX_{1,2} \cdot CCX_{0,2} \cdot CZ_{0,2} \cdot Z_0 \cdot CZ_{0,1} \\
& \xleftarrow{E_{15}} CX_{0,1} \cdot CCX_{1,2} \cdot CX_{0,1} \cdot CCX_{0,1} \cdot \overline{CX_{0,2} \cdot CCX_{1,2} \cdot CX_{0,2} \cdot CX_{0,2} \cdot CCX_{0,2} \cdot CZ_{0,2} \cdot Z_0 \cdot CZ_{0,1}} \\
& \xrightarrow{X_4} CX_{0,1} \cdot CCX_{1,2} \cdot CX_{0,1} \cdot \overline{CCX_{0,1} \cdot CCX_{0,1} \cdot CCX_{1,2} \cdot CCX_{0,1} \cdot CX_{0,2} \cdot CCX_{0,2} \cdot CZ_{0,2} \cdot Z_0 \cdot CZ_{0,1}} \\
& \xrightarrow{E_{18}} CX_{0,1} \cdot CCX_{1,2} \cdot CX_{0,1} \cdot CCX_{1,2} \cdot CCX_{0,1} \cdot CX_{0,2} \cdot CCX_{0,2} \cdot CZ_{0,2} \cdot Z_0 \cdot CZ_{0,1} \\
& \xrightarrow{X_1} \overline{CCX_{0,2} \cdot CCX_{1,2} \cdot CCX_{0,2}} \cdot CCX_{1,2} \cdot CCX_{0,1} \cdot CX_{0,2} \cdot CCX_{0,2} \cdot CZ_{0,2} \cdot Z_0 \cdot CZ_{0,1} \\
& \xrightarrow{X_{12}} \overline{CCX_{1,2} \cdot CCX_{0,2} \cdot CCX_{1,2} \cdot CCX_{1,2}} \cdot CCX_{0,1} \cdot CX_{0,2} \cdot CCX_{0,2} \cdot CZ_{0,2} \cdot Z_0 \cdot CZ_{0,1}
\end{aligned}$$

$$\begin{aligned}
& \xrightarrow{(24)} CCX_{1,2} \cdot CCX_{0,2} \cdot CCX_{0,1} \cdot CX_{0,2} \cdot CCX_{0,2} \cdot CZ_{0,2} \cdot Z_0 \cdot CZ_{0,1} \\
& \xleftarrow{E_{11}} CCX_{1,2} \cdot \overline{CZ_{0,2}} \cdot \overline{CZ_{0,2}} \cdot CCX_{0,2} \cdot CCX_{0,1} \cdot CX_{0,2} \cdot CCX_{0,2} \cdot CZ_{0,2} \cdot Z_0 \cdot CZ_{0,1} \\
& \xrightarrow{C_{96}} CCX_{1,2} \cdot CZ_{0,2} \cdot \overline{CCX_{0,2}} \cdot \overline{CZ_{0,2}} \cdot CCX_{0,1} \cdot CX_{0,2} \cdot CCX_{0,2} \cdot CZ_{0,2} \cdot Z_0 \cdot CZ_{0,1} \\
& \xrightarrow{C_{81}} CCX_{1,2} \cdot CZ_{0,2} \cdot CCX_{0,2} \cdot \overline{CCX_{0,1}} \cdot \overline{CZ_{0,1}} \cdot \overline{CZ_{0,2}} \cdot CX_{0,2} \cdot CCX_{0,2} \cdot CZ_{0,2} \cdot Z_0 \cdot CZ_{0,1} \\
& \xrightarrow{C_{60}} CCX_{1,2} \cdot CZ_{0,2} \cdot CCX_{0,2} \cdot CCX_{0,1} \cdot \overline{CZ_{0,2}} \cdot \overline{CZ_{0,1}} \cdot \overline{CX_{0,2}} \cdot CCX_{0,2} \cdot CZ_{0,2} \cdot Z_0 \cdot CZ_{0,1} \\
& \xleftarrow{C_{24}} CCX_{1,2} \cdot CZ_{0,2} \cdot CCX_{0,2} \cdot CCX_{0,1} \cdot CZ_{0,2} \cdot \overline{CX_{0,2}} \cdot \overline{CZ_{0,1}} \cdot \overline{CCX_{0,2}} \cdot CZ_{0,2} \cdot Z_0 \cdot CZ_{0,1} \\
& \xrightarrow{C_{80}} CCX_{1,2} \cdot CZ_{0,2} \cdot CCX_{0,2} \cdot CCX_{0,1} \cdot CZ_{0,2} \cdot CX_{0,2} \cdot \overline{CCX_{0,2}} \cdot \overline{CZ_{0,1}} \cdot \overline{CZ_{0,2}} \cdot CZ_{0,2} \cdot Z_0 \cdot CZ_{0,1} \\
& \xrightarrow{E_{11}} CCX_{1,2} \cdot CZ_{0,2} \cdot CCX_{0,2} \cdot CCX_{0,1} \cdot CZ_{0,2} \cdot CX_{0,2} \cdot CCX_{0,2} \cdot \overline{CZ_{0,1}} \cdot Z_0 \cdot CZ_{0,1} \\
& \xrightarrow{C_{88}} CCX_{1,2} \cdot CZ_{0,2} \cdot CCX_{0,2} \cdot CCX_{0,1} \cdot CZ_{0,2} \cdot CX_{0,2} \cdot CCX_{0,2} \cdot \overline{Z_0} \cdot \overline{CZ_{0,1}} \cdot CZ_{0,1} \\
& \xrightarrow{E_2} CCX_{1,2} \cdot CZ_{0,2} \cdot CCX_{0,2} \cdot CCX_{0,1} \cdot CZ_{0,2} \cdot CX_{0,2} \cdot CCX_{0,2} \cdot Z_0 \\
& \xleftarrow{E_{11}} CCX_{1,2} \cdot CZ_{0,2} \cdot CCX_{0,2} \cdot CCX_{0,1} \cdot CZ_{0,2} \cdot \overline{CX_{0,2}} \cdot \overline{CZ_{0,2}} \cdot \overline{CZ_{0,2}} \cdot CCX_{0,2} \cdot Z_0 \\
& \xleftarrow{C_{63}} CCX_{1,2} \cdot CZ_{0,2} \cdot CCX_{0,2} \cdot CCX_{0,1} \cdot \overline{CZ_{0,2}} \cdot \overline{CZ_{0,2}} \cdot \overline{Z_0} \cdot \overline{CX_{0,2}} \cdot CZ_{0,2} \cdot CCX_{0,2} \cdot Z_0 \\
& \xrightarrow{E_{11}} CCX_{1,2} \cdot CZ_{0,2} \cdot CCX_{0,2} \cdot CCX_{0,1} \cdot \overline{Z_0} \cdot \overline{CX_{0,2}} \cdot CZ_{0,2} \cdot CCX_{0,2} \cdot Z_0 \\
& \xleftarrow{C_{90}} CCX_{1,2} \cdot CZ_{0,2} \cdot CCX_{0,2} \cdot CCX_{0,1} \cdot \overline{CX_{0,2}} \cdot \overline{Z_0} \cdot \overline{CZ_{0,2}} \cdot CCX_{0,2} \cdot Z_0 \\
& \xleftarrow{C_{103}} CCX_{1,2} \cdot CZ_{0,2} \cdot CCX_{0,2} \cdot CCX_{0,1} \cdot CX_{0,2} \cdot \overline{CZ_{0,2}} \cdot \overline{Z_0} \cdot \overline{CCX_{0,2}} \cdot Z_0 \\
& \xrightarrow{C_{58}} CCX_{1,2} \cdot CZ_{0,2} \cdot CCX_{0,2} \cdot CCX_{0,1} \cdot CX_{0,2} \cdot CZ_{0,2} \cdot \overline{CCX_{0,2}} \cdot \overline{Z_0} \cdot Z_0 \\
& \xrightarrow{E_3} CCX_{1,2} \cdot CZ_{0,2} \cdot CCX_{0,2} \cdot CCX_{0,1} \cdot CX_{0,2} \cdot CZ_{0,2} \cdot CCX_{0,2} \\
\\
& (\delta_{37}) : CCX_{0,2} \cdot CCX_{0,1} \cdot CX_{0,2} \cdot CCX_{0,2} \cdot \overline{X_2} \cdot \overline{X_1} \xleftarrow{B_{19}} CCX_{0,2} \cdot CCX_{0,1} \cdot CX_{0,2} \cdot \overline{CCX_{0,2}} \cdot \overline{X_1} \cdot \overline{X_2} \\
& \xleftarrow{C_{37}} CCX_{0,2} \cdot \overline{CCX_{0,1}} \cdot \overline{CX_{0,2}} \cdot \overline{X_1} \cdot \overline{CCX_{0,2}} \cdot X_2 \\
& \xleftarrow{C_{35}} \overline{CCX_{0,2}} \cdot \overline{X_1} \cdot \overline{CCX_{0,1}} \cdot CCX_{0,2} \cdot X_2 \\
& \xleftarrow{C_{37}} \overline{X_1} \cdot \overline{CCX_{0,2}} \cdot CCX_{0,1} \cdot \overline{CCX_{0,2}} \cdot X_2 \\
& \xleftarrow{C_{109}} X_1 \cdot CCX_{0,2} \cdot \overline{CCX_{0,1}} \cdot \overline{X_2} \cdot \overline{CX_{0,1}} \cdot \overline{CCX_{0,2}} \\
& \xleftarrow{C_{39}} X_1 \cdot \overline{CCX_{0,2}} \cdot \overline{X_2} \cdot \overline{CCX_{0,1}} \cdot CX_{0,1} \cdot CCX_{0,2} \\
& \xleftarrow{C_{109}} X_1 \cdot \overline{X_2} \cdot \overline{CX_{0,1}} \cdot \overline{CCX_{0,2}} \cdot CCX_{0,1} \cdot CX_{0,1} \cdot CCX_{0,2} \\
& \xleftarrow{C_{89}} X_1 \cdot X_2 \cdot \overline{CCX_{0,2}} \cdot \overline{CX_{0,1}} \cdot \overline{CCX_{0,1}} \cdot CX_{0,1} \cdot CCX_{0,2} \\
& \xrightarrow{C_{119}} X_1 \cdot X_2 \cdot CCX_{0,2} \cdot \overline{CCX_{0,1}} \cdot \overline{CX_{0,2}} \cdot \overline{CX_{0,1}} \cdot \overline{CX_{0,1}} \cdot CCX_{0,2} \\
& \xrightarrow{(22)} X_1 \cdot X_2 \cdot CCX_{0,2} \cdot \overline{CCX_{0,1}} \cdot \overline{CX_{0,2}} \cdot CCX_{0,2} \\
& \xrightarrow{C_{105}} X_1 \cdot X_2 \cdot CCX_{0,2} \cdot \overline{CX_{0,2}} \cdot \overline{CCX_{0,1}} \cdot CCX_{0,2}
\end{aligned}$$

[illegible]

$$\begin{aligned}
& \xrightarrow{C_{96}} CZ_{0,1} \cdot CZ_{0,2} \cdot K_{1,2} \cdot X_1 \cdot X_2 \cdot CZ_{0,2} \cdot CCX_{1,2} \cdot CZ_{0,2} \cdot CCX_{0,2} \cdot CCX_{0,1} \cdot CX_{0,2} \cdot \overline{CCX_{0,2}} \cdot \overline{CZ_{0,2}} \cdot CZ_{0,2} \cdot X_2 \cdot X_1 \cdot K_{1,2} \\
& \xrightarrow{E_{11}} CZ_{0,1} \cdot CZ_{0,2} \cdot K_{1,2} \cdot X_1 \cdot X_2 \cdot CZ_{0,2} \cdot CCX_{1,2} \cdot CZ_{0,2} \cdot \overline{CCX_{0,2}} \cdot \overline{CCX_{0,1}} \cdot CX_{0,2} \cdot \overline{CCX_{0,2}} \cdot X_2 \cdot X_1 \cdot K_{1,2} \\
& \xrightarrow{\delta_{37}} CZ_{0,1} \cdot CZ_{0,2} \cdot K_{1,2} \cdot X_1 \cdot X_2 \cdot CZ_{0,2} \cdot CCX_{1,2} \cdot CZ_{0,2} \cdot \overline{X_1 \cdot X_2 \cdot CCX_{0,2} \cdot CX_{0,2} \cdot CCX_{0,1} \cdot \overline{CCX_{0,2}}} \cdot K_{1,2} \\
& \xleftarrow{C_1} CZ_{0,1} \cdot CZ_{0,2} \cdot K_{1,2} \cdot X_1 \cdot X_2 \cdot CZ_{0,2} \cdot CCX_{1,2} \cdot CZ_{0,2} \cdot X_1 \cdot X_2 \cdot CCX_{0,2} \cdot CX_{0,2} \cdot \overline{CCX_{0,1} \cdot \overline{K_{1,2}} \cdot \overline{CCX_{0,1}}} \\
& \xrightarrow{C_{38}} CZ_{0,1} \cdot CZ_{0,2} \cdot K_{1,2} \cdot X_1 \cdot X_2 \cdot CZ_{0,2} \cdot CCX_{1,2} \cdot CZ_{0,2} \cdot X_1 \cdot X_2 \cdot CCX_{0,2} \cdot \overline{CX_{0,2} \cdot \overline{K_{1,2}} \cdot \overline{CCX_{0,2}}} \cdot CCX_{0,1} \\
& \xleftarrow{C_{28}} CZ_{0,1} \cdot CZ_{0,2} \cdot K_{1,2} \cdot X_1 \cdot X_2 \cdot CZ_{0,2} \cdot CCX_{1,2} \cdot CZ_{0,2} \cdot X_1 \cdot X_2 \cdot \overline{CCX_{0,2} \cdot \overline{K_{1,2}} \cdot \overline{CZ_{0,2}}} \cdot CCX_{0,2} \cdot CCX_{0,1} \\
& \xleftarrow{C_1} CZ_{0,1} \cdot CZ_{0,2} \cdot K_{1,2} \cdot X_1 \cdot X_2 \cdot CZ_{0,2} \cdot CCX_{1,2} \cdot CZ_{0,2} \cdot \overline{X_1 \cdot X_2 \cdot \overline{K_{1,2}} \cdot \overline{CCX_{0,1}}} \cdot CZ_{0,2} \cdot CCX_{0,2} \cdot CCX_{0,1} \\
& \xrightarrow{B_{19}} CZ_{0,1} \cdot CZ_{0,2} \cdot \overline{K_{1,2} \cdot X_1 \cdot X_2 \cdot CZ_{0,2} \cdot CCX_{1,2} \cdot CZ_{0,2} \cdot \overline{X_2 \cdot X_1 \cdot K_{1,2}}} \cdot CCX_{0,1} \cdot CZ_{0,2} \cdot CCX_{0,2} \cdot CCX_{0,1} \\
& \xleftarrow{D_8} CZ_{0,1} \cdot CZ_{0,2} \cdot \overline{r_8} \cdot CCX_{0,1} \cdot \overline{CZ_{0,2} \cdot CCX_{0,2} \cdot CCX_{0,1}} \\
& \xrightarrow{C_{96}} CZ_{0,1} \cdot CZ_{0,2} \cdot r_8 \cdot CCX_{0,1} \cdot \overline{CCX_{0,2} \cdot \overline{CZ_{0,2} \cdot CCX_{0,1}}} \\
& \xrightarrow{C_{81}} CZ_{0,1} \cdot CZ_{0,2} \cdot r_8 \cdot \overline{CCX_{0,1} \cdot CCX_{0,2} \cdot \overline{CCX_{0,1}}} \cdot CZ_{0,1} \cdot CZ_{0,2} \\
& \xleftarrow{X_9} CZ_{0,1} \cdot CZ_{0,2} \cdot r_8 \cdot \overline{CCX_{0,2} \cdot CCX_{0,1} \cdot CCX_{0,2}} \cdot CZ_{0,1} \cdot CZ_{0,2} \\
& \xleftarrow{X_6} CZ_{0,1} \cdot CZ_{0,2} \cdot r_8 \cdot \overline{CX_{2,1} \cdot CCX_{0,1} \cdot CX_{2,1}} \cdot CZ_{0,1} \cdot CZ_{0,2} \\
& \xleftarrow{D_6} CZ_{0,1} \cdot CZ_{0,2} \cdot r_8 \cdot \overline{r_6} \cdot CZ_{0,1} \cdot CZ_{0,2} \\
\\
& r_7 \cdot r_8 \cdot \overline{r_7} \cdot r_8 \cdot r_7 \cdot r_8 \xrightarrow{\xi_2} \overline{r_7 \cdot r_8 \cdot r_6 \cdot CZ_{0,2} \cdot CZ_{0,1} \cdot r_8 \cdot r_7 \cdot r_8} \xrightarrow{\xi_2} \overline{r_6 \cdot CZ_{0,2} \cdot CZ_{0,1} \cdot r_8 \cdot r_6 \cdot CZ_{0,2} \cdot CZ_{0,1} \cdot r_8 \cdot r_7 \cdot r_8} \\
& \xrightarrow{\xi_3} \overline{CZ_{0,2} \cdot CZ_{0,1} \cdot r_6 \cdot r_8 \cdot r_6 \cdot CZ_{0,2} \cdot CZ_{0,1} \cdot r_8 \cdot r_7 \cdot r_8} \\
& \xleftarrow{(8,8)} CZ_{0,2} \cdot CZ_{0,1} \cdot \overline{r_6 \cdot r_8 \cdot r_6 \cdot \overline{r_8} \cdot r_8} \cdot CZ_{0,2} \cdot CZ_{0,1} \cdot r_8 \cdot r_7 \cdot r_8 \\
\\
& \xrightarrow{(6;8)} CZ_{0,2} \cdot CZ_{0,1} \cdot r_8 \cdot CZ_{0,2} \cdot CZ_{0,1} \cdot r_8 \cdot \overline{r_7} \cdot r_8 \\
& \xrightarrow{\xi_2} CZ_{0,2} \cdot CZ_{0,1} \cdot r_8 \cdot CZ_{0,2} \cdot CZ_{0,1} \cdot r_8 \cdot \overline{r_6 \cdot CZ_{0,2} \cdot CZ_{0,1}} \cdot r_8 \\
& \xrightarrow{\xi_3} CZ_{0,2} \cdot CZ_{0,1} \cdot \overline{r_8 \cdot CZ_{0,2} \cdot CZ_{0,1} \cdot r_8} \cdot \overline{CZ_{0,2} \cdot CZ_{0,1} \cdot r_6 \cdot r_8} \\
& \xrightarrow{\delta_{38}} CZ_{0,2} \cdot CZ_{0,1} \cdot \overline{CZ_{0,1} \cdot CZ_{0,2} \cdot r_8 \cdot r_6 \cdot CZ_{0,1} \cdot CZ_{0,2} \cdot CZ_{0,2} \cdot CZ_{0,1} \cdot r_6 \cdot r_8} \\
\\
& \xrightarrow{E_{11}} CZ_{0,2} \cdot CZ_{0,1} \cdot CZ_{0,1} \cdot CZ_{0,2} \cdot r_8 \cdot r_6 \cdot \overline{CZ_{0,1} \cdot CZ_{0,1} \cdot r_6 \cdot r_8} \\
& \xrightarrow{E_2} CZ_{0,2} \cdot \overline{CZ_{0,1} \cdot CZ_{0,1}} \cdot CZ_{0,2} \cdot r_8 \cdot r_6 \cdot r_6 \cdot r_8 \\
& \xrightarrow{E_2} CZ_{0,2} \cdot CZ_{0,2} \cdot r_8 \cdot r_6 \cdot r_6 \cdot r_8 \\
& \xrightarrow{E_{11}} r_8 \cdot \overline{r_6 \cdot r_6} \cdot r_8 \\
& \xrightarrow{(6;6)} r_8 \cdot r_8 \\
& \xrightarrow{(8,8)} \varepsilon
\end{aligned}$$
